# Supplementary material for: Robust 3D Object Detection from LiDAR-Radar Point Clouds via Cross-Modal Feature Augmentation
Source: arXiv:2309.17336 source file (2024-03-12)
Supplement: Supplementary file 1 [file supp.tex]

\section{Supplementary}
\subsection{Notation}

For the reader's convenience, all mathematical notation used \gab{@JN `in the main text'?} is summarized in Tab.~\ref{tab:notationtable} with definitions.

\begin{table}[t!]
\caption{Notation used in the main text \chris{@GC, use small font for this table. Ugly.}}
\begin{tabularx}{0.5\textwidth}{@{}XX@{}}
\toprule
Symbol & Definition \\
\hline
\hline
 $p_i \in \mathbb{R}^{3+A}$ & a single input point \\
 $\mathbf{P} \in \mathbb{R}^{N\times (3+A)}$ & Set of input point cloud \\ 
  $N$ & Number of input points \\
  $A$ & Dimension of raw point attribute \\
  $p_i = [t_i, f_i^A]$ & single point \\
  $t_i \in \mathbb{R}^3$ & Position of point $i$\\
  $f_i \in \mathbb{R}^A$ & raw point attributes \\
  {$\!\begin{aligned} 
  \mathbf{Q}&= \{q_1, q_2, \cdots, q_k\}   \\
  &\in \mathbb{R}^{N_f\times(3+D)}
  \end{aligned}$} & Foreground point cloud\\
  $N_f$ & Number of foreground points \\
  $D$ & Dimension of latent features \\
  $\hat{o}_i$ & Predicted offset during clustering \\ 
  $\hat{t}_i$ & $t_i+\hat{o}_i$, shifted point\\ 
  $\mathcal{L}_{O-Reg}$ & Offset regression loss\\
  $\mathbf{IM}$ & Instance mask, 1 if point in object\\ 
  $\mathbf{C}$ & Set of points after self-clustering\\ 
  $c_i=[\hat{t}_i,f_i^D]$ & A point $i$ after self-clustering\\
  $X$ & Primary modality domain \\
  $\hat{X}$ & Auxiliary modality domain \\ 
  $T$ & Shared common space \\
  $F_{pri}$ & Mapping from $X$ to $T$\\
  $F_{aux}$ & Mapping from $\hat{X}$ to $T$ \\ 
  $N_p$ & Number of pairs chosen for matching\\
  $\mathcal{L}_{FM}$ & Cross-modal hallucination loss\\
  $\mathcal{L}_{ref}$ & Refinement loss\\
  $\mathcal{L}_{cls}$ & Classification loss \\
  $\mathcal{L}_{S-Det}$ &  Shared head loss \\
  $\mathcal{L}_{s1}$ & Stage one training loss\\
  $\mathcal{L}_{s2}$ & Stage two training loss\\
\bottomrule
\end{tabularx}
\label{tab:notationtable}
\end{table}

\subsection{Model Details}

Here we provide the detailed architecture of our framework. The proposed framework mainly consists of 4 parts: 

\noindent{\textbf{Backbone} }

In this work, we adopt a point-based backbone for feature extraction using SA (Set-Abstraction) layers \cite{qi2017pointnet++} with center-awared sampling. We use two different radii in each SA layer for ball query grouping. The notation for SA layer is defined as: $$SA(npoints, [radii], [num\_query], [dimension]]$$, where $npoints$ denotes the selected center points for ball query, $radii$ denotes the ball query radii, $num\_query$ denotes the number of grouped points and the $dimension$ denotes the feature dimension. The notation for MLP is defined as: $$MLP(dim_0 \rightarrow dim_1 \rightarrow \cdots \rightarrow dim_k)$$ And the concatenation operation is defined as $$CAT(dim_0, dim_1, \cdots, dim_k)$$Thus, the backbone we used for LiDAR inputs is defined as follows:

\begin{gather*}
    SA(4096, [0.2, 0.8], [16, 32], [[16, 16, 32], [32, 32, 64]) \\
    MLP(CAT(32,64) \rightarrow 64) \\
    SA(1024, [0.8, 1.6], [16, 32], [[64, 64, 128], [64, 96, 128]) \\
    MLP(CAT(128, 128) \rightarrow 128)\\
    SA(512, [1.6, 4.8], [16, 32], [[128, 128, 256], [128, 256, 256]) \\
    MLP(CAT(256, 256) \rightarrow 256)
    \label{def:LiDAR_BB}
\end{gather*}

The backbone we used for radar inputs is defined as follows:
\begin{gather*}
    SA(512, [0.2, 0.8], [16, 32], [[16, 16, 32], [32, 32, 64]) \\
    MLP(CAT(32,64) \rightarrow 64) \\
    SA(512, [0.8, 1.6], [16, 32], [[64, 64, 128], [64, 96, 128]) \\
    MLP(CAT(128, 128) \rightarrow 128)\\
    SA(256, [1.6, 4.8], [16, 32], [[128, 128, 256], [128, 256, 256]) \\
    MLP(CAT(256, 256) \rightarrow 256)
    \label{def:radar_BB}
\end{gather*}

\noindent{\textbf{Self-clustering Module}}

The self-clustering module contains two parts. The first part is offset regression, which is defined as:
\begin{gather*}
    MLP(256 \rightarrow 128 \rightarrow 3)
\end{gather*}
The above definition applies for both LiDAR and radar. 

The second part is the cluster integration, definition for both LiDAR and radar inputs:

\begin{gather*}
    SA(256, [4.8, 6.4], [16, 32], [[256, 256, 512], [256, 512, 1024]])\\
    MLP(CAT(512, 1024) \rightarrow 512)
\end{gather*}

\noindent{\textbf{Feature Projection Module}}

The feature projection module contains a 4-layer MLP, which shares the same setting for both LiDAR and radar features as:

\begin{gather*}
    MLP(512 \rightarrow 512 \rightarrow 512 \rightarrow 512)
\end{gather*}

\noindent{\textbf{Detection Head}}

The detection head contains two branches, one for bounding box classification, one for regression. And they are defined as follows in both radar and LiDAR:

\begin{gather*}
    cls \;branch: MLP(CAT(512, 512) \rightarrow 256\rightarrow 256\rightarrow 3) \\
    reg \;branch: MLP(CAT(512, 512) \rightarrow 256\rightarrow 256\rightarrow 30)
\end{gather*}

\subsection{Implementation details}

\noindent{\textbf{Data Augmentation}}

For the training of baseline models for LiDAR, we apply two level data augmentation, including scene-level and object level. The detail settings are as follows:

\noindent{\textbf{Scene-level augmentation}}

\begin{itemize}
    \item Random world flip along x axis.
    \item Random world rotation along z axis with random angle with range $[ -\frac{\pi}{4}, \frac{\pi}{4}]$.
    \item Random world scaling with random factors with range $[0.95, 1.05]$
\end{itemize}

\noindent{\textbf{Object-level augmentation}}
\begin{itemize}
    \item Random sample objects from other scenes containing more than 5 points to the current scene. Number of sampled objects per class is: 20 for cars, 15 for pedestrians and 15 for cyclists. 
\end{itemize}

As stated in \cite{vod}, the above mentioned data augmentation methods is violated to radar velocity measurements. Thus, we disable the augmentation methods in radar model except the random world flip. 

\noindent{\textbf{Baseline Implementation}}

The baseline models reported in this paper is implemented in OpenPCD\footnote{https://github.com/open-mmlab/OpenPCDet.git} library. Most of them are available as official implementations. One exception is the 3DSSD, we use the implementation in this github repo\footnote{https://github.com/qiqihaer/3DSSD-pytorch-openPCDet.git}. For all those baselines, we train for 80 epochs with maximun batch size available on RTX 3090 and keep other settings as it is defined in the original configuration files. 

\noindent{\textbf{Training settings for our method}}

For our methods, we carried out 2-stage training to stablize the training process. 

\noindent{\textbf{First stage}} The first stage training for backbone weights initialization is exactly the same with baseline models stated above. The number of points we used for LiDAR is set to 16384 and radar is 512. We use learning rate of 0.01 and adam one-cycle optimizer with weight decay of 0.2 and momentum of 0.9. 

\noindent{\textbf{Second stage}} In the second stage training, the weights for backbone and self-clustering module is initialized from the model we trained from the first stage. In this stage, we disable all the augmentation methods mentioned above for radar point cloud consistency. The radius we used for selective matching is set to 1 meter. The learning rate is set to be 1e-4 with the same optimizer used in stage one. The predicted object proposals are filtered using NMS with an IoU threshold of 0.01. 

\subsection{More Experiments on VOD}

\subsubsection{Effect of training constraints}
We further explore the contribution of our feature-matching loss and shared detection loss to the performance by training our pipeline without $\mathcal{L}_{FM}$ and $\mathcal{L}_{S-Det}$ with LiDAR as the primary modality. The result in Tab.~\ref{tab:ablation_loss_function} clearly shows a performance increase when $\mathcal{L}_{FM}$ is enabled, comparing the first two rows. The feature-matching loss increases the mAP by more than 7 points, which proves that our proposed method can effectively utilize the information from cross-modal features. Besides, comparing the last two rows, we gain about 1 point improvement for mAP with $\mathcal{L}_{S-Det}$. This improvement shows that constraints from the shared detection head help the projection module generate meaningful shared space features in a task-specific manner. Again, similar conclusions are observed for radar detection, and we omit its discussion to avoid repetition.

\begin{table}[t!]
    \centering
    \resizebox{\columnwidth}{!}{
    \begin{tabular}{c|cc|cccc}
    \hline
        \multirow{2}{*}{Modality} & \multirow{2}{*}{$\mathcal{L}_{FM}$}  & \multirow{2}{*}{$\mathcal{L}_{S-Det}$} & Car & Pedestrian & Cyclist & \multirow{2}{*}{mAP} \\
        & & & (IoU=0.7) & (IoU=0.5) & (IoU=0.5)& \\
        \hline
         \multirow{3}{*}{LiDAR}& & & 48.86 & 48.91 & 67.88 & 55.22  \\
         \cline{2-7}
         & $\checkmark$& & 58.22 & 54.35 & 76.62 & 63.06  \\
        \cline{2-7}
         & $\checkmark$& $\checkmark$& \textbf{58.82} & \textbf{56.29} & \textbf{78.17} & \textbf{64.42} \\
        \hline
    \end{tabular}
    }
    \caption{Ablation on feature matching loss $\mathcal{L}_{FM}$ and shared detection head loss $\mathcal{L}_{S-Det}$}
    \label{tab:ablation_loss_function}
\end{table}
\subsubsection{Improvements from the backbone}

\begin{table*}[t!]
\centering
\vspace{2pt}
\resizebox{\textwidth}{!}{
\SetTblrInner{rowsep=0.5pt,colsep=4pt}
\begin{tblr}{c|c|c c c c|c c c c|c c c c}
\hline
\SetCell[r=2]{c} Backbone & \SetCell[r=2]{c} Modality
 & \SetCell[c=4]{c} Car
 & & & &\SetCell[c=4]{c} Pedestrian
 & & & &\SetCell[c=4]{c} Cyclist & & &\\
%  \hline
 & & 0  & 1-5  & 5-20  & $\geq$20  & 0  & 1-5 & 5-20 & $\geq$20  & 0  & 1-5 & 5-20 & $\geq$20   \\
\hline
Base Model & \SetCell[r=2]{c} radar & 43.2\% &12.0\%&24.2\%&20.5\%&54.0\%&13.1\%&25.1\%&7.7\%&21.1\%&10.5\%&40.3\%&28.1\%\\
Full Model&&41.6\%&15.0\%&27.1\%&16.4\%&49.0\%&15.9\%&27.6\%&7.5\%&19.2\%&10.0\%&48.3\%&22.6\%\\
\hline
Base Model&\SetCell[r=2]{c}LiDAR&7.5\%&9.7\%&31.3\%&51.5\%&57.8\%&20.4\%&18.7\%&3.2\%&20.8\%&13.2\%&43.2\%&22.8\%\\
Full Model&&7.3\%&10.4\%&36.5\%&45.8\%&15.8\%&21.1\%&55.5\%&7.7\%&7.2\%&7.5\%&63.7\%&21.7\%\\
\hline
\end{tblr}
}
\caption{Percentage of instance boxes w.r.t number of points in the final layer. The 'Base Model' refers to the model trained without cross-modal supervision. And the 'Full Model' refers to backbone trained with cross-modal supervision.}
\label{tab:final_pts_in_gt_box}
\end{table*}

To find out why the detection performance get improved with backbone trained with cross-modal supervision even without the hallucination branch. We gather the statistic results on the backbone output, as shown in Table \ref{tab:final_pts_in_gt_box}. We can see that percentage of instance boxes with 0 points drops when we introduce cross-modal supervision for both LiDAR and radar, which means the instance recall rates is improved. Besides, the percentage of instance boxes with points between 5-20 points get increased in all three classes, especially for pedestrian and cyclist on LiDAR. Such improvement leads to the performance boost for object detection in both modality.

\subsubsection{What is the best subspace dimension}

To find out the best dimension for the shared space of both modalities, we conduct experiments with LiDAR inputs as the primary modal data. Note that the backbone outputs per point feature vector with dimension of 512, we will project this feature to different size with a 4-layer MLP module. The dimension will decrease or increase by a step size of 128 and until they reach the target size. Detail results are shown in Table \ref{tab:sub_space}. 

\begin{table}[t!]
    \centering
    \resizebox{\linewidth}{!}{
    \SetTblrInner{rowsep=0.5pt,colsep=4pt}
    \begin{tblr}{c|cccc}
    \hline
         \SetCell[r=2]{c}Feature Size& Car & Pedestrian & Cyclist & \SetCell[r=2]{c}mAP \\
         & (IoU=0.7) & (IoU=0.5) & (IoU=0.5) & \\
         \hline
         128 & 57.70 & 48.91 & 68.60 & 58.40 \\
         256 & 57.63 & 49.92& 76.39 & 61.31 \\
         512 & \textbf{58.82}&	\textbf{56.29}&	\textbf{78.17}&	\textbf{64.42}\\
         640 & 58.79&	49.20&	77.01&	61.66\\
         768 & 56.43&	47.14&	76.50&	60.02\\
         1024 & 58.65&	50.04&	76.75&	61.81\\
         \hline
    \end{tblr}
    }
    \caption{Performance results w.r.t shared feature space dimension between modalities. Best performance is shown in \textbf{bold}}
    \label{tab:sub_space}
\end{table}

\subsubsection{More quantitative results}

\begin{table*}[t!]
\centering
\vspace{2pt}
% \SetTblrInner{rowsep=0.5pt,colsep=4pt}
\resizebox{\textwidth}{!}{
\SetTblrInner{rowsep=0.5pt,colsep=4pt}
\begin{tblr}{c|c|c c c c|c c c c|c c c c}
\hline
\SetCell[r=2]{c} Method & \SetCell[r=2]{c} Modality
 & \SetCell[c=4]{c} Car(IoU=0.5)
 & & & &\SetCell[c=4]{c} Pedestrian(IoU=0.25)
 & & & &\SetCell[c=4]{c} Cyclist(IoU=0.25) & & &\\
%  \hline
 & & overall& 0-5 & 5-10 & $>$10 & overall& 0-5 & 5-10 & $>$10 & overall& 0-5 & 5-10 & $>$10  \\
\hline
pointpillar\cite{pointpillar} & \SetCell[r=3]{c} Radar & {30.93} & \textbf{18.90} & 45.54 & 53.11& 26.17 & 22.98 & 39.36 & 11.08 &61.07 &45.83 &70.27 &65.22  \\
\hline
IASSD\cite{zhang2022not} &  & 31.24 & 14.39& 48.11& \textbf{67.25} & 32.50 & 29.94 &61.23 &21.57 & 60.69 &47.54 &80.27 &\textbf{70.25} \\
\hline
\textbf{Ours} & & \textbf{32.02}& 18.20& \textbf{51.37}& 66.97 & \textbf{40.42} & \textbf{31.98} & \textbf{68.50} & \textbf{40.91} &\textbf{68.67} & \textbf{49.73} &\textbf{83.24} &68.56\\
\hline 
\hline
  & 
 & \SetCell[c=4]{c} Car(IoU=0.7)
 & & & &\SetCell[c=4]{c} Pedestrian(IoU=0.5)
 & & & &\SetCell[c=4]{c} Cyclist(IoU=0.5) & & &\\
%  \hline
 & & overall& 0-40 & 40-100 & $>$100 & overall& 0-40 & 40-100 & $>$100 & overall& 0-40 & 40-100 & $>$100  \\
\hline
pointpillar\cite{pointpillar} & \SetCell[r=3]{c} LiDAR &  40.30 & 6.88& 19.02& 58.32 & 44.06 & 3.91 & 25.83 &48.02 &64.65 &8.77 &32.46 &78.09 \\
\hline
IASSD\cite{zhang2022not} &  & 57.94 & 12.73 & 46.55& 75.14 & 29.40 & 3.30 &9.78 & 32.54 &68.26 &6.09 &60.10 &71.87 \\
\hline
\textbf{Ours} &  & \textbf{58.82}& \textbf{18.62}& \textbf{48.15}& \textbf{76.74} & \textbf{56.29} & \textbf{7.23} & \textbf{47.40} & \textbf{66.48} &\textbf{78.17} &\textbf{16.59} &\textbf{69.89} & \textbf{87.00} \\
\hline 
\end{tblr}
}
 \caption{Detection performance on VOD validation set w.r.t number of points per object. The best results are showed in \textbf{bold}. }
 
\label{tab:ablation_mAP_points}
\end{table*}

\begin{table*}[t!]
\centering
\vspace{2pt}

\resizebox{\textwidth}{!}{

\SetTblrInner{rowsep=0.5pt,colsep=4pt}
\begin{tblr}{c|c|c c c c|c c c c|c c c c}
\hline
\SetCell[r=2]{c} Method & \SetCell[r=2]{c} Modality
 & \SetCell[c=4]{c} Car(IoU=0.5)
 & & & &\SetCell[c=4]{c} Pedestrian(IoU=0.25)
 & & & &\SetCell[c=4]{c} Cyclist(IoU=0.25) & & &\\
%  \hline
 & & overall& 0-20 m  & 20-40 m  & $>$40 m & overall& 0-20 m  & 20-40 m  & $>$40 m & overall&0-20 m  & 20-40 m  & $>$40 m &  \\
\hline
pointpillar\cite{pointpillar} & \SetCell[r=3]{c} Radar&  30.93 & 46.83  & \textbf{27.04}  & 3.66 & 26.17& 31.62  & 16.68  & 1.49 &61.07 &60.40  & 58.86  & 7.07\\
\hline
IASSD\cite{zhang2022not} & &  31.24 & \textbf{55.92}  & 20.26  & 3.65 & 32.50& 39.19  & 25.04  & 3.20 &60.69 &66.01  & 64.36  & 13.68 \\
\hline
\textbf{Ours} & &  \textbf{32.02} & 55.66&25.81& \textbf{4.16}& \textbf{40.42}& \textbf{47.54}  & \textbf{26.80}  & \textbf{6.19} &\textbf{68.67} &\textbf{73.68}  & \textbf{66.27}  & \textbf{22.56} \\
\hline  
\hline
 & 
 & \SetCell[c=4]{c} Car(IoU=0.7)
 & & & &\SetCell[c=4]{c} Pedestrian(IoU=0.5)
 & & & &\SetCell[c=4]{c} Cyclist(IoU=0.5) & & &\\
%  \hline
 & & overall&0-20 m  & 20-40 m  & $>$40 m & overall& 0-20 m  & 20-40 m  & $>$40 m & overall&0-20 m  & 20-40 m  & $>$40 m &  \\
\hline
pointpillar\cite{pointpillar} & \SetCell[r=3]{c} LiDAR &  40.30 &61.51& 37.46&5.75 & 44.06 & 43.28&29.76&3.09 &64.65 &67.76& 62.26& 13.98 \\
\hline
IASSD\cite{zhang2022not} &  & 57.94 & \textbf{70.62}& \textbf{64.66}& 19.05& 29.40 & 36.91 & 7.92& 2.55 & 68.26 &73.09& 59.38& 23.21\\
\hline
\textbf{Ours} & & \textbf{58.82}  & 70.37& 64.62&\textbf{19.33} & \textbf{56.29}& \textbf{62.87}& \textbf{46.91}& \textbf{6.49} &\textbf{78.17} & \textbf{82.65}&\textbf{76.96}&\textbf{26.28}\\
\hline 
\end{tblr}}
 \caption{Detection performance on VOD validation set w.r.t distance. The best results are showed in \textbf{bold}. }
 
\label{tab:mAP_distance}
\end{table*}

Here we provide more evaluation statistics of our method with the re-proposed pointpillar used in \cite{vod} and the recently proposed memory efficient model \cite{zhang2022not}. Results in Table \ref{tab:ablation_mAP_points} shows that our method perform outperform the other methods with a large margin for pedestrians and cyclists. This result is correspondent to the Table \ref{tab:final_pts_in_gt_box}. The backbone network trained with cross-modal supervision get improved on foreground sampling, which helps locate objects with less points like pedestrians and cyclist. Besides, improvements for objects with more than 100 points indicates that the generated hallucination features help the detection head to predict more accurate bounding boxes. However, the improvement for radar vehicle detection is marginal. This is mainly because the hallucination can not fully make up the poor geometry information for radar point clouds, which remains difficult to regress accurate bounding box for larger objects like Cars. Similar results are also presented in Table. \ref{tab:mAP_distance}, our method gain considerable performance boost for distant pedestrians and cyclists compared to other methods. All the above-mentioned results prove that the superiority for small object detection of our method.

\subsection{More qualitative evaluation}

\subsubsection{LiDAR object detection}

\subsubsection{Radar object detection}

\begin{figure*}[t!]
    \begin{minipage}[t!]{.22\textwidth}
        \centering
        \begin{subfigure}{.5\textwidth}
            \caption{Ground-truth}
        \end{subfigure}%
        \begin{subfigure}{\textwidth}
            \centering
            \includegraphics[width=\textwidth]{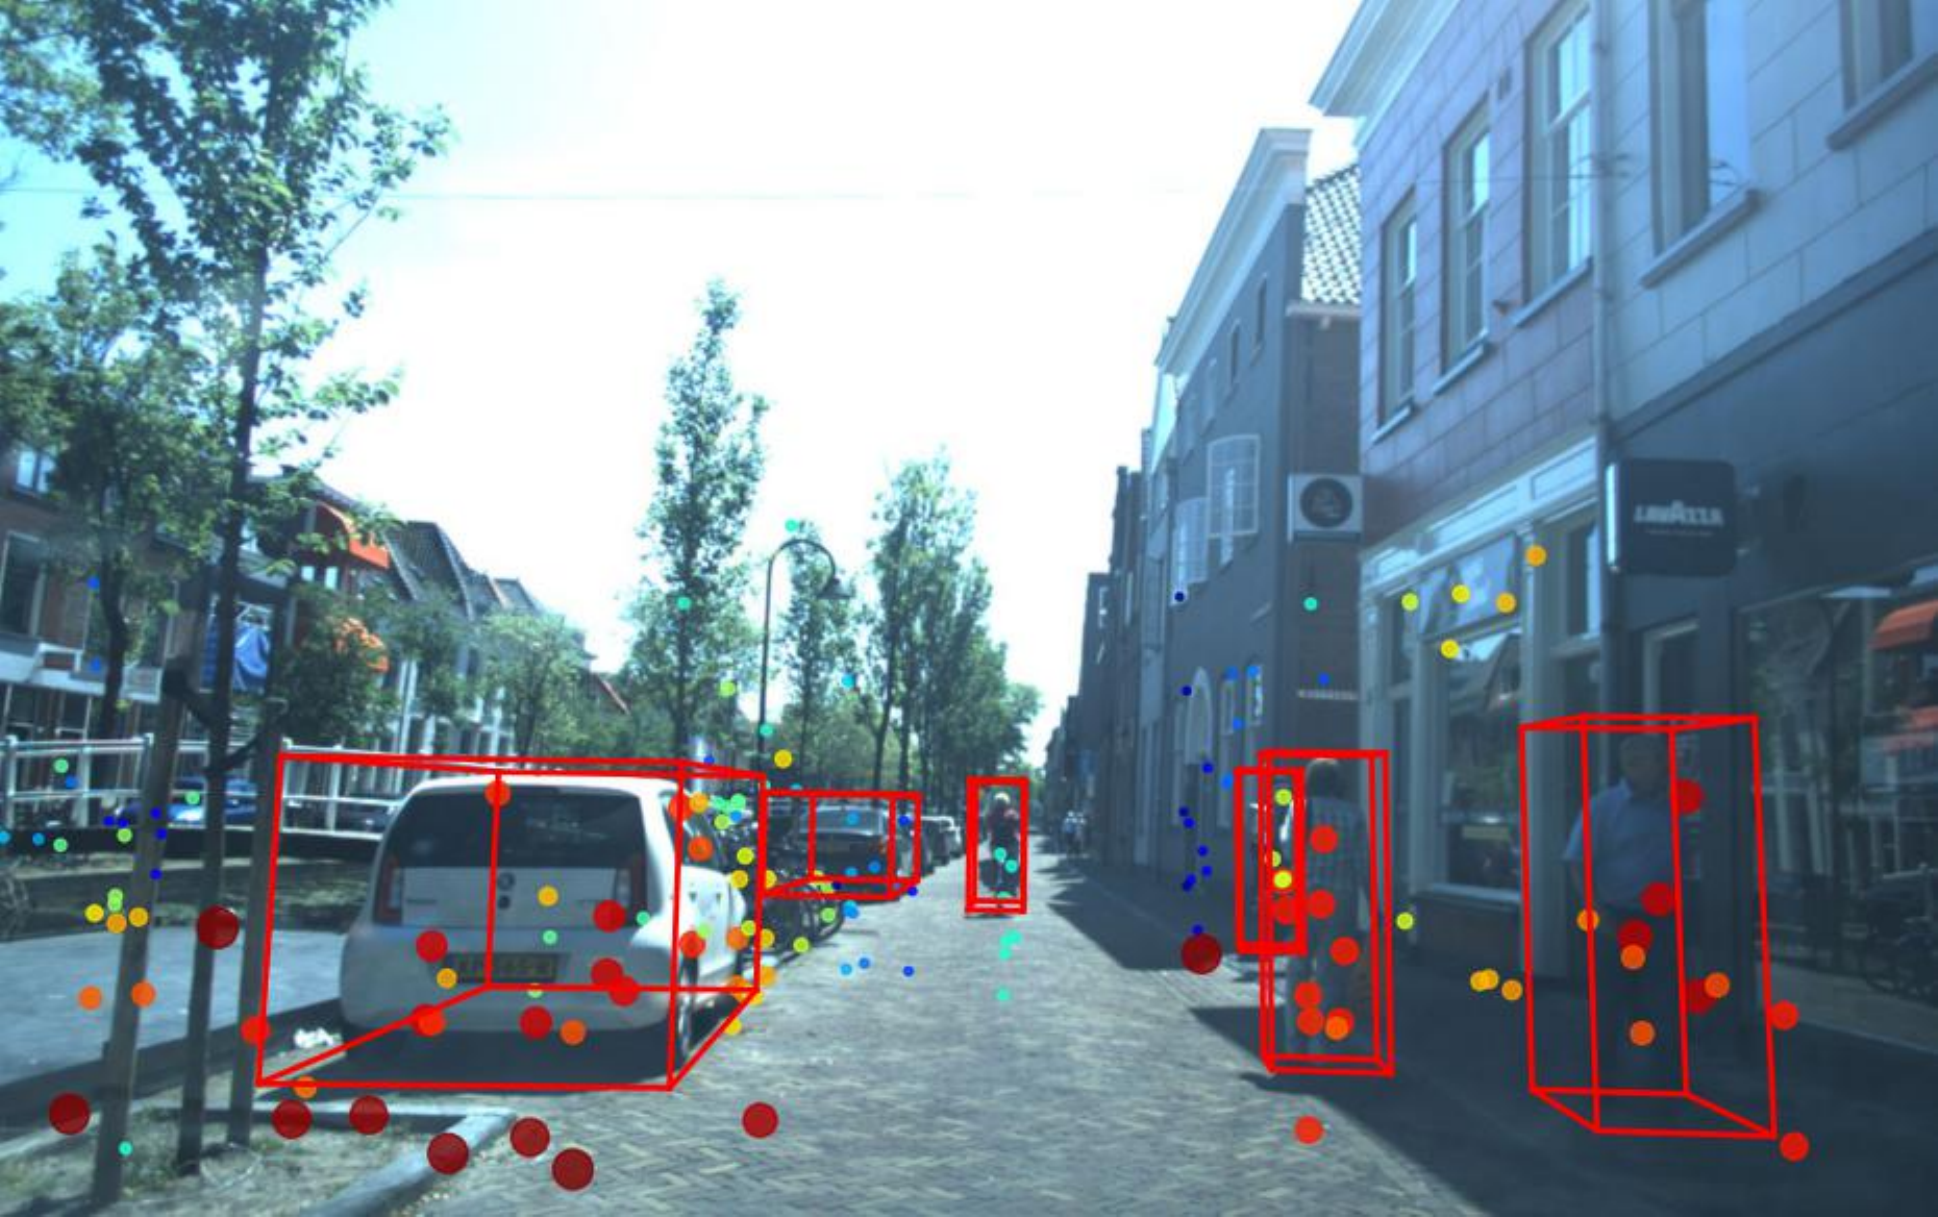}
        \end{subfigure}%
        \begin{subfigure}{\textwidth}
            \centering
            \includegraphics[width=\textwidth]{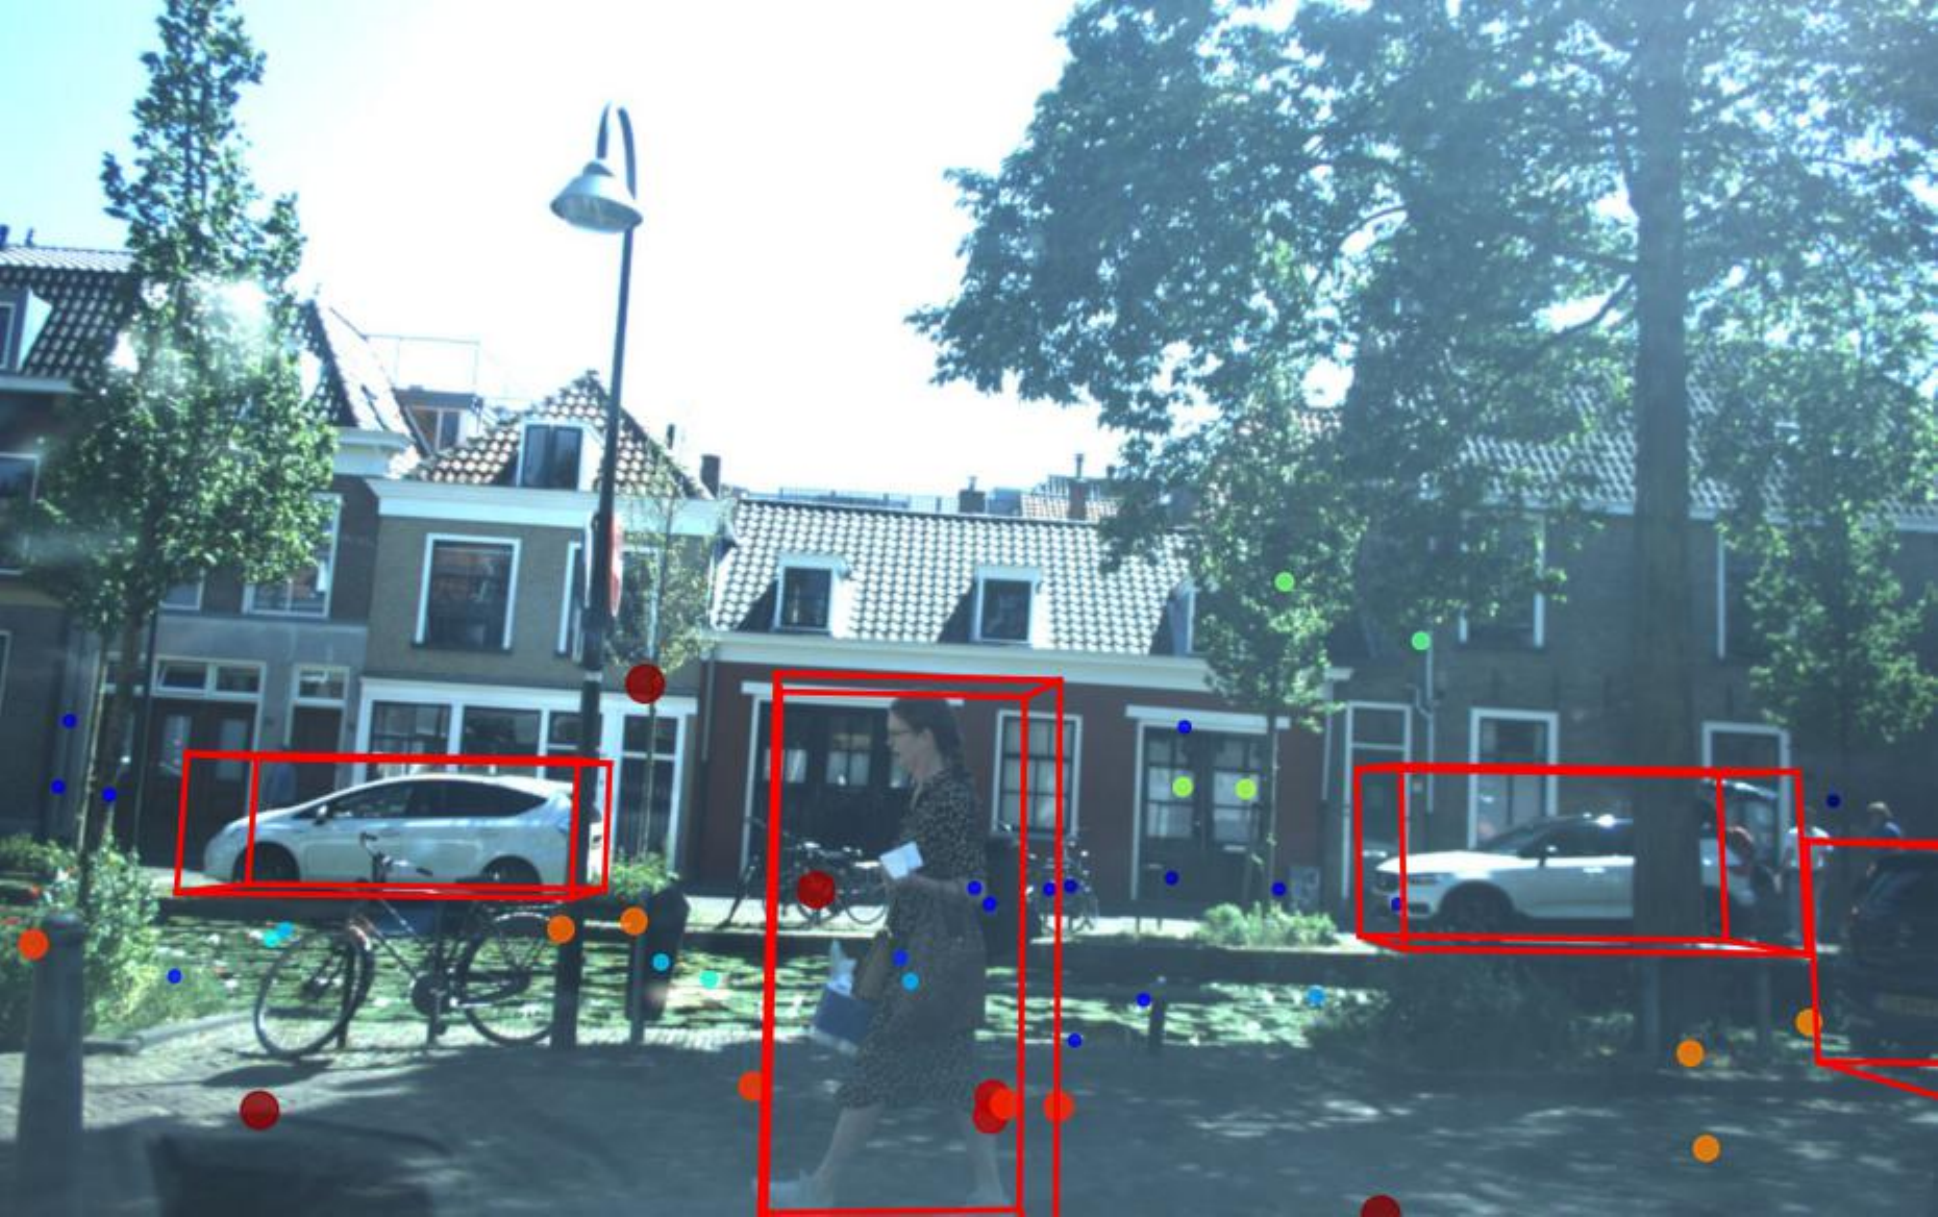}
        \end{subfigure}%
        \begin{subfigure}{\textwidth}
            \centering
            \includegraphics[width=\textwidth]{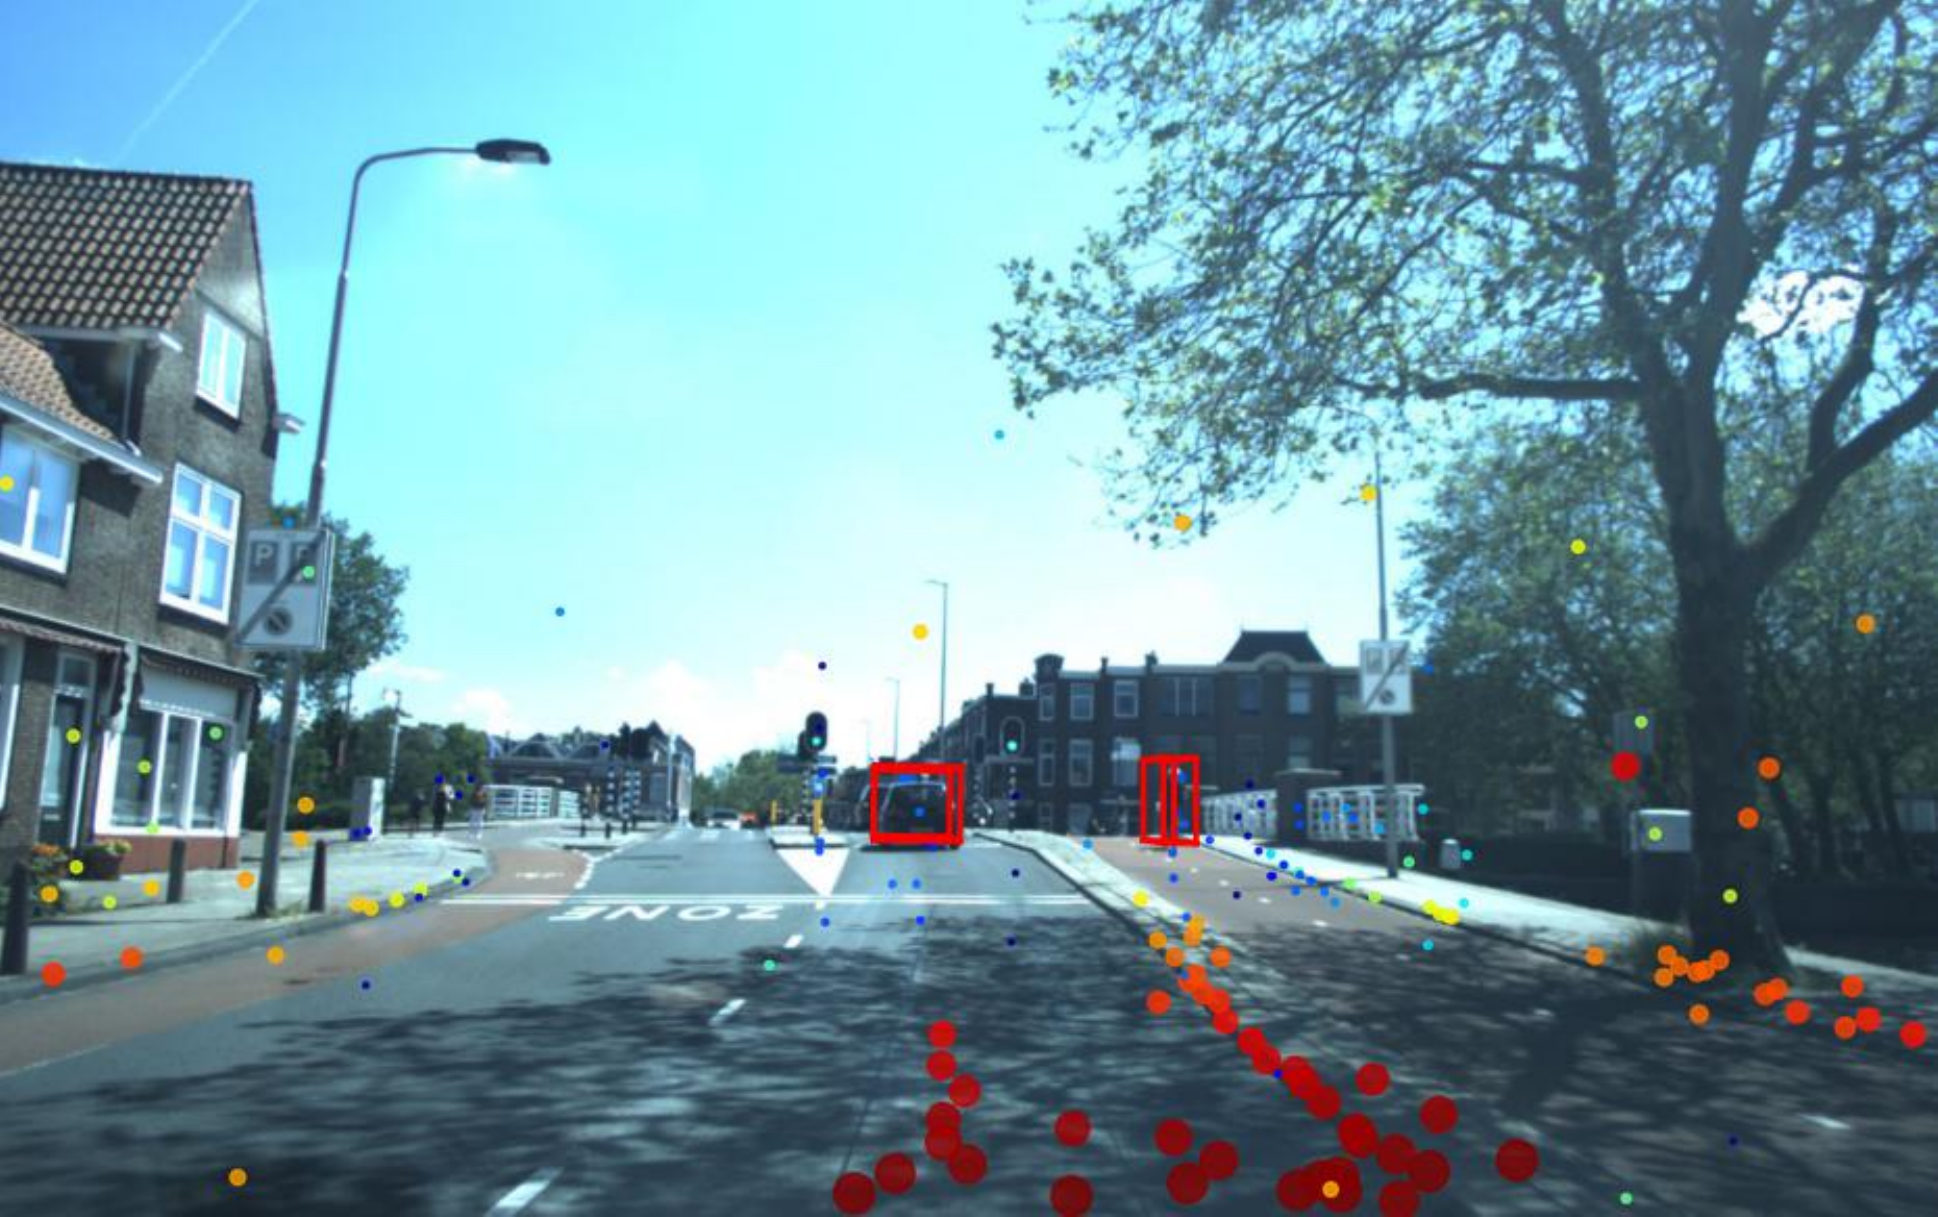}
        \end{subfigure}%
        \begin{subfigure}{\textwidth}
            \centering
            \includegraphics[width=\textwidth]{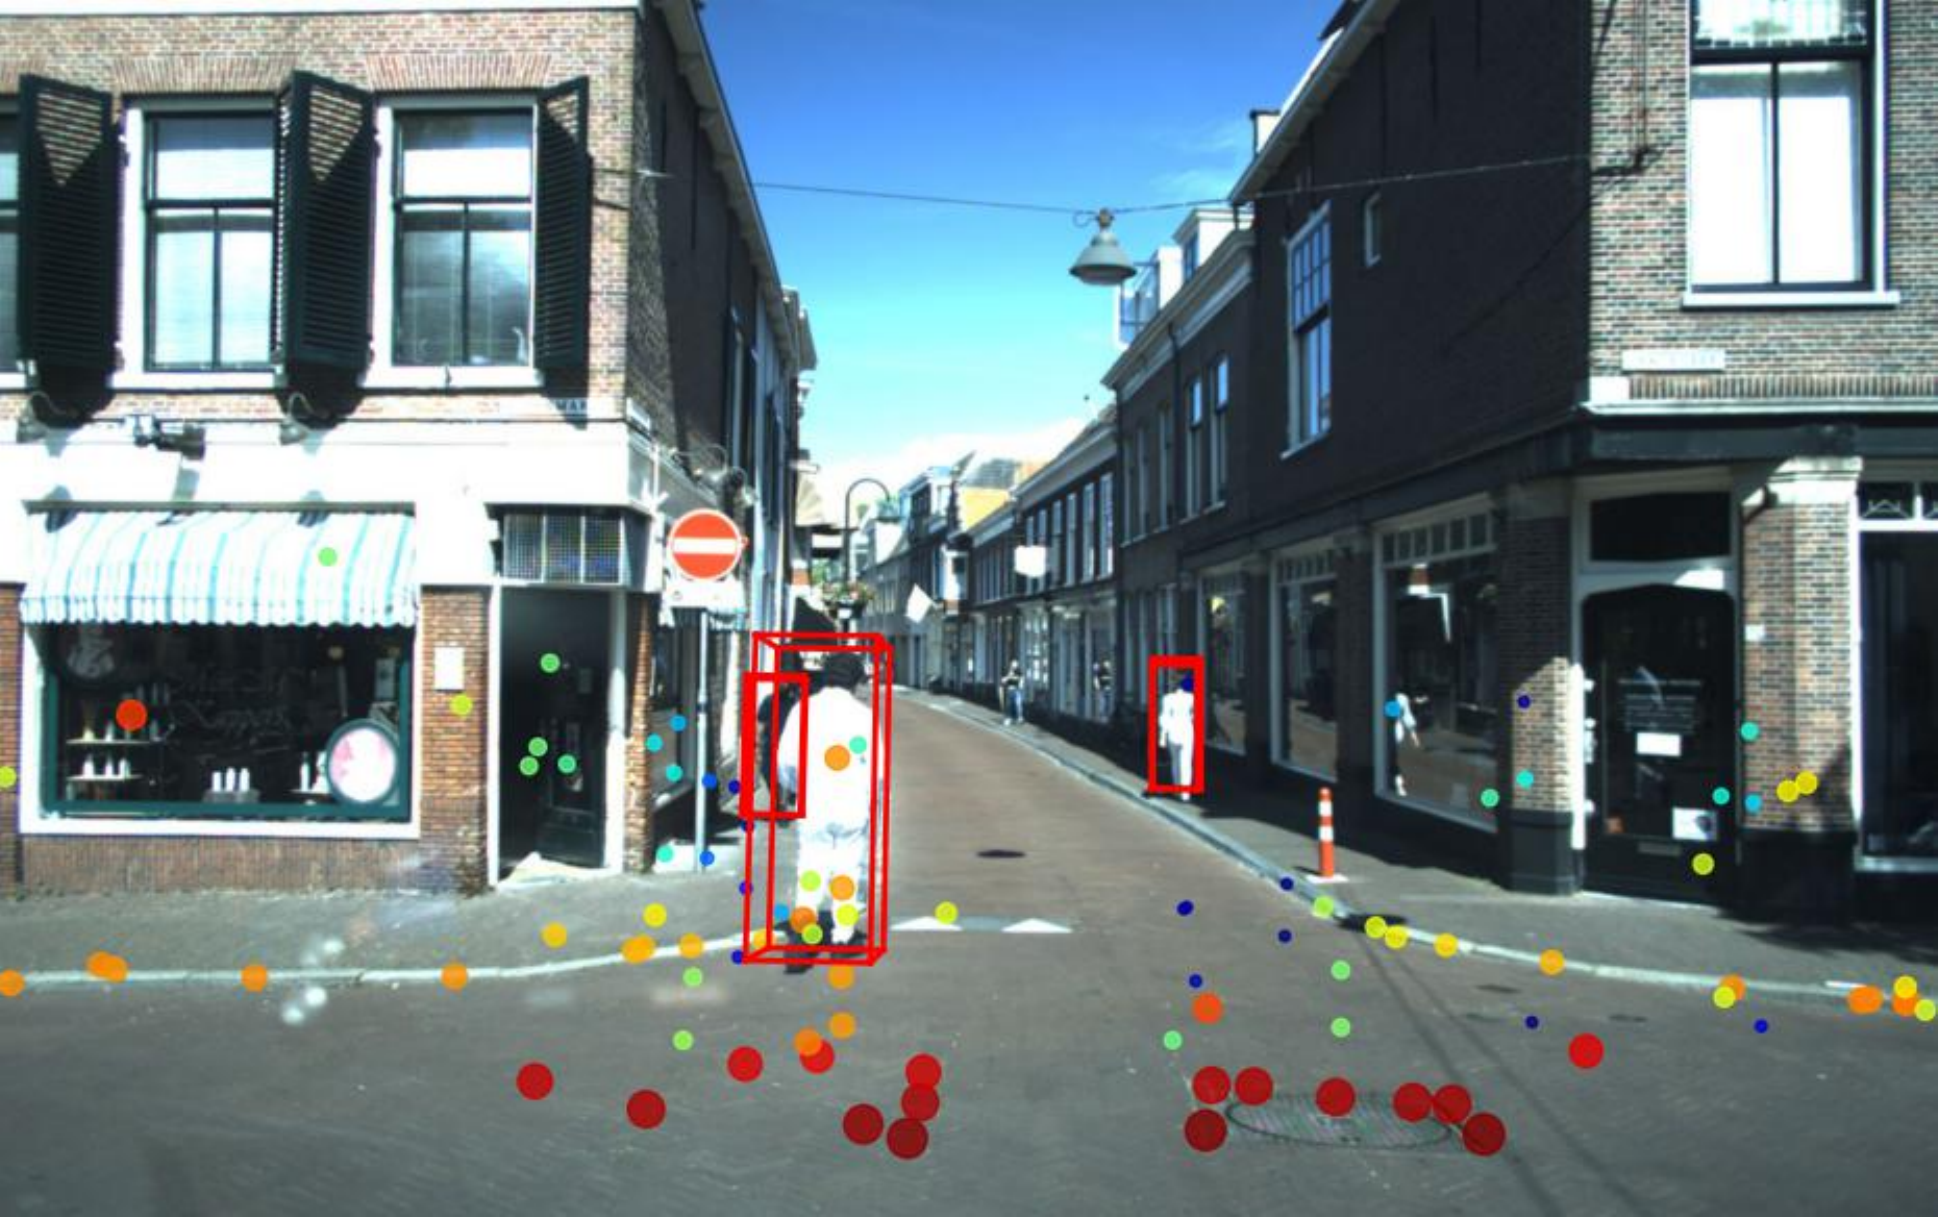}
        \end{subfigure}%
    \end{minipage}\\
    \begin{minipage}[t!]{.22\textwidth}
        \centering
        \begin{subfigure}{.5\textwidth}
            \caption{Ours}
        \end{subfigure}%
        \begin{subfigure}{\textwidth}
            \centering
            \includegraphics[width=\textwidth]{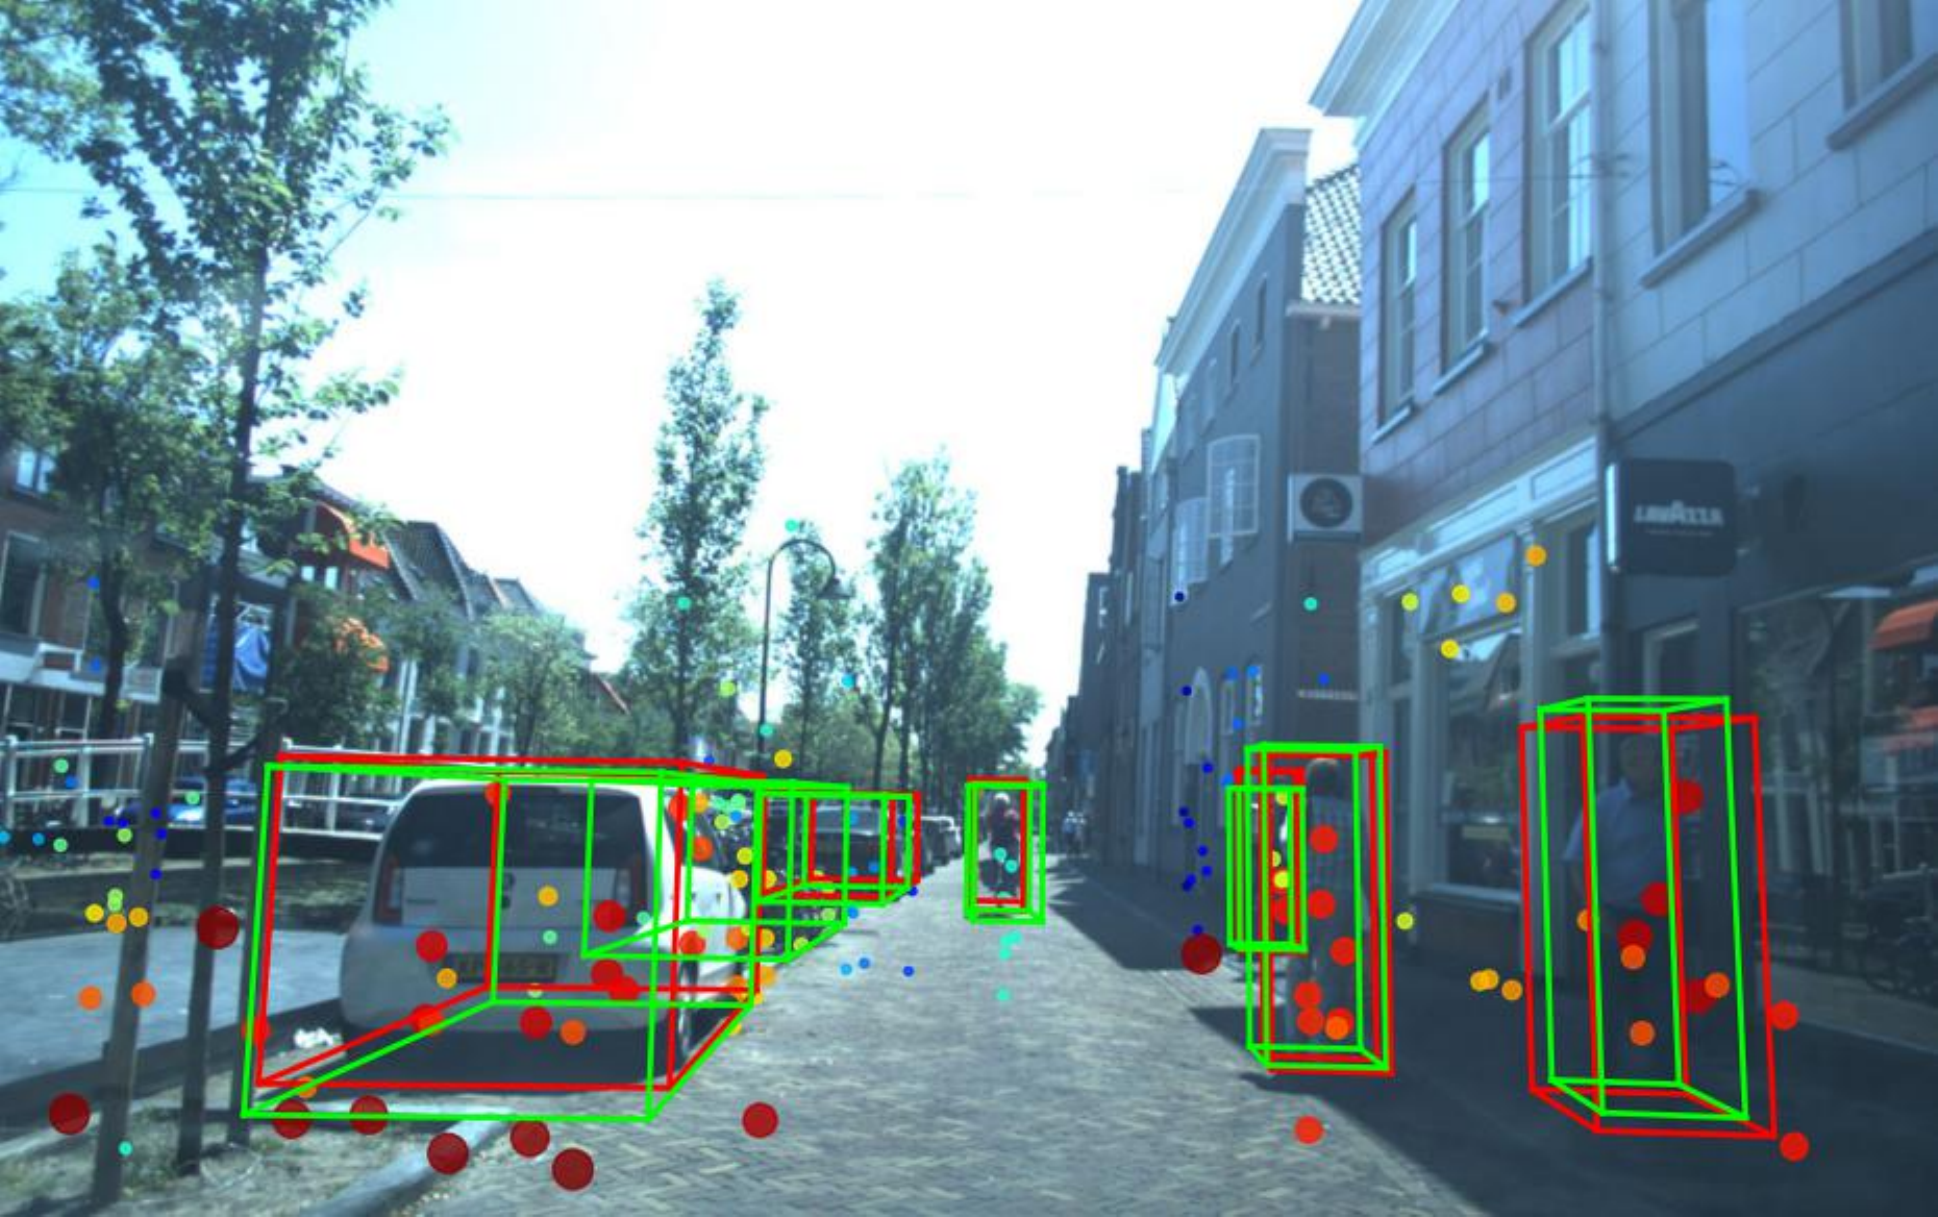}
        \end{subfigure}%
        \begin{subfigure}{\textwidth}
            \centering
            \includegraphics[width=\textwidth]{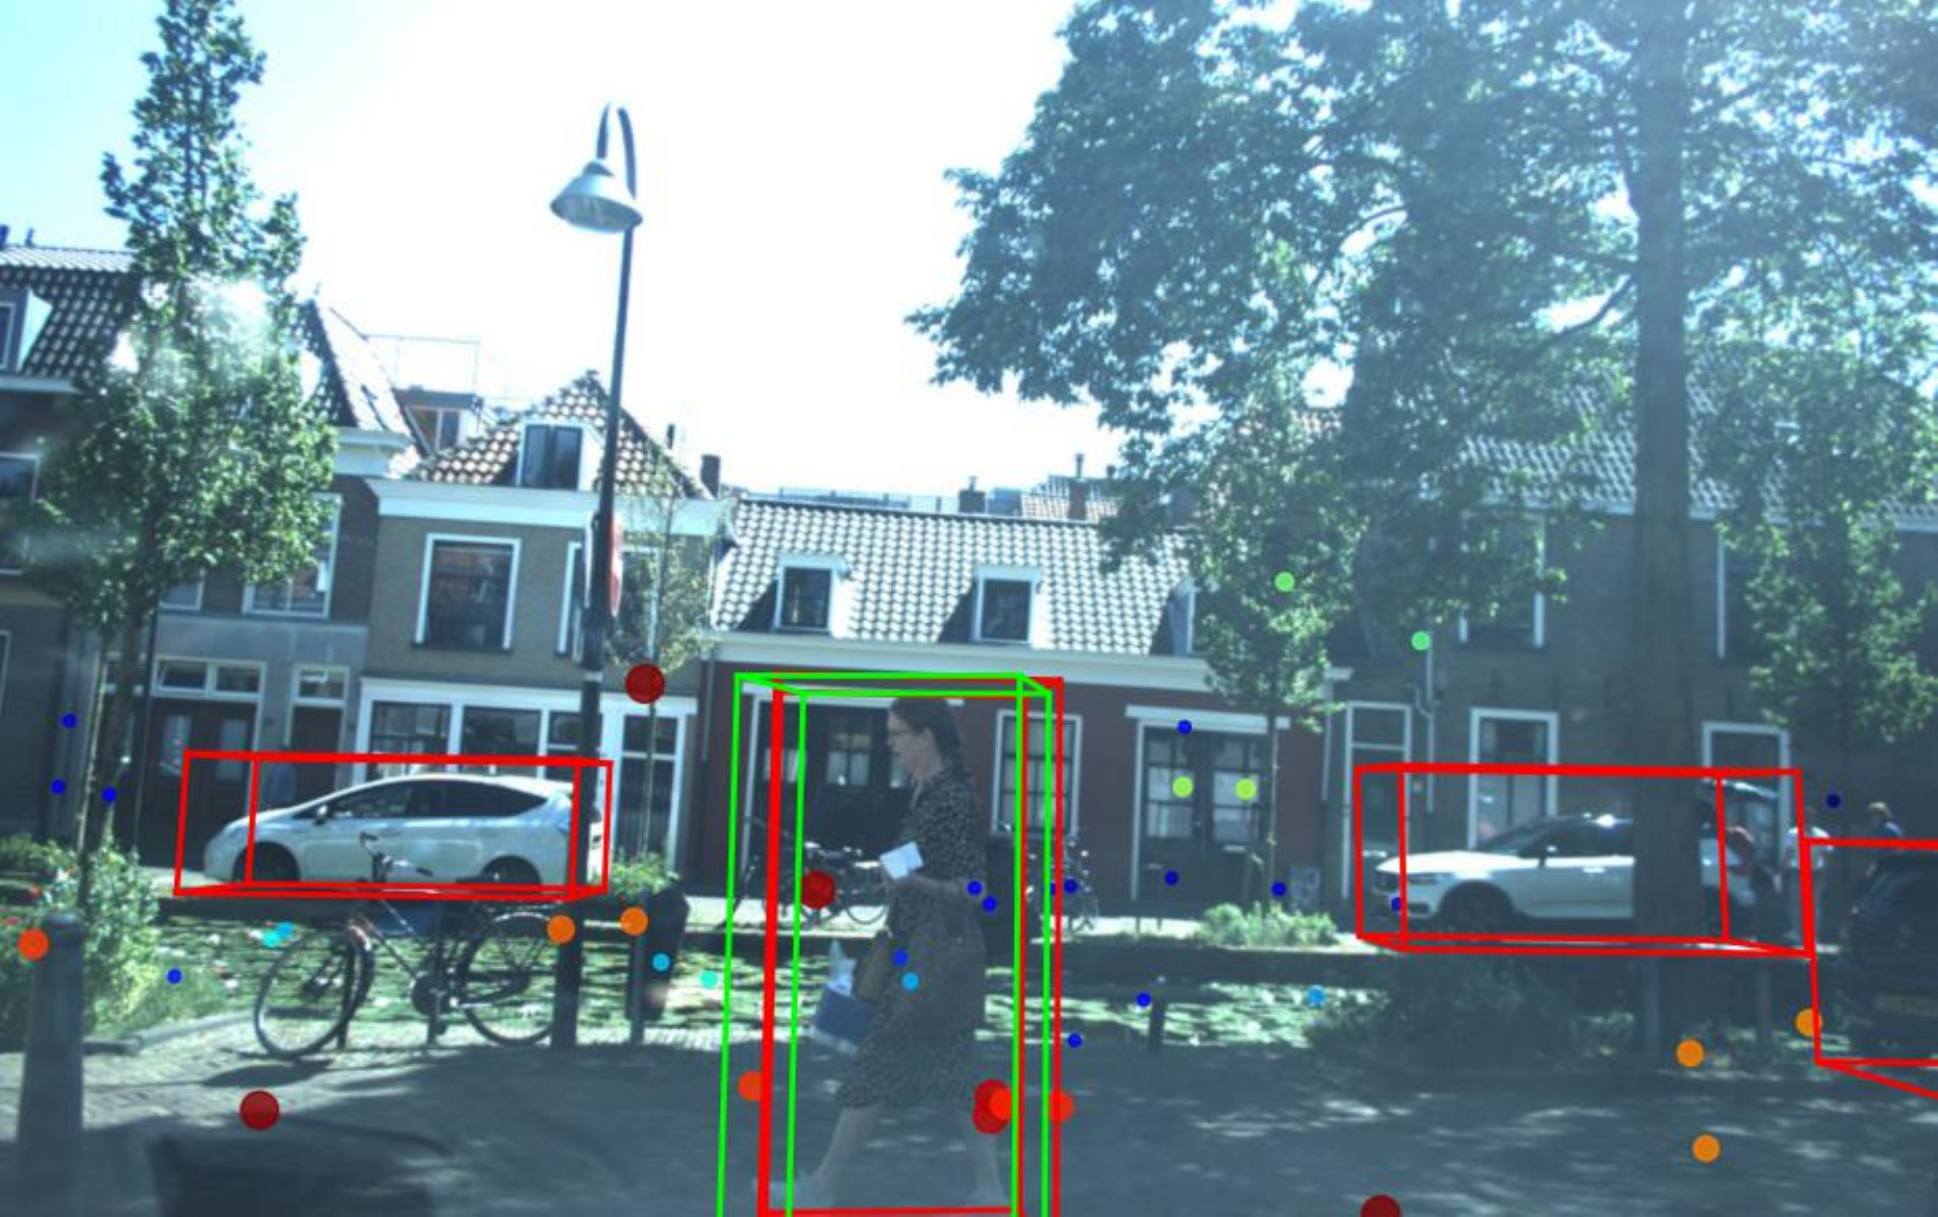}
        \end{subfigure}%
        \begin{subfigure}{\textwidth}
            \centering
            \includegraphics[width=\textwidth]{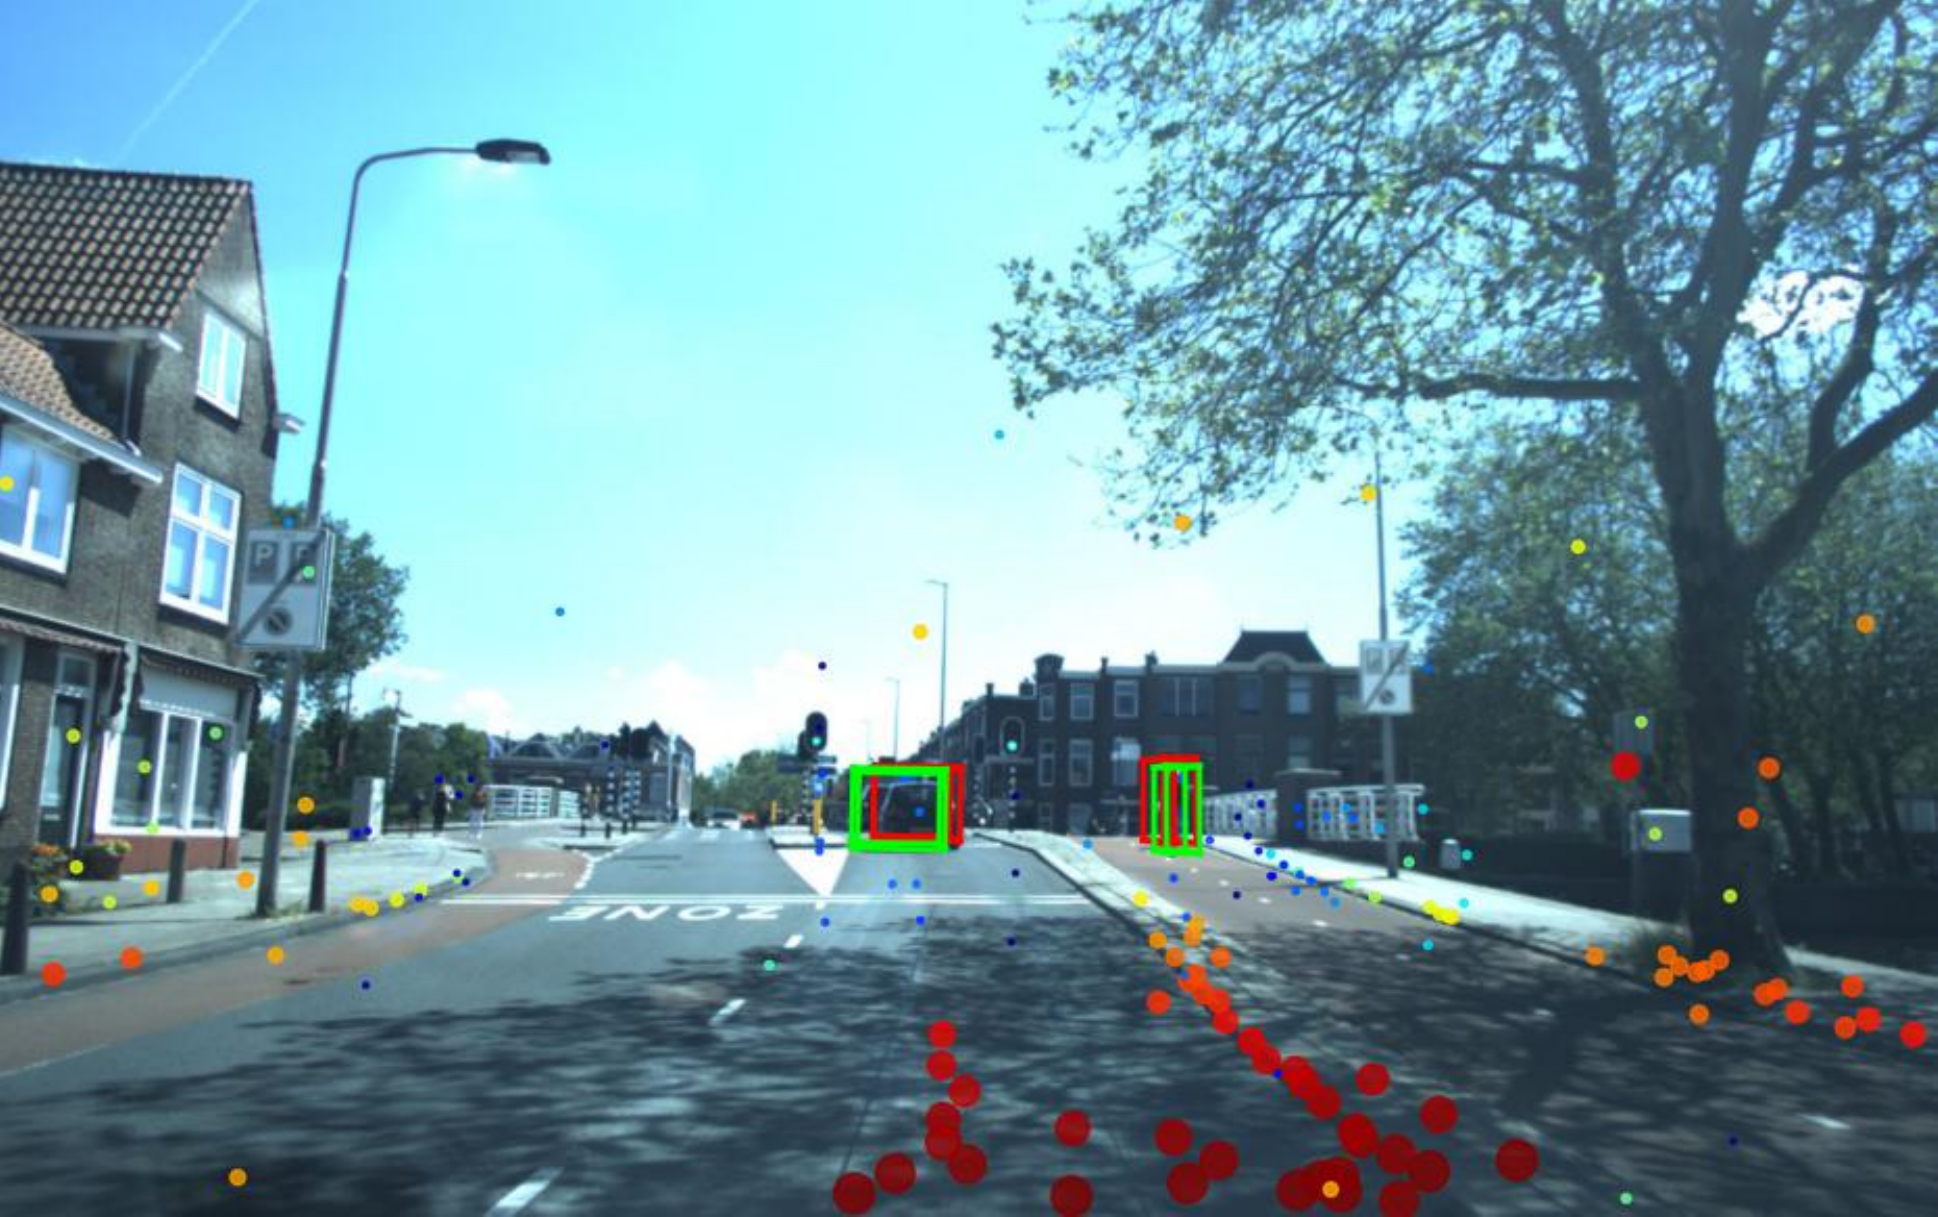}
        \end{subfigure}%
        \begin{subfigure}{\textwidth}
            \centering
            \includegraphics[width=\textwidth]{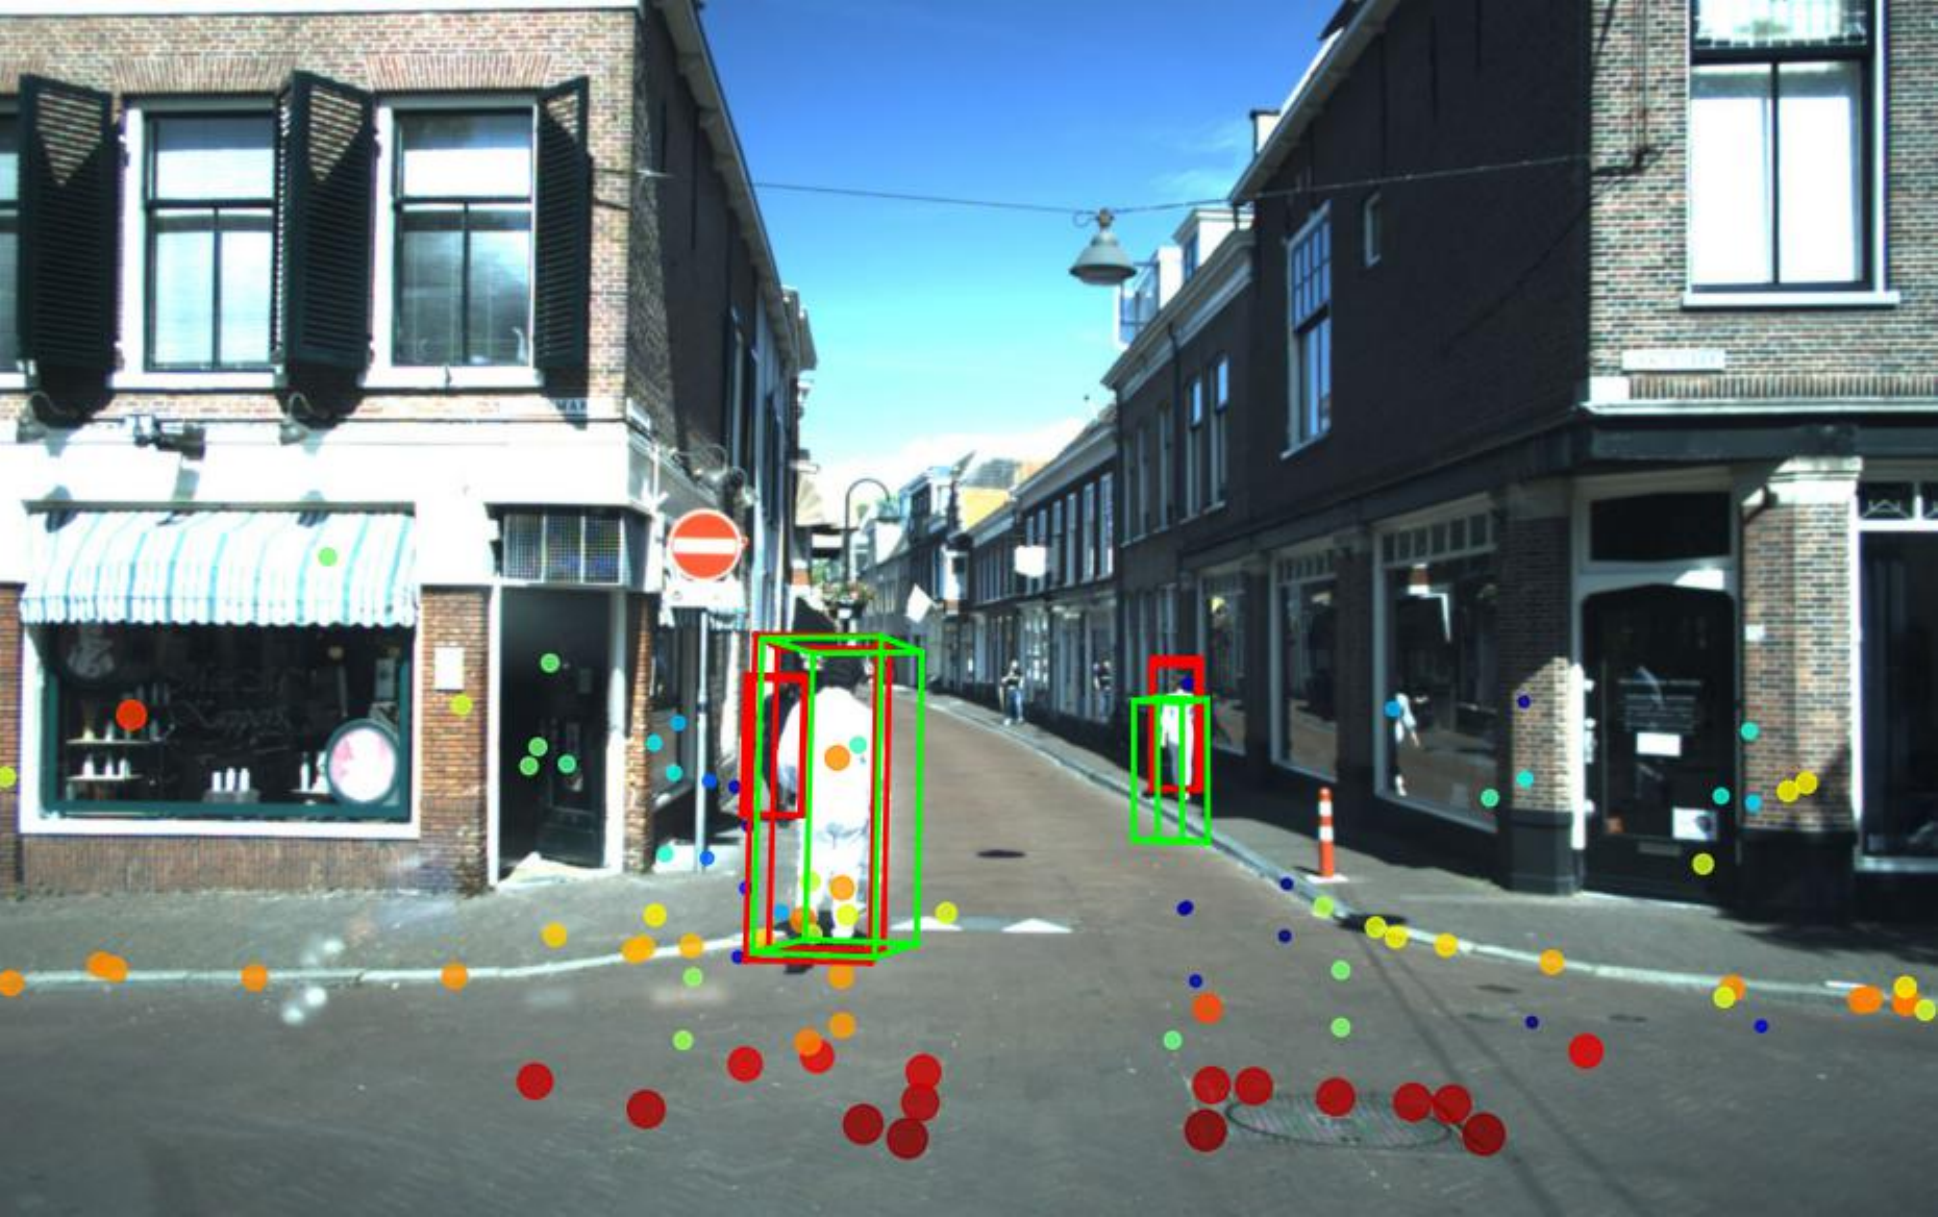}
        \end{subfigure}%
    \end{minipage}\\
    \begin{minipage}[t!]{.22\textwidth}
        \centering
        \begin{subfigure}{.5\textwidth}
            \caption{pointpillar}
        \end{subfigure}%
        \begin{subfigure}{\textwidth}
            \centering
            \includegraphics[width=\textwidth]{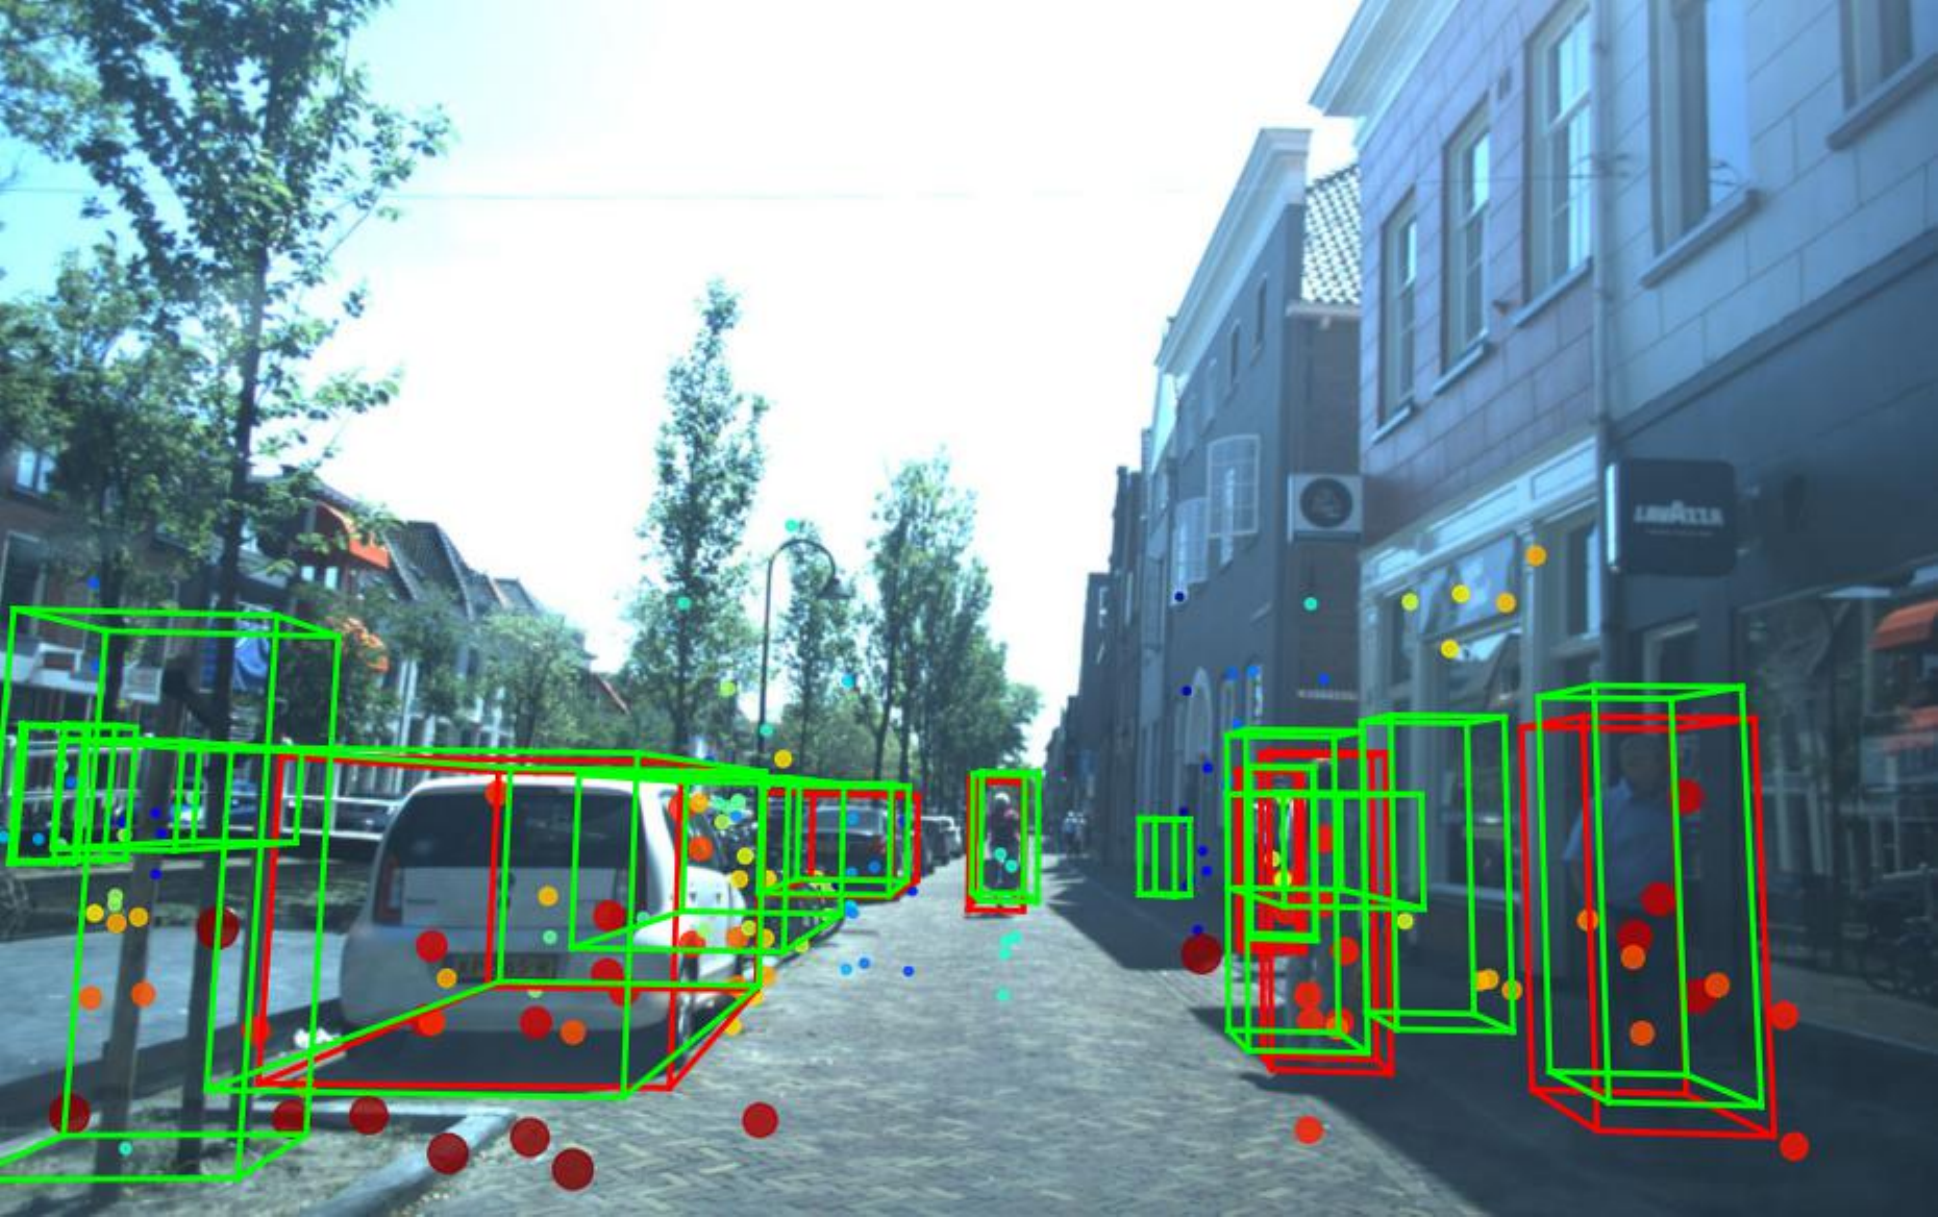}
        \end{subfigure}%
        \begin{subfigure}{\textwidth}
            \centering
            \includegraphics[width=\textwidth]{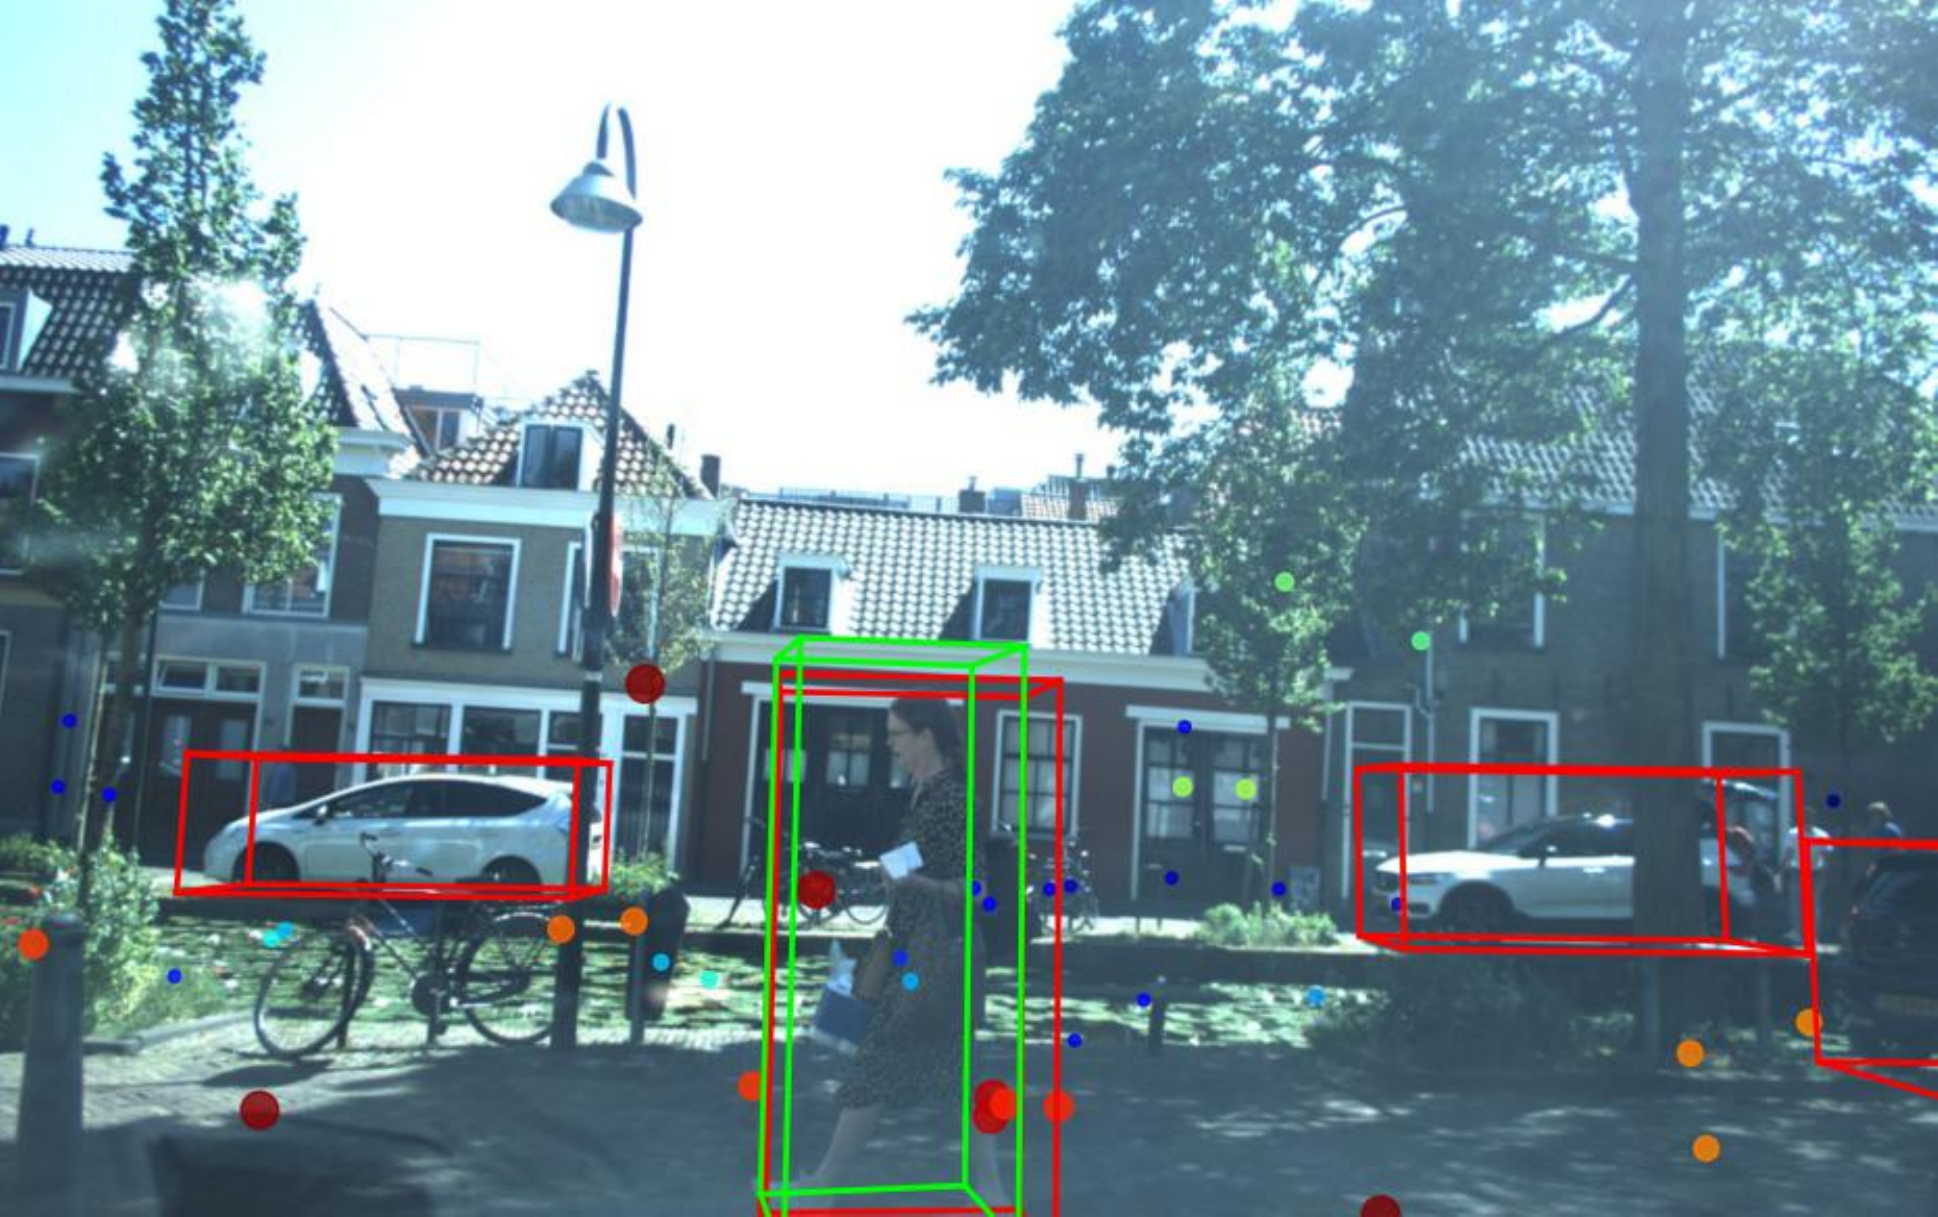}
        \end{subfigure}%
        \begin{subfigure}{\textwidth}
            \centering
            \includegraphics[width=\textwidth]{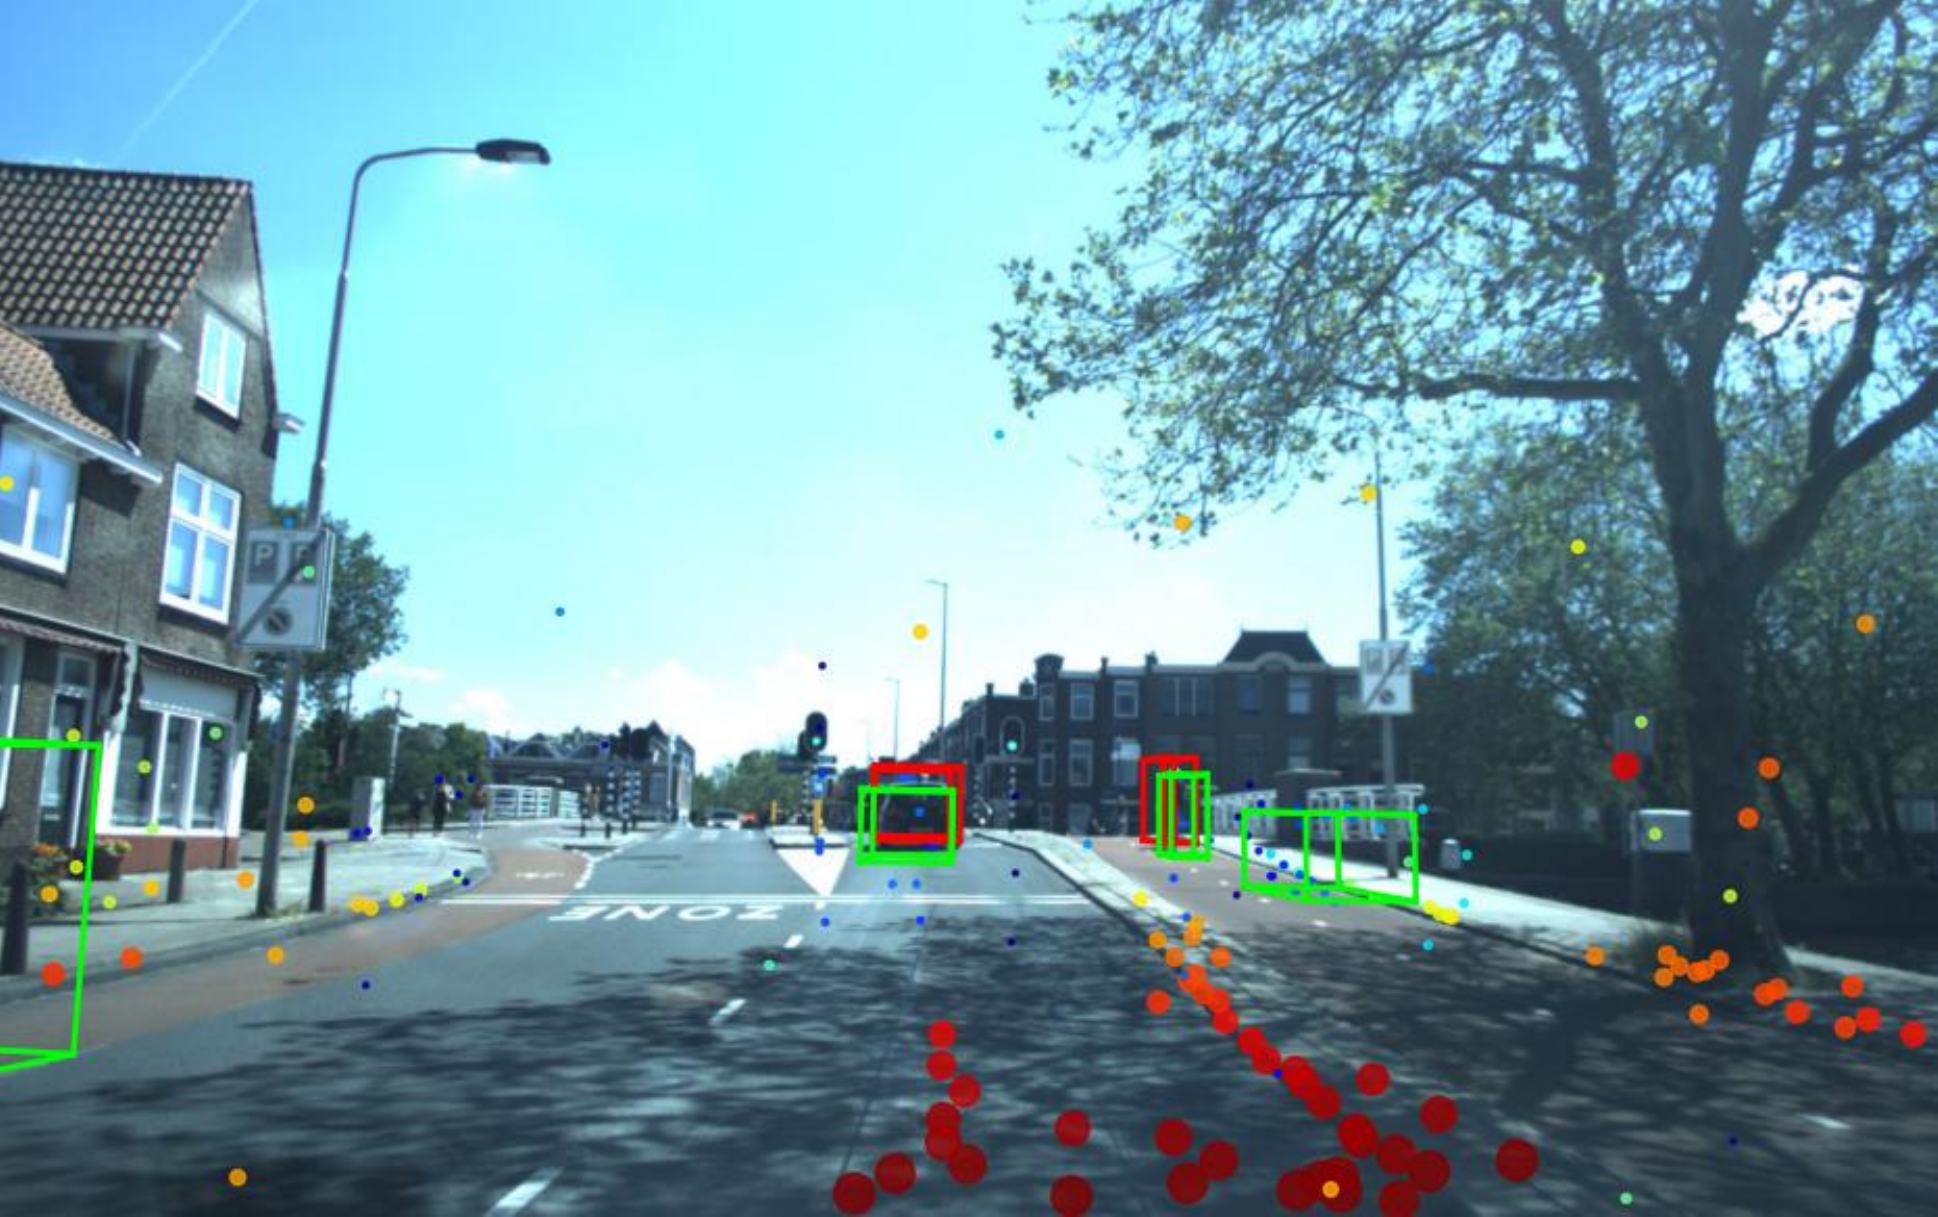}
        \end{subfigure}%
        \begin{subfigure}{\textwidth}
            \centering
            \includegraphics[width=\textwidth]{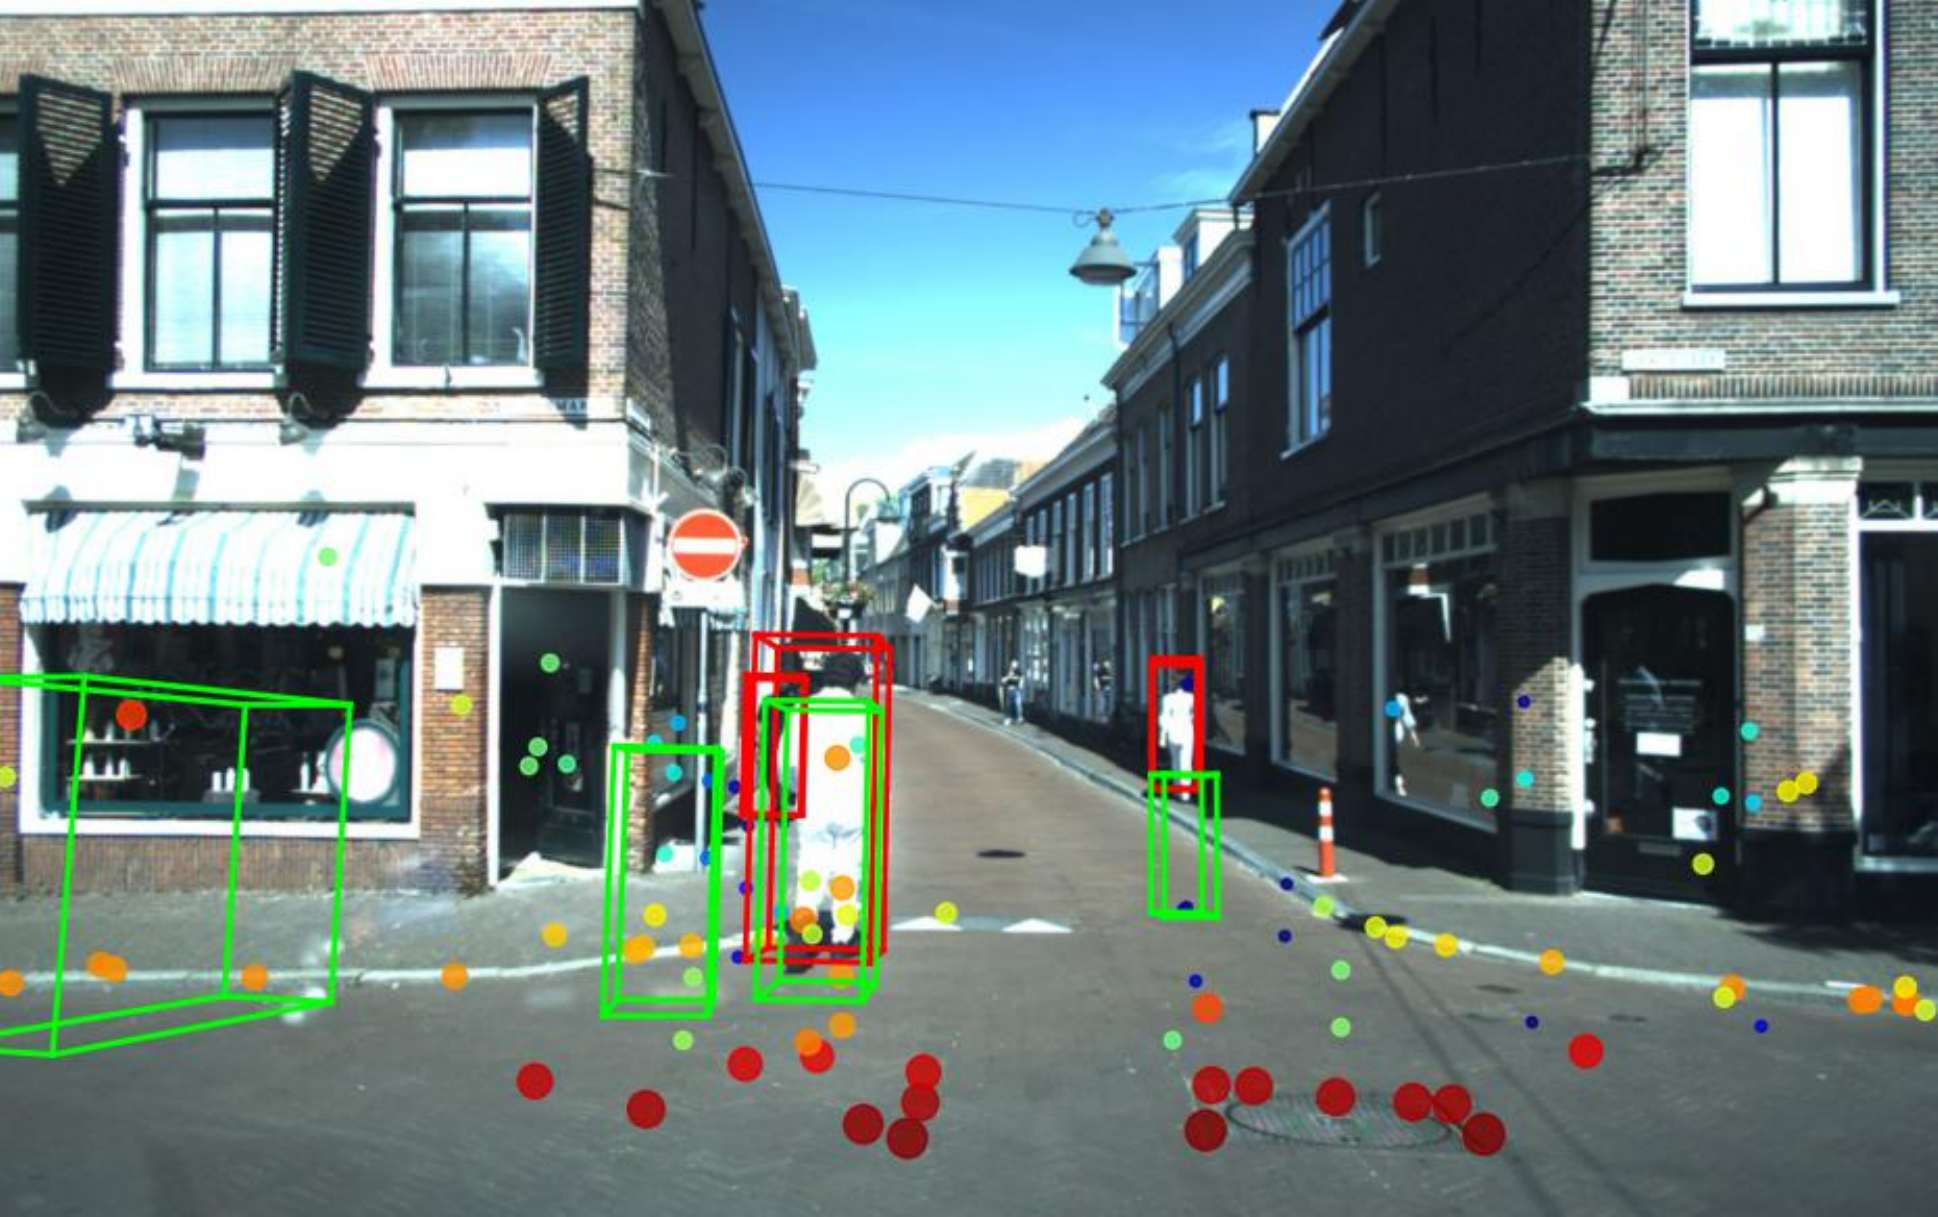}
        \end{subfigure}%
    \end{minipage}\\
    \begin{minipage}[t!]{.22\textwidth}
        \centering
        \begin{subfigure}{.5\textwidth}
            \caption{SECOND}
        \end{subfigure}%
        \begin{subfigure}{\textwidth}
            \centering
            \includegraphics[width=\textwidth]{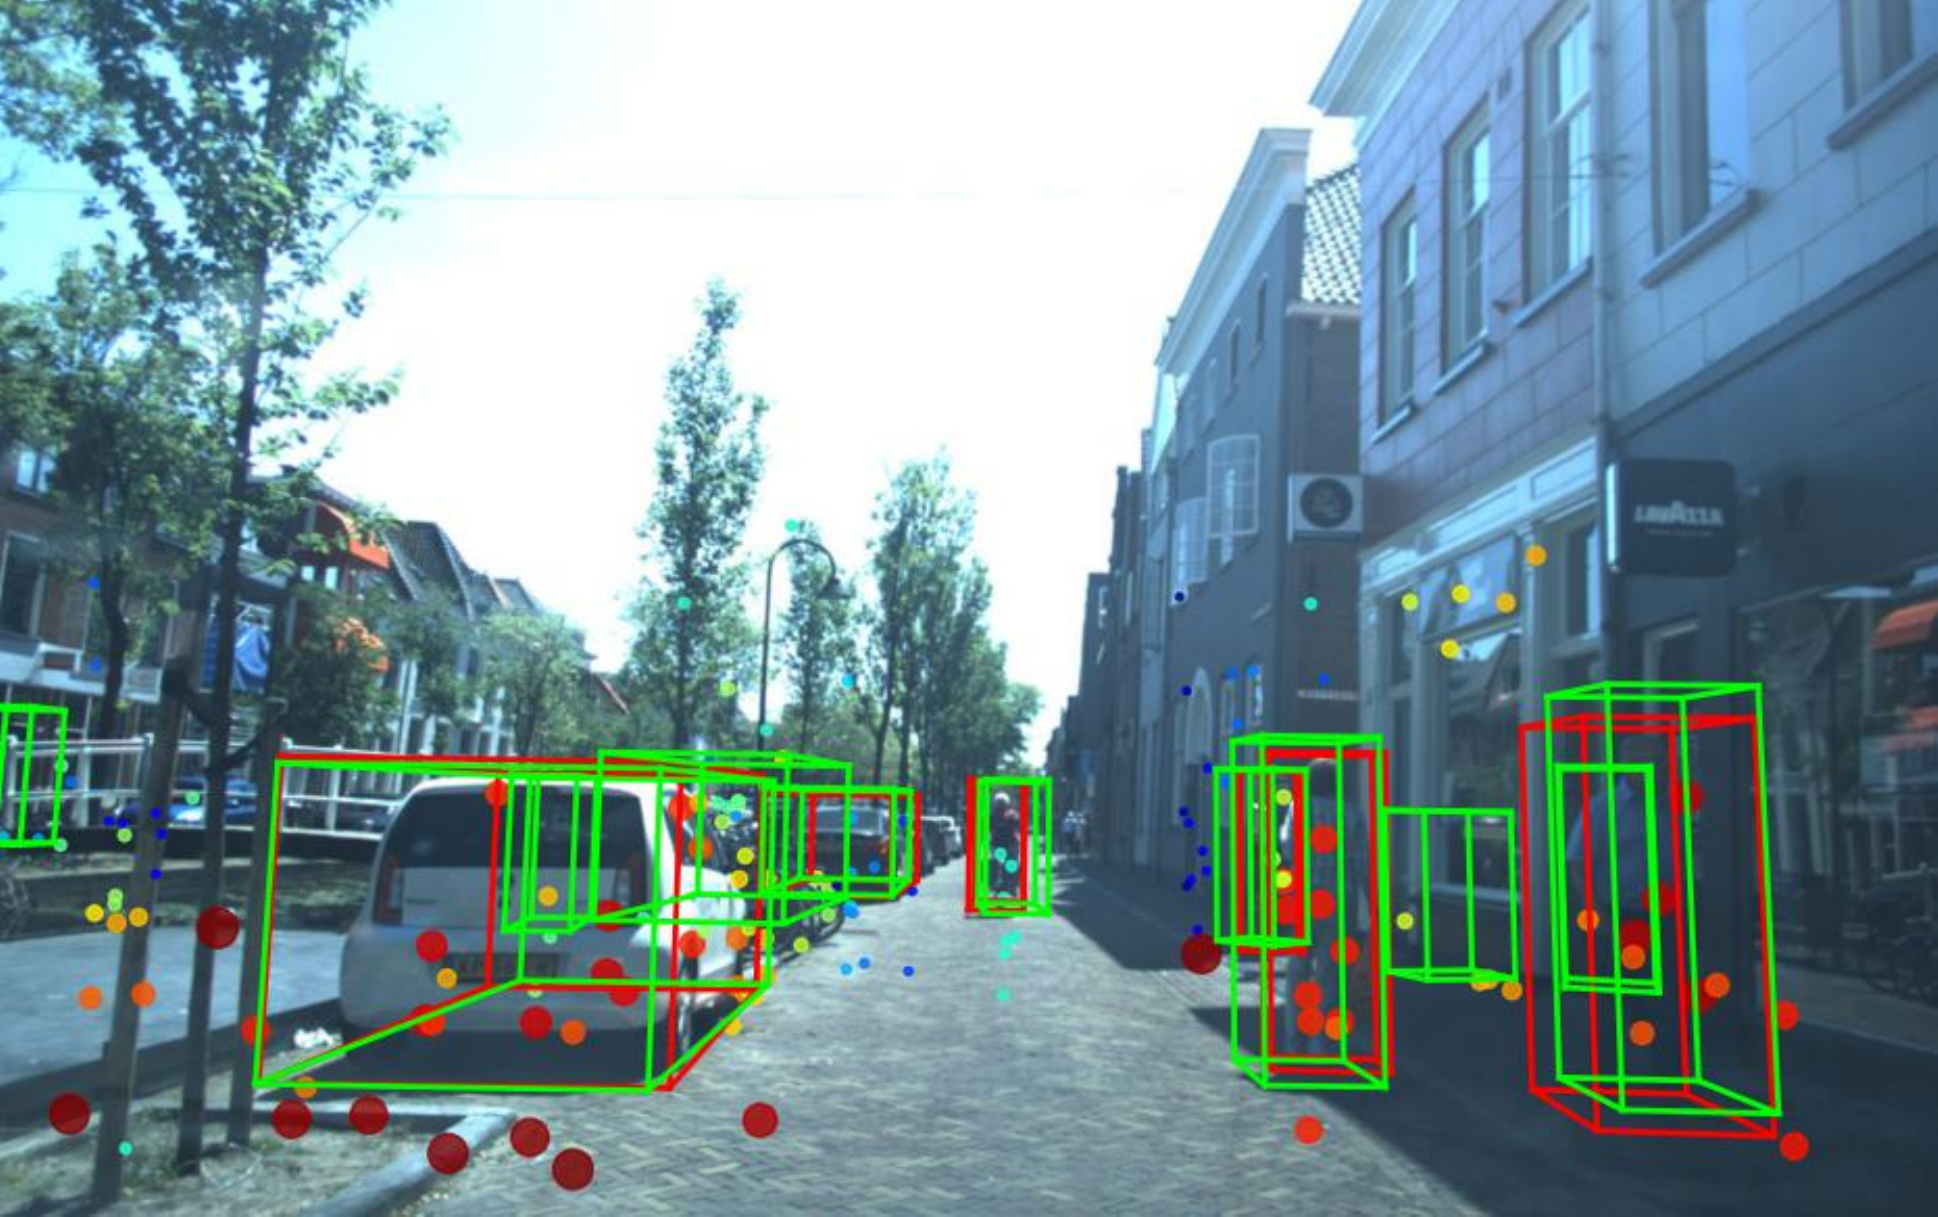}
        \end{subfigure}%
        \begin{subfigure}{\textwidth}
            \centering
            \includegraphics[width=\textwidth]{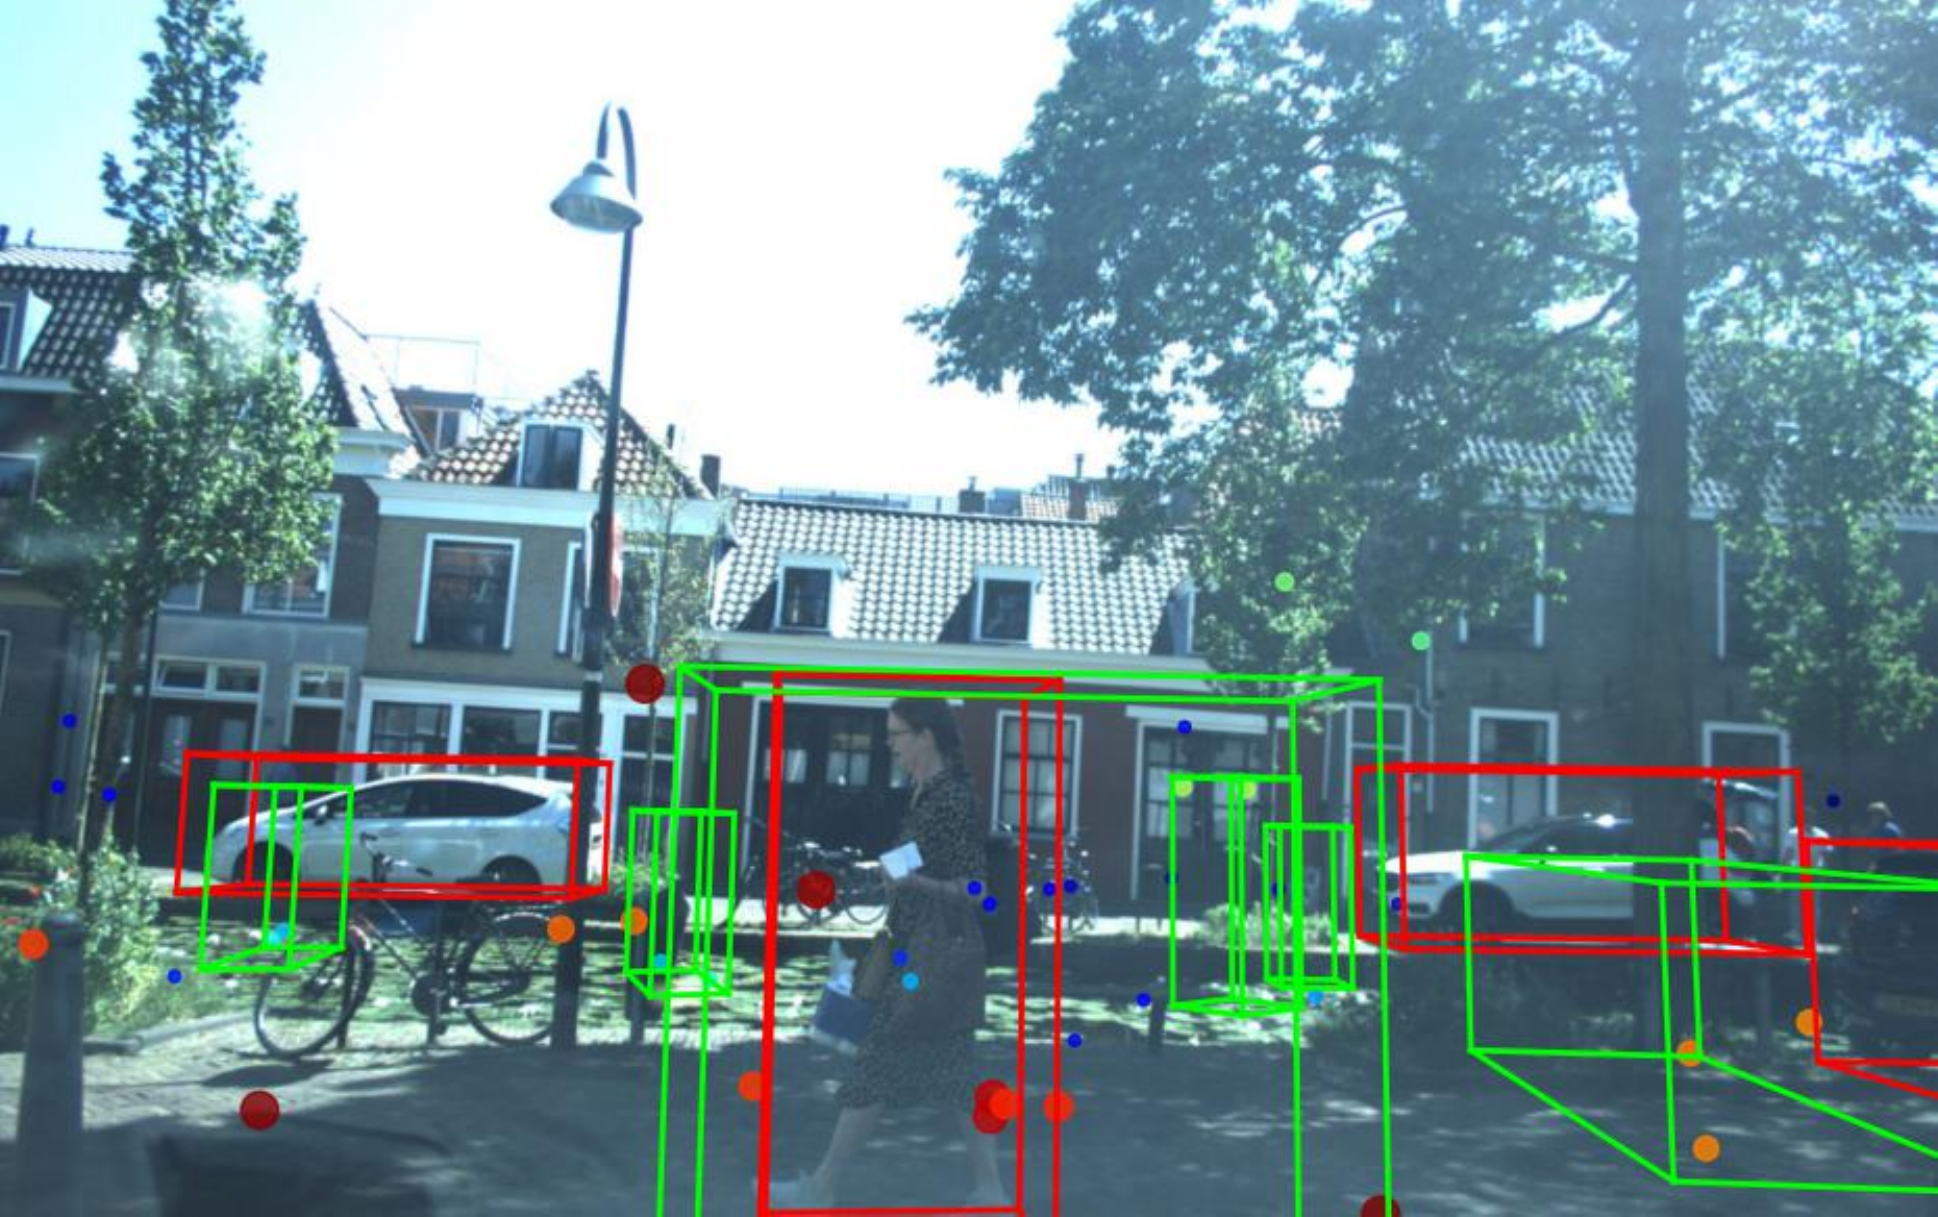}
        \end{subfigure}%
        \begin{subfigure}{\textwidth}
            \centering
            \includegraphics[width=\textwidth]{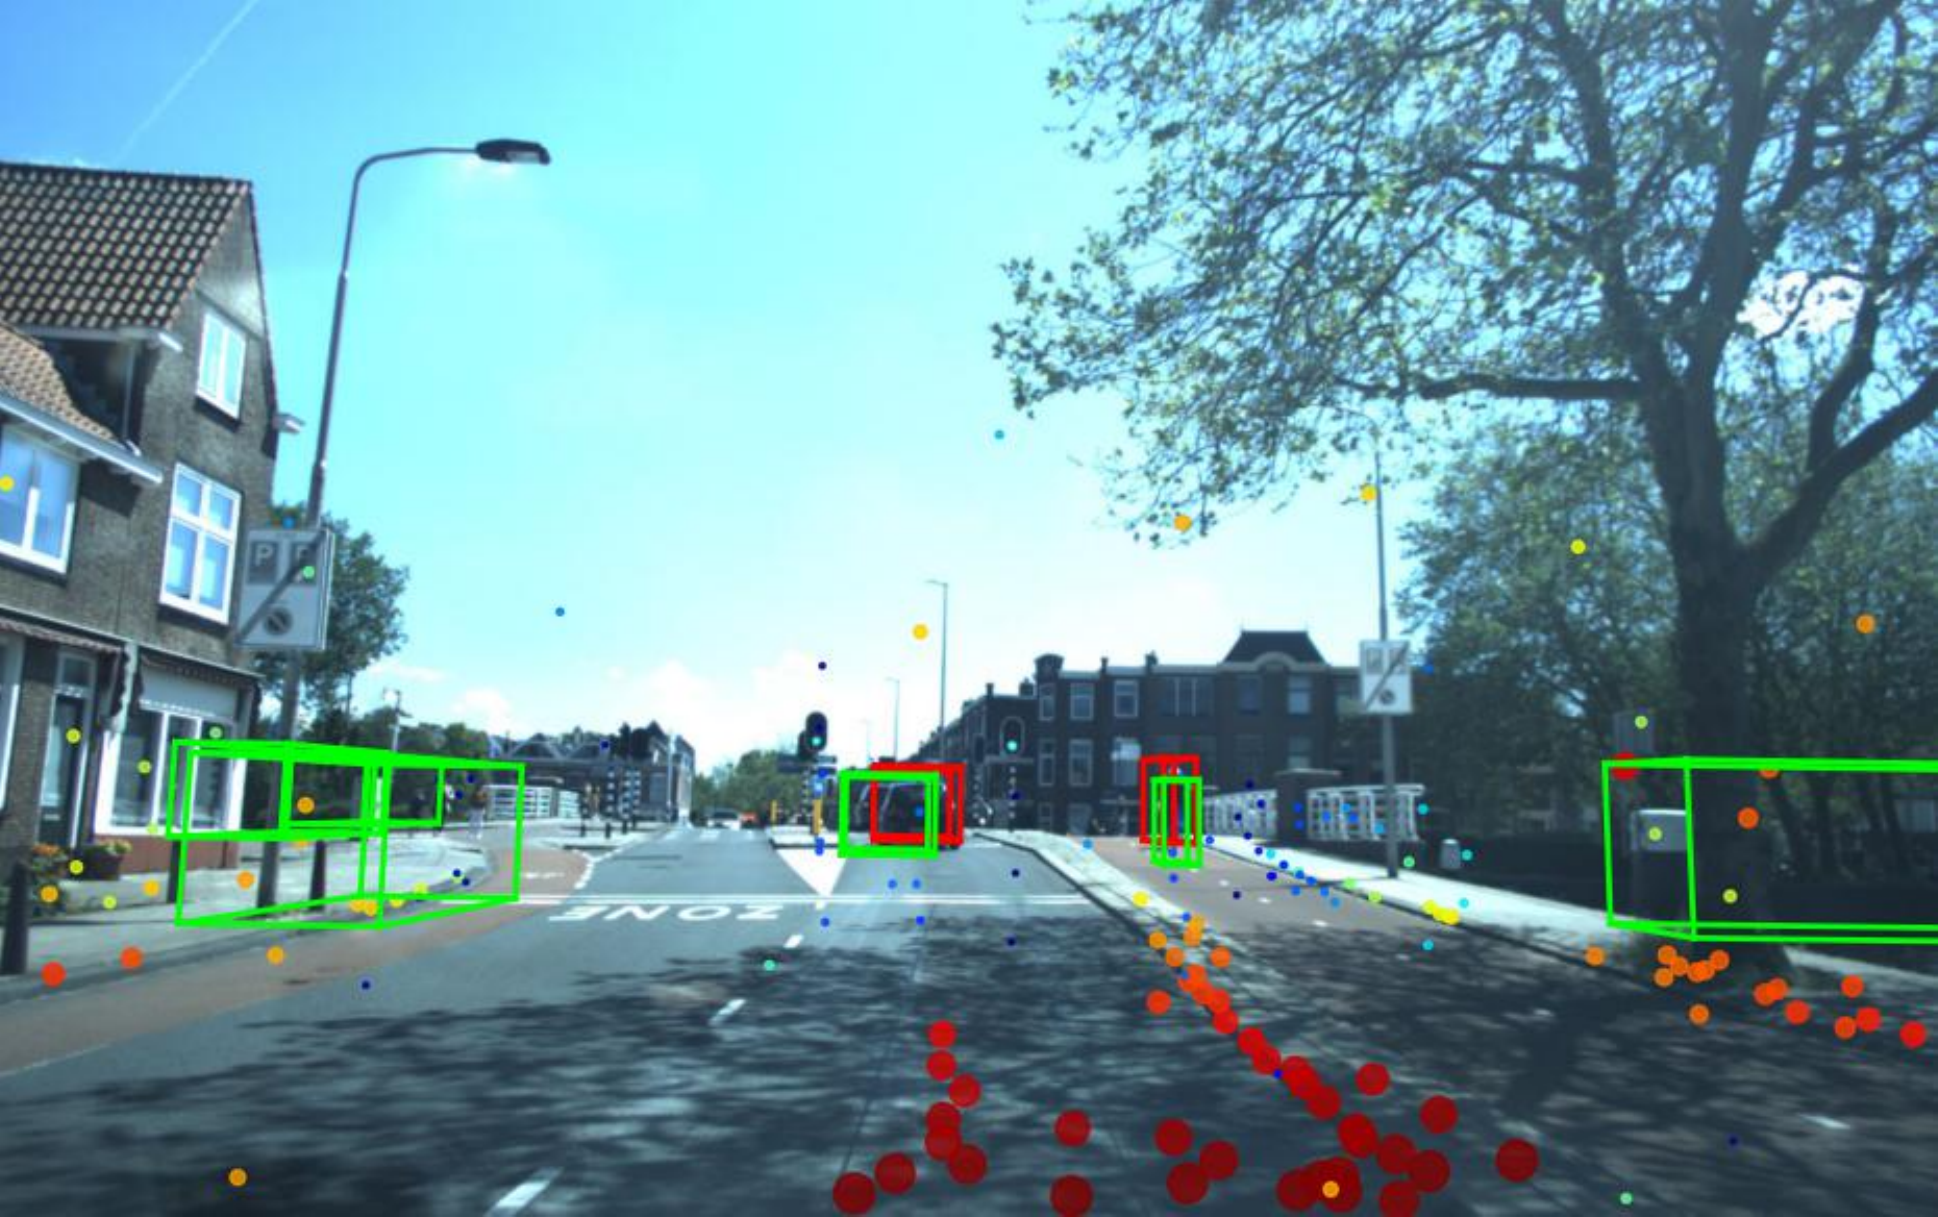}
        \end{subfigure}%
        \begin{subfigure}{\textwidth}
            \centering
            \includegraphics[width=\textwidth]{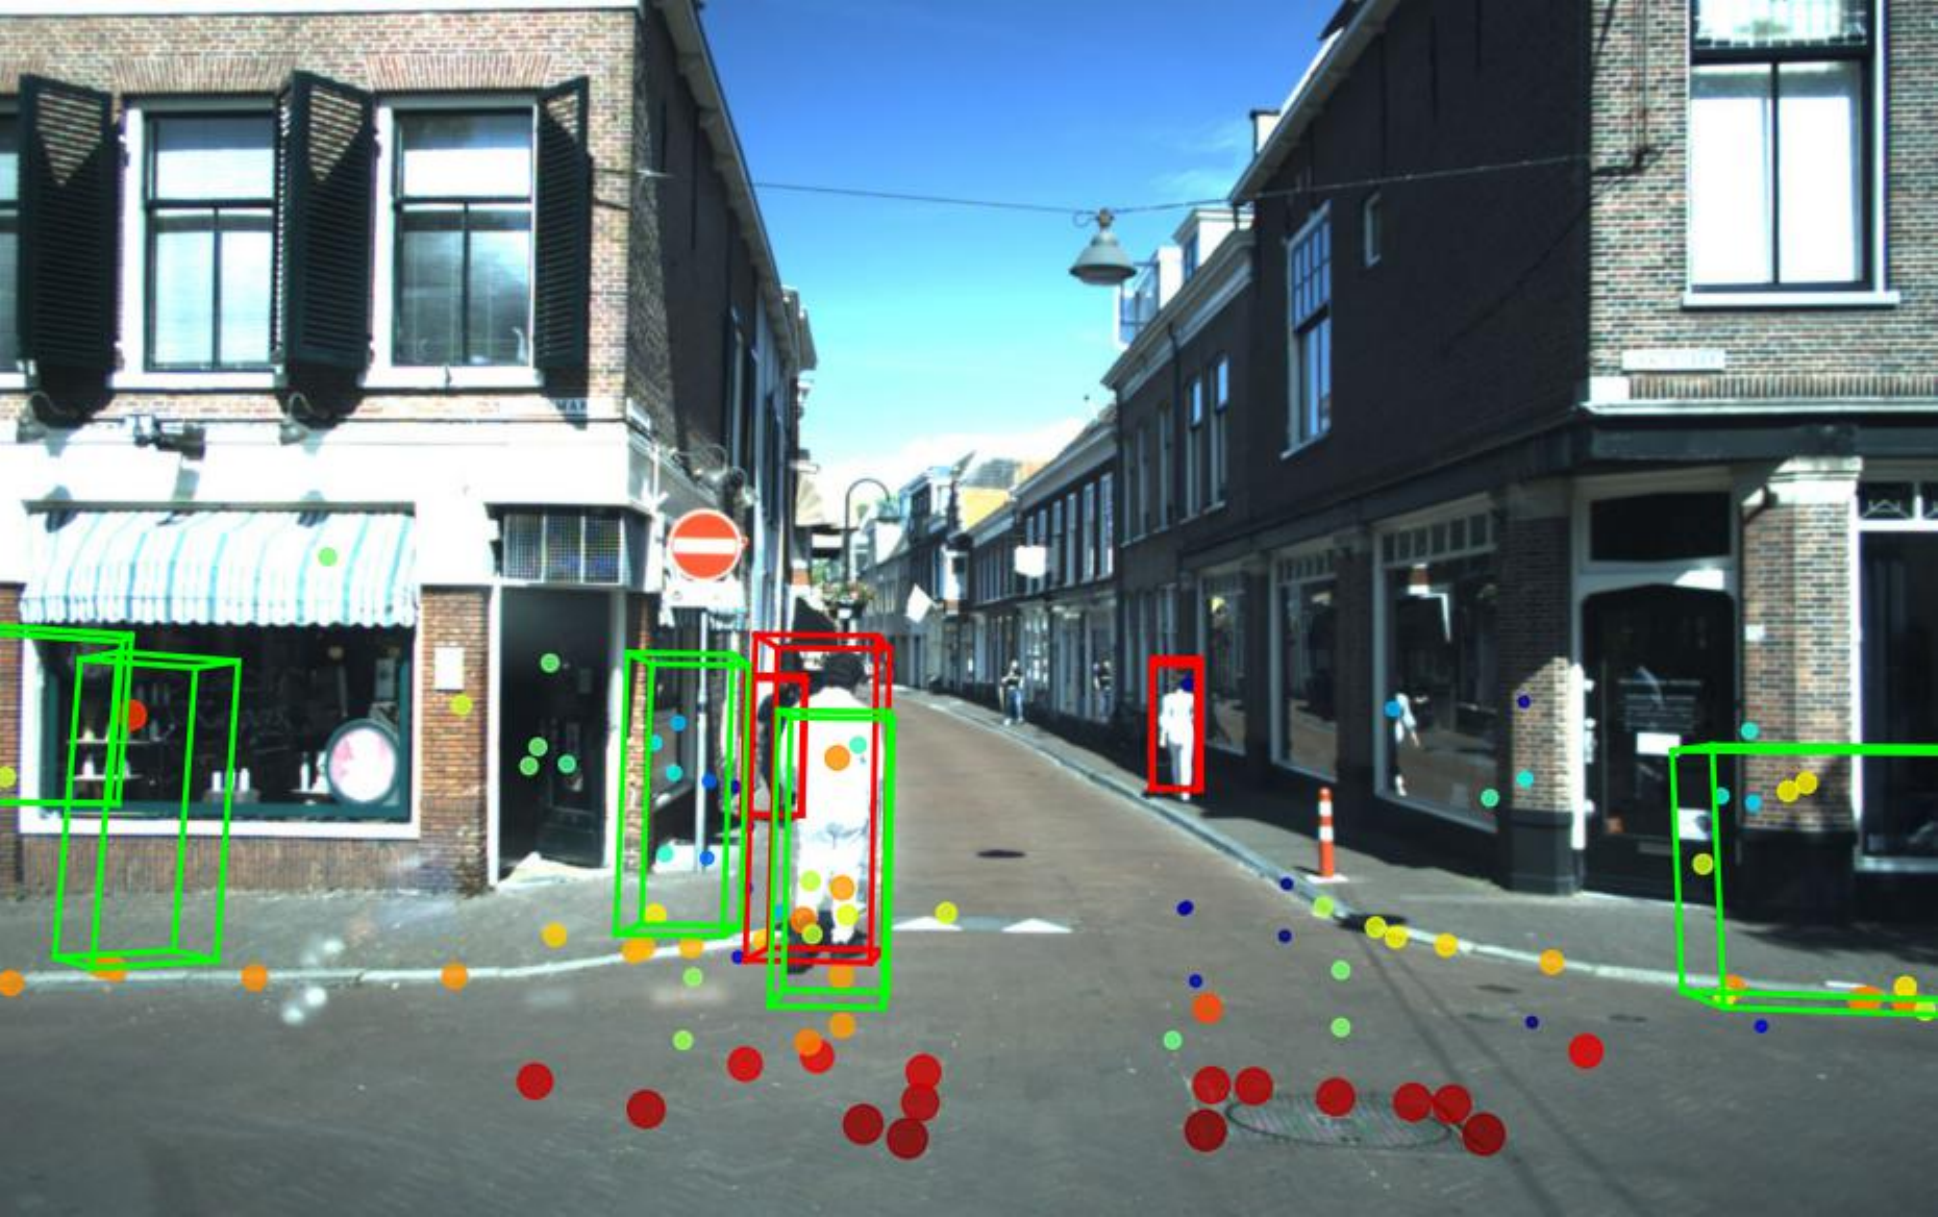}
        \end{subfigure}%
    \end{minipage}\\
    \begin{minipage}[t!]{.22\textwidth}
        \centering
        \begin{subfigure}{.5\textwidth}
            \caption{CenterPoint}
        \end{subfigure}%
        \begin{subfigure}{\textwidth}
            \centering
            \includegraphics[width=\textwidth]{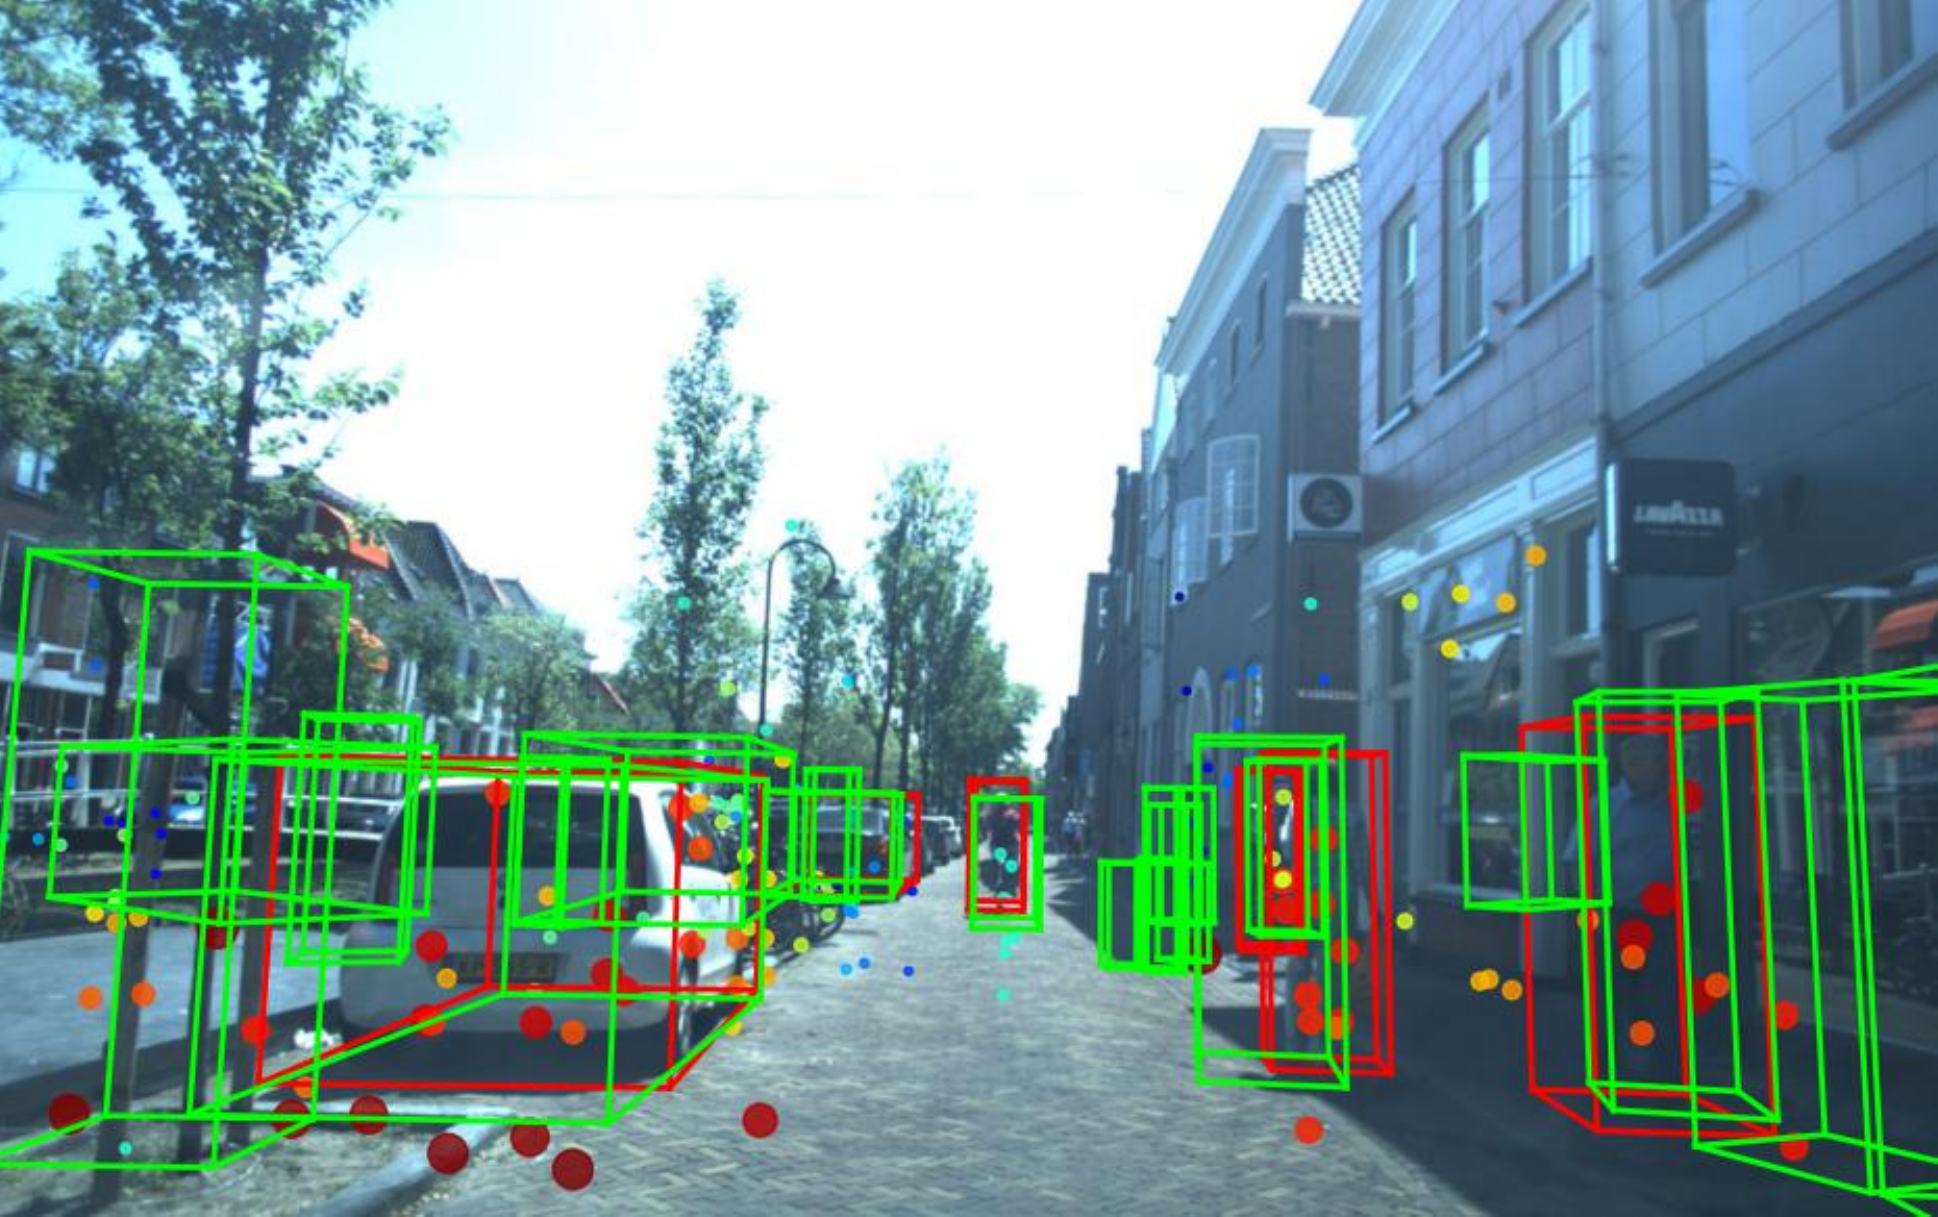}
        \end{subfigure}%
        \begin{subfigure}{\textwidth}
            \centering
            \includegraphics[width=\textwidth]{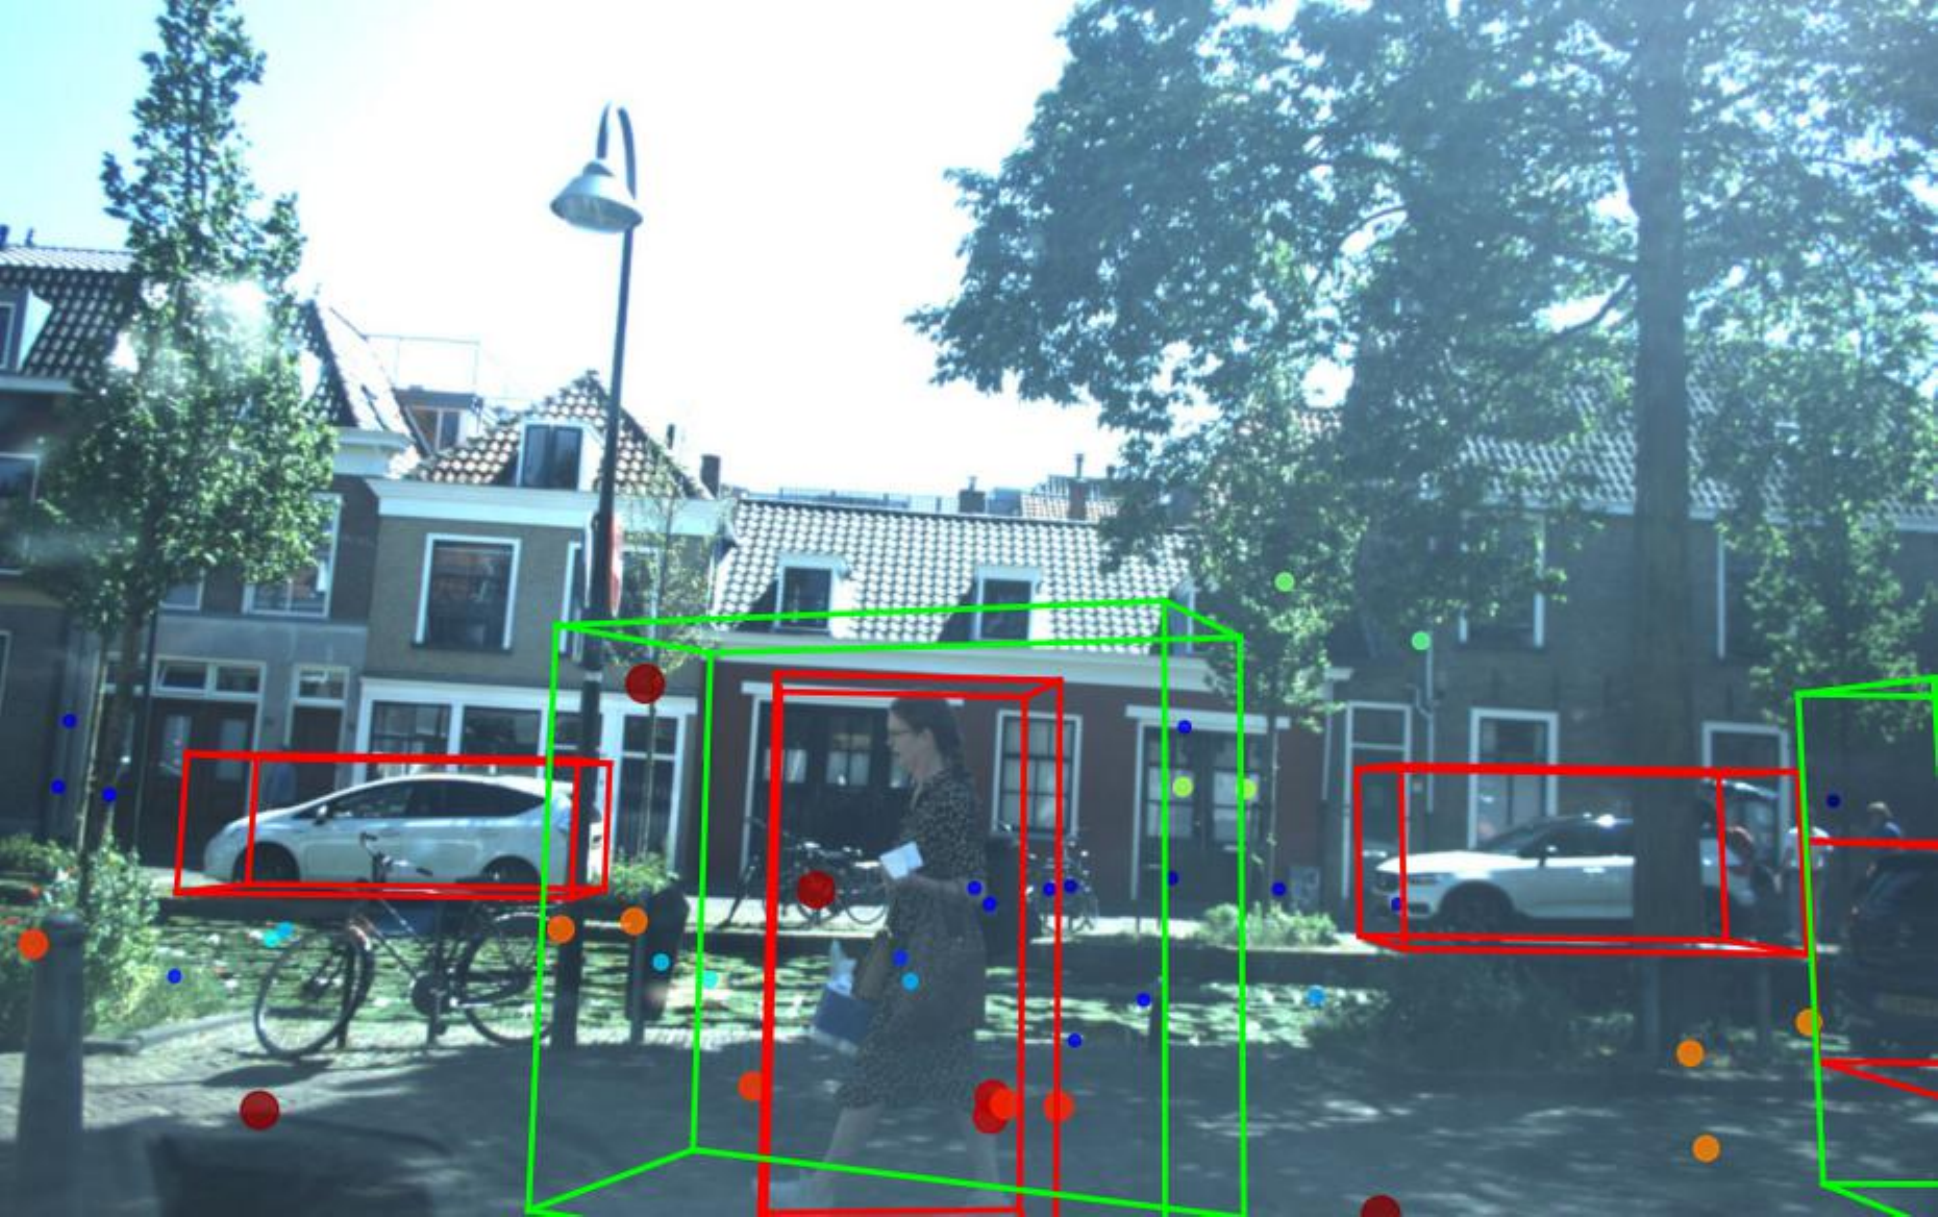}
        \end{subfigure}%
        \begin{subfigure}{\textwidth}
            \centering
            \includegraphics[width=\textwidth]{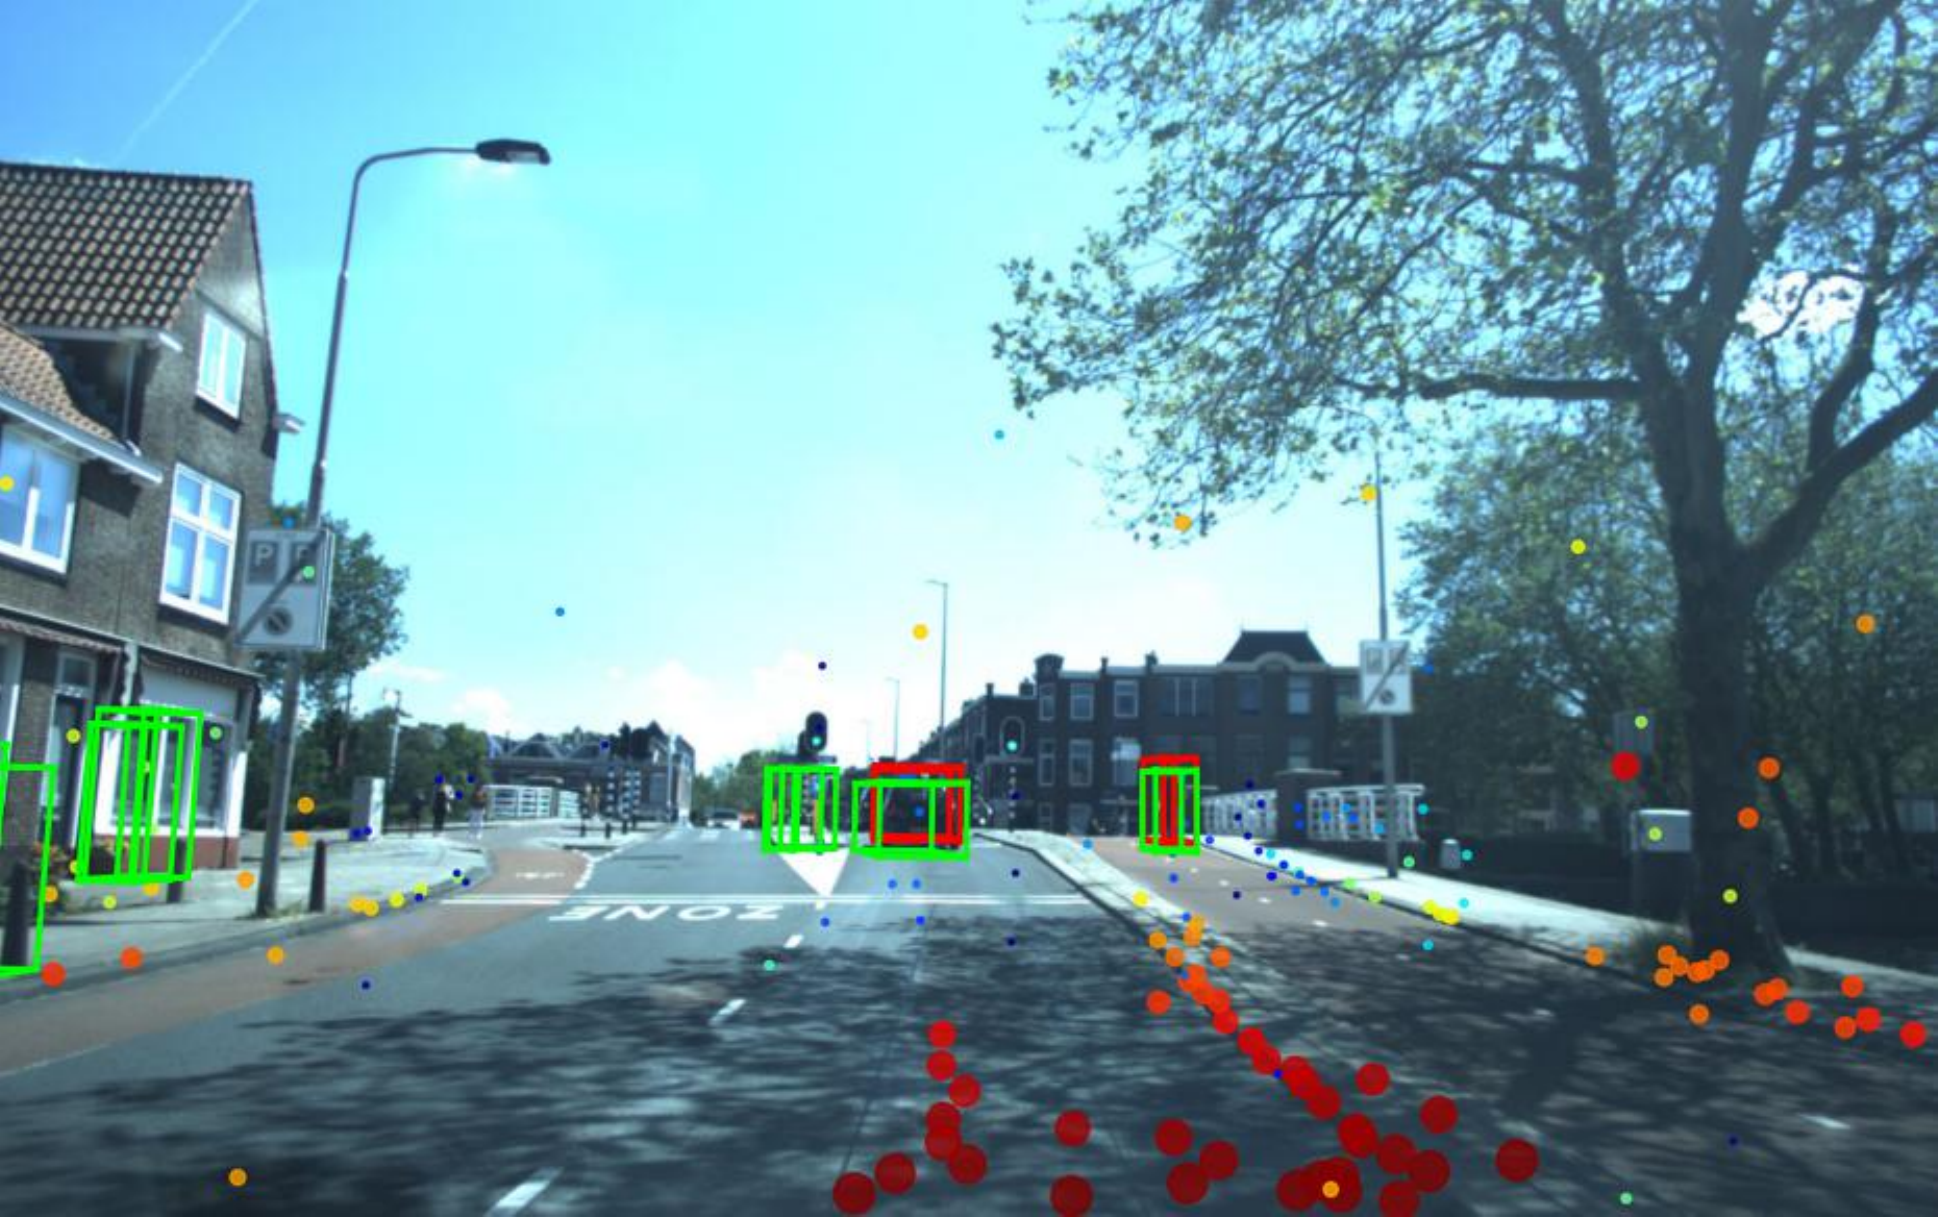}
        \end{subfigure}%
        \begin{subfigure}{\textwidth}
            \centering
            \includegraphics[width=\textwidth]{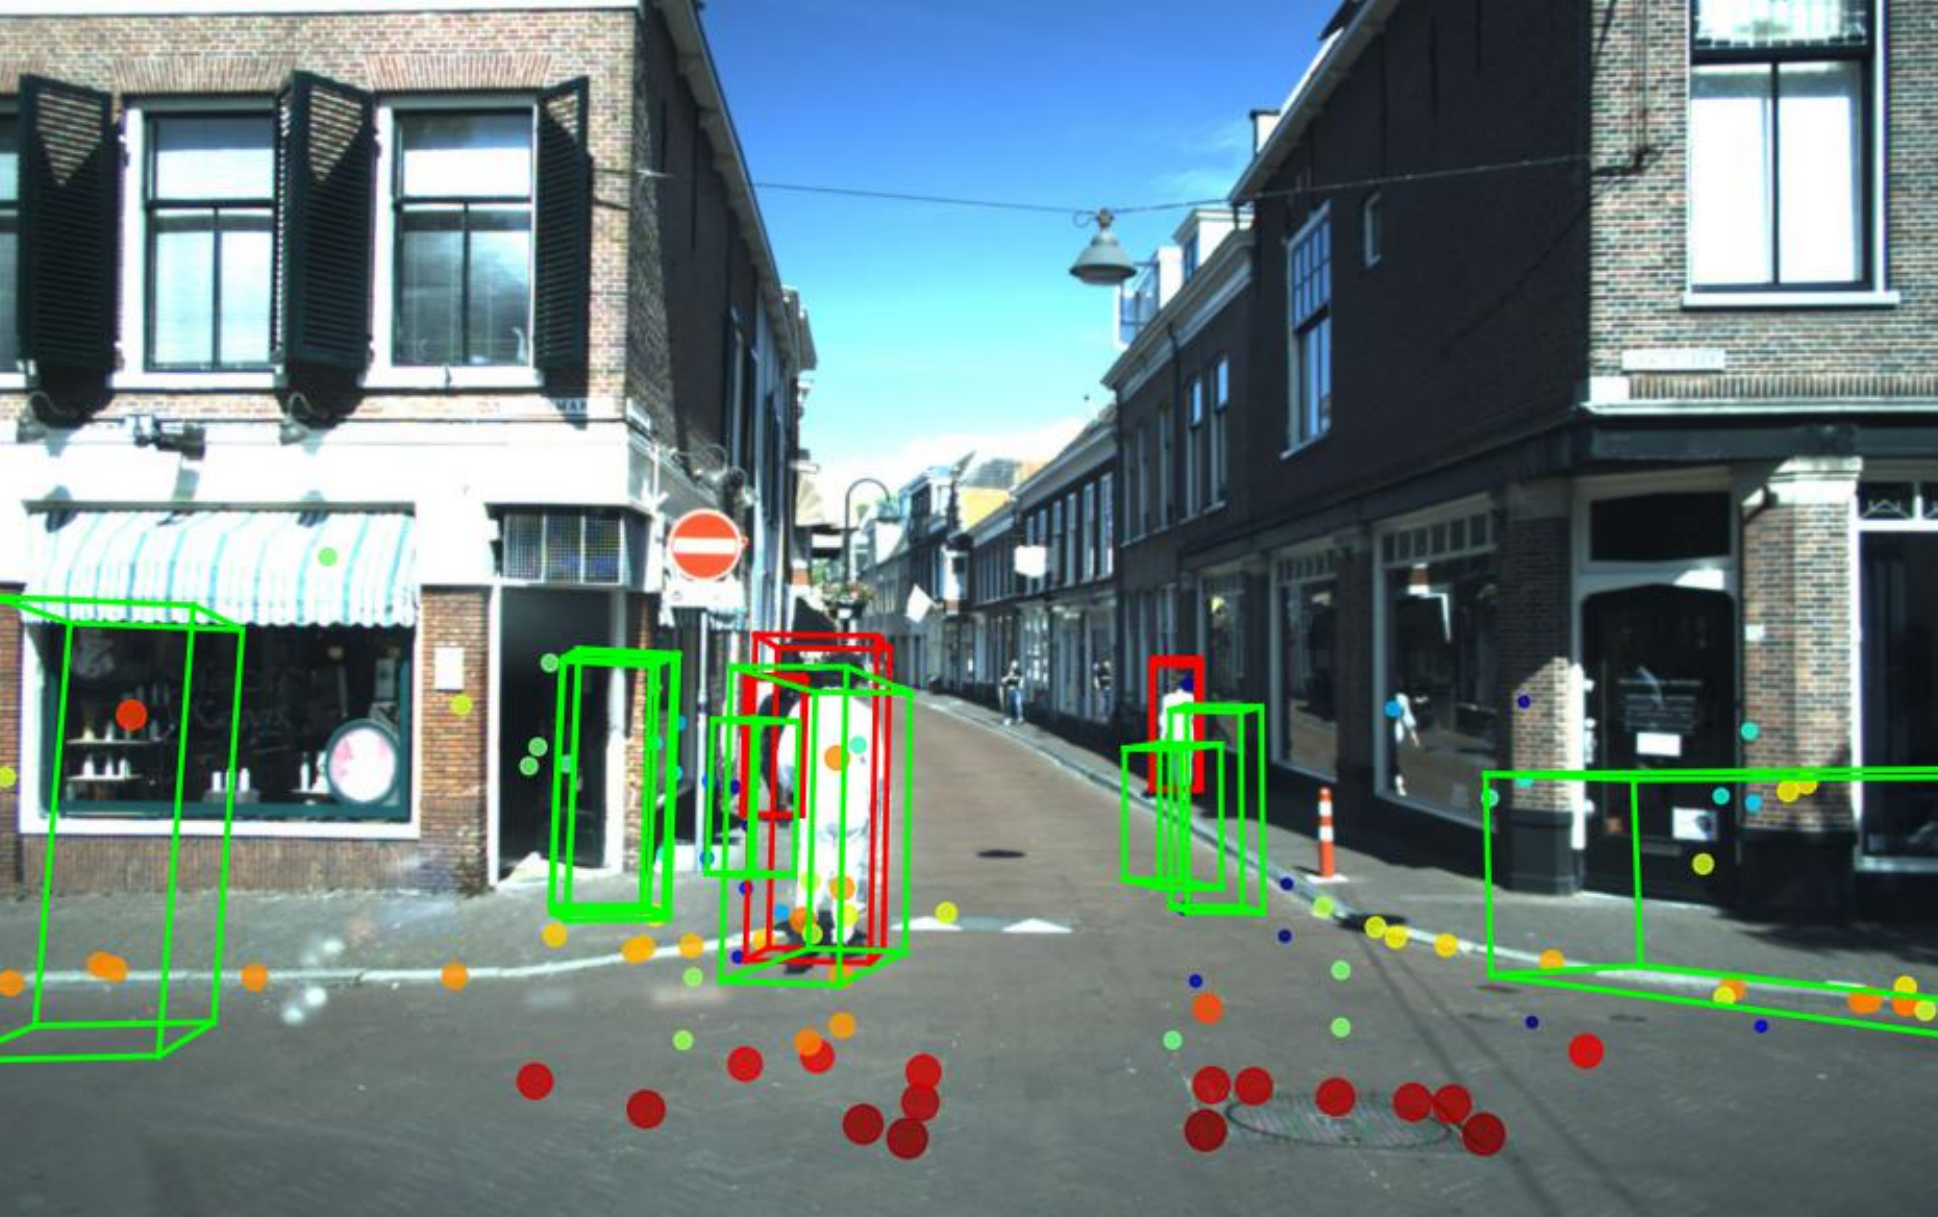}
        \end{subfigure}%
    \end{minipage}\\
    \begin{minipage}[t!]{.22\textwidth}
        \centering
        \begin{subfigure}{.5\textwidth}
            \caption{PointRCNN}
        \end{subfigure}%
        \begin{subfigure}{\textwidth}
            \centering
            \includegraphics[width=\textwidth]{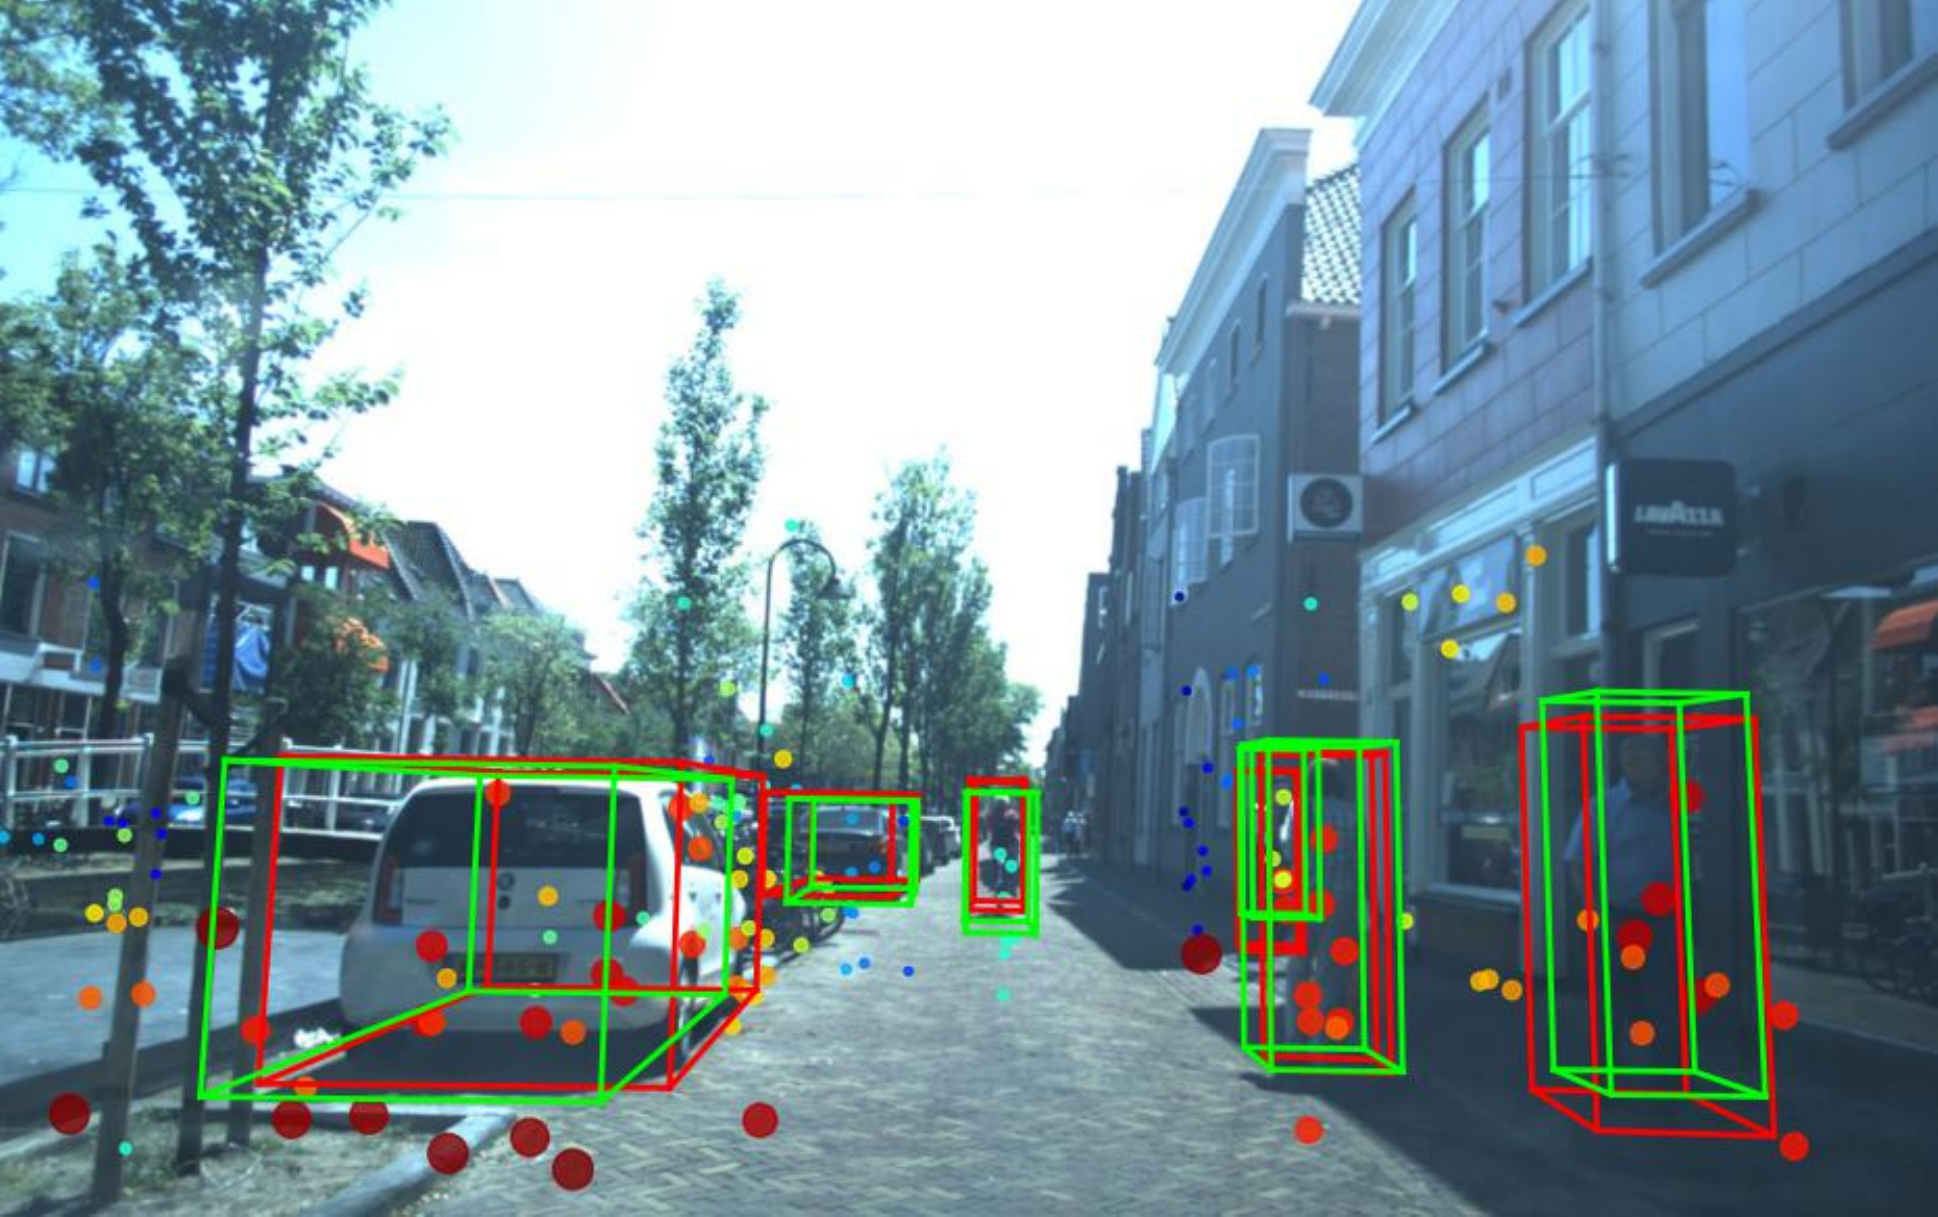}
        \end{subfigure}%
        \begin{subfigure}{\textwidth}
            \centering
            \includegraphics[width=\textwidth]{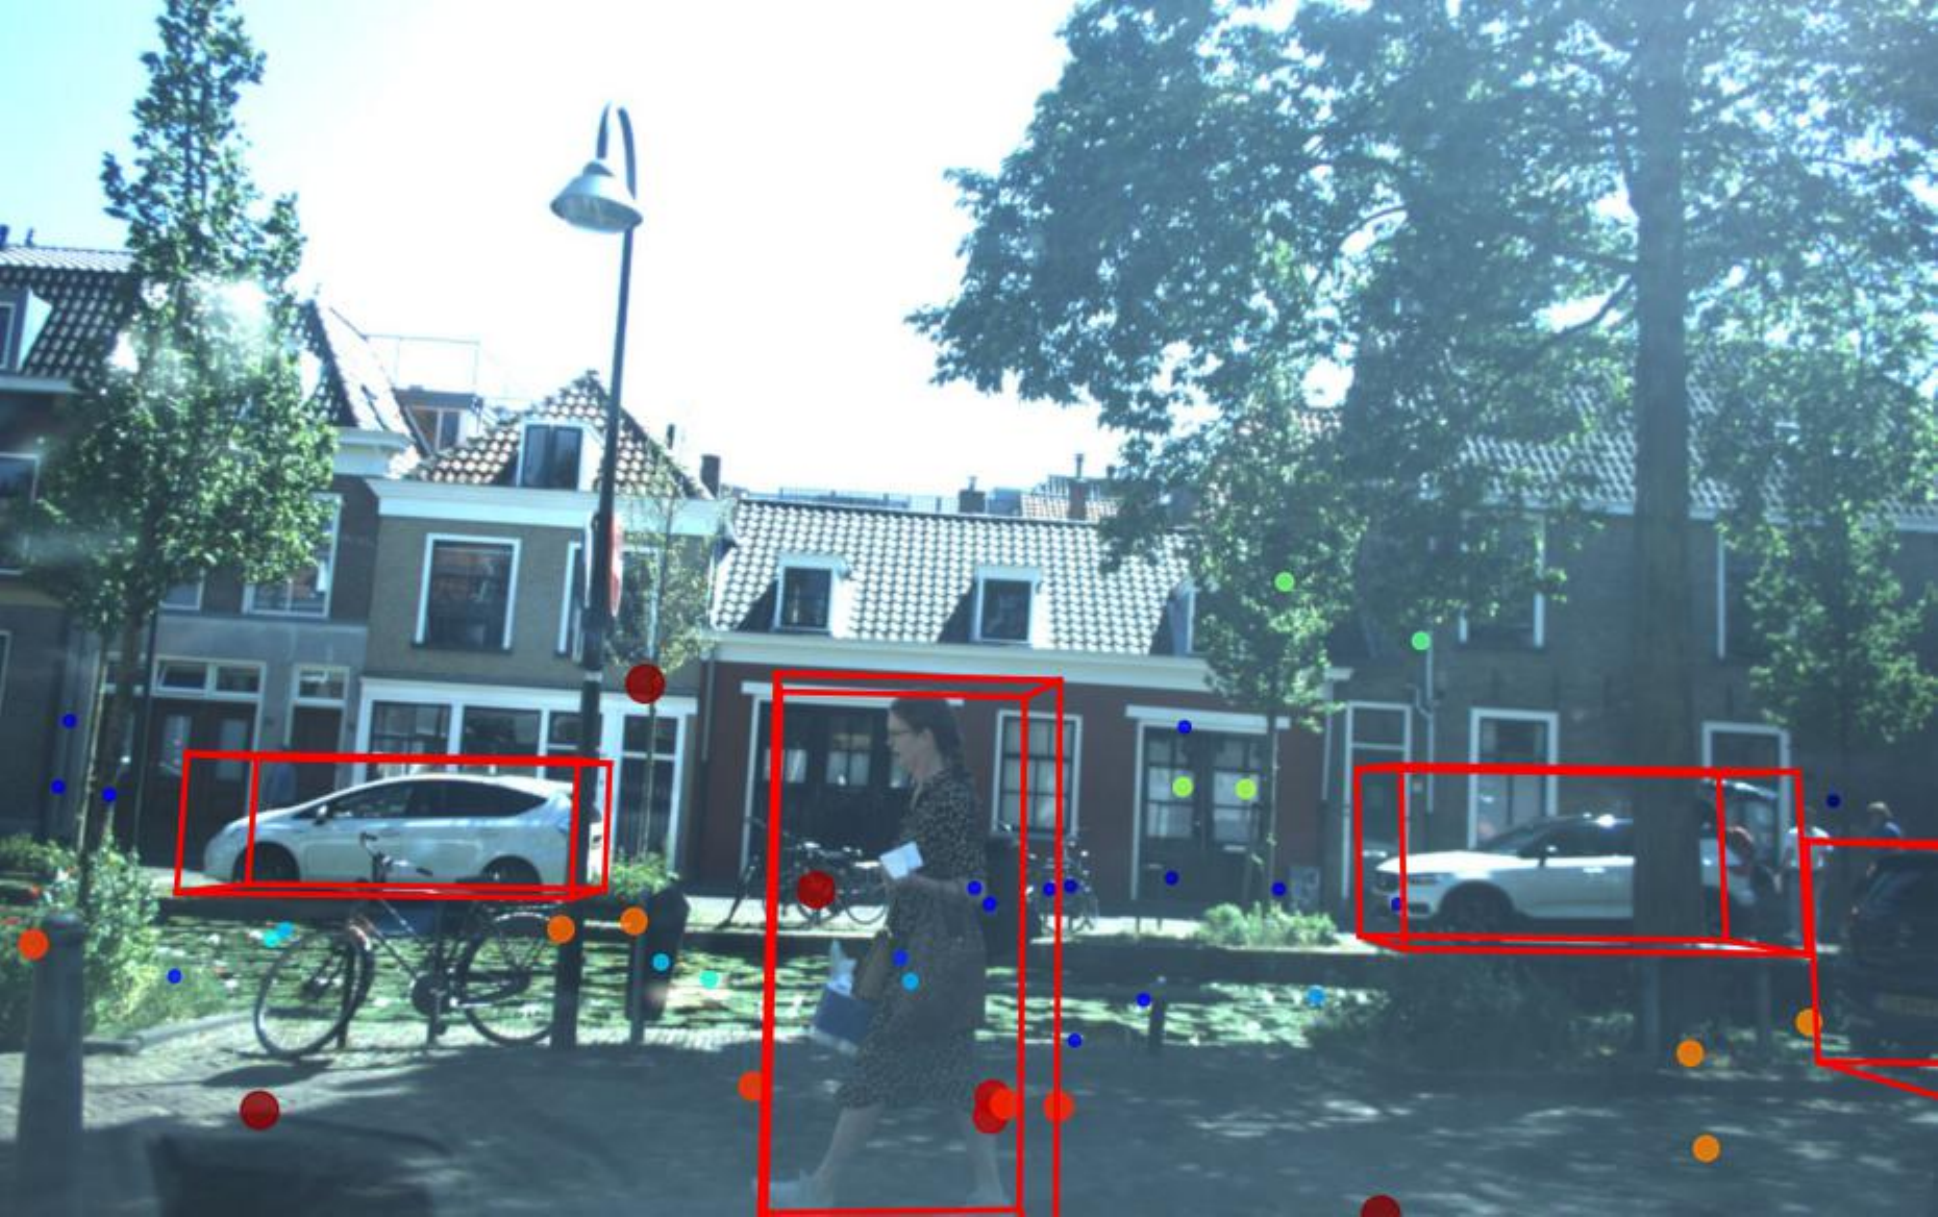}
        \end{subfigure}%
        \begin{subfigure}{\textwidth}
            \centering
        \includegraphics[width=\textwidth]{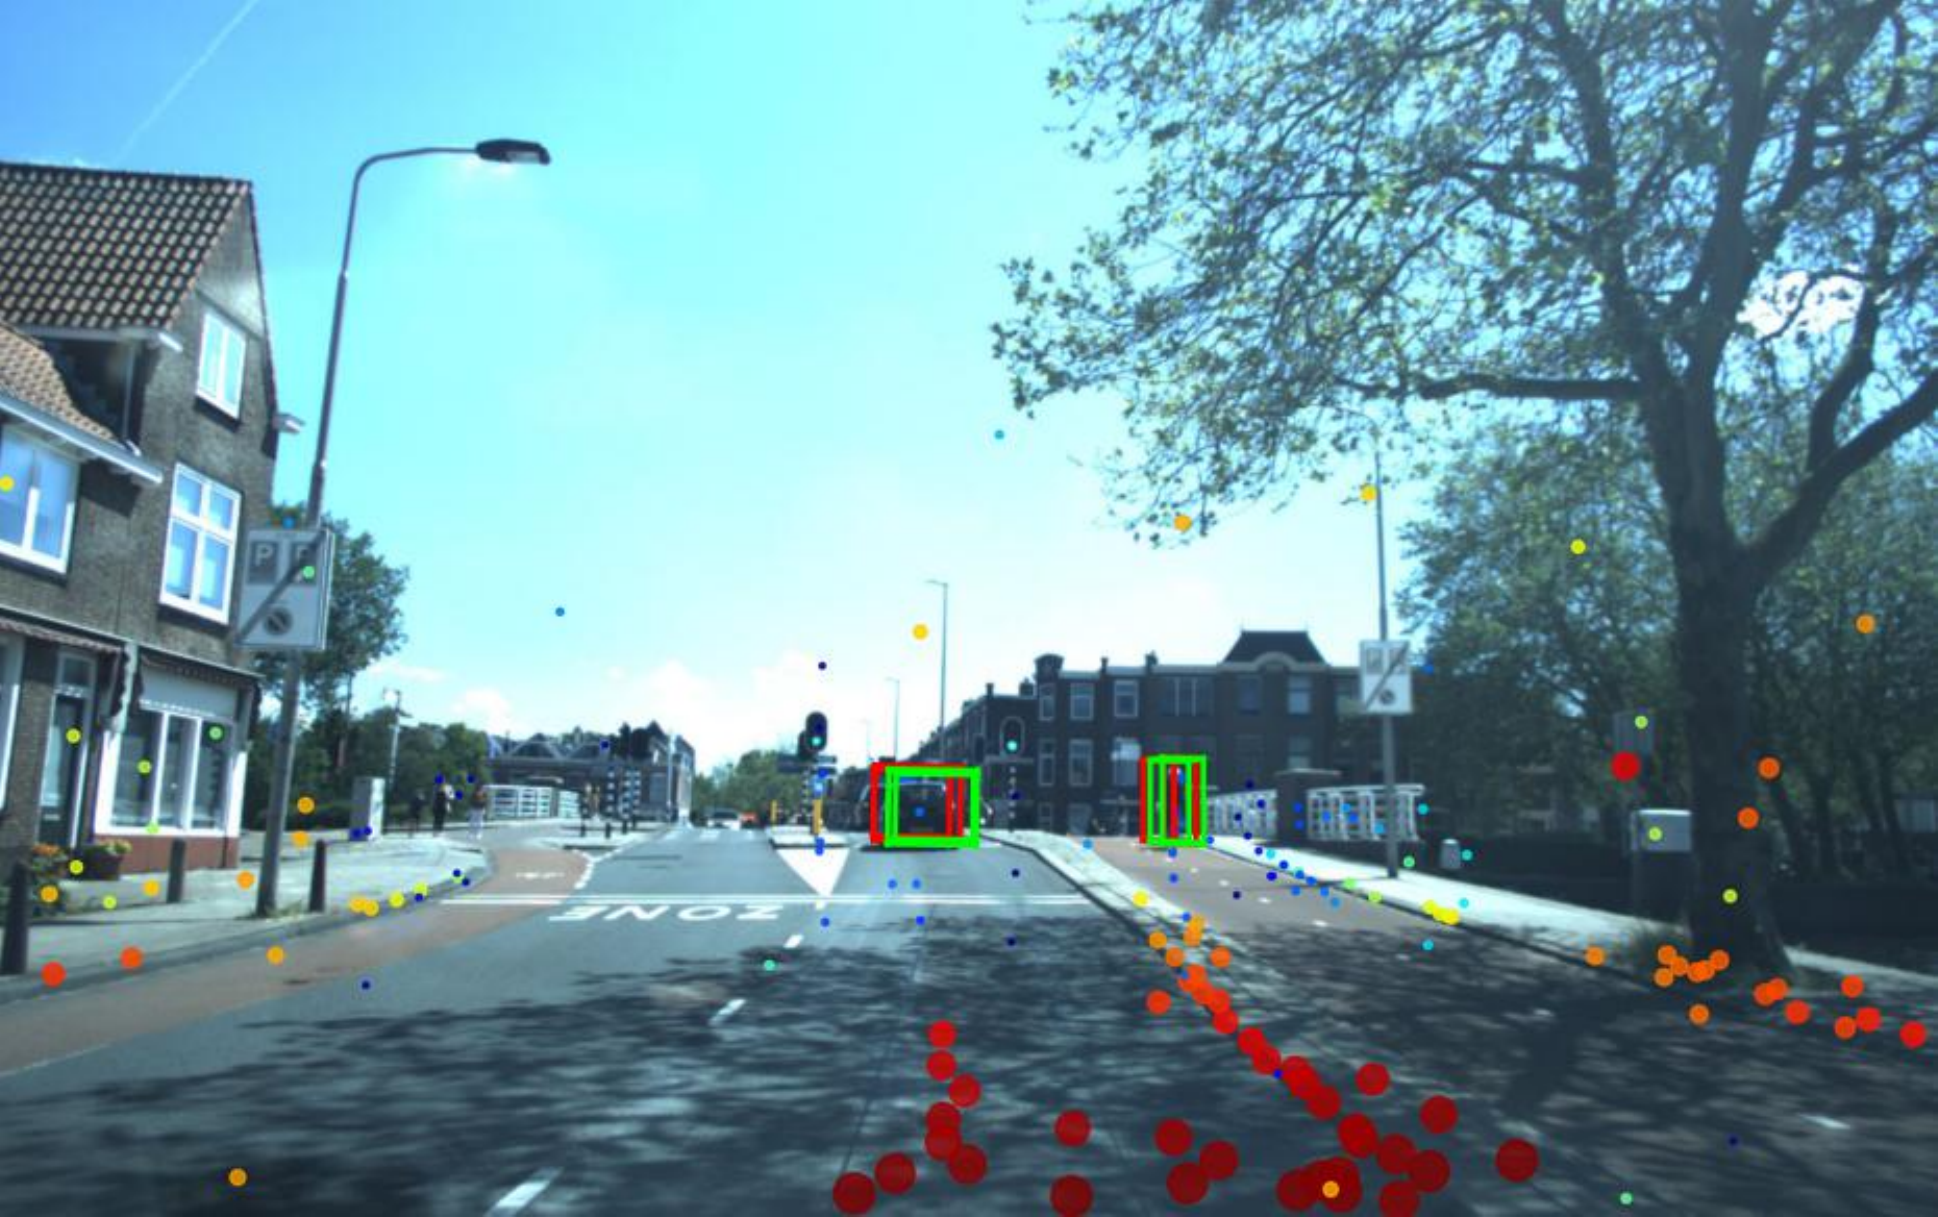}
        \end{subfigure}%
        \begin{subfigure}{\textwidth}
            \centering
            \includegraphics[width=\textwidth]{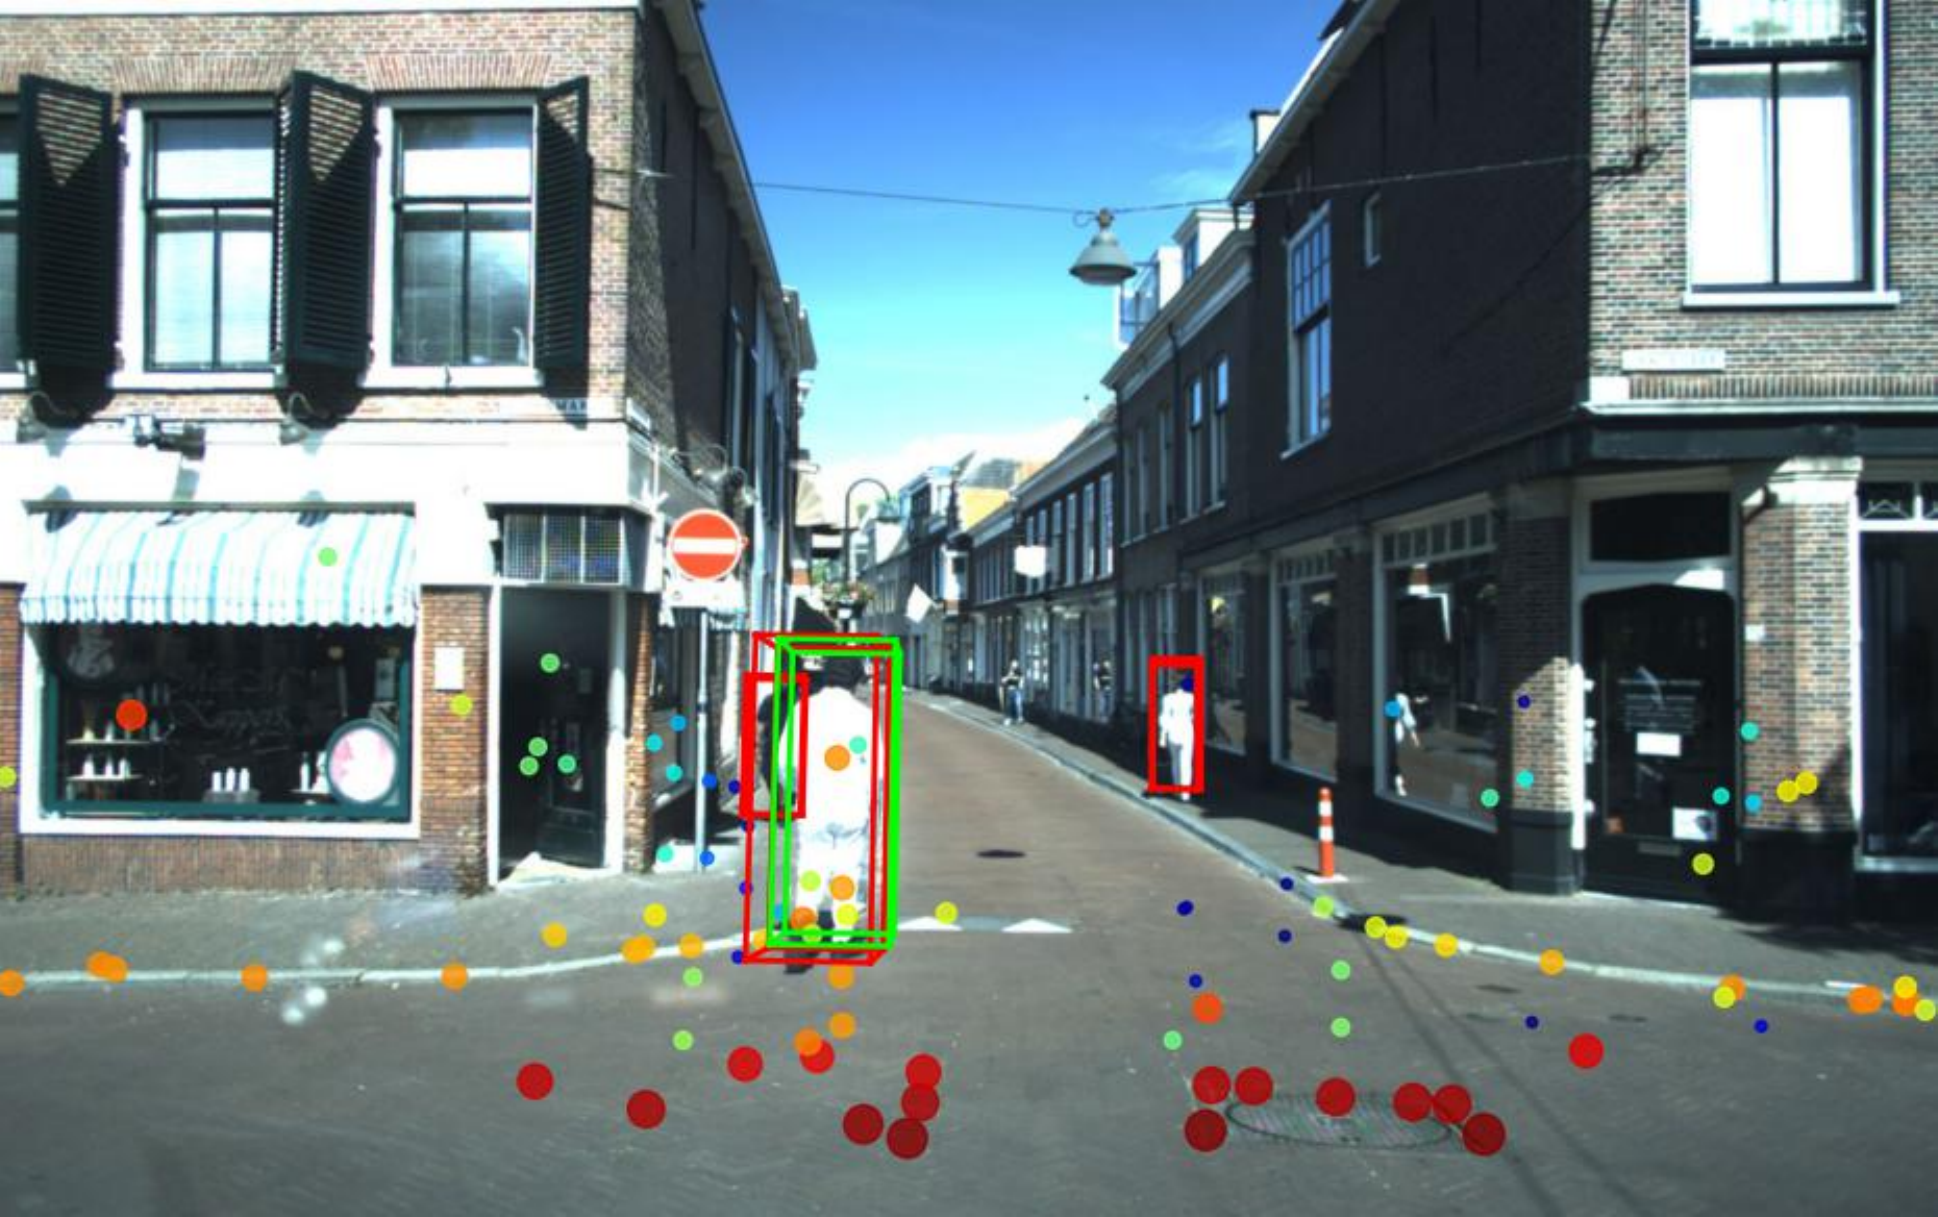}
        \end{subfigure}%
    \end{minipage}\\
    \begin{minipage}[t!]{.22\textwidth}
        \centering
        \begin{subfigure}{.5\textwidth}
            \caption{3DSSD}
        \end{subfigure}%
        \begin{subfigure}{\textwidth}
            \centering
            \includegraphics[width=\textwidth]{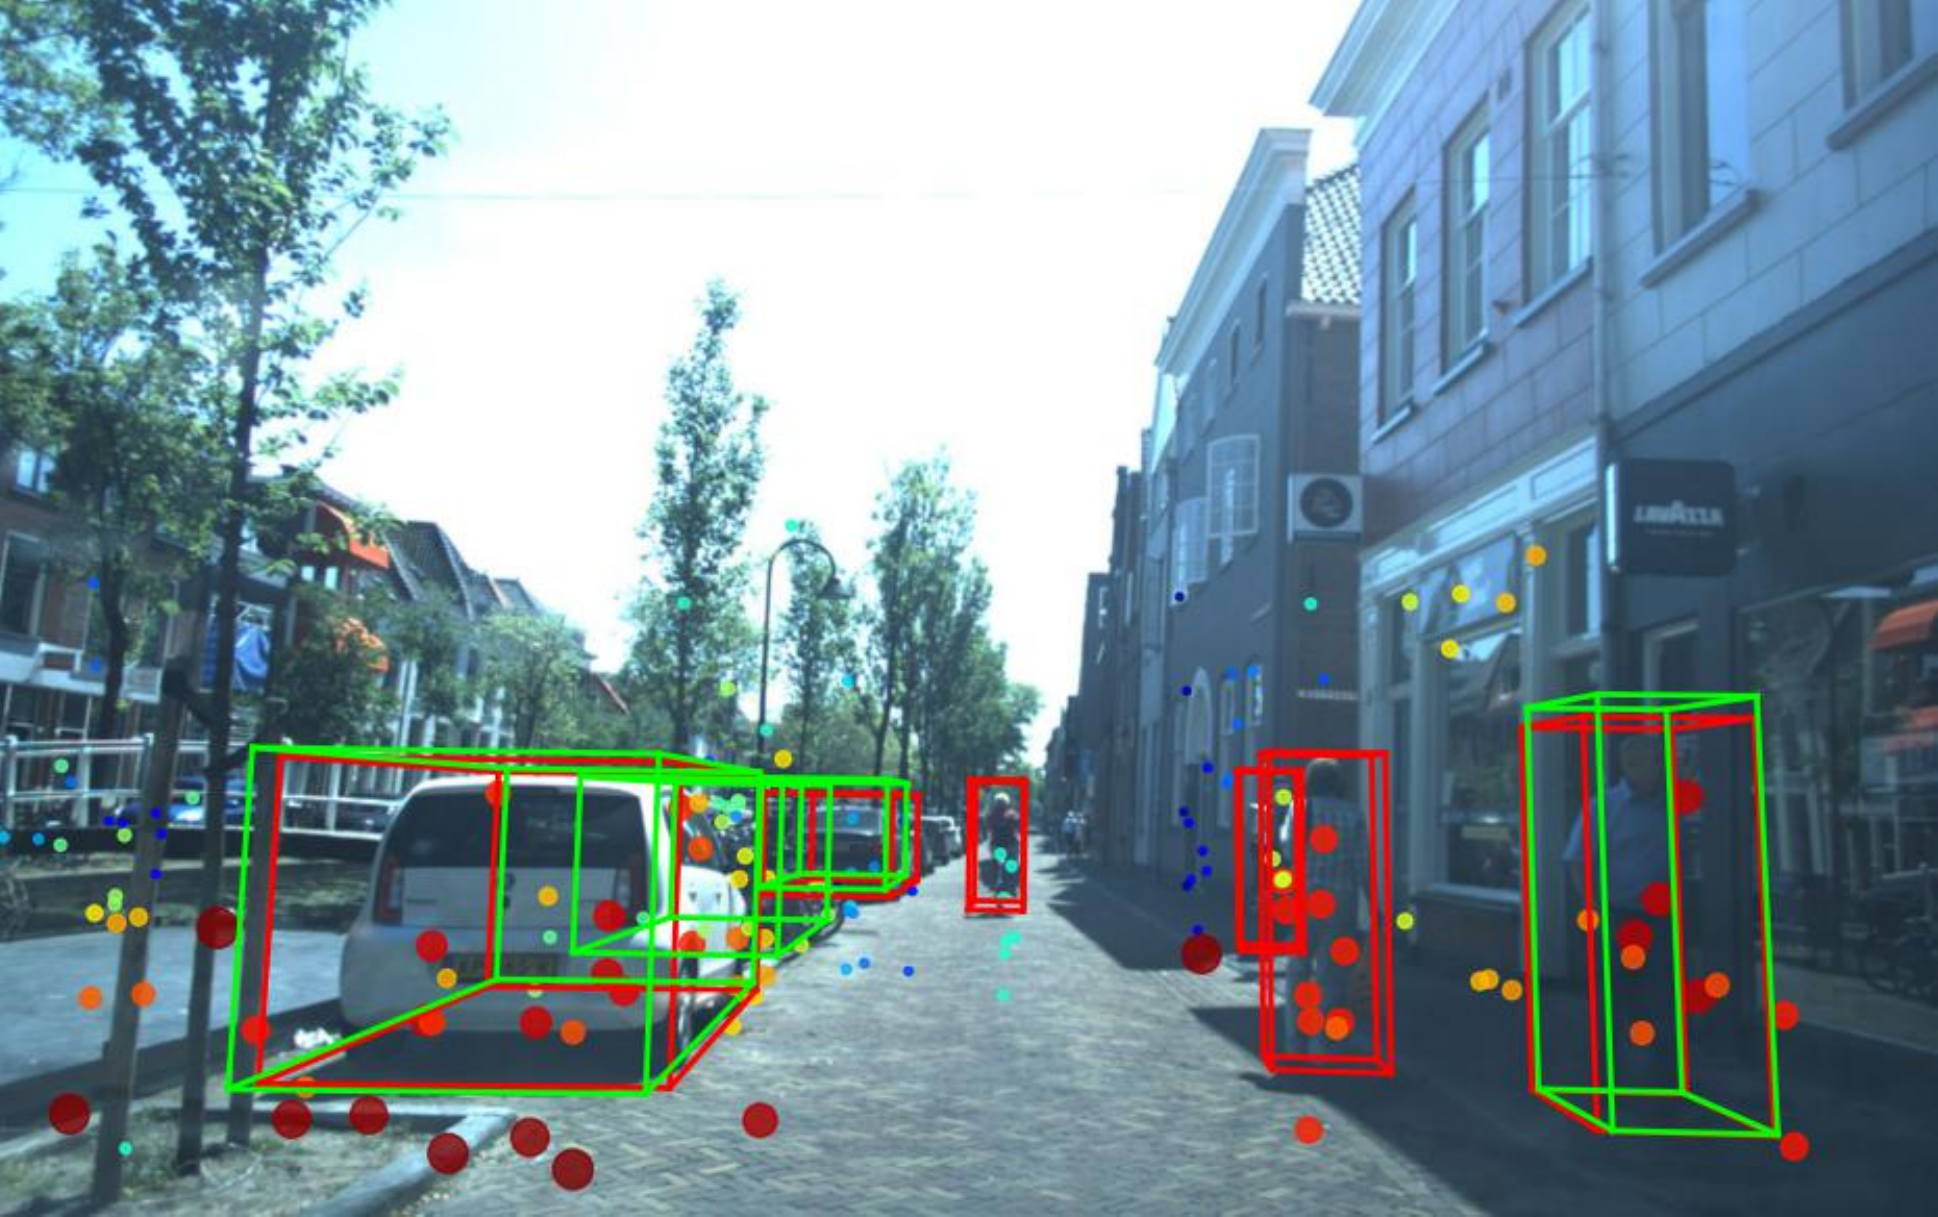}
        \end{subfigure}%
        \begin{subfigure}{\textwidth}
            \centering
            \includegraphics[width=\textwidth]{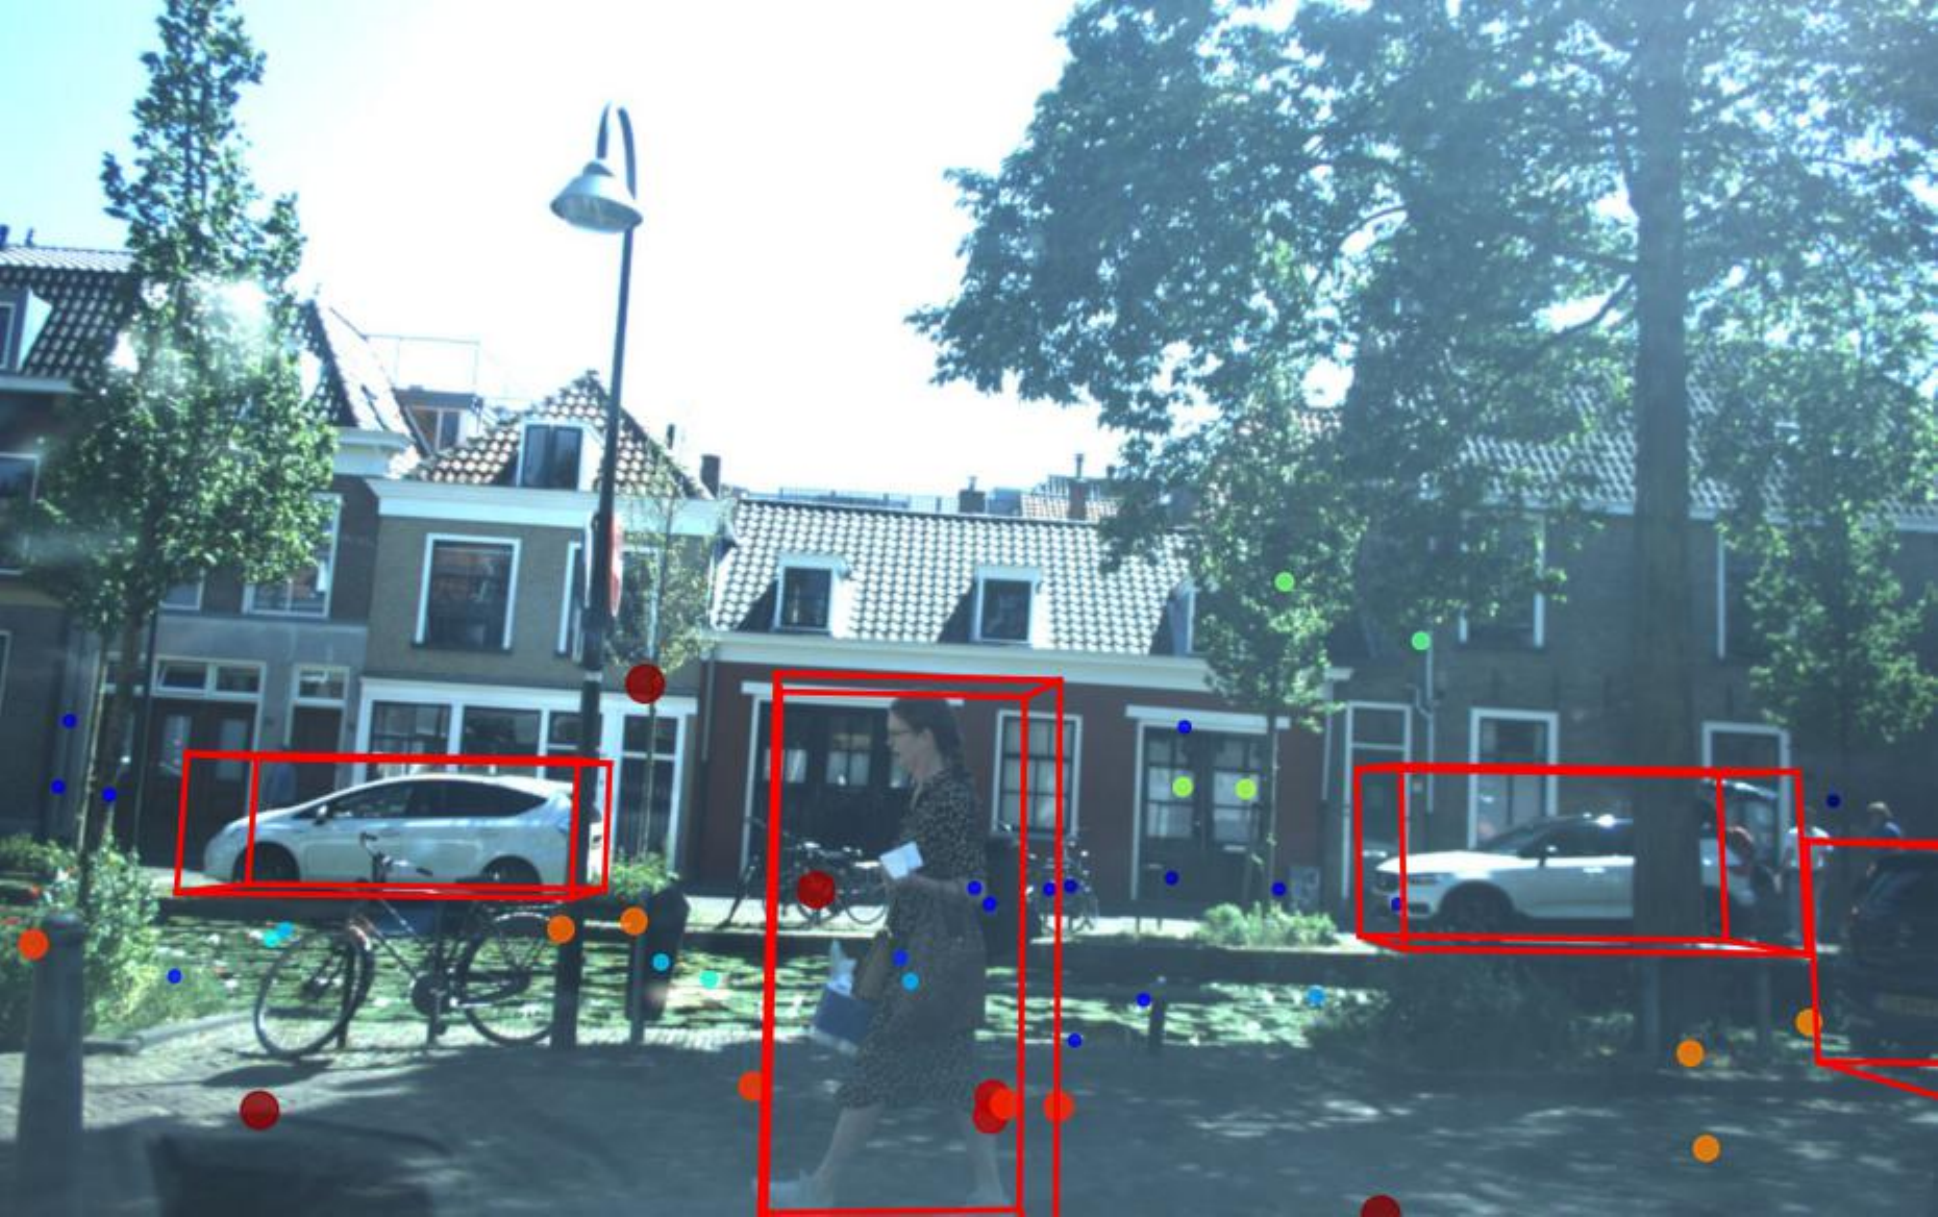}
        \end{subfigure}%
        \begin{subfigure}{\textwidth}
            \centering
            \includegraphics[width=\textwidth]{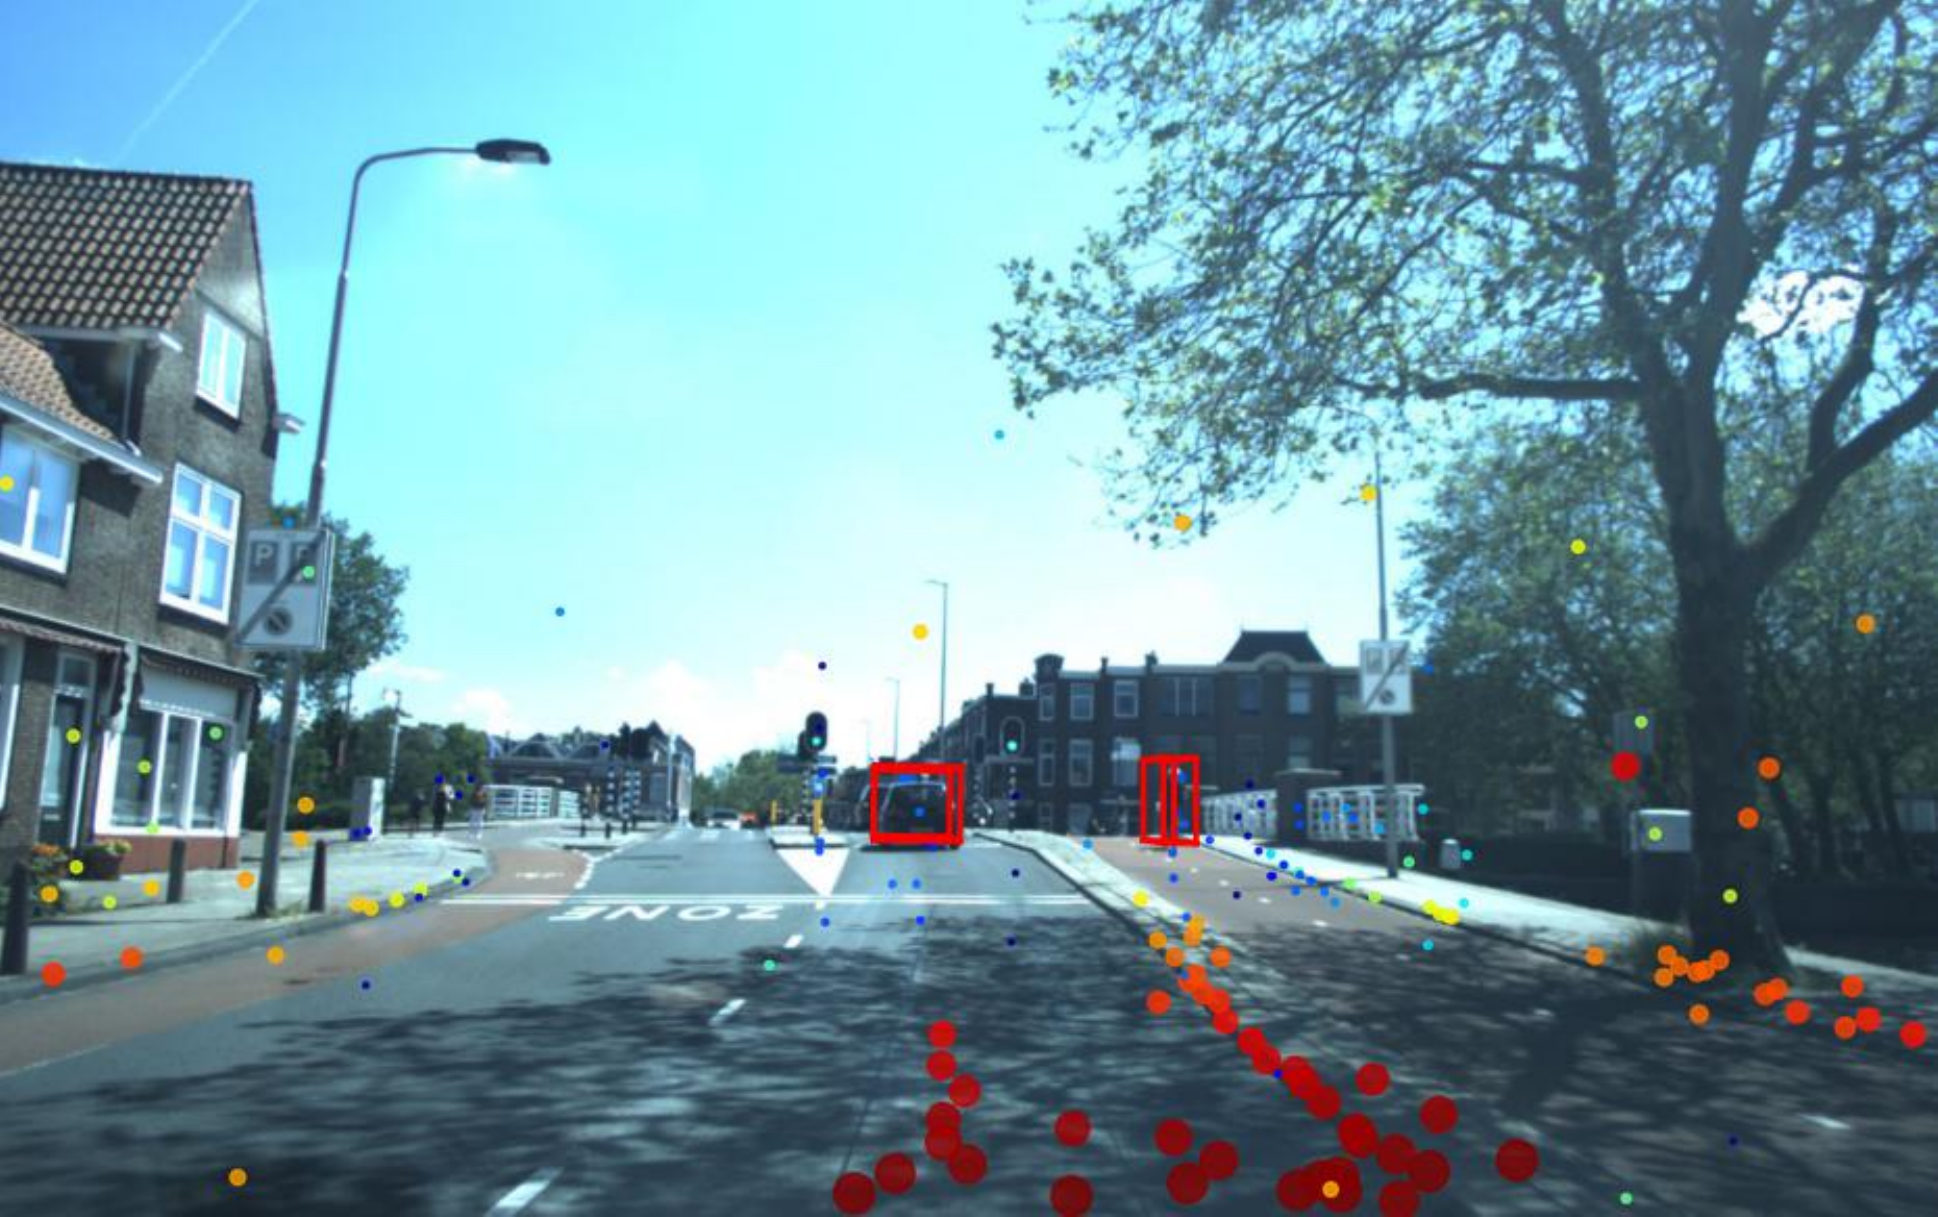}
        \end{subfigure}%
        \begin{subfigure}{\textwidth}
            \centering
            \includegraphics[width=\textwidth]{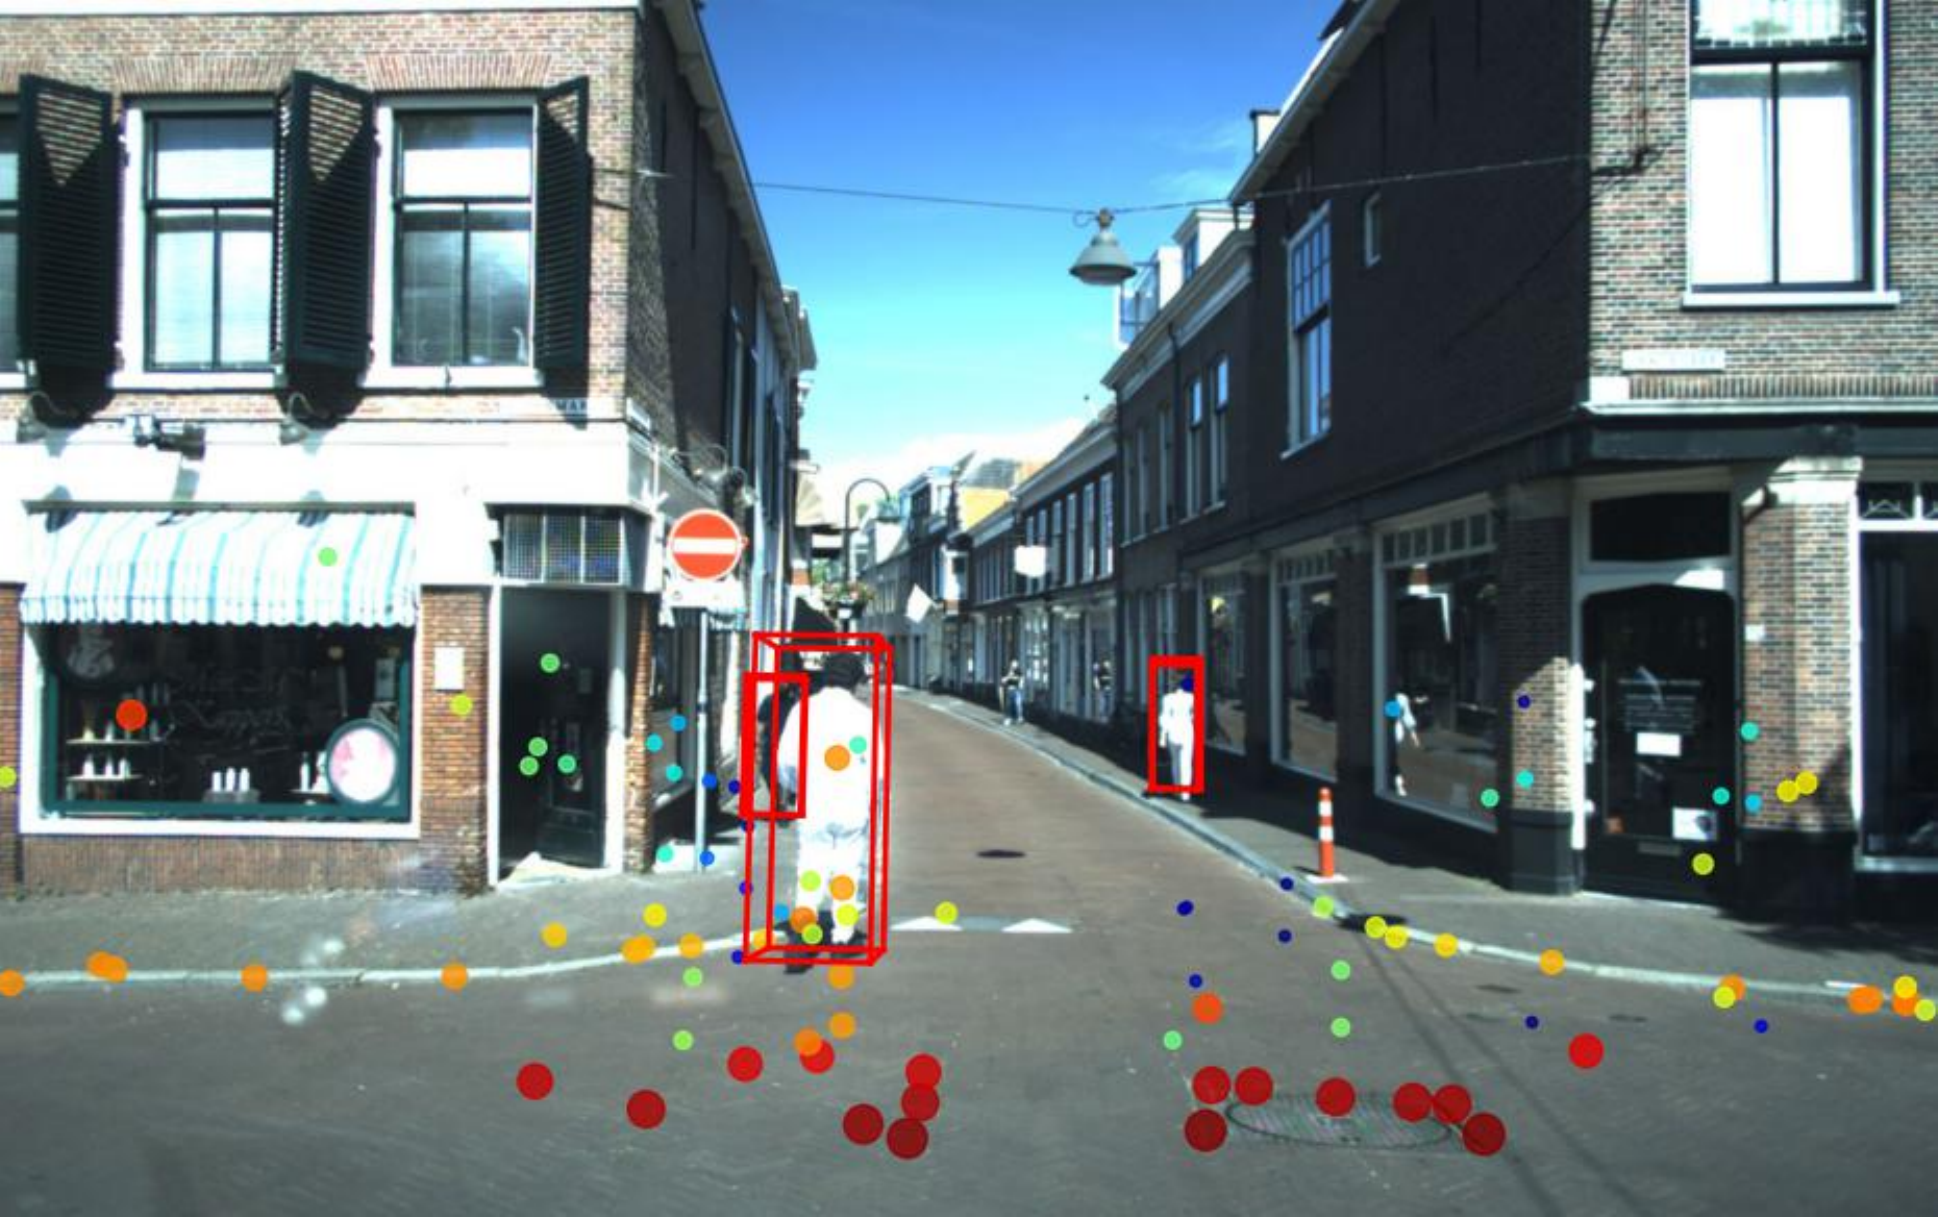}
        \end{subfigure}%
    \end{minipage}\\
    \begin{minipage}[t!]{.22\textwidth}
        \centering
        \begin{subfigure}{.5\textwidth}
            \caption{IASSD}
        \end{subfigure}%
        \begin{subfigure}{\textwidth}
            \centering
            \includegraphics[width=\textwidth]{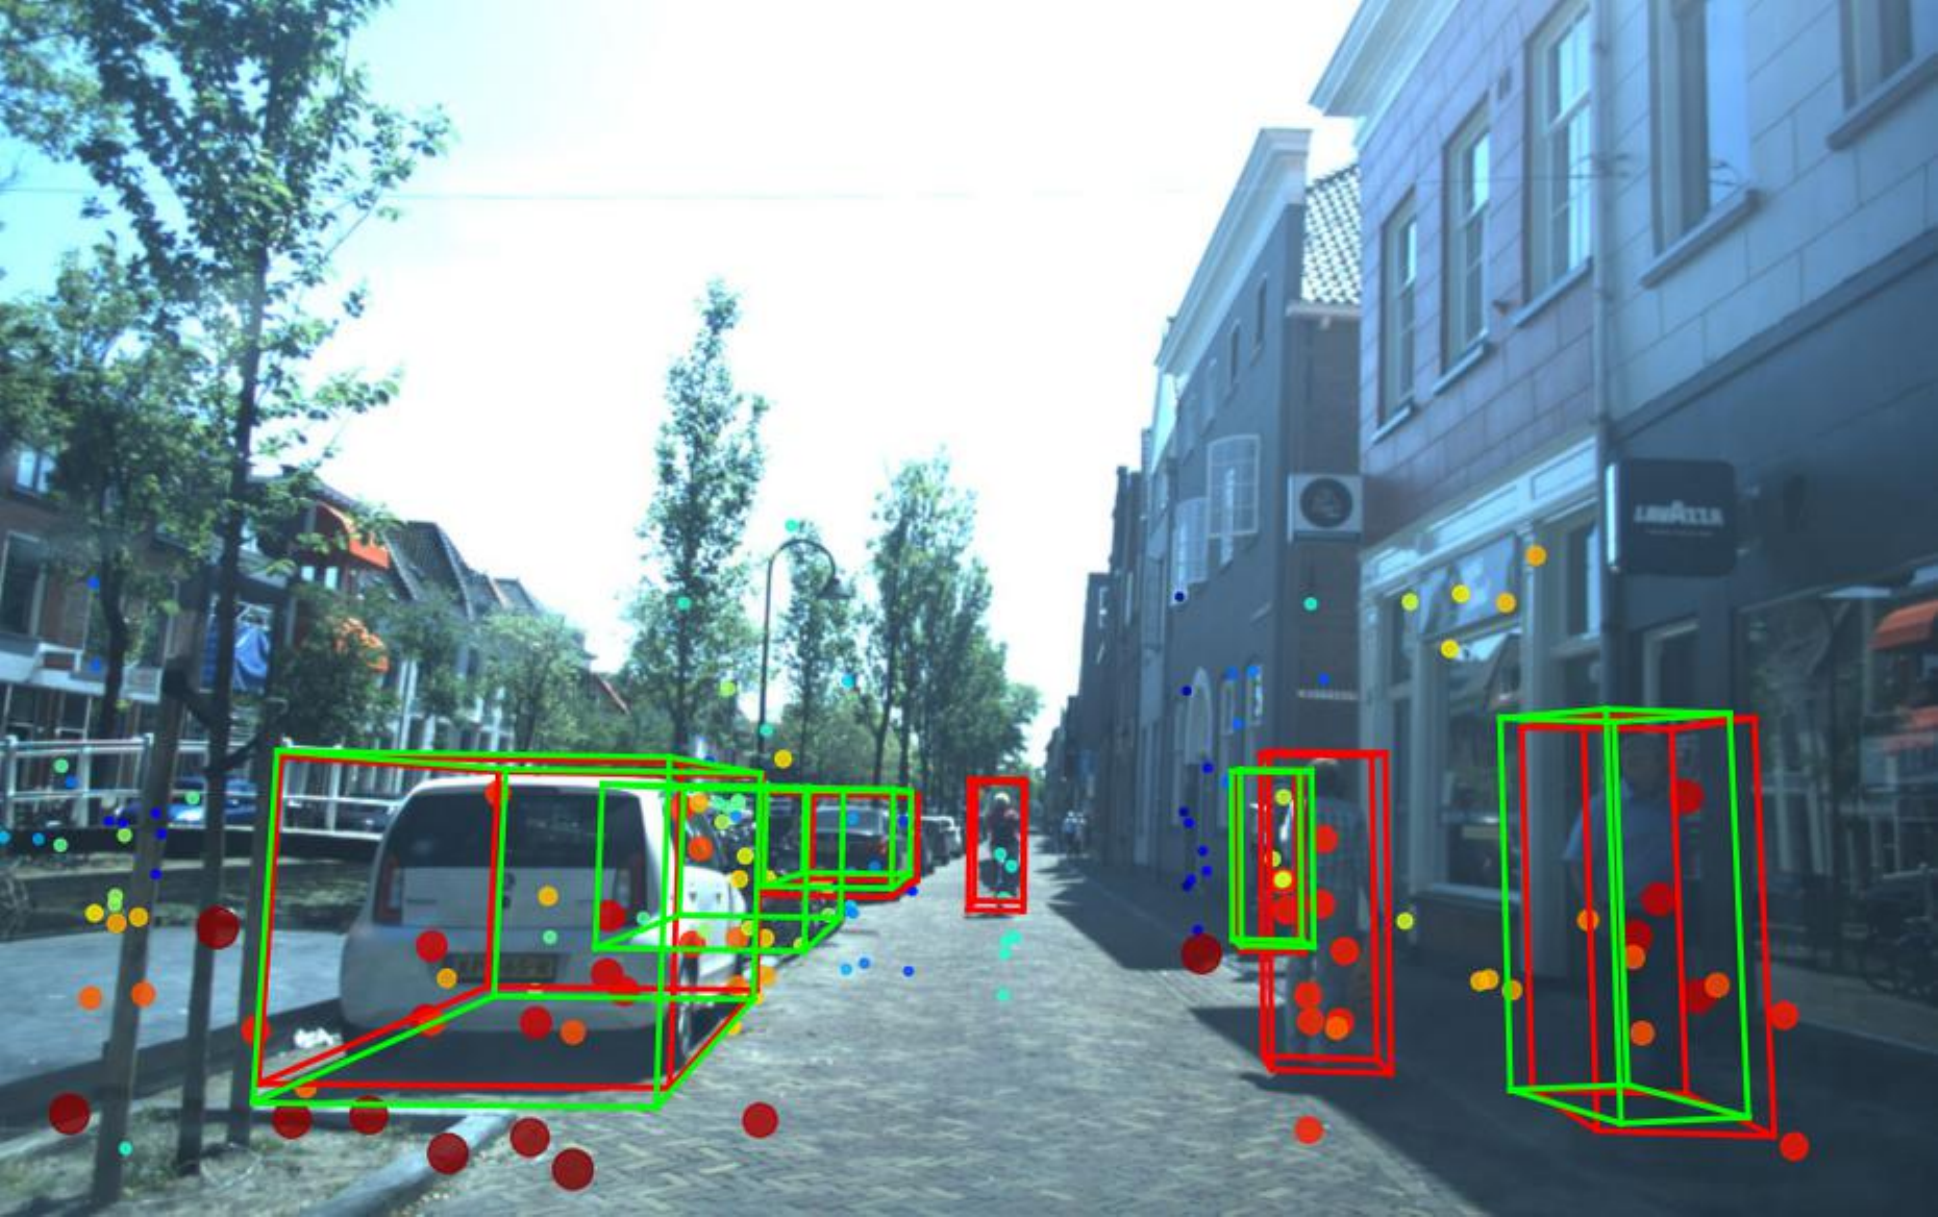}
        \end{subfigure}%
        \begin{subfigure}{\textwidth}
            \centering
            \includegraphics[width=\textwidth]{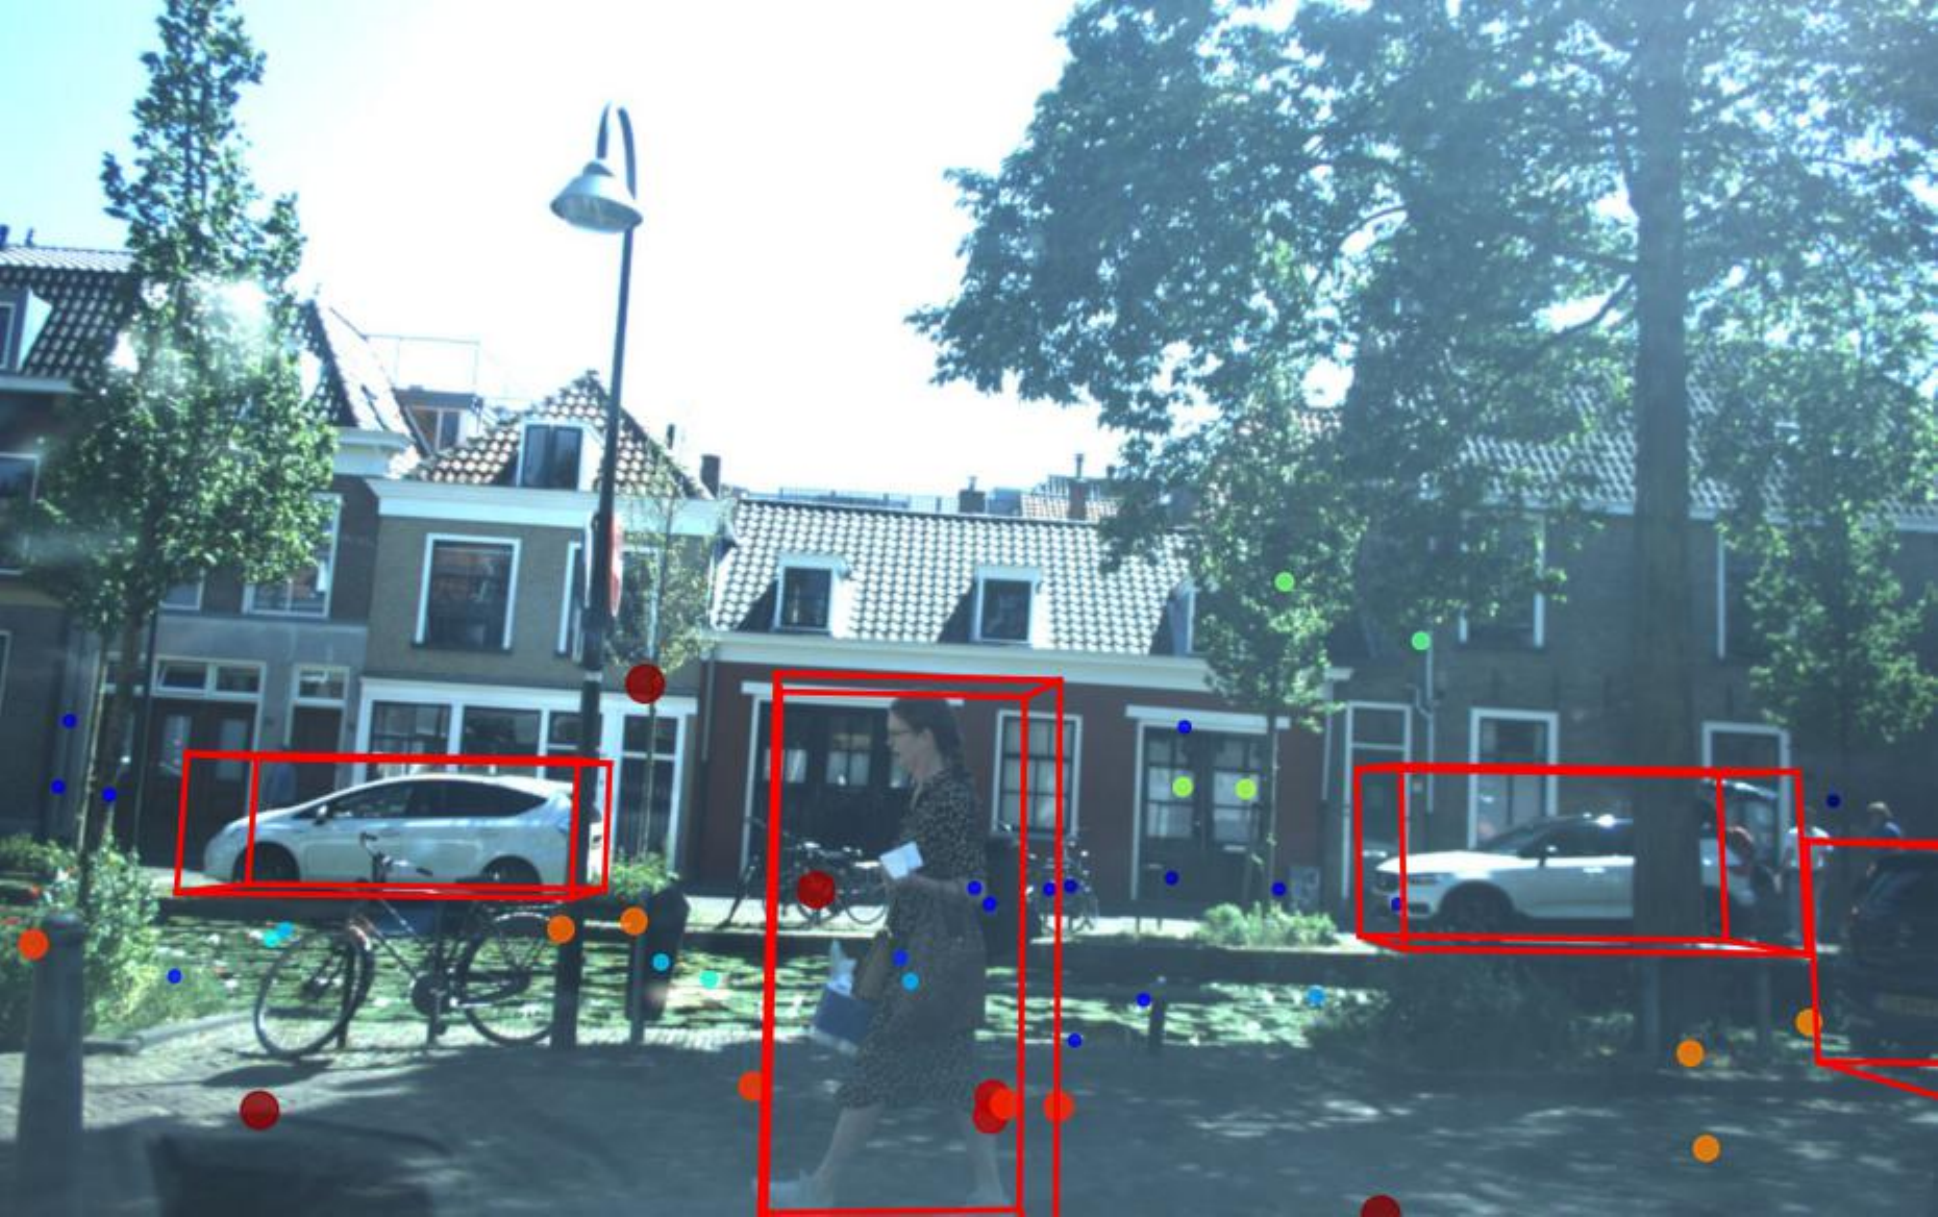}
        \end{subfigure}%
        \begin{subfigure}{\textwidth}
            \centering
            \includegraphics[width=\textwidth]{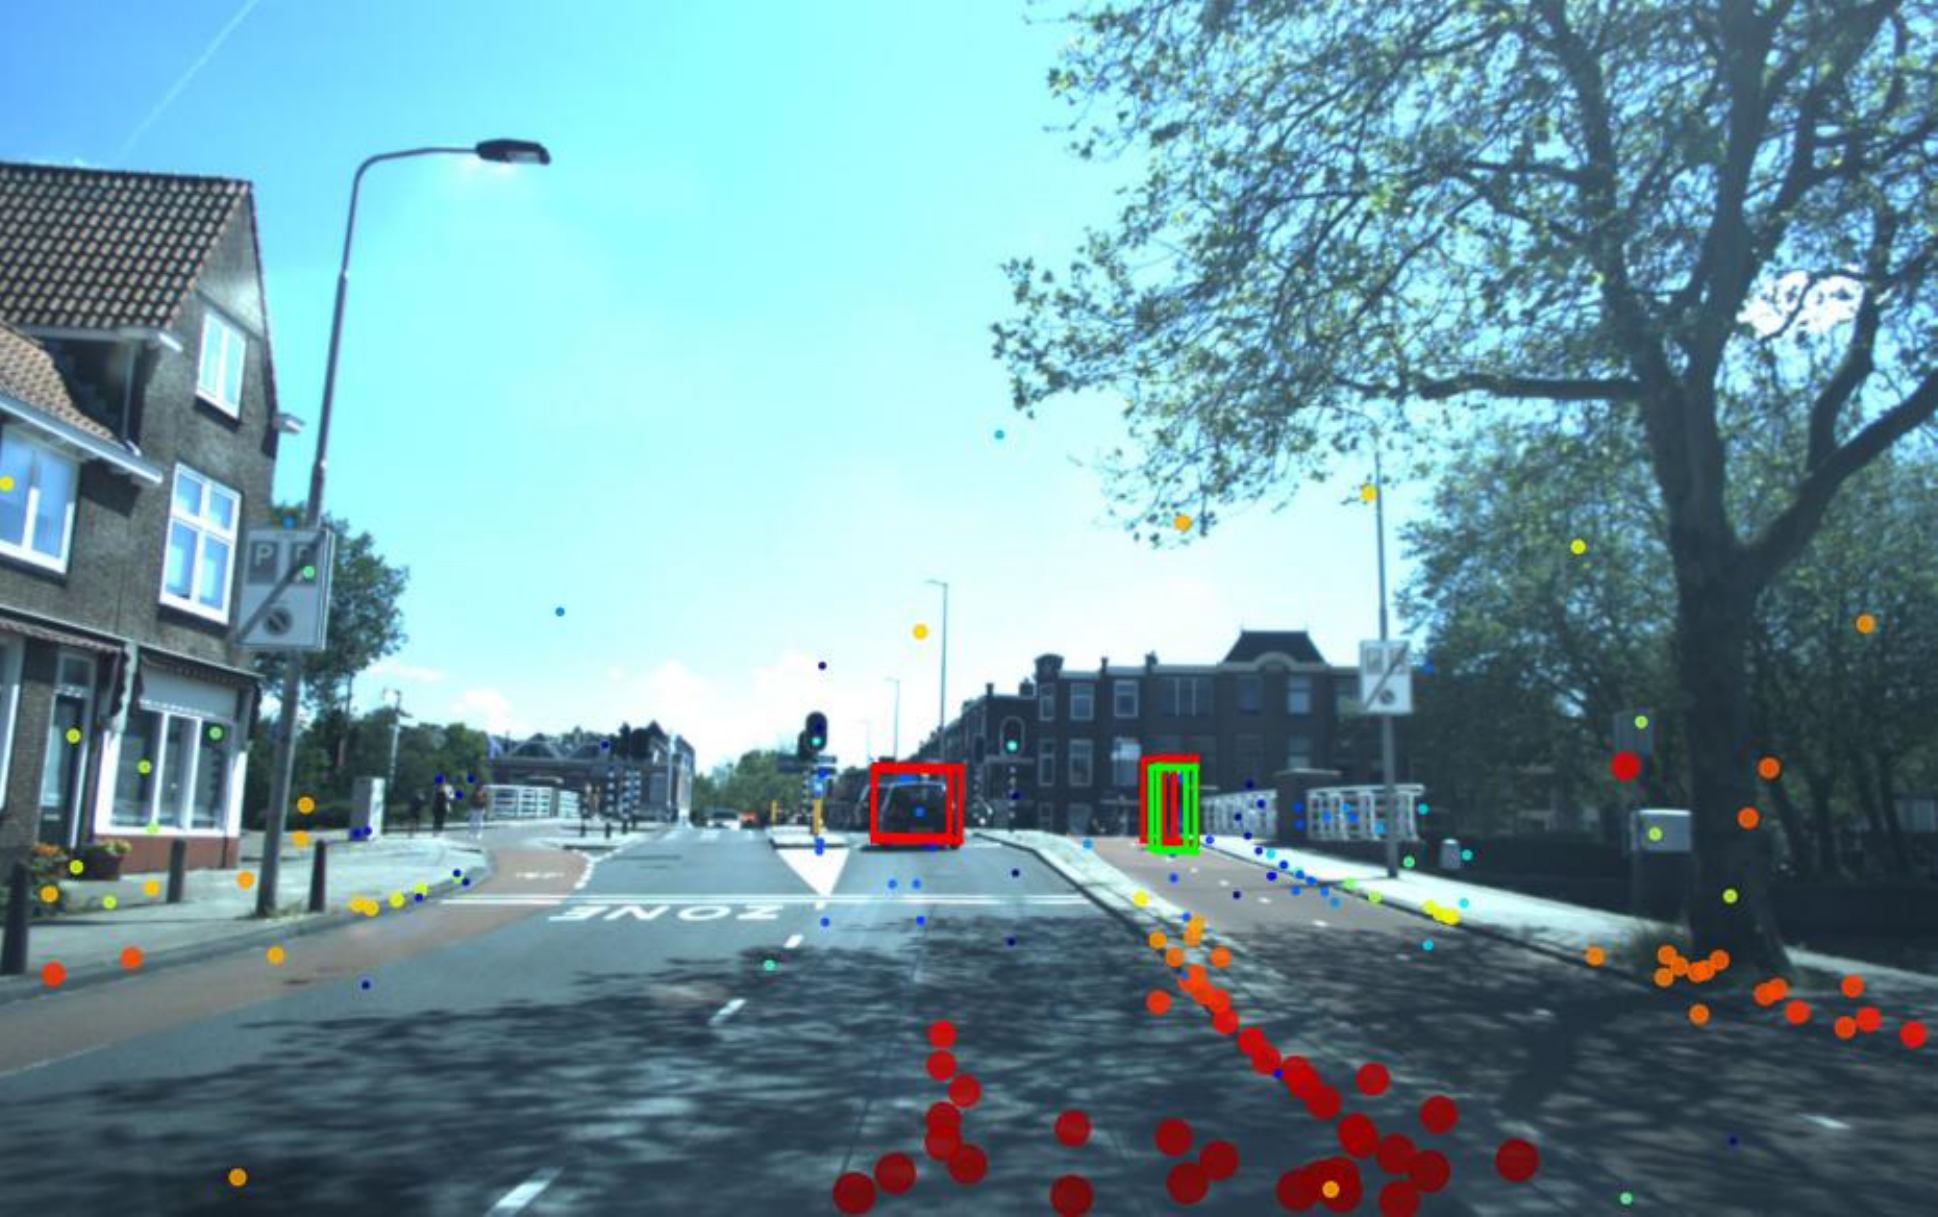}
        \end{subfigure}%
        \begin{subfigure}{\textwidth}
            \centering
            \includegraphics[width=\textwidth]{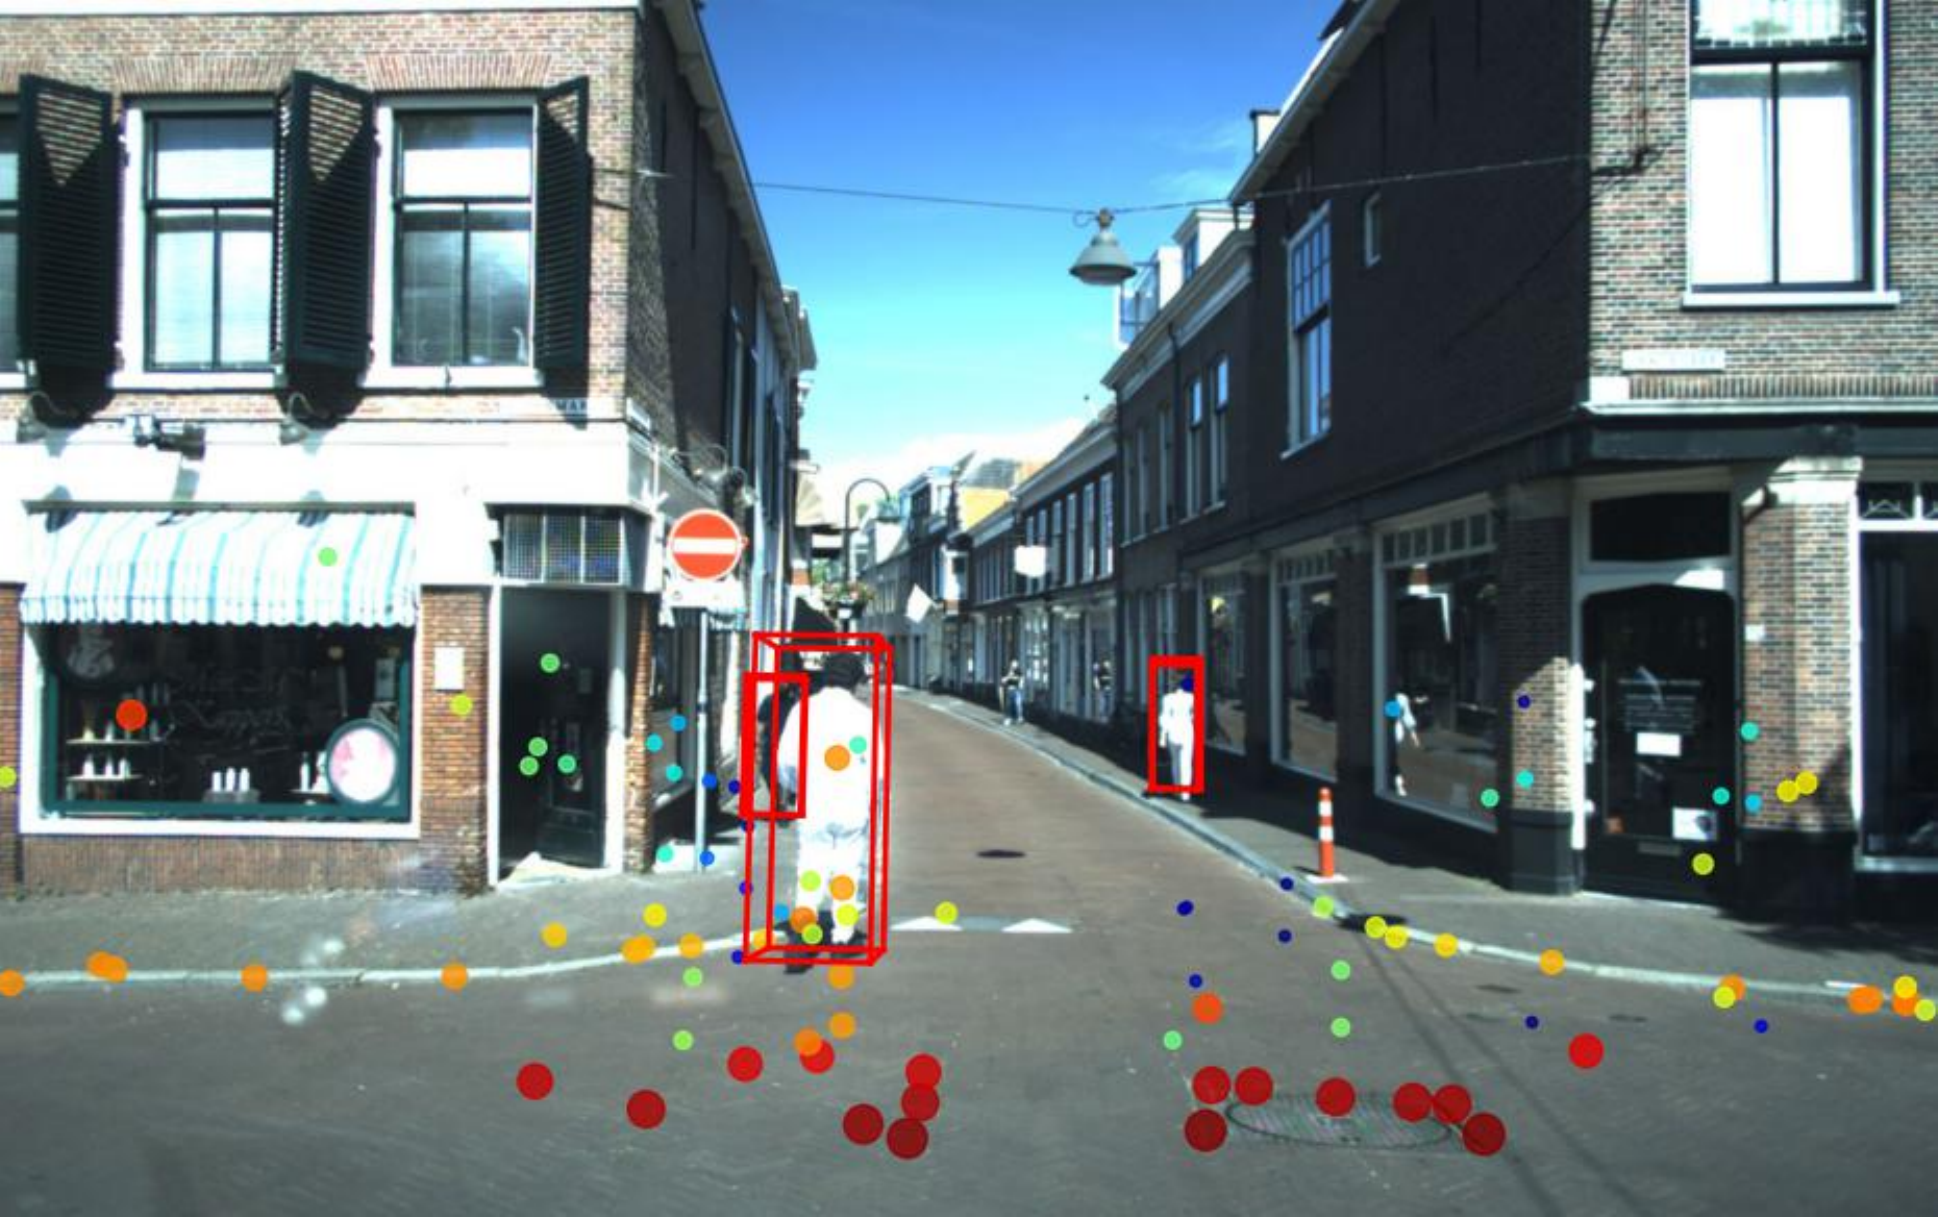}
        \end{subfigure}%
    \end{minipage}\\
    \begin{minipage}[t!]{.22\textwidth}
        \centering
        \begin{subfigure}{.5\textwidth}
            \caption{PVRCNN}
        \end{subfigure}%
        \begin{subfigure}{\textwidth}
            \centering
            \includegraphics[width=\textwidth]{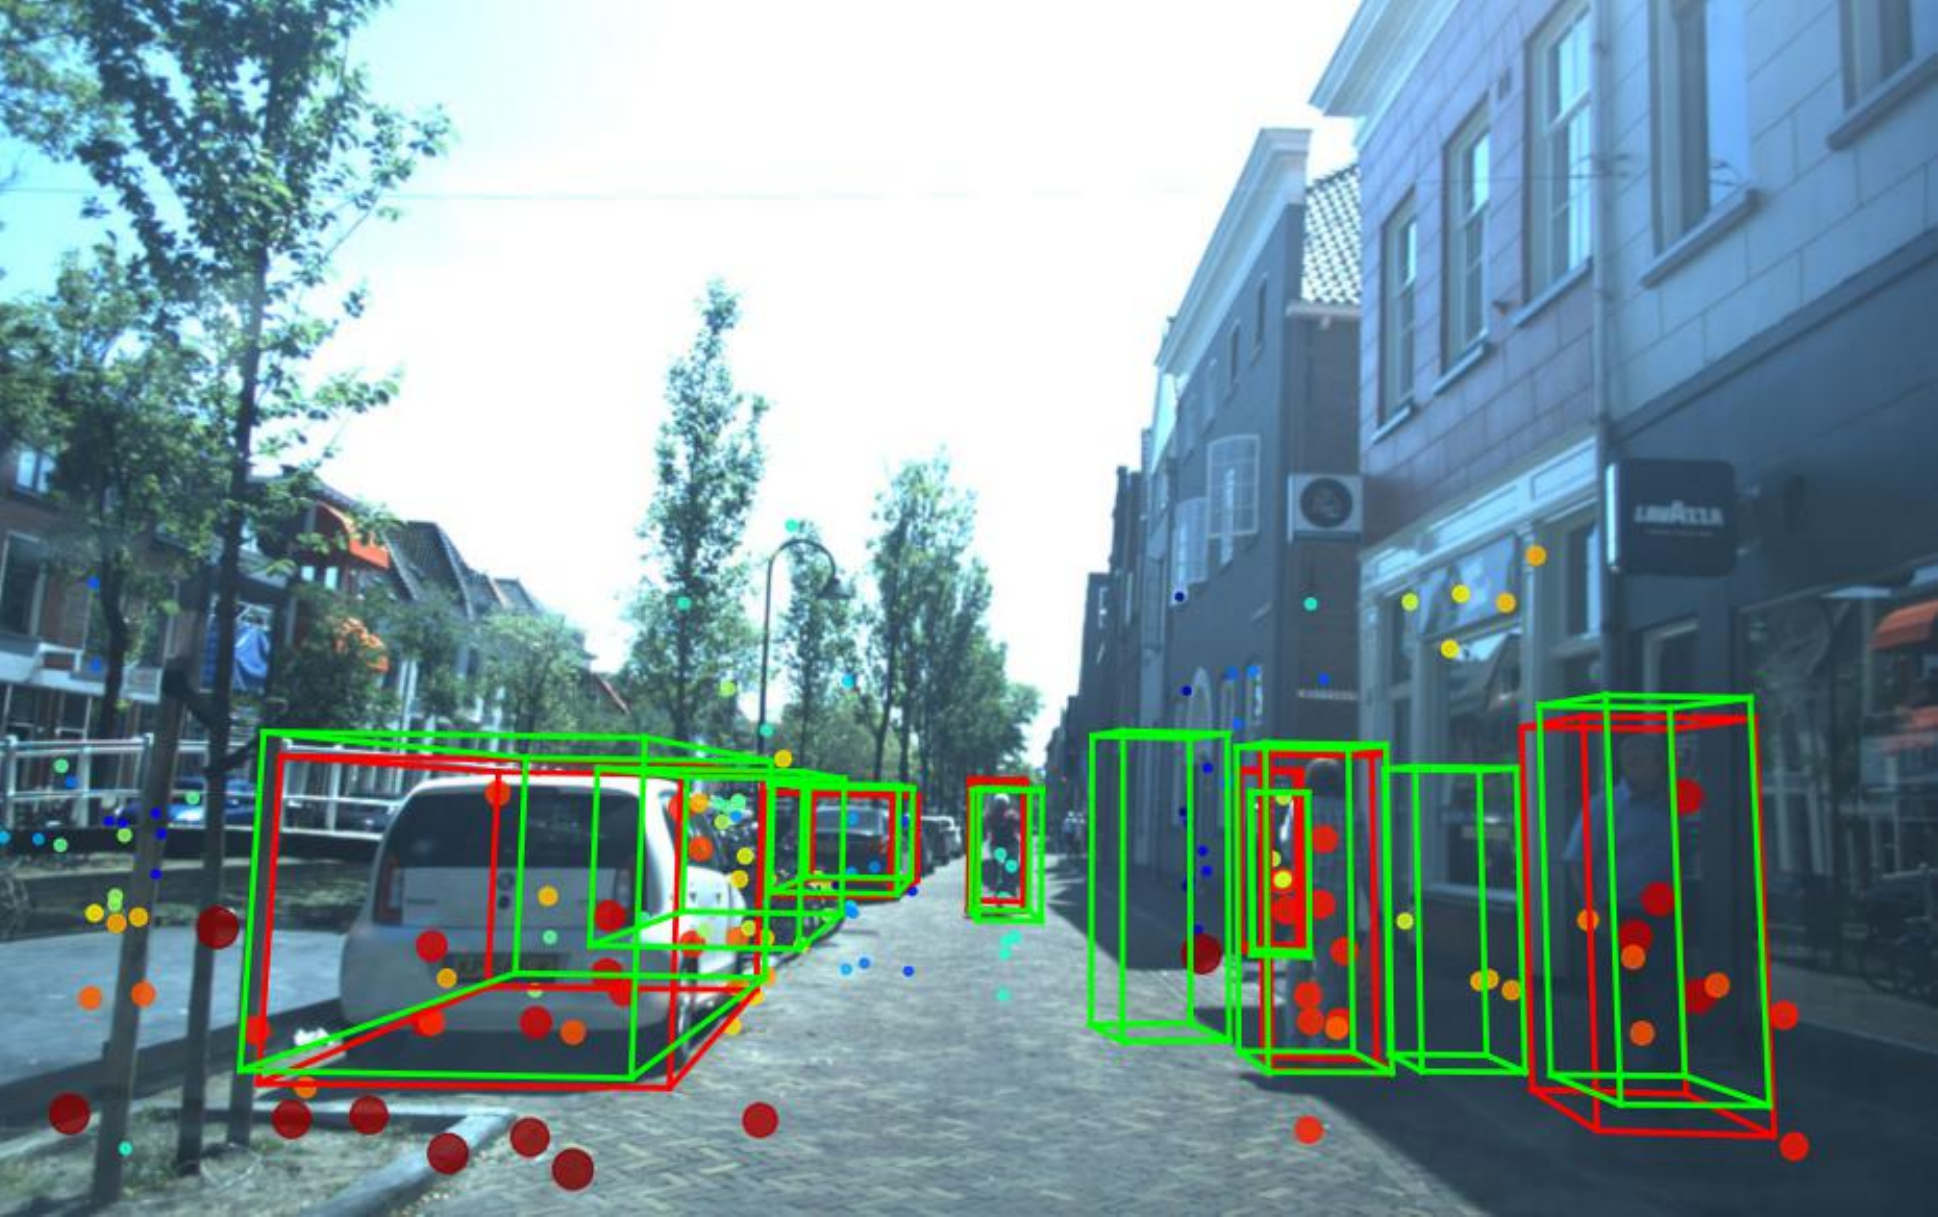}
        \end{subfigure}%
        \begin{subfigure}{\textwidth}
            \centering
            \includegraphics[width=\textwidth]{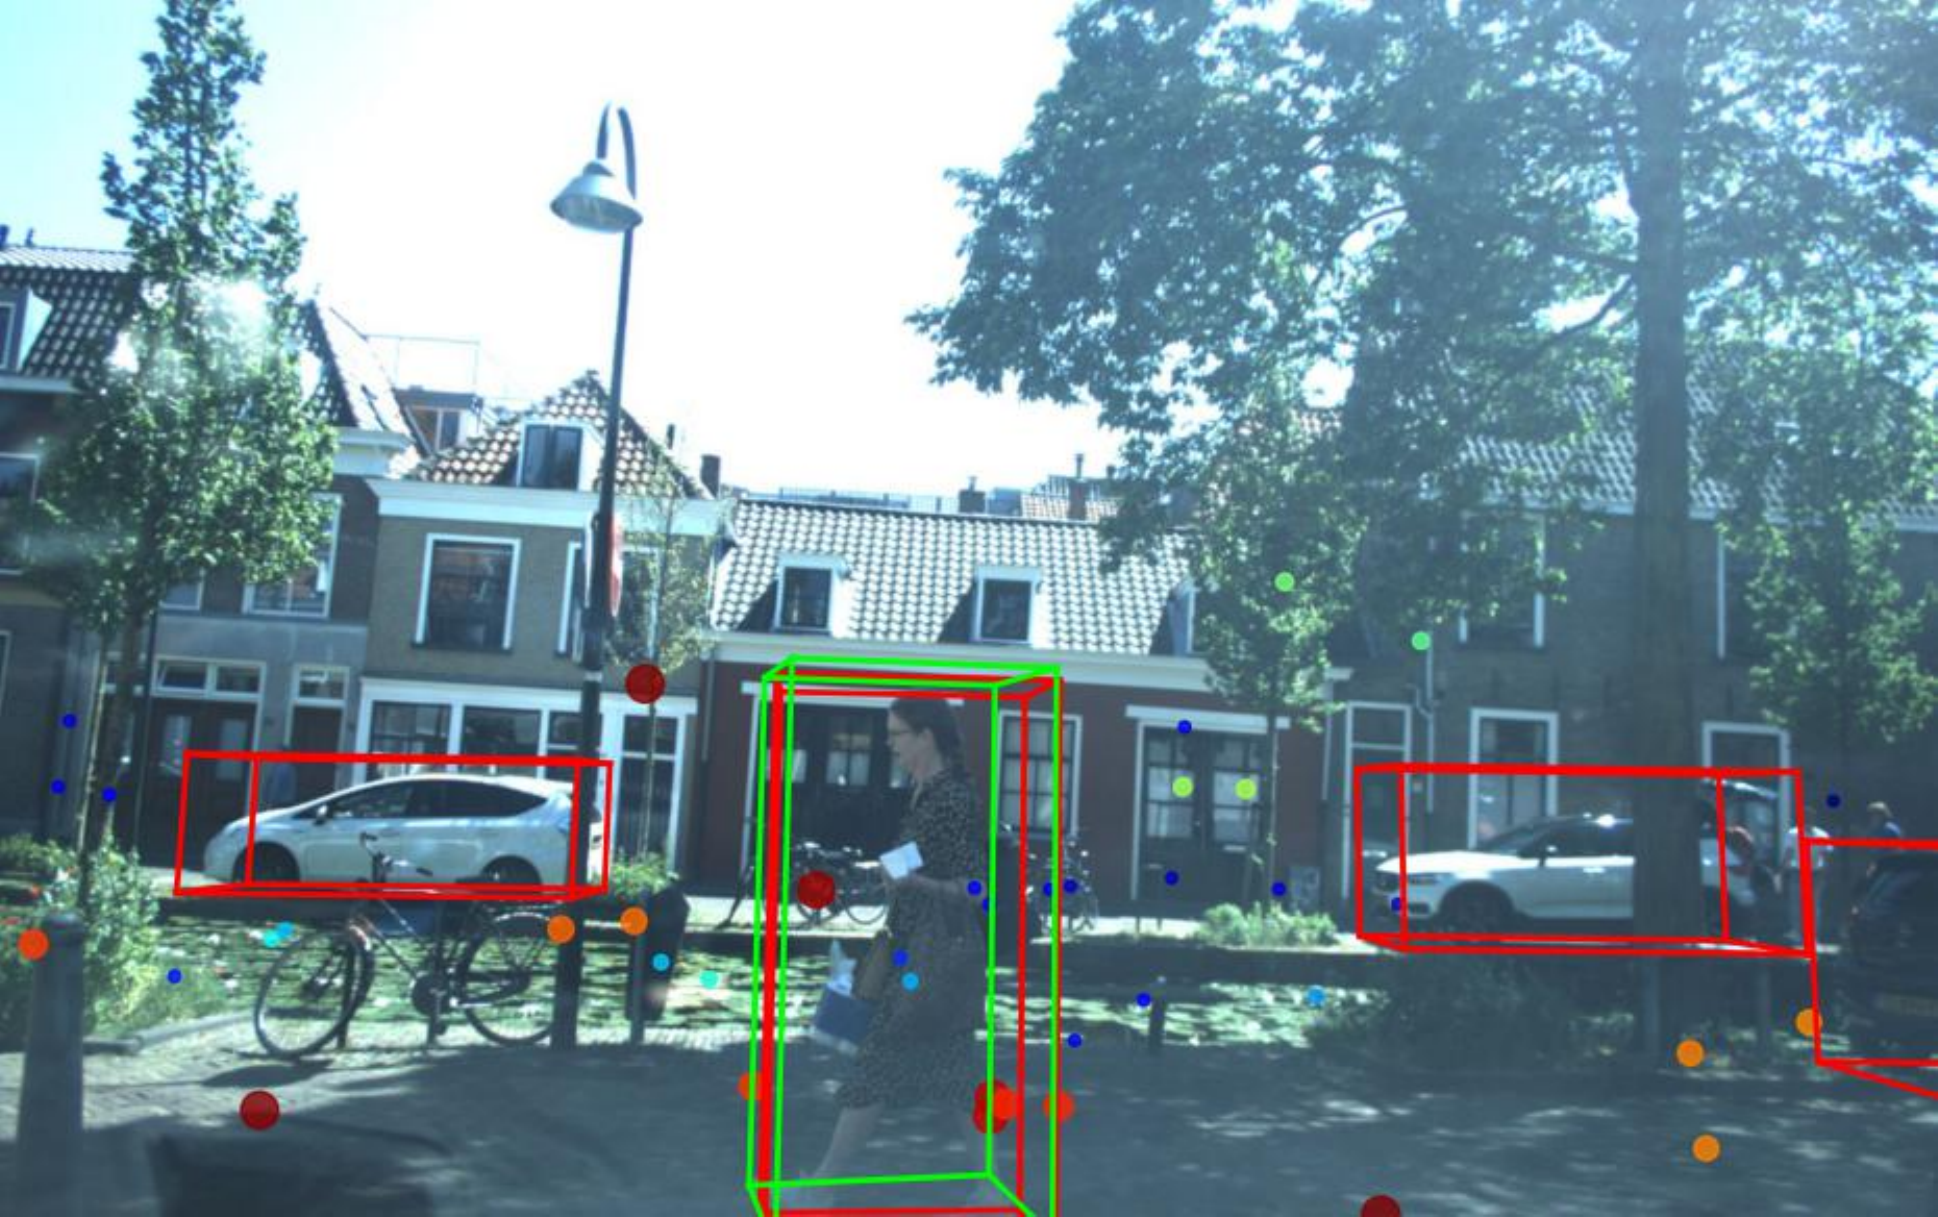}
        \end{subfigure}%
        \begin{subfigure}{\textwidth}
            \centering
            \includegraphics[width=\textwidth]{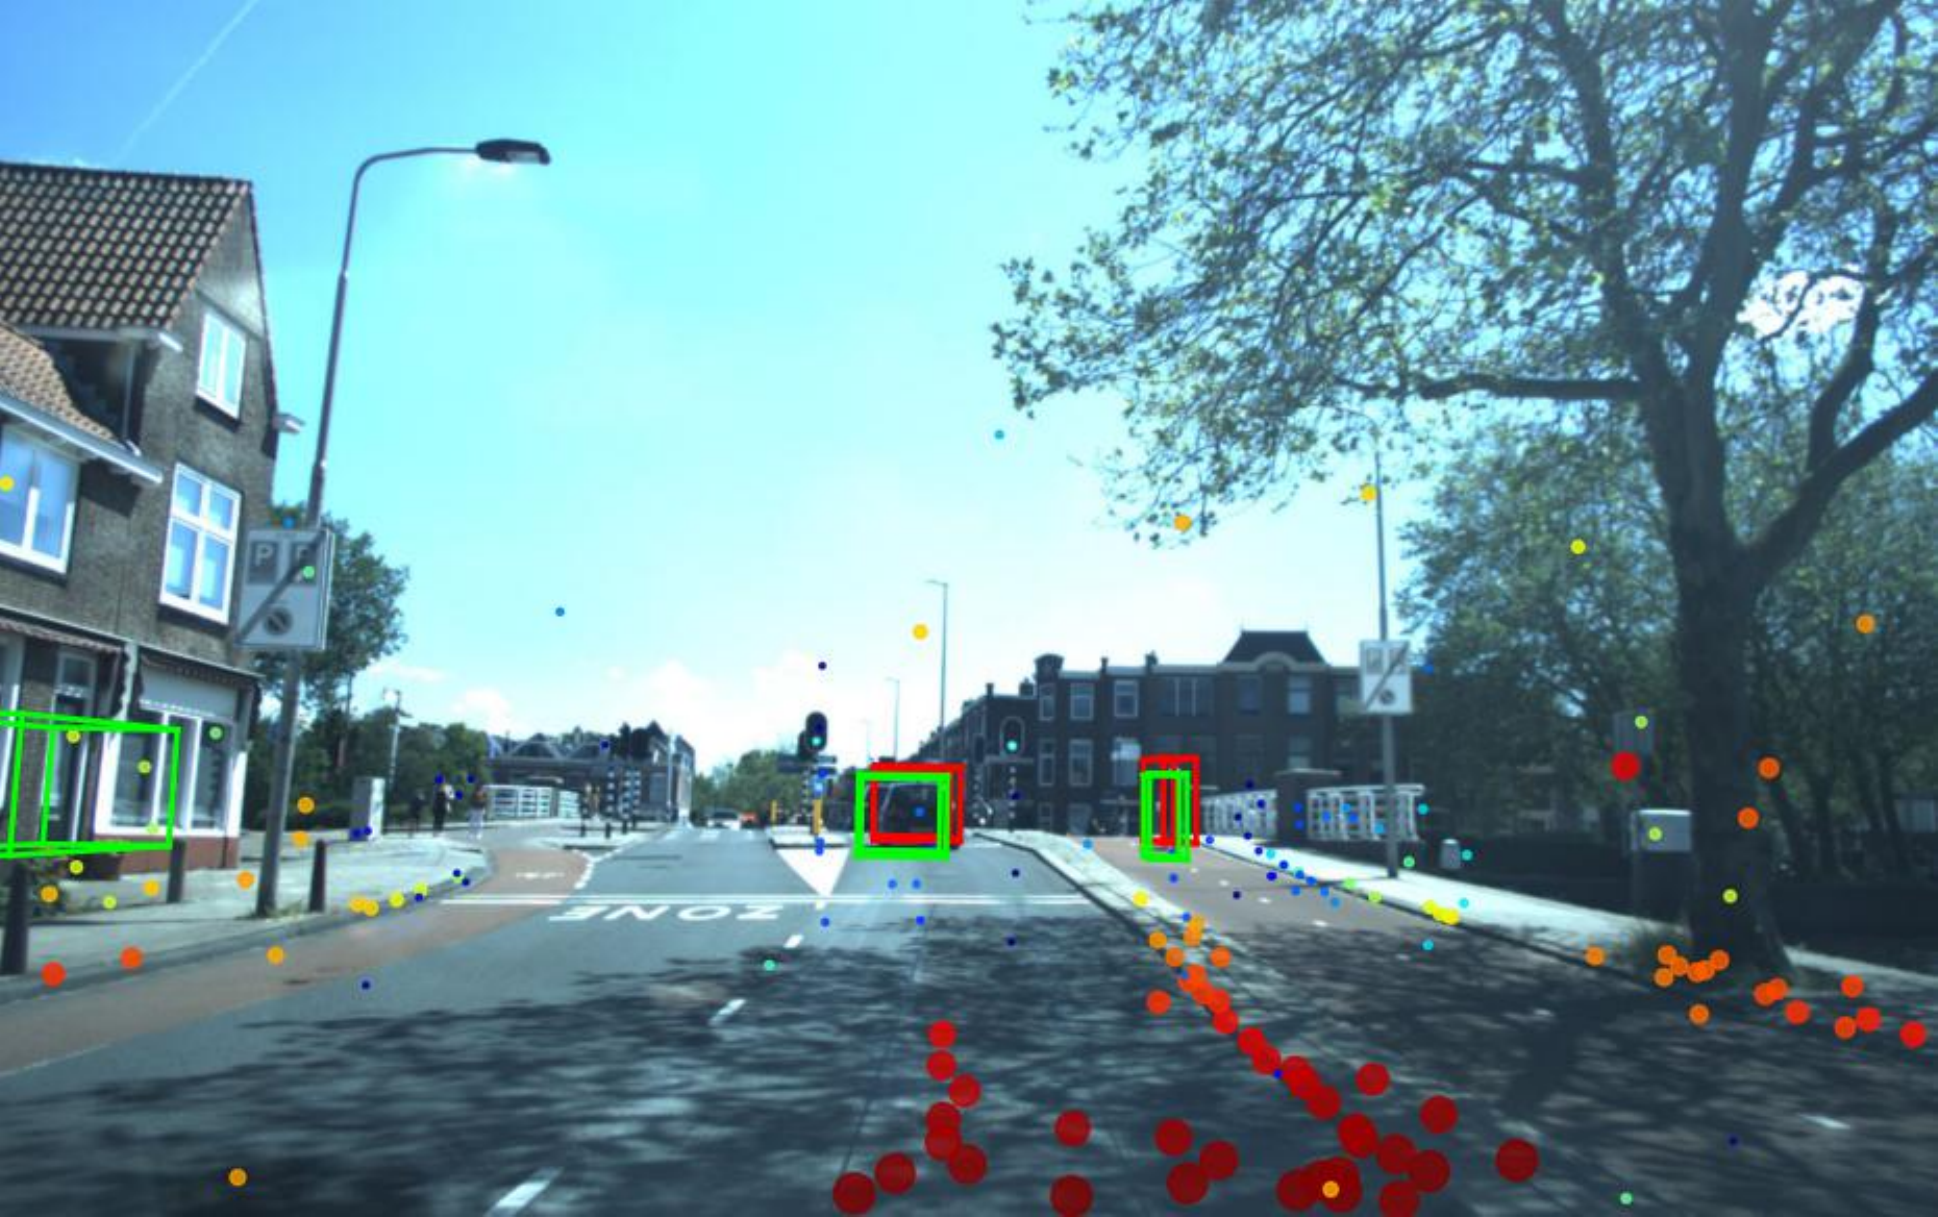}
        \end{subfigure}%
        \begin{subfigure}{\textwidth}
            \centering
            \includegraphics[width=\textwidth]{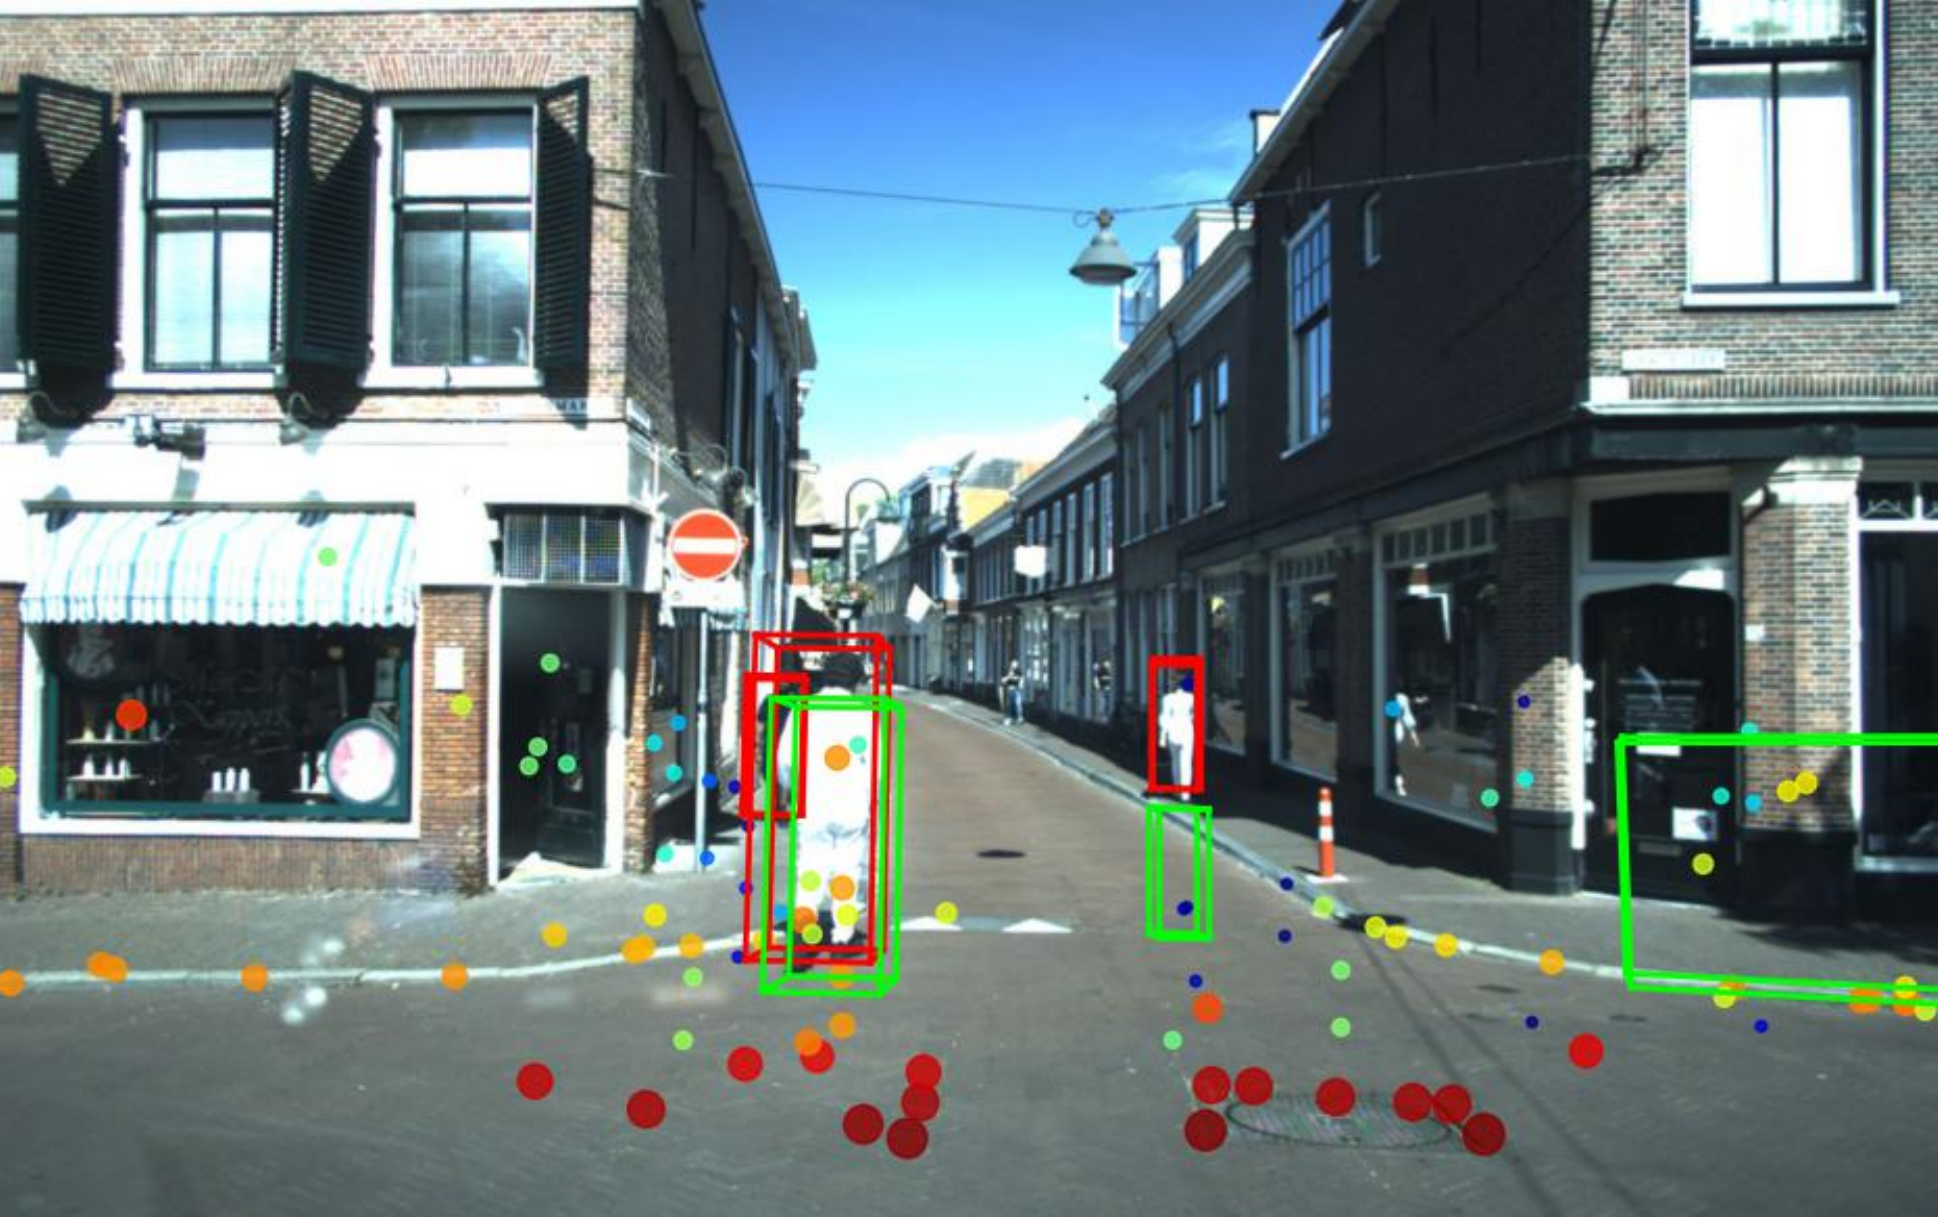}
        \end{subfigure}%
    \end{minipage}\\
    \caption{Radar qualitative evaluation. Predictions by different methods are shown in \textcolor{green}{green} while ground-truth bounding boxes are shown in \textcolor{red}{red}}. \hant{we needs think new colour for radar point cloud?}
\end{figure*}

\newpage
\begin{figure*}[ht!]
    \centering
    \begin{minipage}{0.32\textwidth}
        \centering
        \begin{subfigure}{\textwidth}
            \centering
            \includegraphics[width=\textwidth]{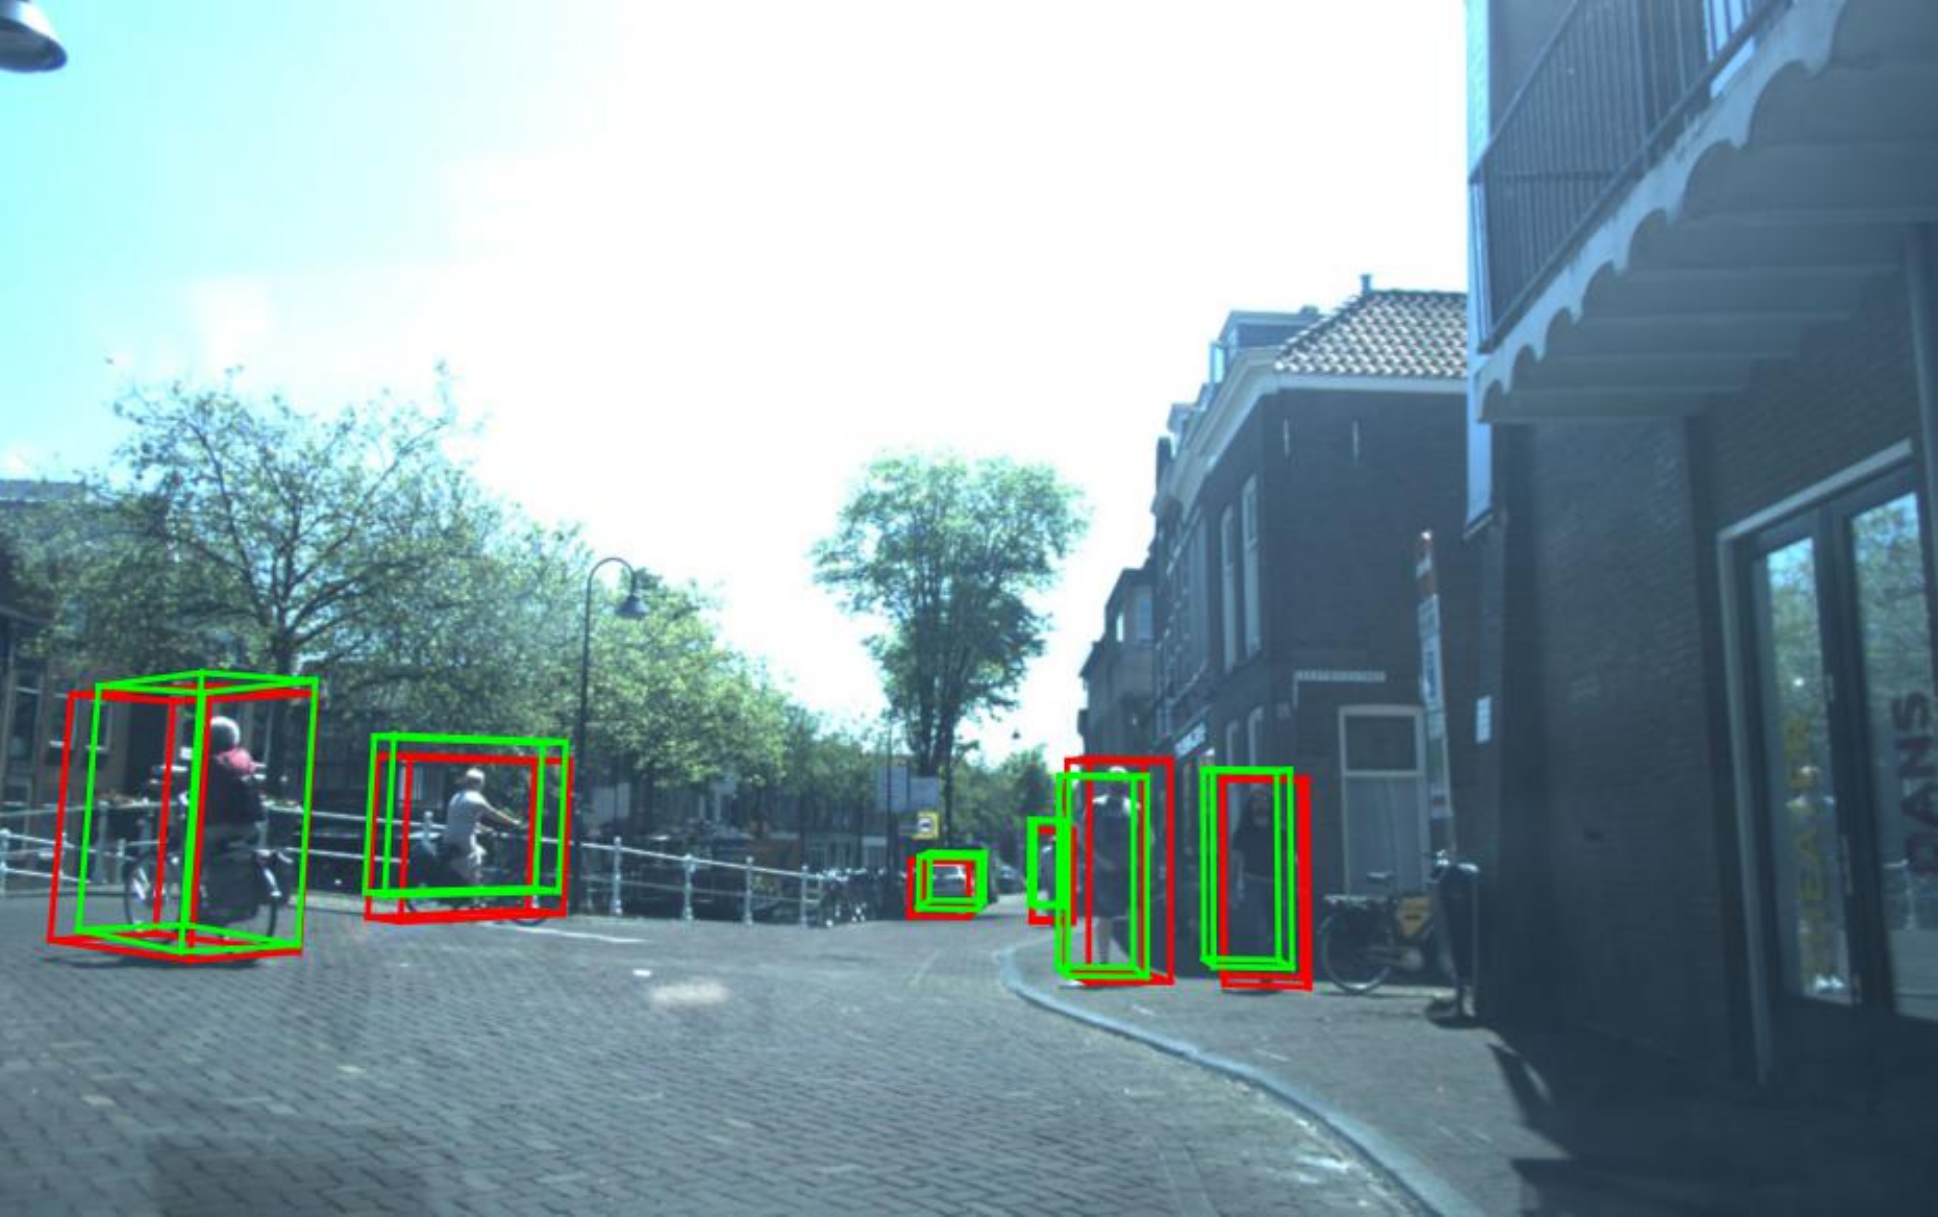}
        \end{subfigure}
        \begin{subfigure}{\textwidth}
            \centering
            \includegraphics[width=\textwidth]{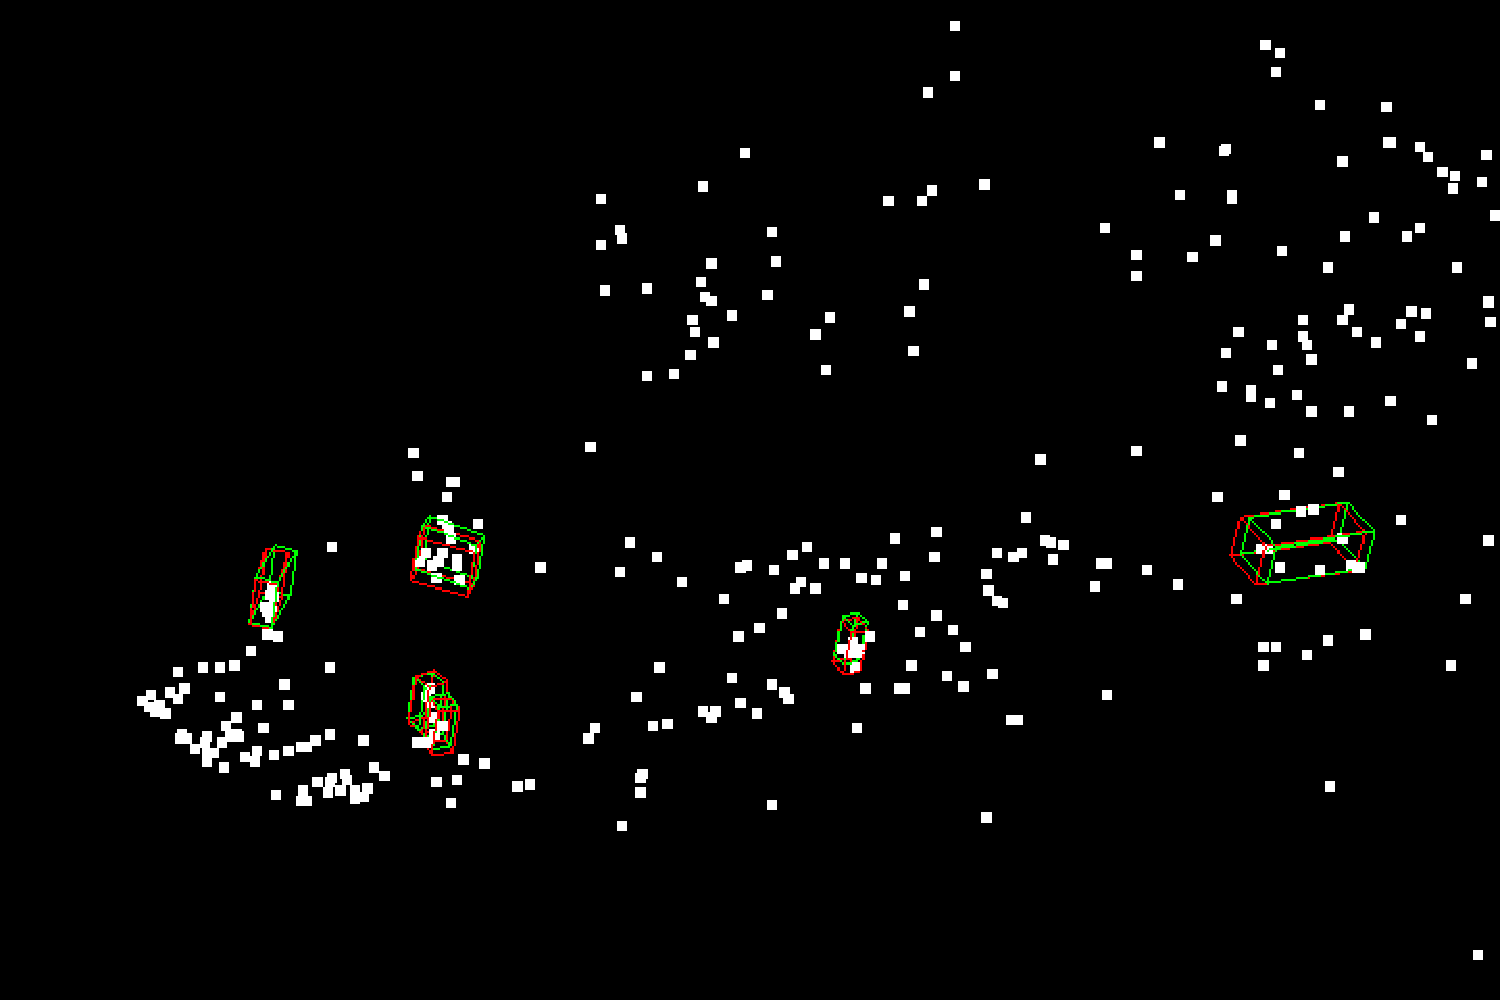}
        \end{subfigure}
        \begin{subfigure}{\textwidth}
            \centering
            \includegraphics[width=\textwidth]{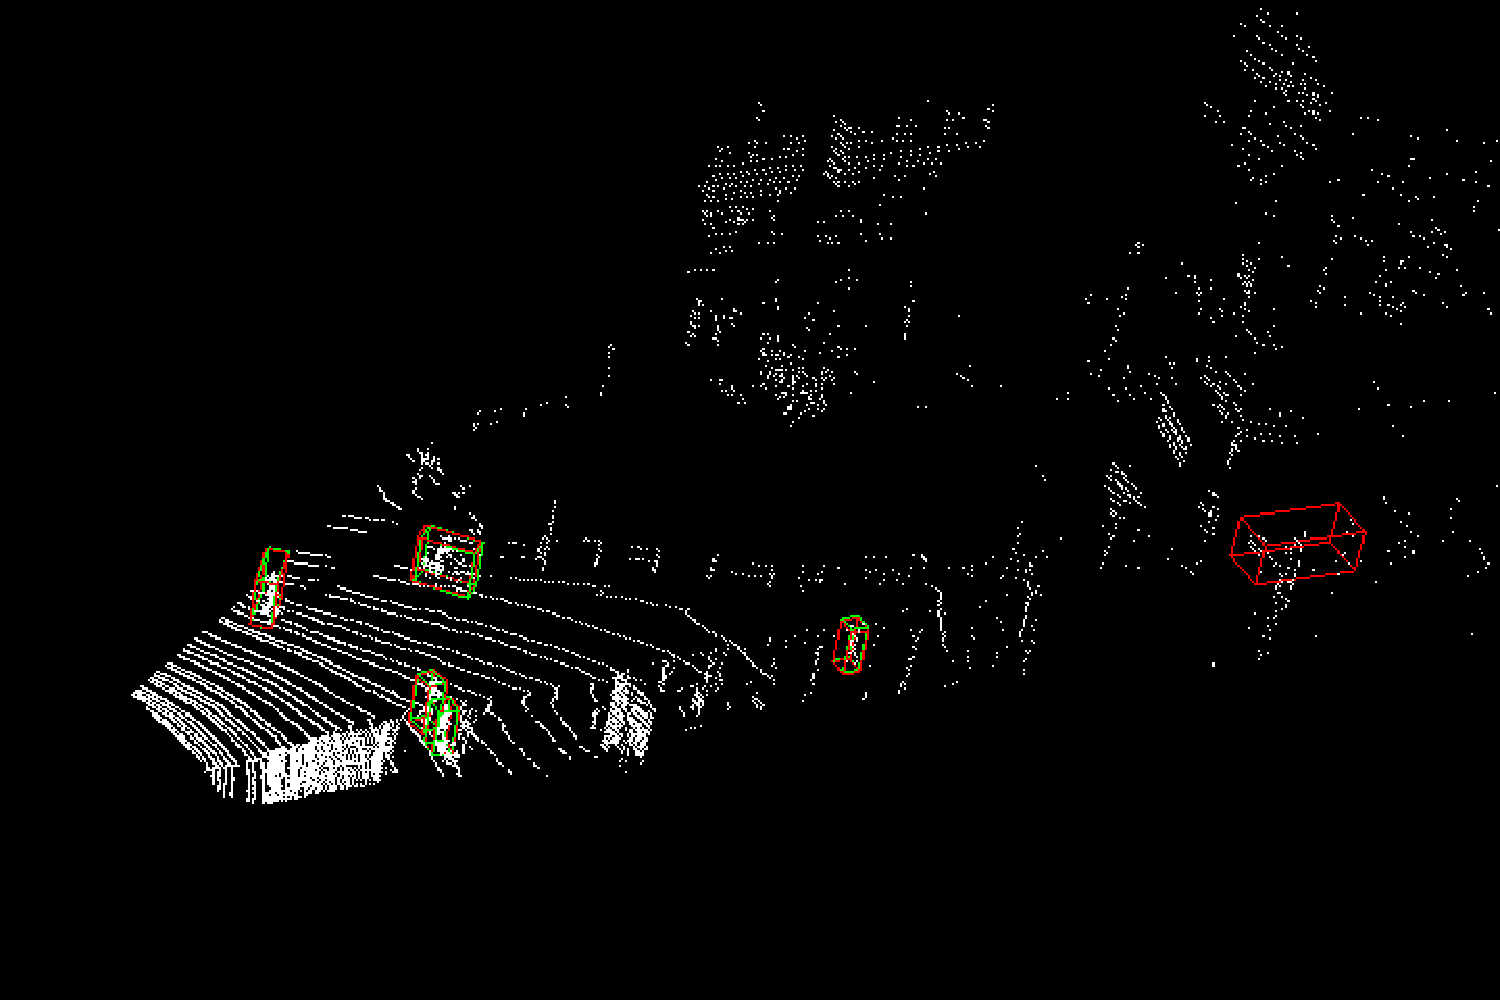}
        \end{subfigure} 
    \end{minipage}
    \begin{minipage}{0.32\textwidth}
        \centering
        \begin{subfigure}{\textwidth}
            \centering
            \includegraphics[width=\textwidth]{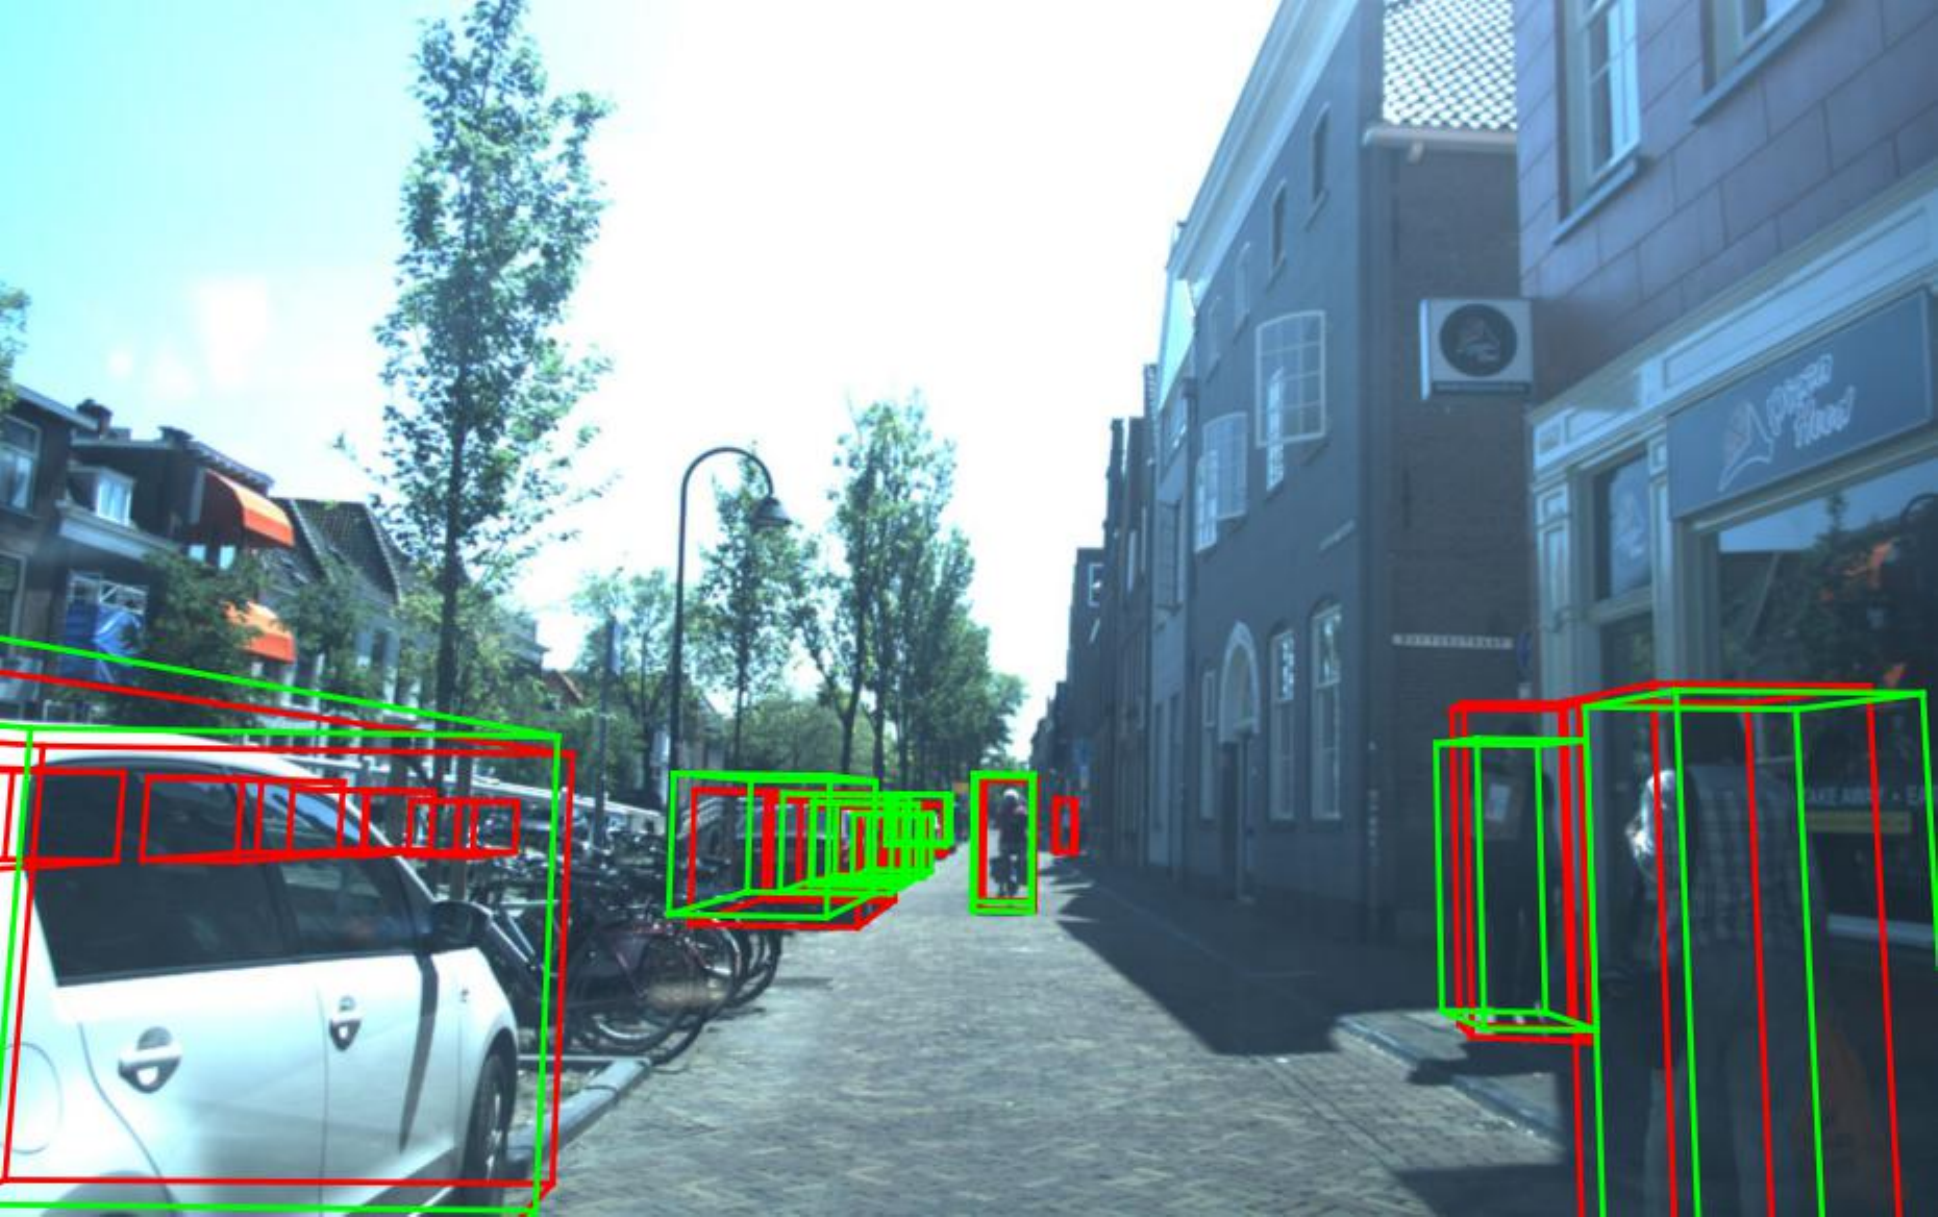}
        \end{subfigure}
        \begin{subfigure}{\textwidth}
            \centering
            \includegraphics[width=\textwidth]{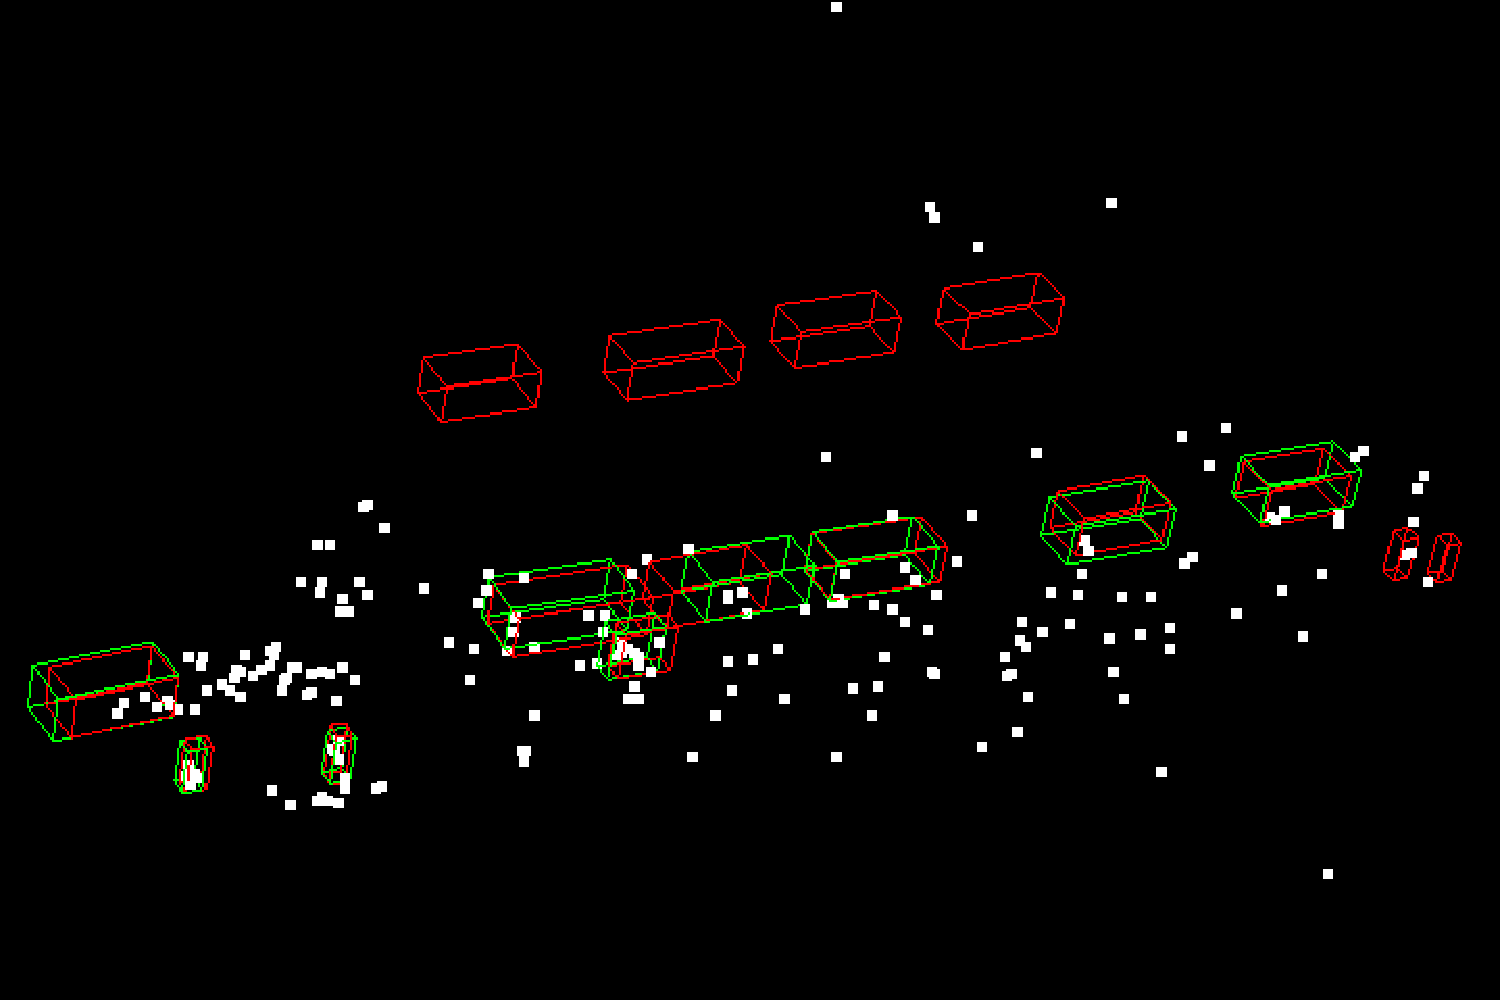}
        \end{subfigure}
        \begin{subfigure}{\textwidth}
            \centering
            \includegraphics[width=\textwidth]{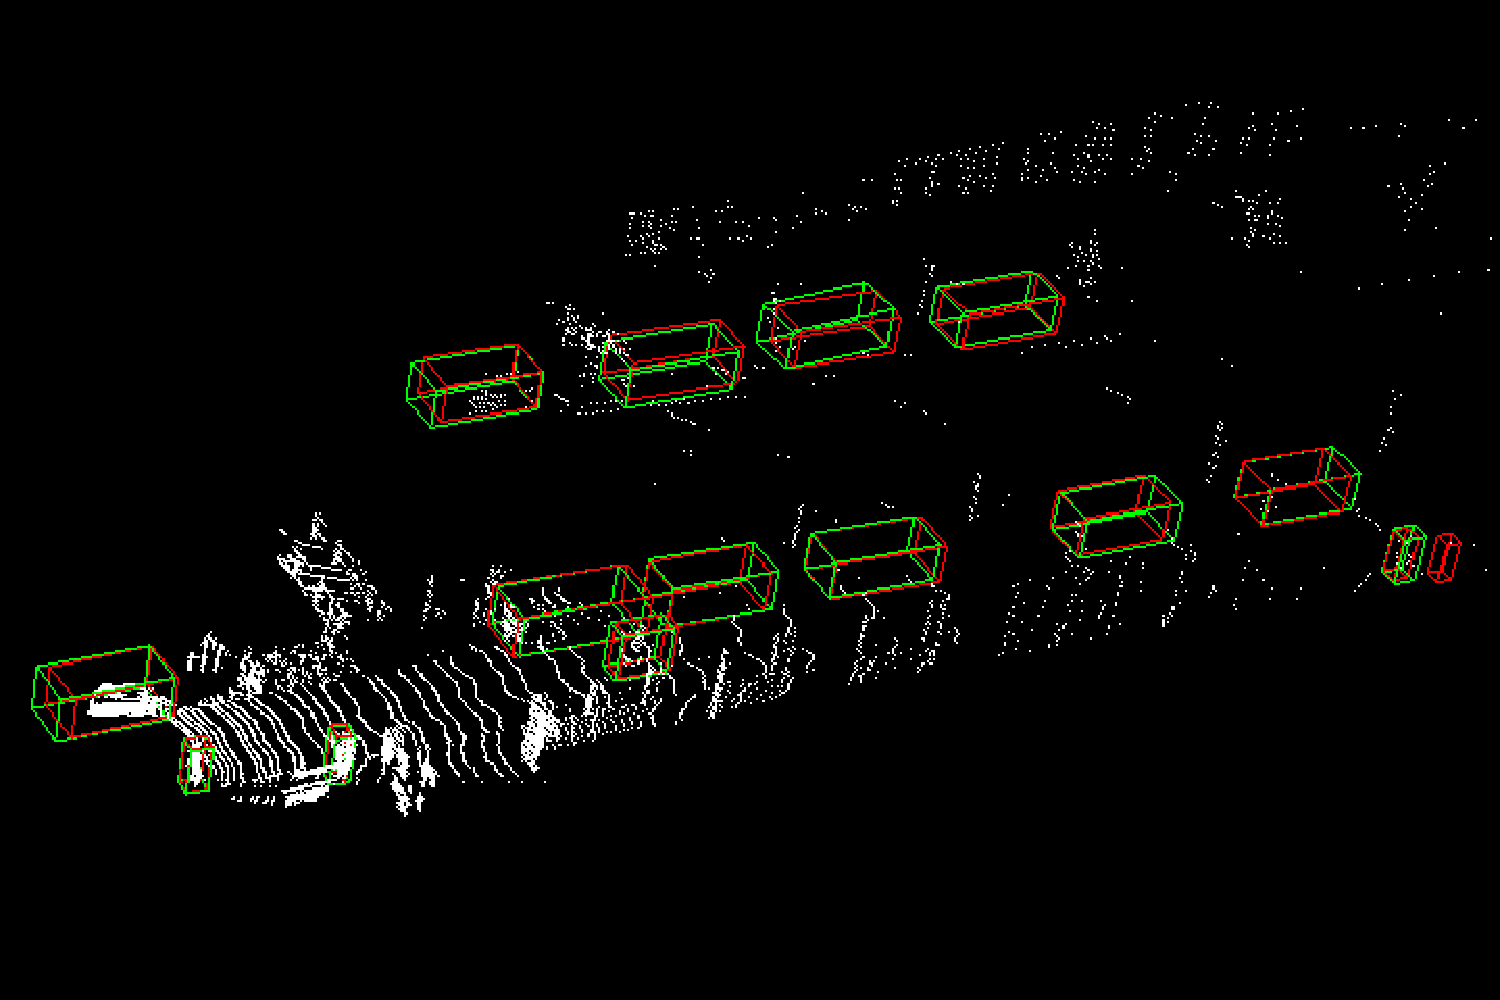}
        \end{subfigure} 
    \end{minipage}
    \begin{minipage}{0.32\textwidth}
        \centering
        \begin{subfigure}{\textwidth}
            \centering
            \includegraphics[width=\textwidth]{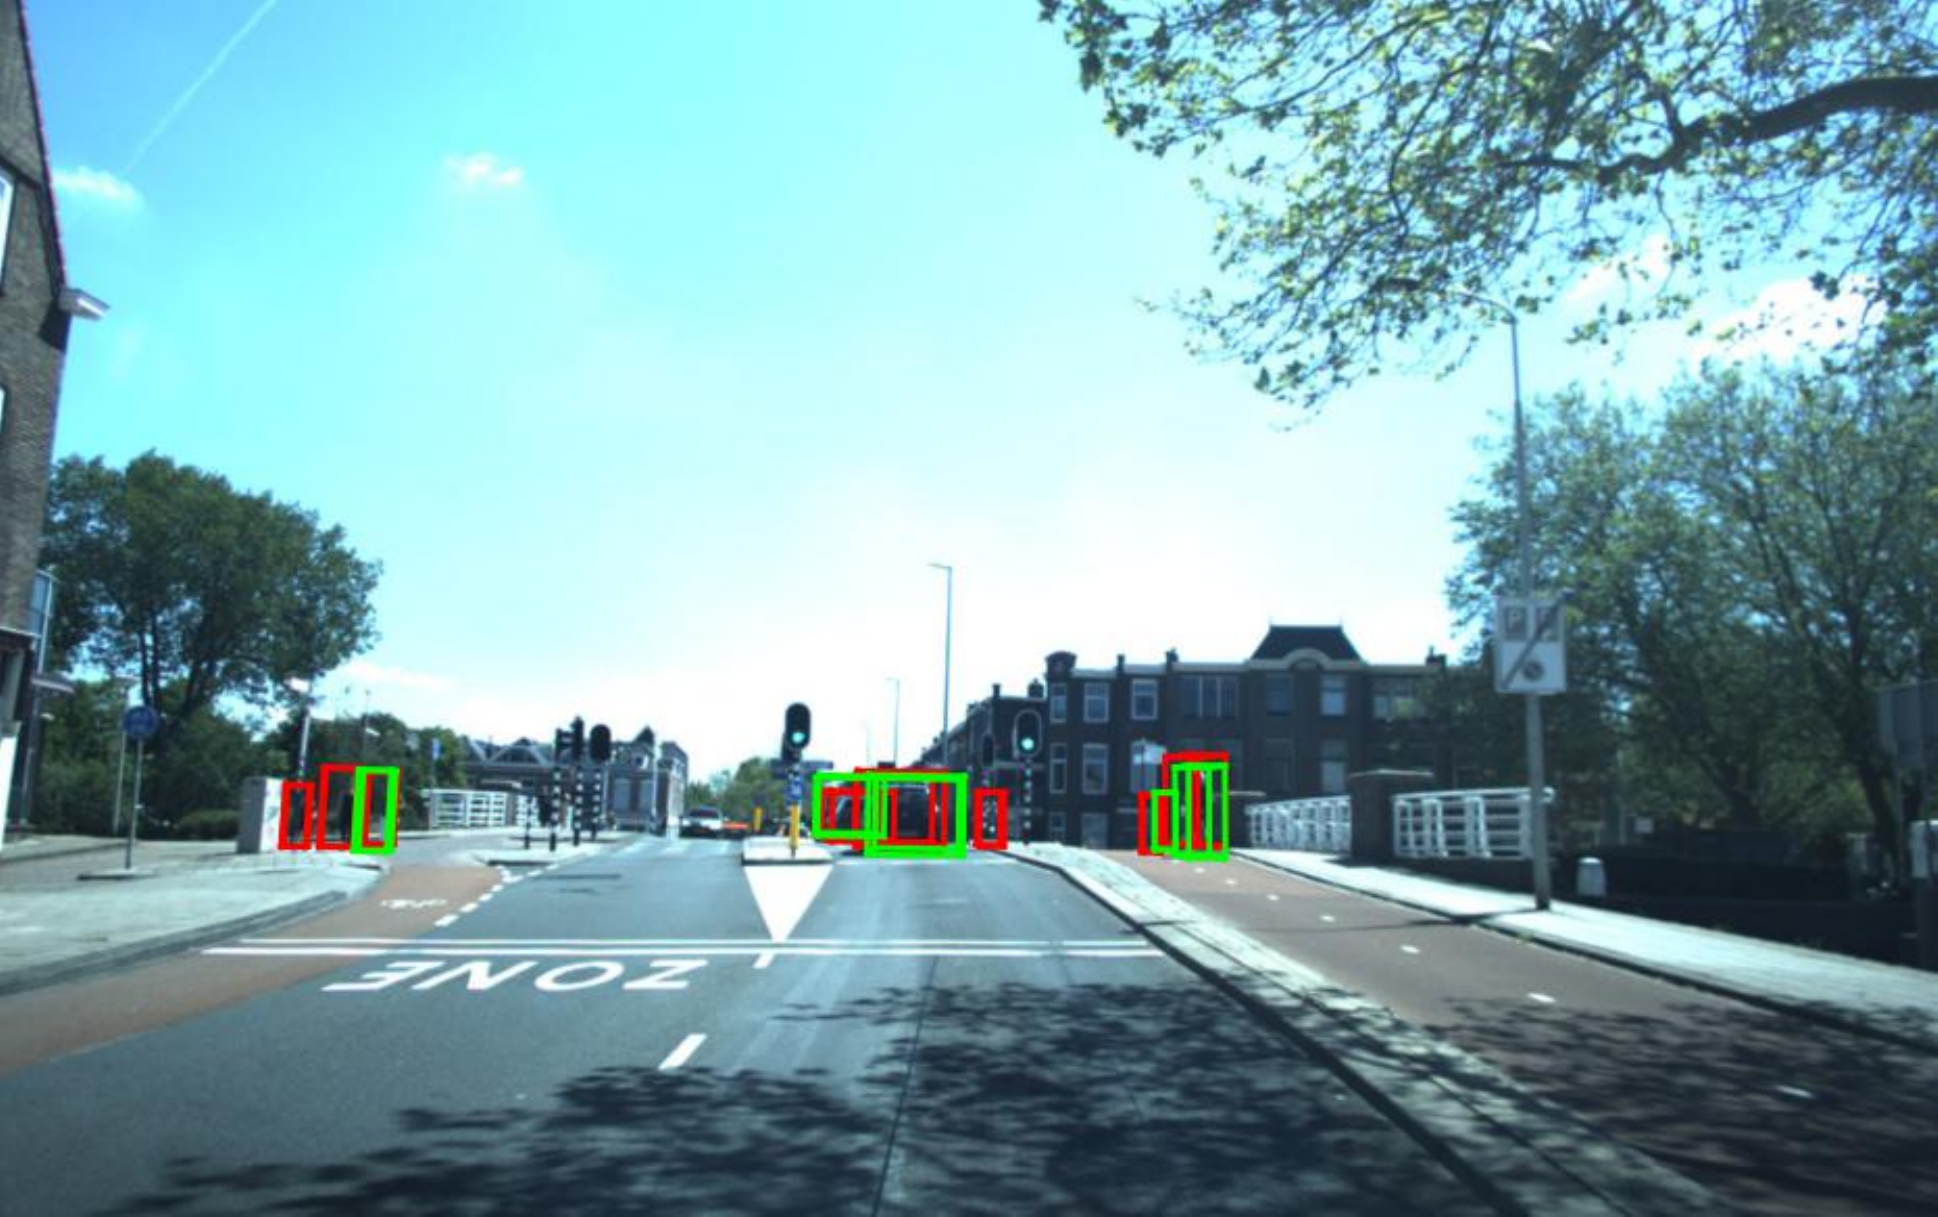}
        \end{subfigure}
        \begin{subfigure}{\textwidth}
            \centering
            \includegraphics[width=\textwidth]{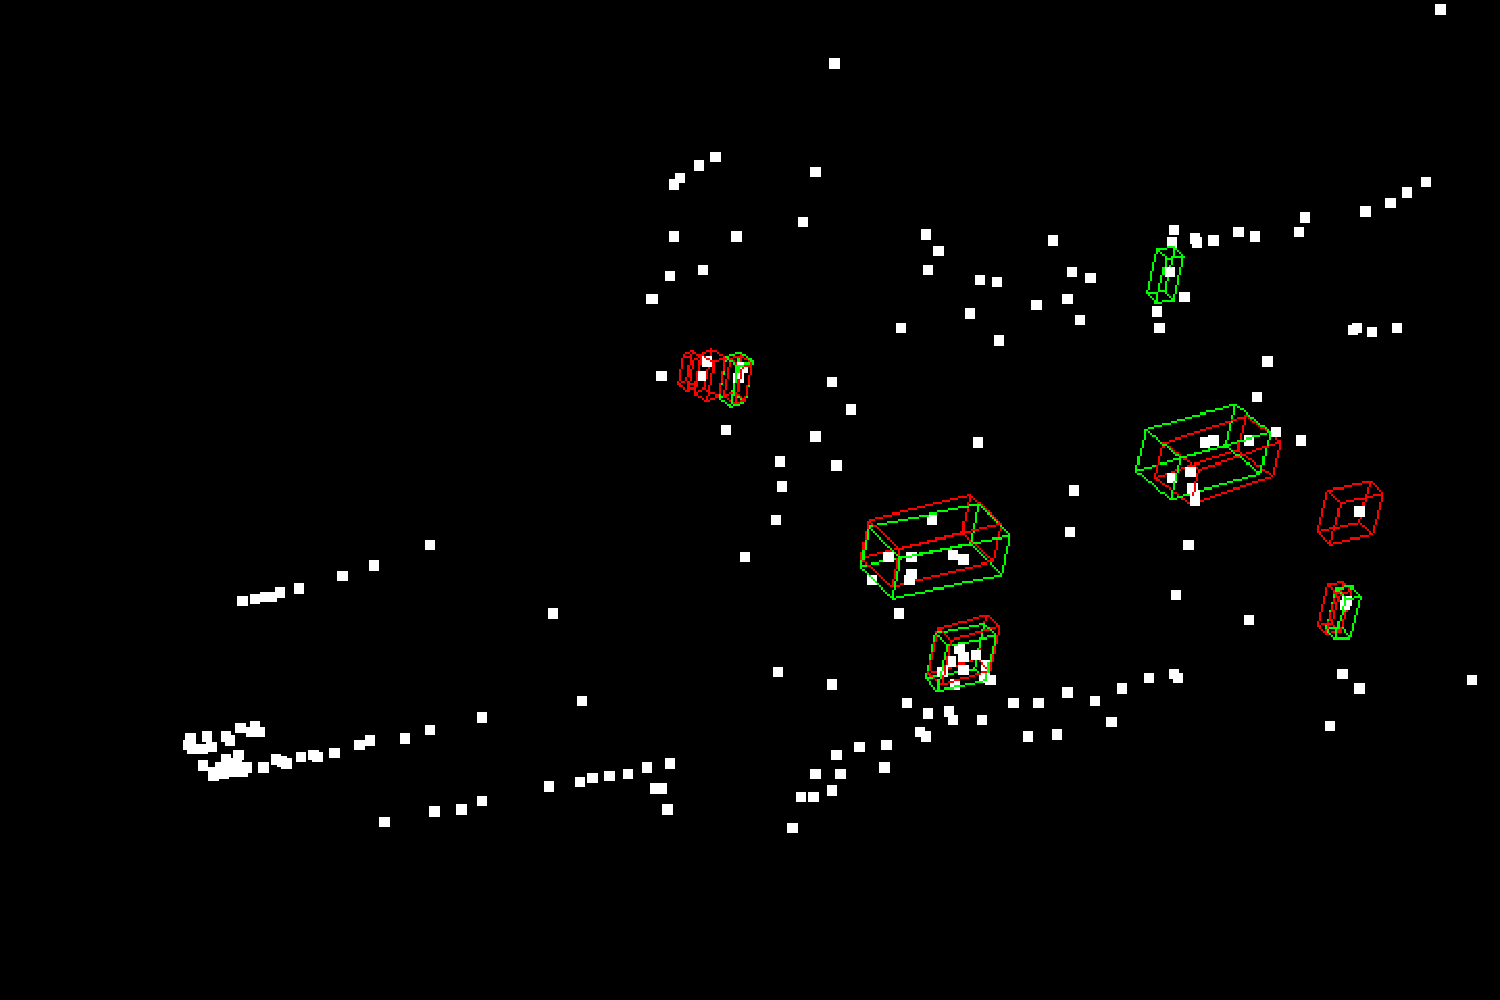}
        \end{subfigure}
        \begin{subfigure}{\textwidth}
            \centering
            \includegraphics[width=\textwidth]{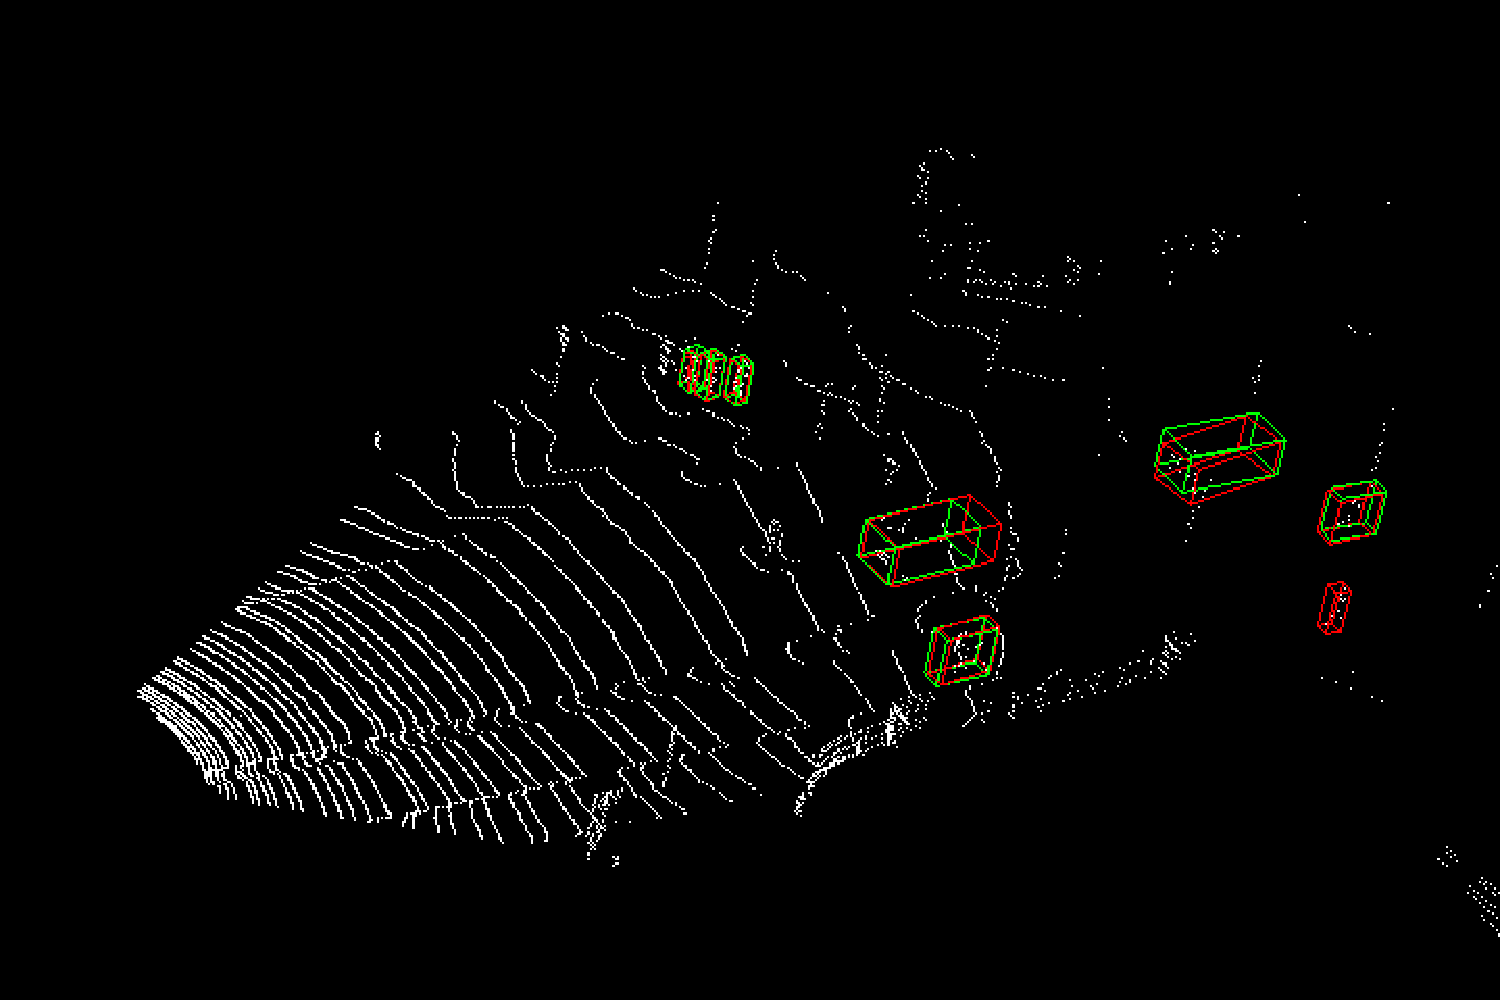}
        \end{subfigure} 
    \end{minipage}

    \caption{Qualitative results on the validation split of VoD. Our predictions are shown in \textcolor{green}{green} while ground-truth bounding boxes are shown in \textcolor{red}{red}}.
\end{figure*}

\newpage
\begin{figure*}[ht!]
    \centering
        \begin{minipage}{.48\textwidth}
            \begin{subfigure}{\textwidth}
            \centering
            \includegraphics[width=\textwidth]{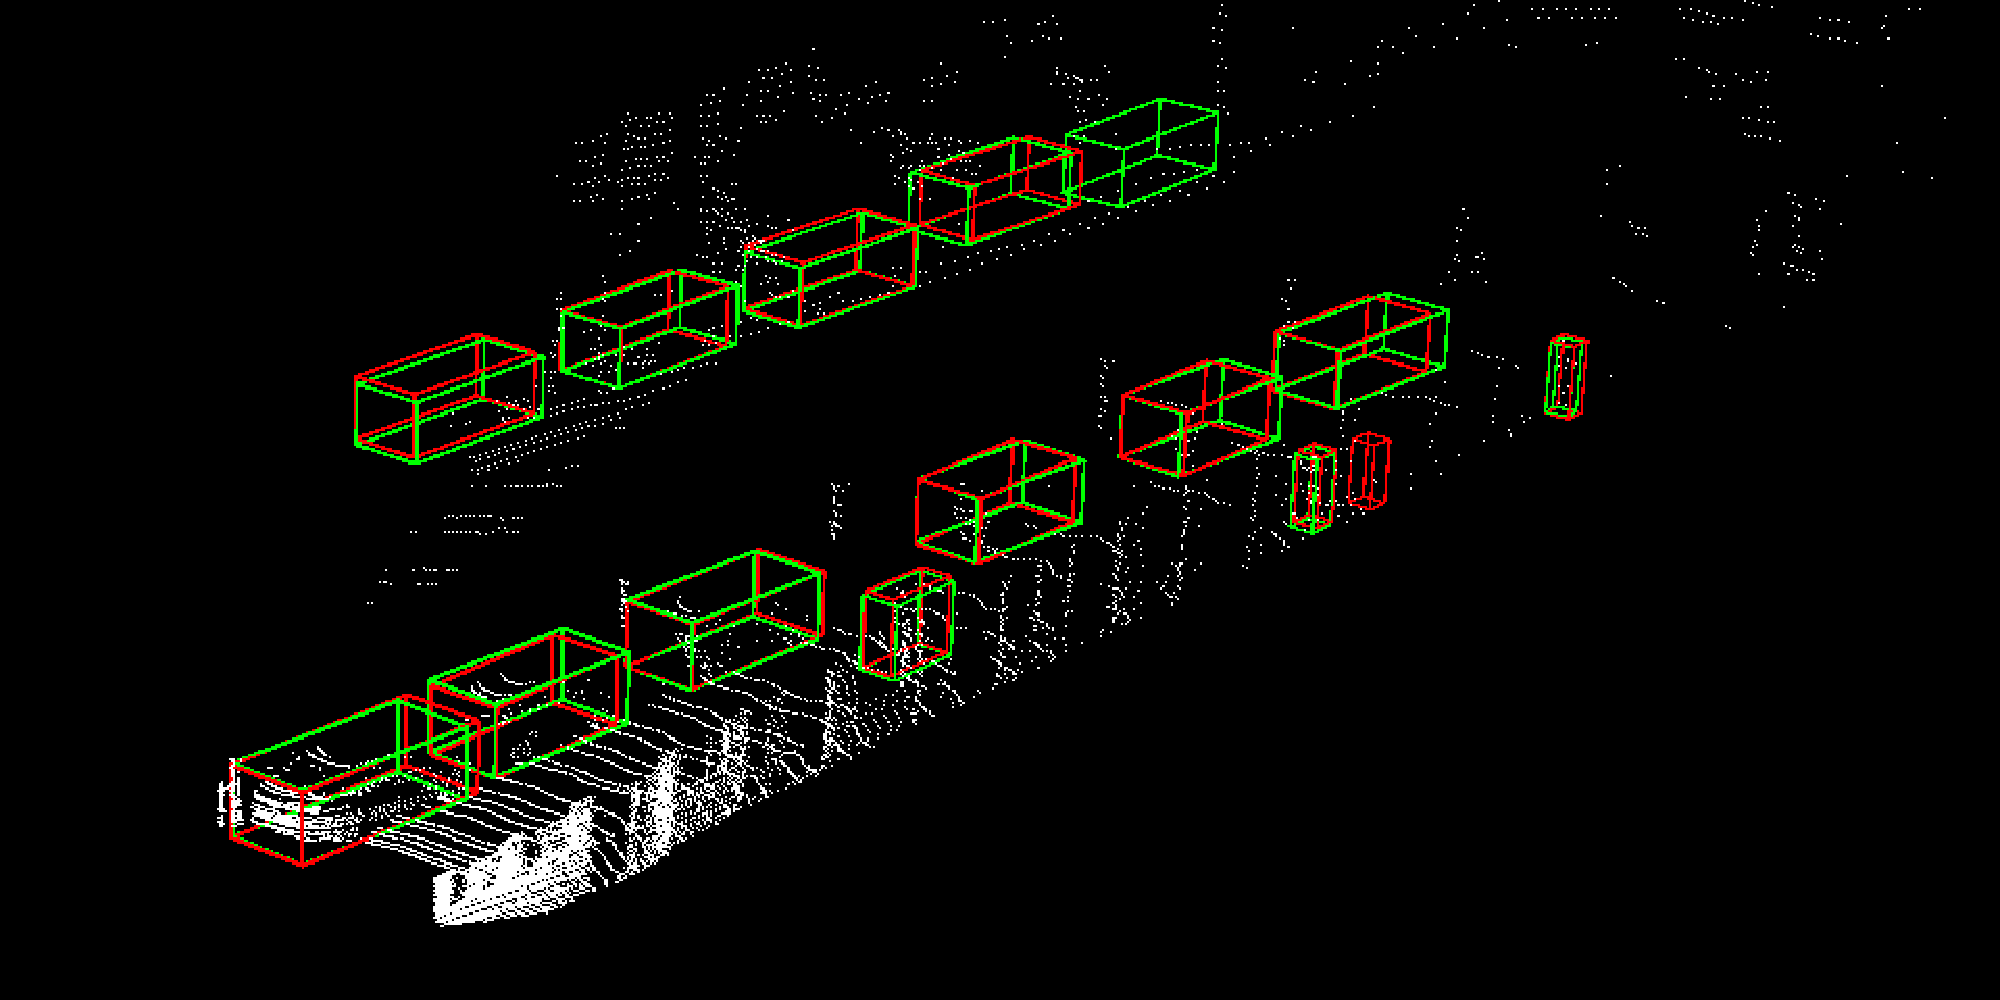}
            % \caption{00187}
            \end{subfigure}%  
        \end{minipage}
        \begin{minipage}{.48\textwidth}
            \begin{subfigure}{\textwidth}
            \centering
            \includegraphics[width=\textwidth]{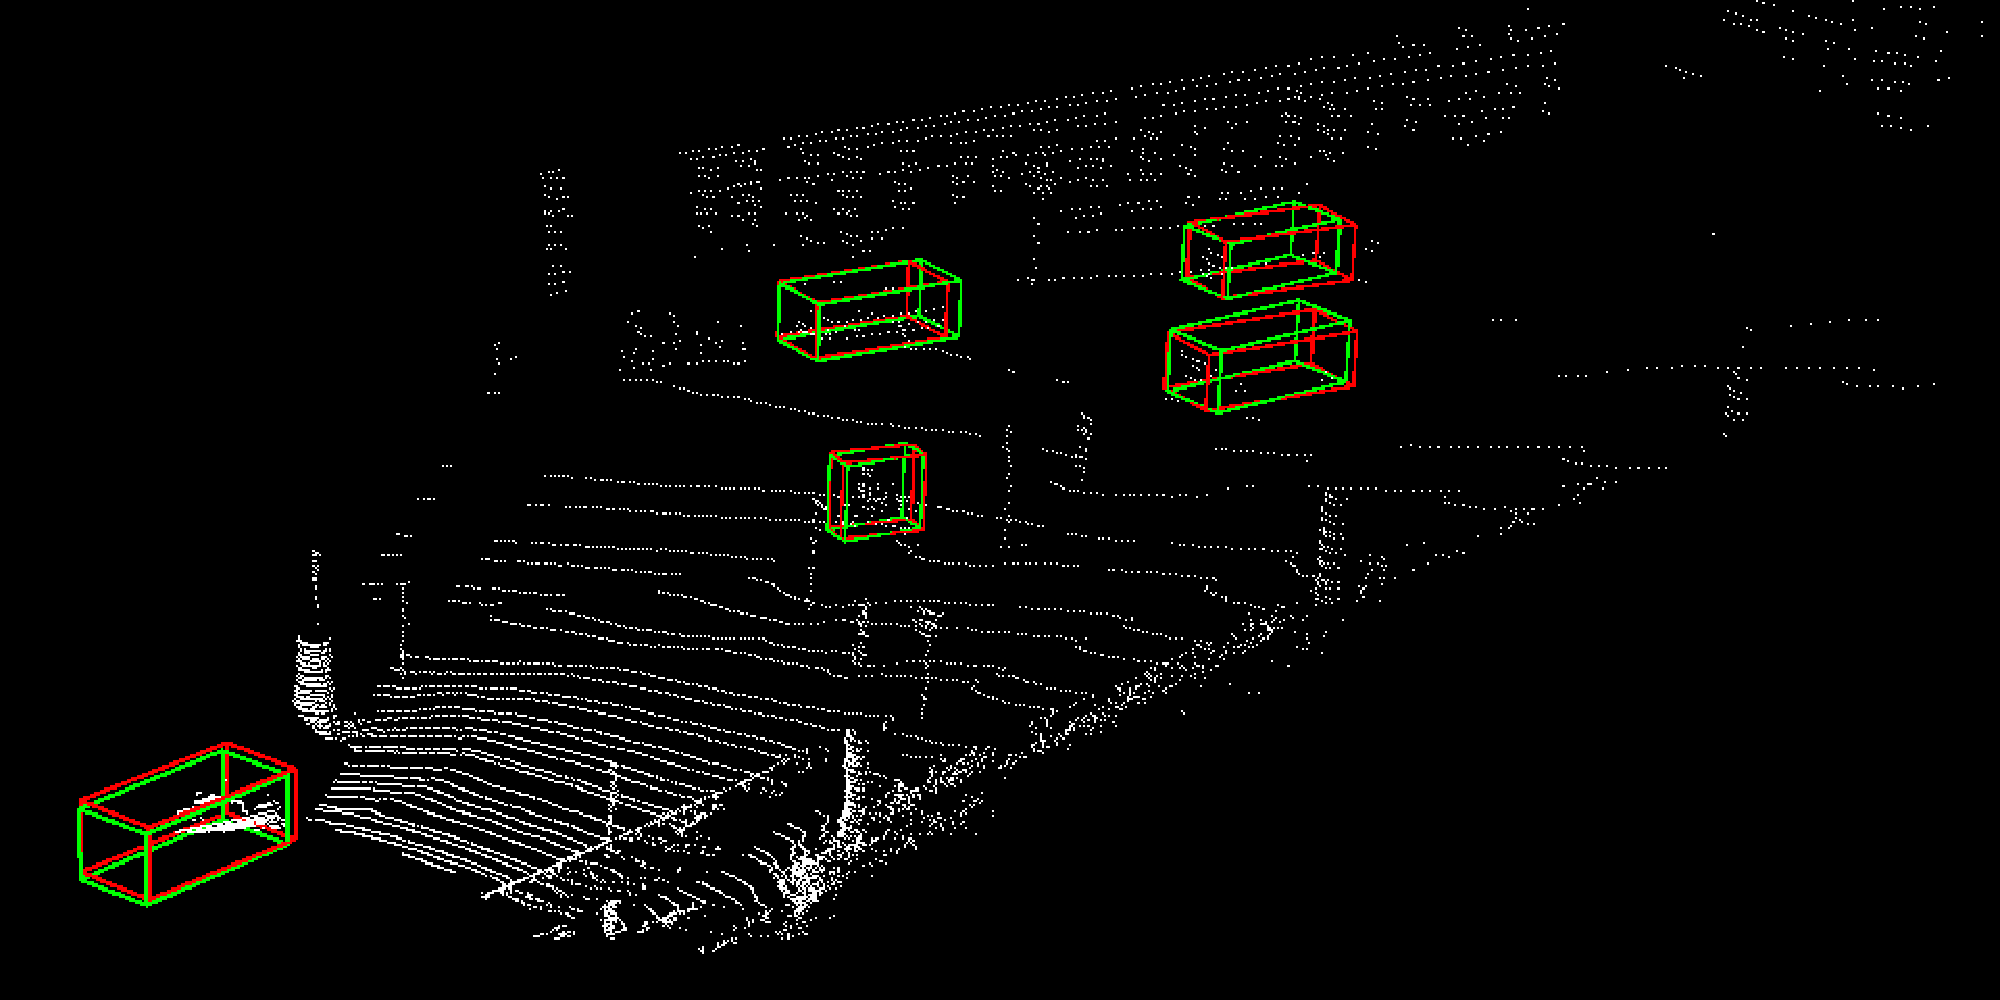}
            % \caption{04740}
            \end{subfigure}%  
        \end{minipage}
        \begin{minipage}{.48\textwidth}
            \begin{subfigure}{\textwidth}
            \centering
            \includegraphics[width=\textwidth]{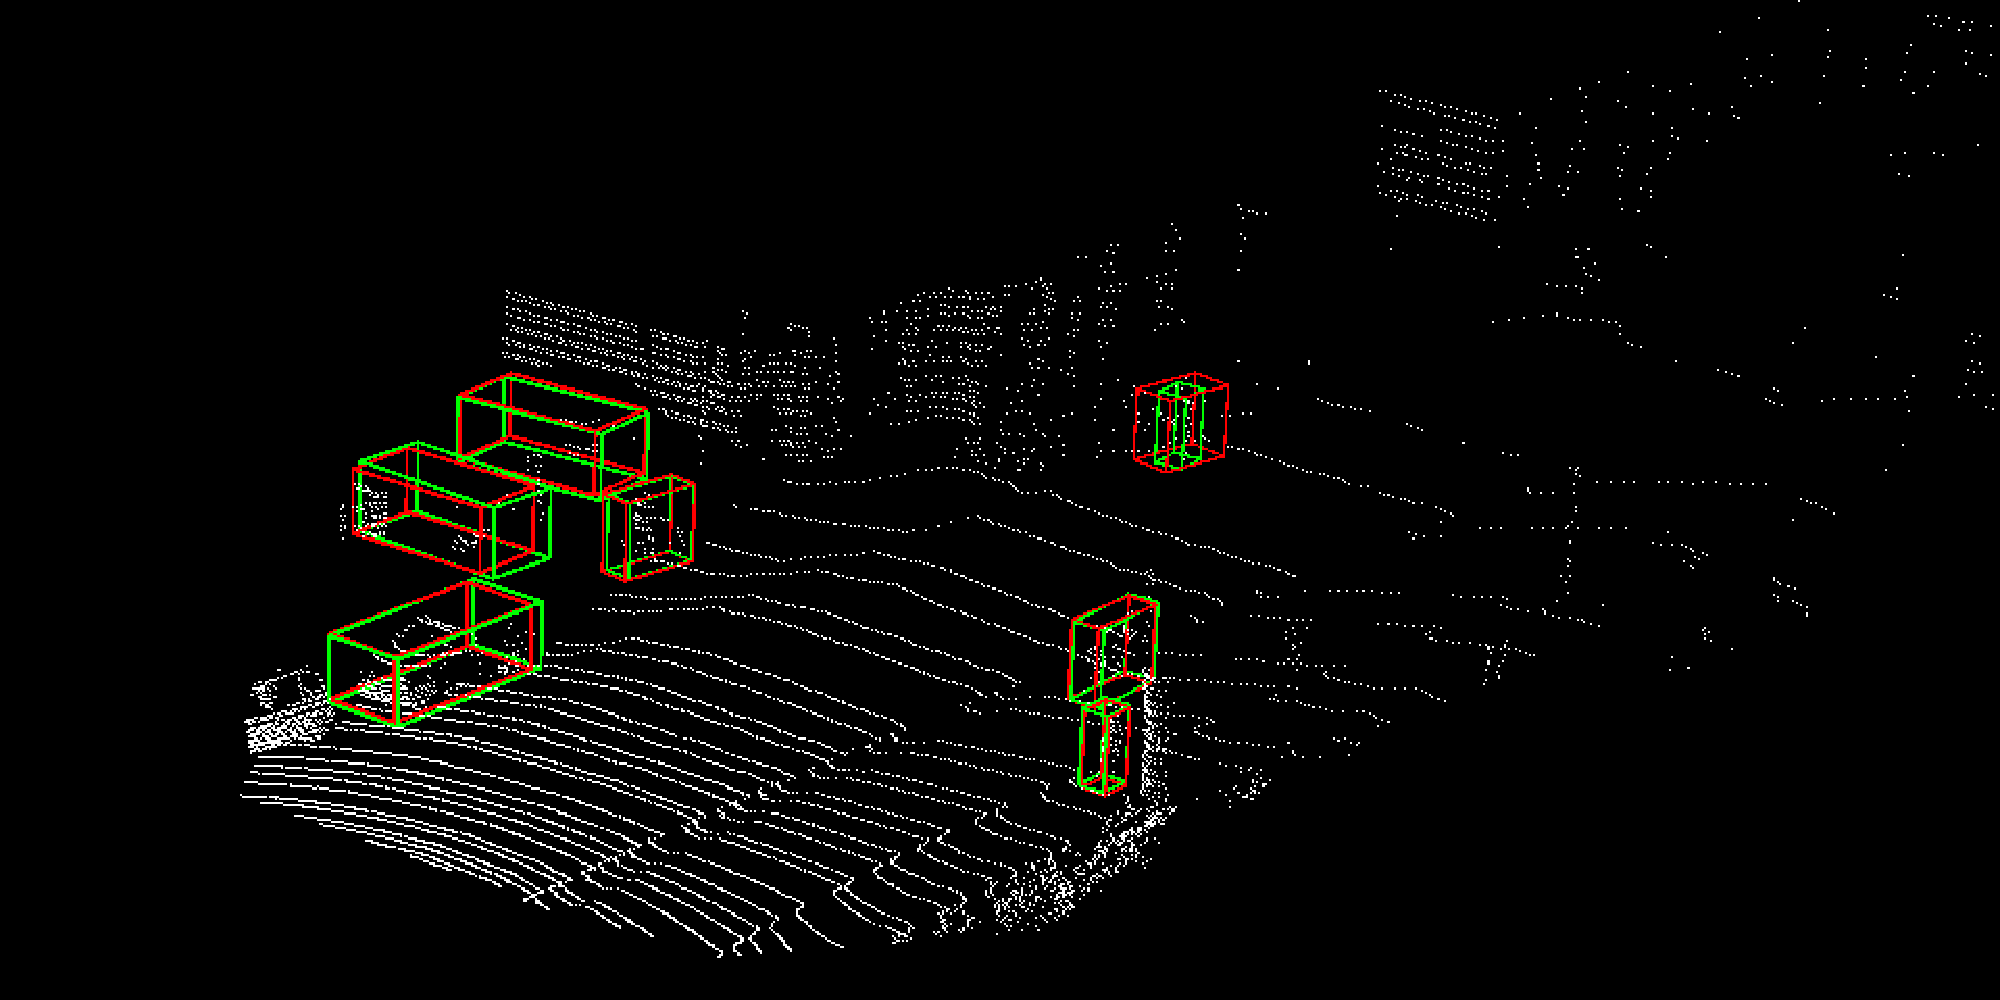}
            % \caption{08433}
            \end{subfigure}%  
        \end{minipage}
        \begin{minipage}{.48\textwidth}
            \begin{subfigure}{\textwidth}
            \centering
            \includegraphics[width=\textwidth]{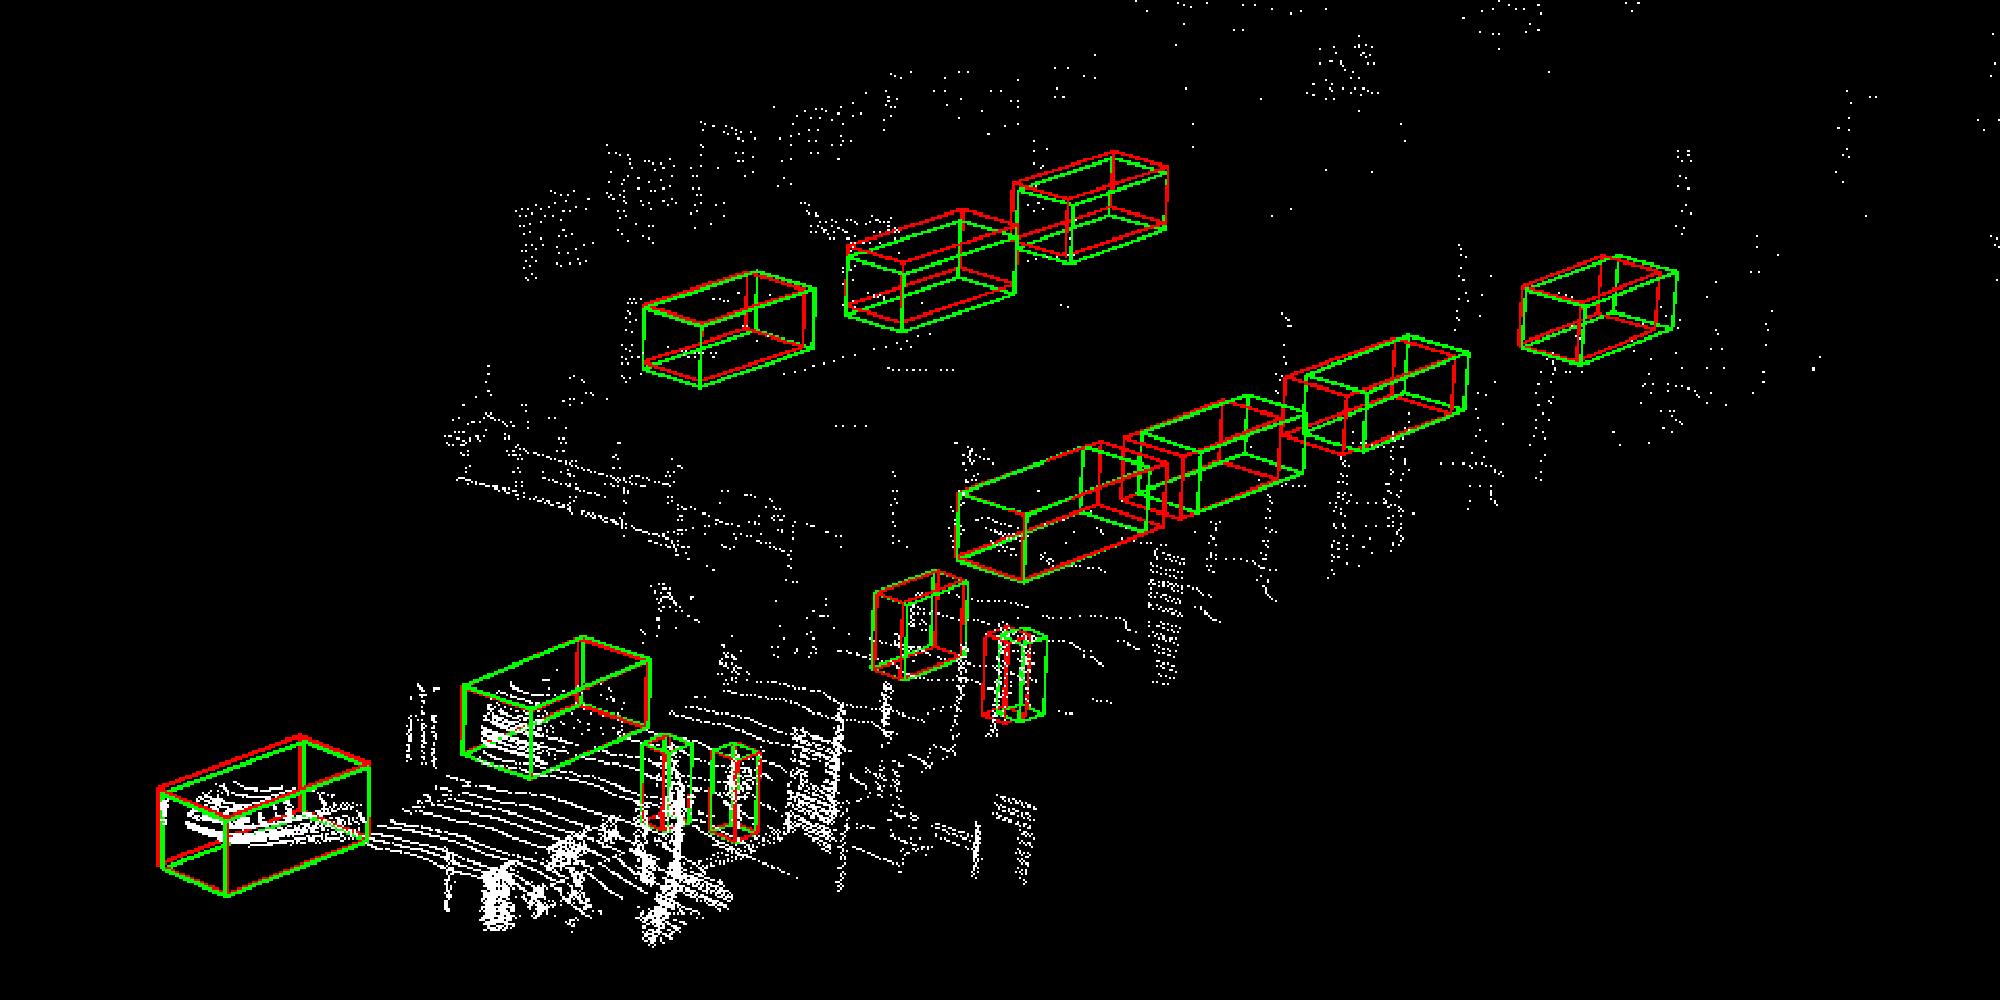}
            % \caption{00277}
            \end{subfigure}%  
        \end{minipage}
        \begin{minipage}{.48\textwidth}
            \begin{subfigure}{\textwidth}
            \centering
            \includegraphics[width=\textwidth]{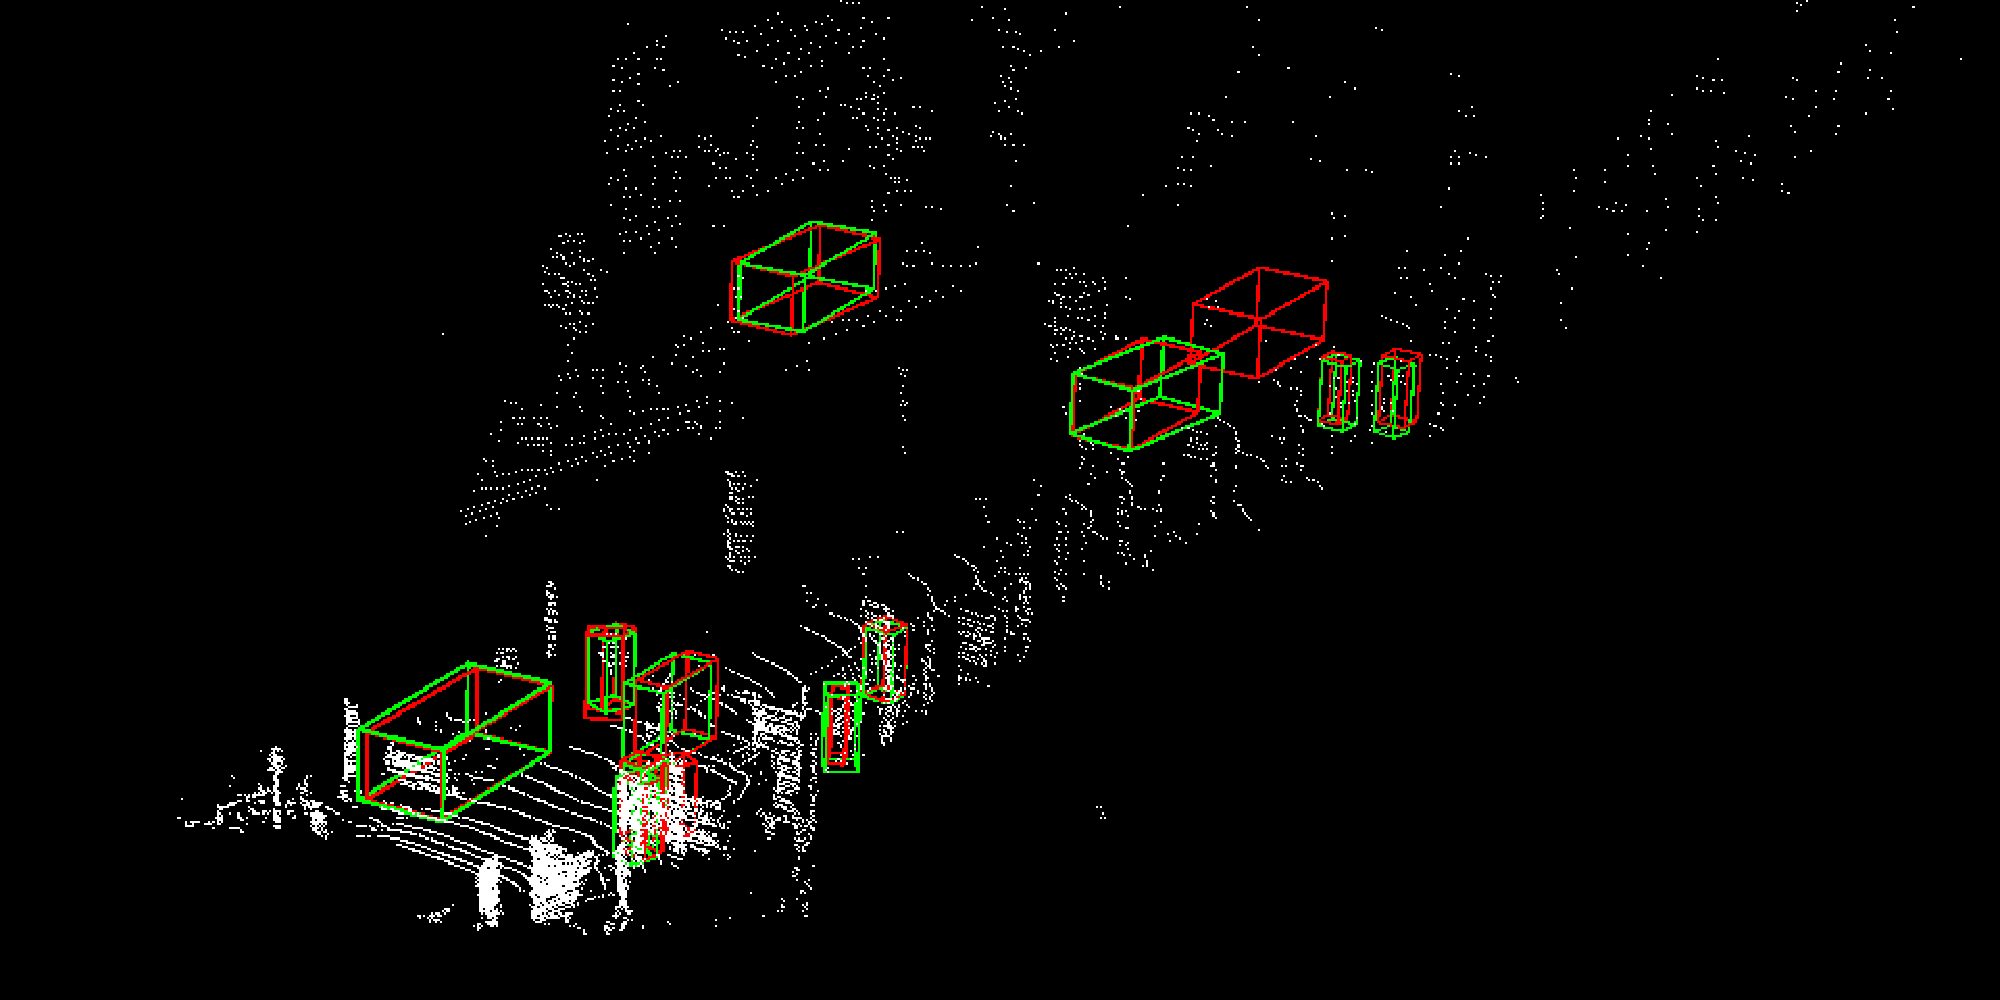}
            % \caption{00277}
            \end{subfigure}%  
        \end{minipage}
        \begin{minipage}{.48\textwidth}
            \begin{subfigure}{\textwidth}
            \centering
            \includegraphics[width=\textwidth]{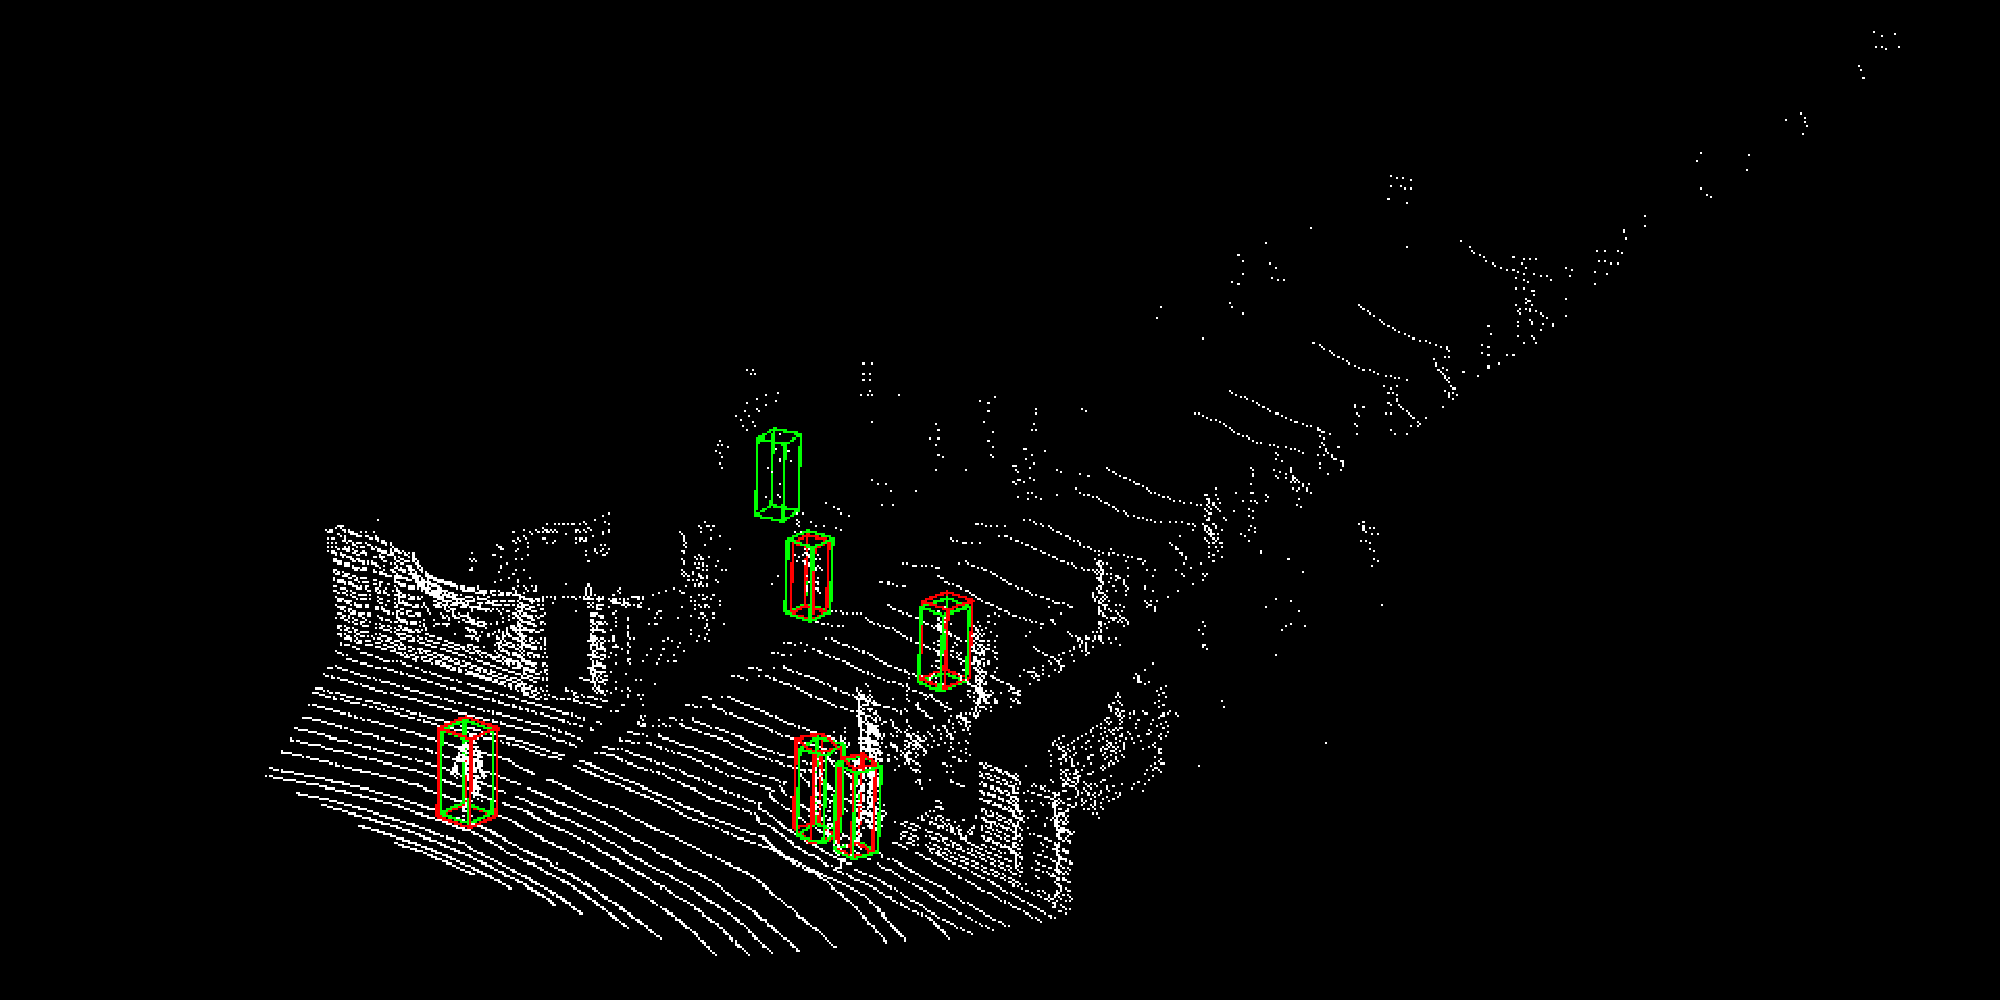}
            % \caption{00277}
            \end{subfigure}%  
        \end{minipage}
        % \begin{minipage}{.48\textwidth}
        %     \begin{subfigure}{\textwidth}
        %     \centering
        %     \includegraphics[width=\textwidth]{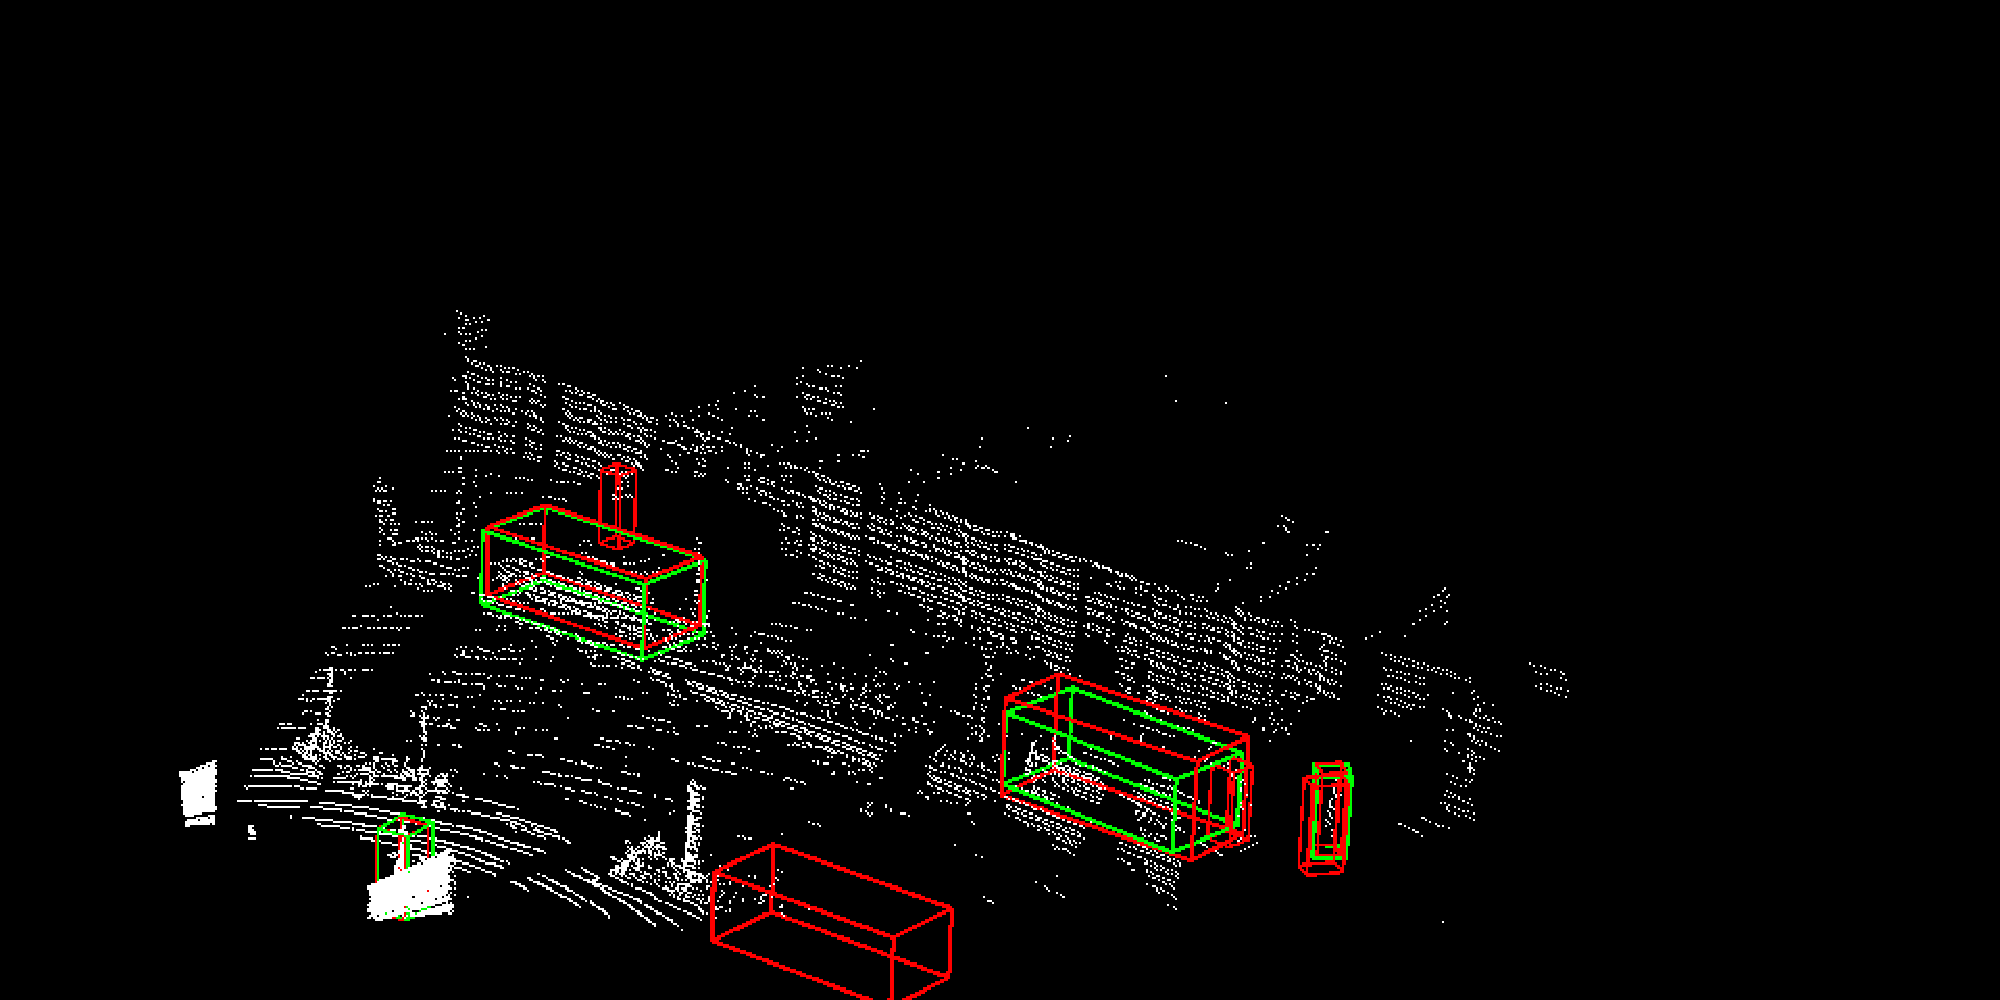}
        %     \caption{03593}
        %     \end{subfigure}%  
        % \end{minipage}
        % \begin{minipage}{.48\textwidth}
        %     \begin{subfigure}{\textwidth}
        %     \centering
        %     \includegraphics[width=\textwidth]{figure/lidar_qualitative_evaluation/04878.png}
        %     \caption{04878}
        %     \end{subfigure}%  
        % \end{minipage}
        % \begin{minipage}{.48\textwidth}
        %     \begin{subfigure}{\textwidth}
        %     \centering
        %     \includegraphics[width=\textwidth]{figure/lidar_qualitative_evaluation/05068.png}
        %     \caption{05068}
        %     \end{subfigure}%  
        % \end{minipage}
    \caption{LiDAR qualitative evaluation. Predictions by our method is shown in \textcolor{green}{green} while ground-truth bounding boxes are shown in \textcolor{red}{red} }
    \end{figure*}

\newpage

\begin{figure*}[t!]
    %%%%%%%%%%%%%%%%%GT%%%%%%%%%%%%%%%%%%%%%
    \begin{minipage}[t!]{0.29\textwidth}
        \centering
        \begin{subfigure}{.5\textwidth}
            \caption{Ground Truth}
        \end{subfigure}%
        \begin{subfigure}{\textwidth}
            \centering
            \includegraphics[width=0.99\textwidth]{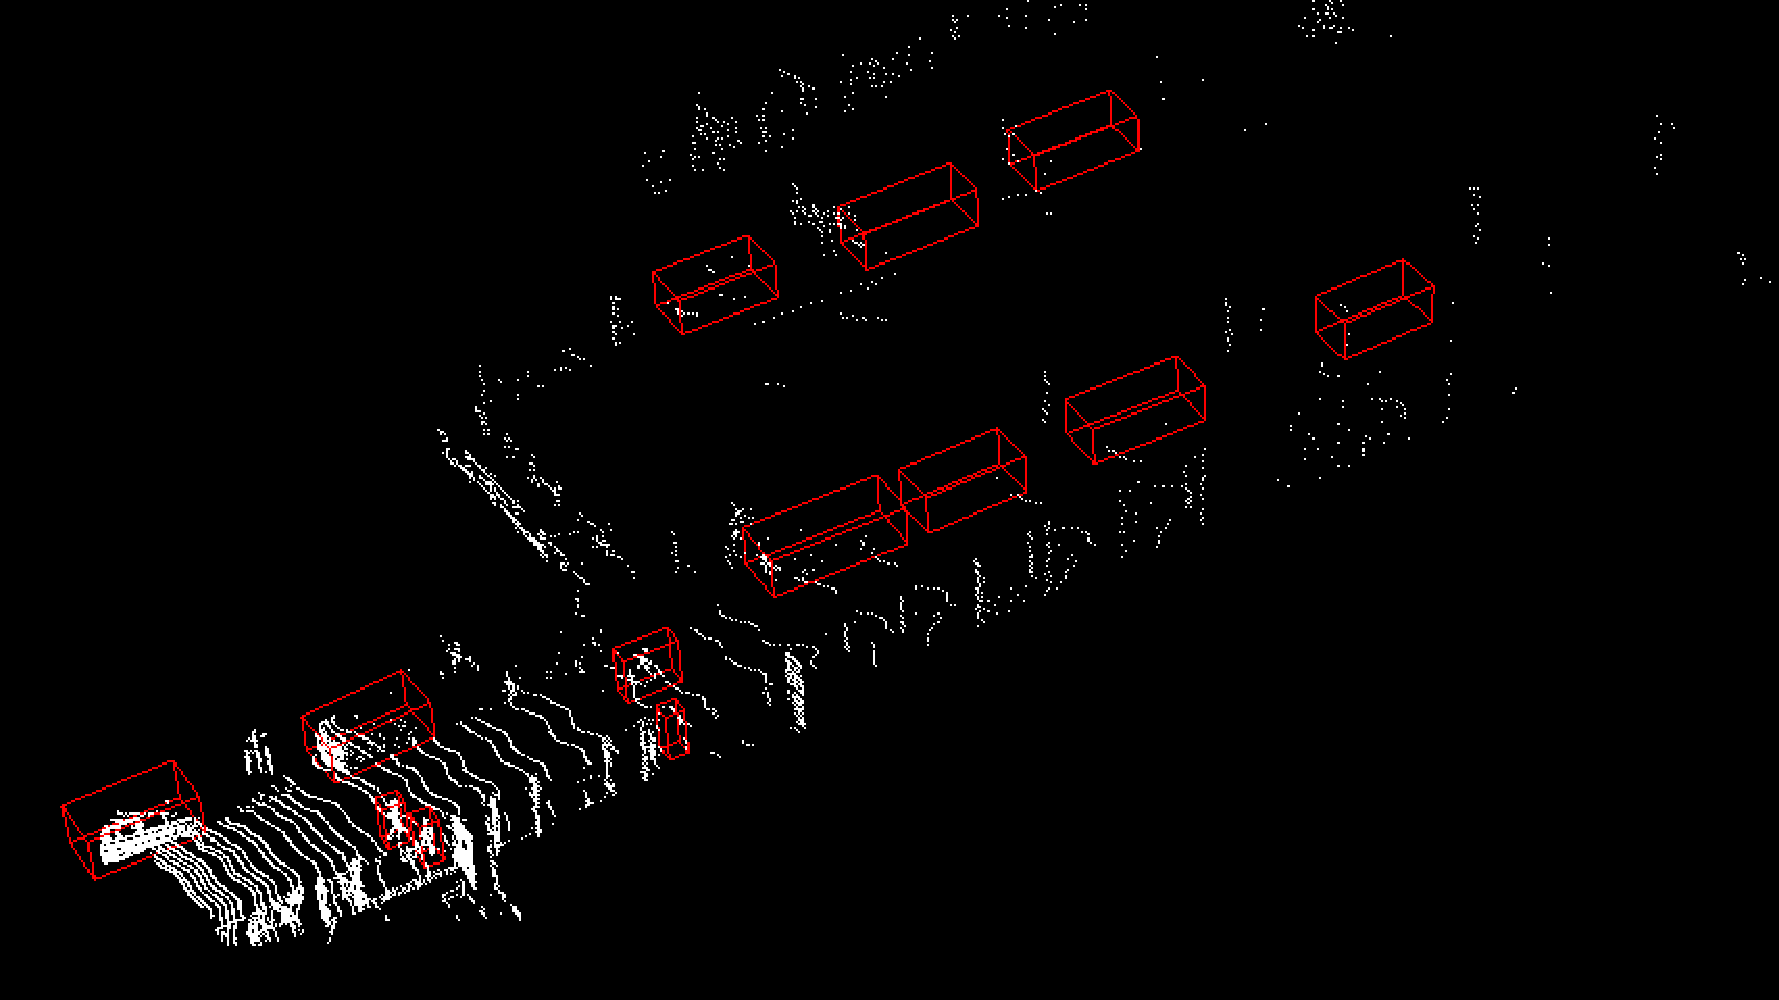}
        \end{subfigure}%
        \begin{subfigure}{\textwidth}
            \centering
            \includegraphics[width=0.99\textwidth]{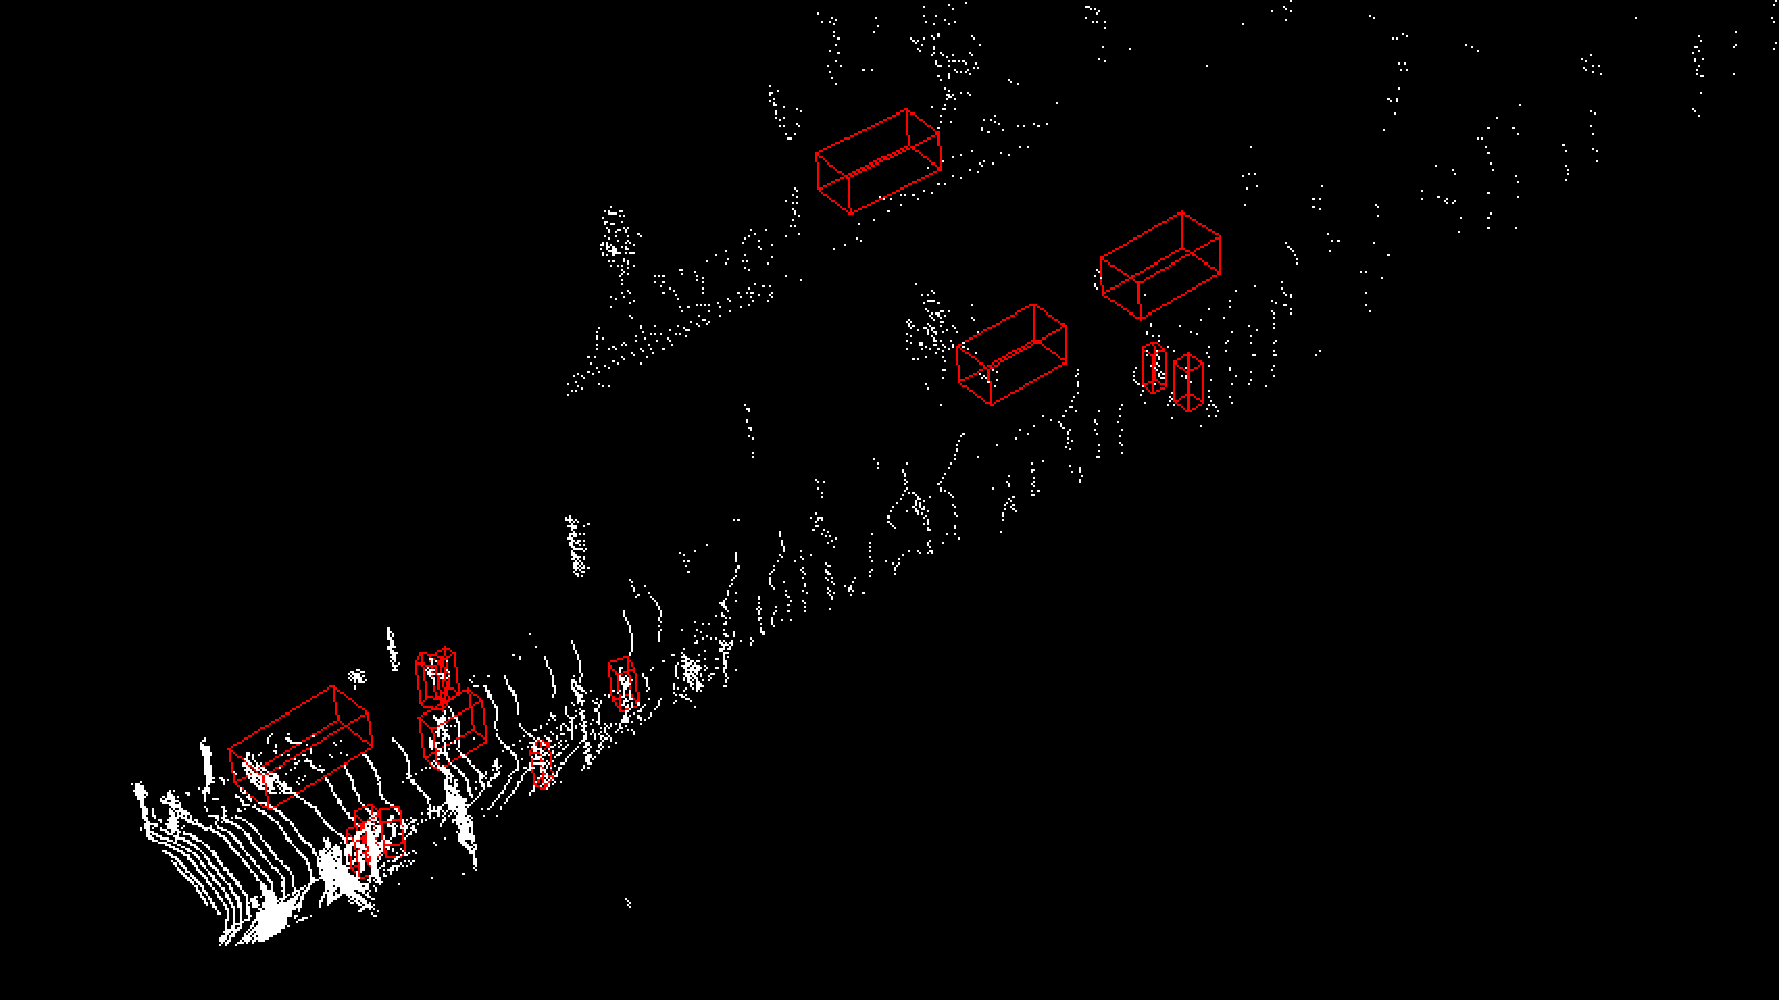}
        \end{subfigure}%
        \begin{subfigure}{\textwidth}
            \centering
            \includegraphics[width=0.99\textwidth]{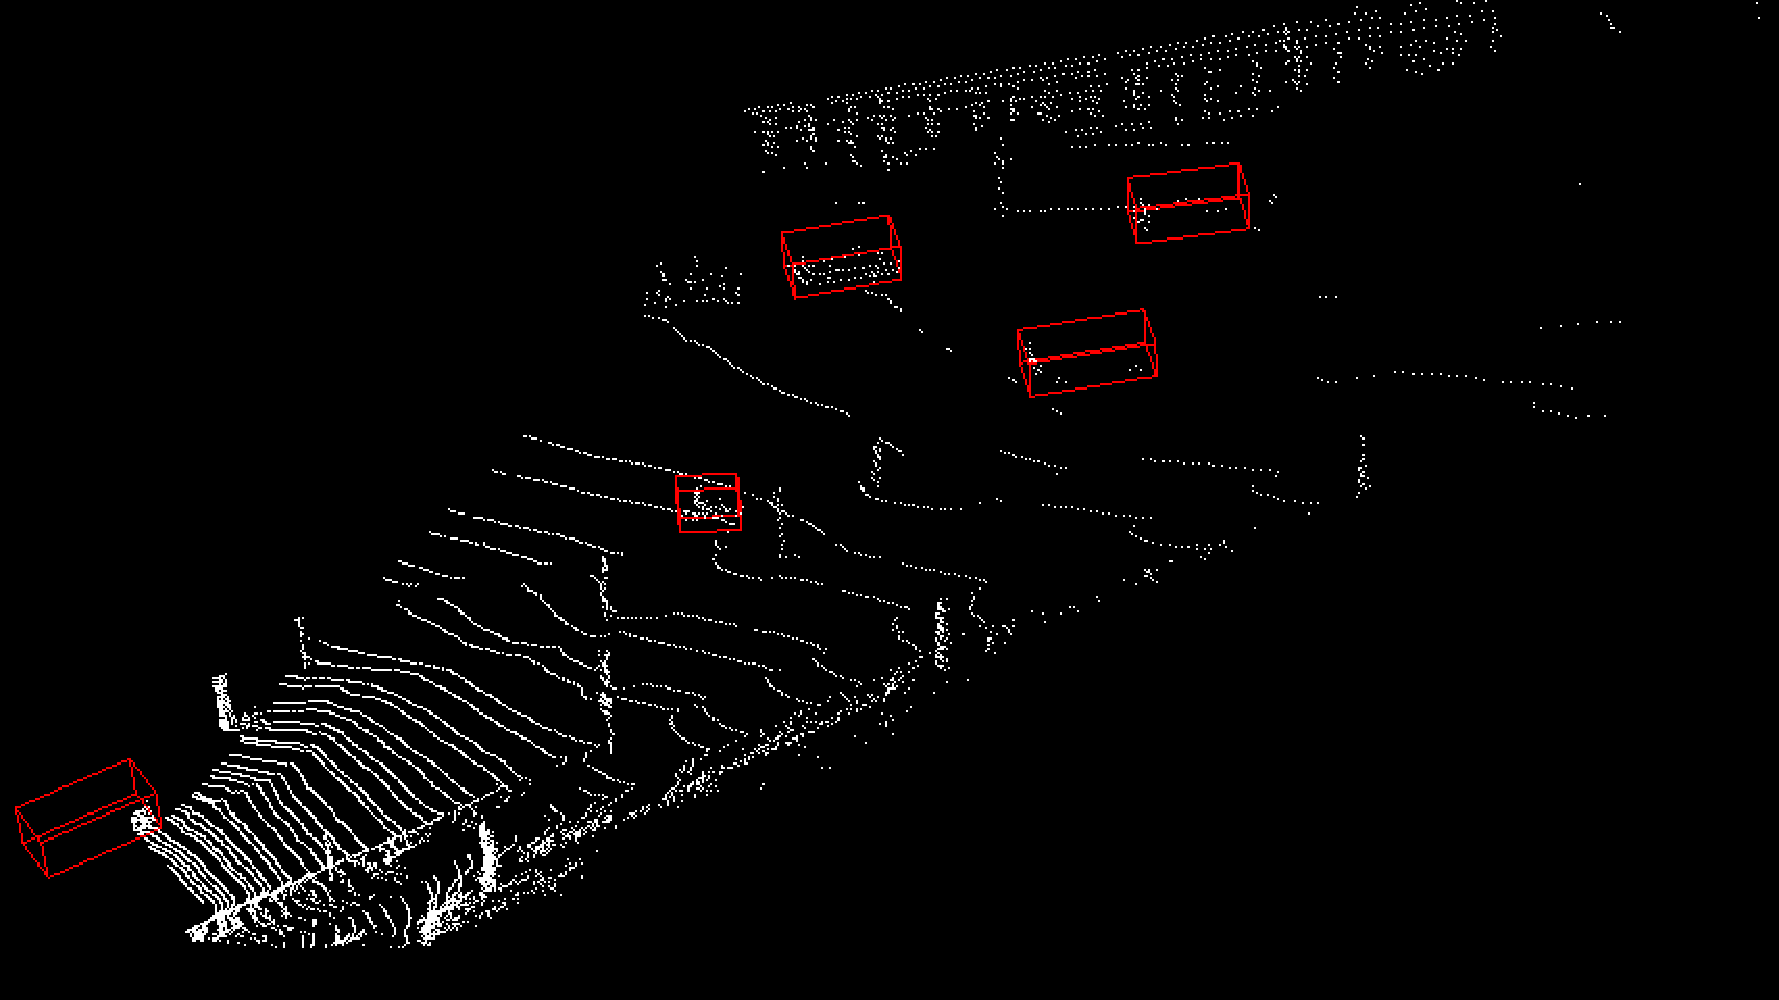}
        \end{subfigure}%
    \end{minipage}\\
    %%%%%%%%%%%%%%%%%CFAR%%%%%%%%%%%%%%%%%%%%%
    \begin{minipage}[t!]{0.29\textwidth}
        \centering
        \begin{subfigure}{.5\textwidth}
            \caption{ours}
        \end{subfigure}%
        \begin{subfigure}{\textwidth}
            \centering
            \includegraphics[width=0.99\textwidth]{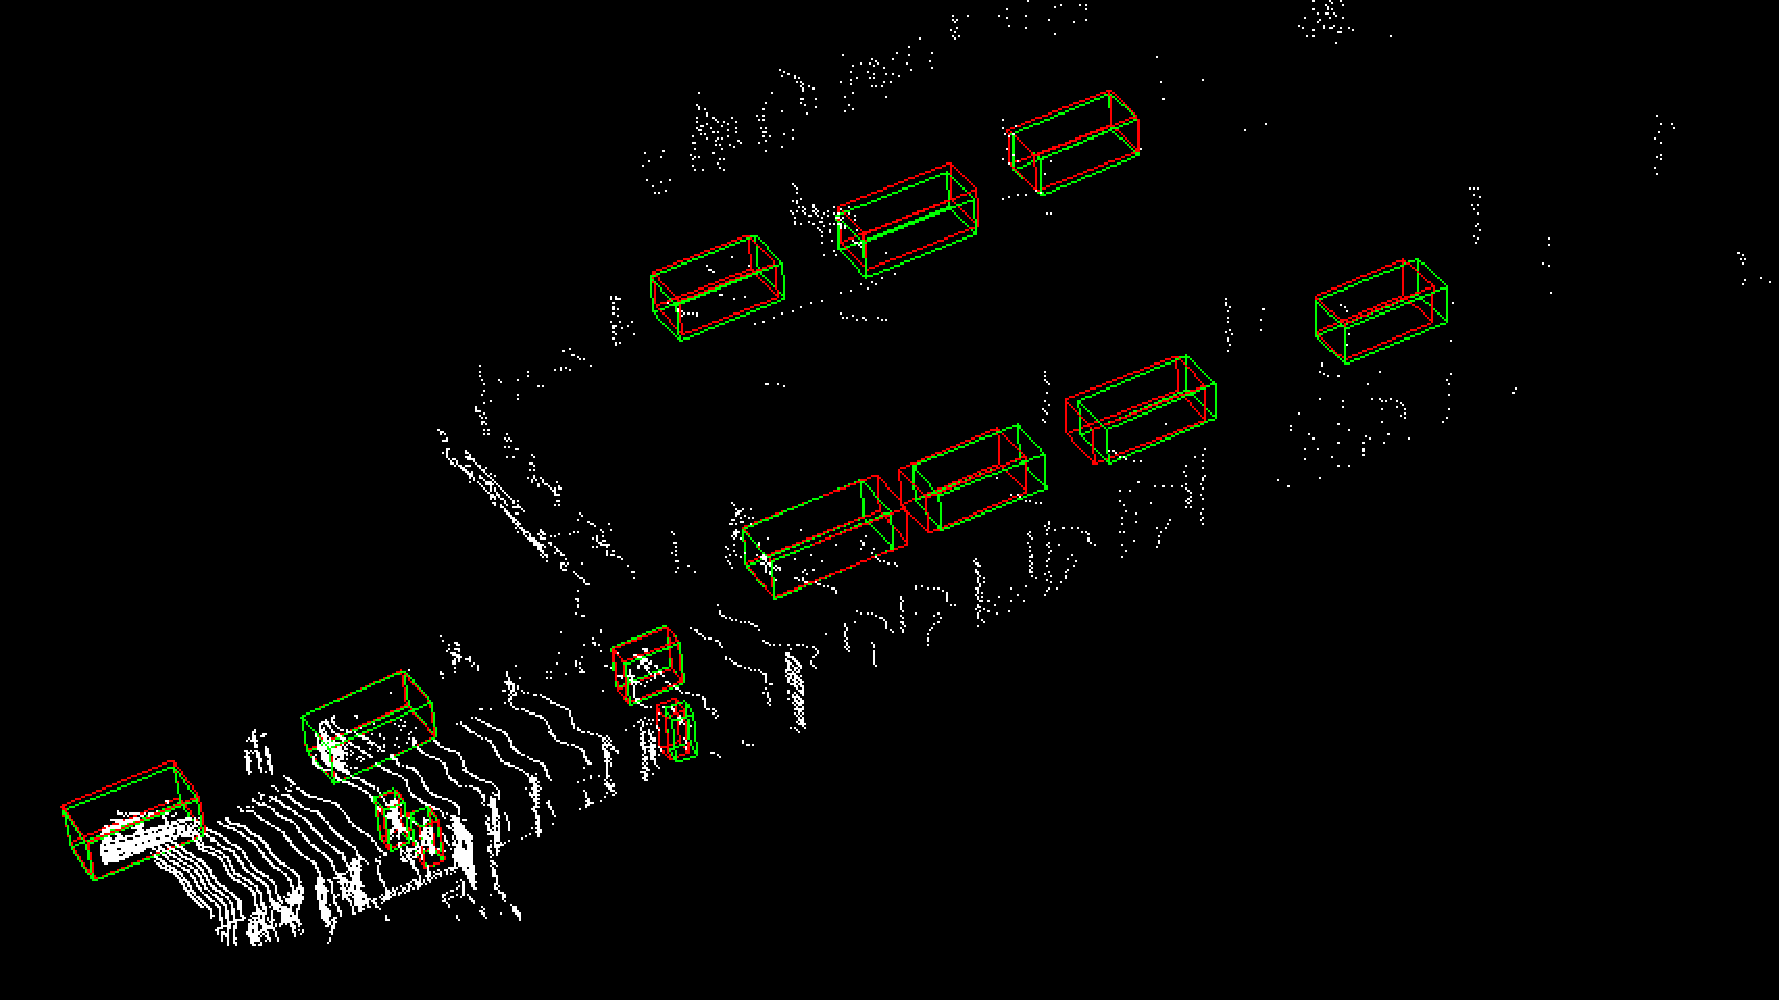}
        \end{subfigure}%
        \begin{subfigure}{\textwidth}
            \centering
            \includegraphics[width=0.99\textwidth]{figure/lidar_against_baselines_eps/CFAR_lidar_rcs00277.eps}
        \end{subfigure}%
        \begin{subfigure}{\textwidth}
            \centering
            \includegraphics[width=0.99\textwidth]{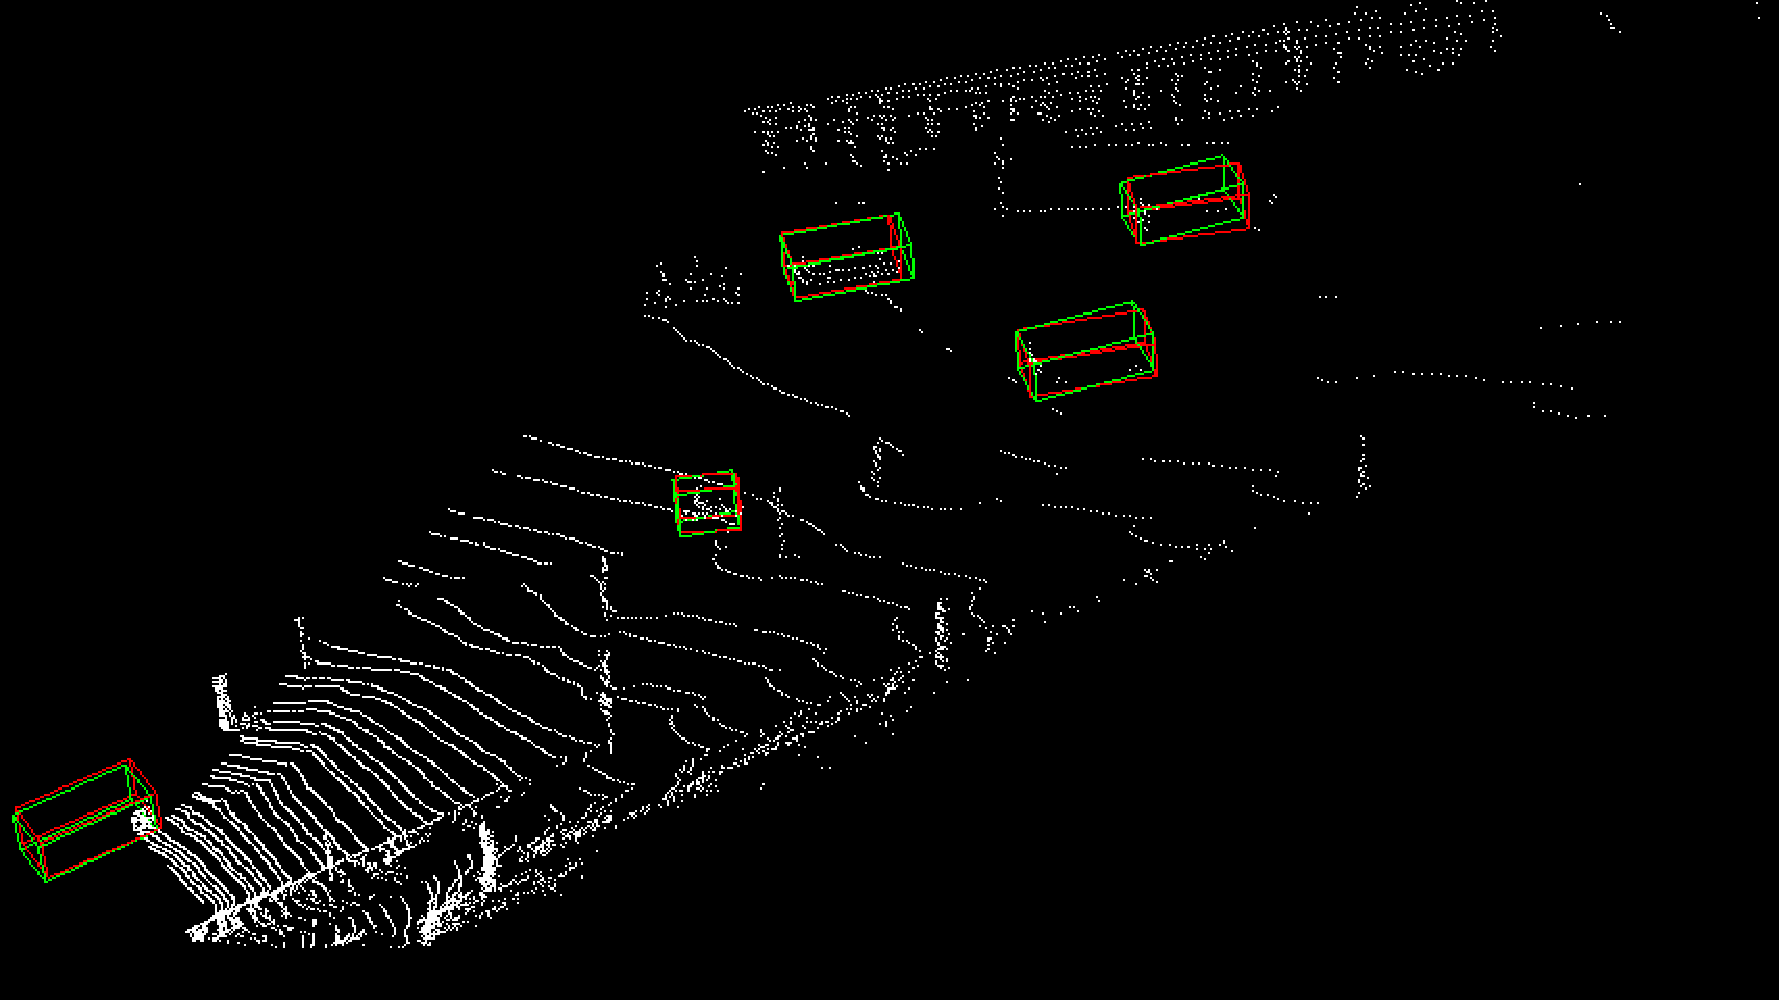}
        \end{subfigure}%
    \end{minipage}\\
    %%%%%%%%%%%%%%%%%POINTPILLARS%%%%%%%%%%%%%%%%%%%%%
    \begin{minipage}[t!]{0.29\textwidth}
        \centering
        \begin{subfigure}{.5\textwidth}
            \caption{pointpillars}
        \end{subfigure}%
        \begin{subfigure}{\textwidth}
            \centering
            \includegraphics[width=0.99\textwidth]{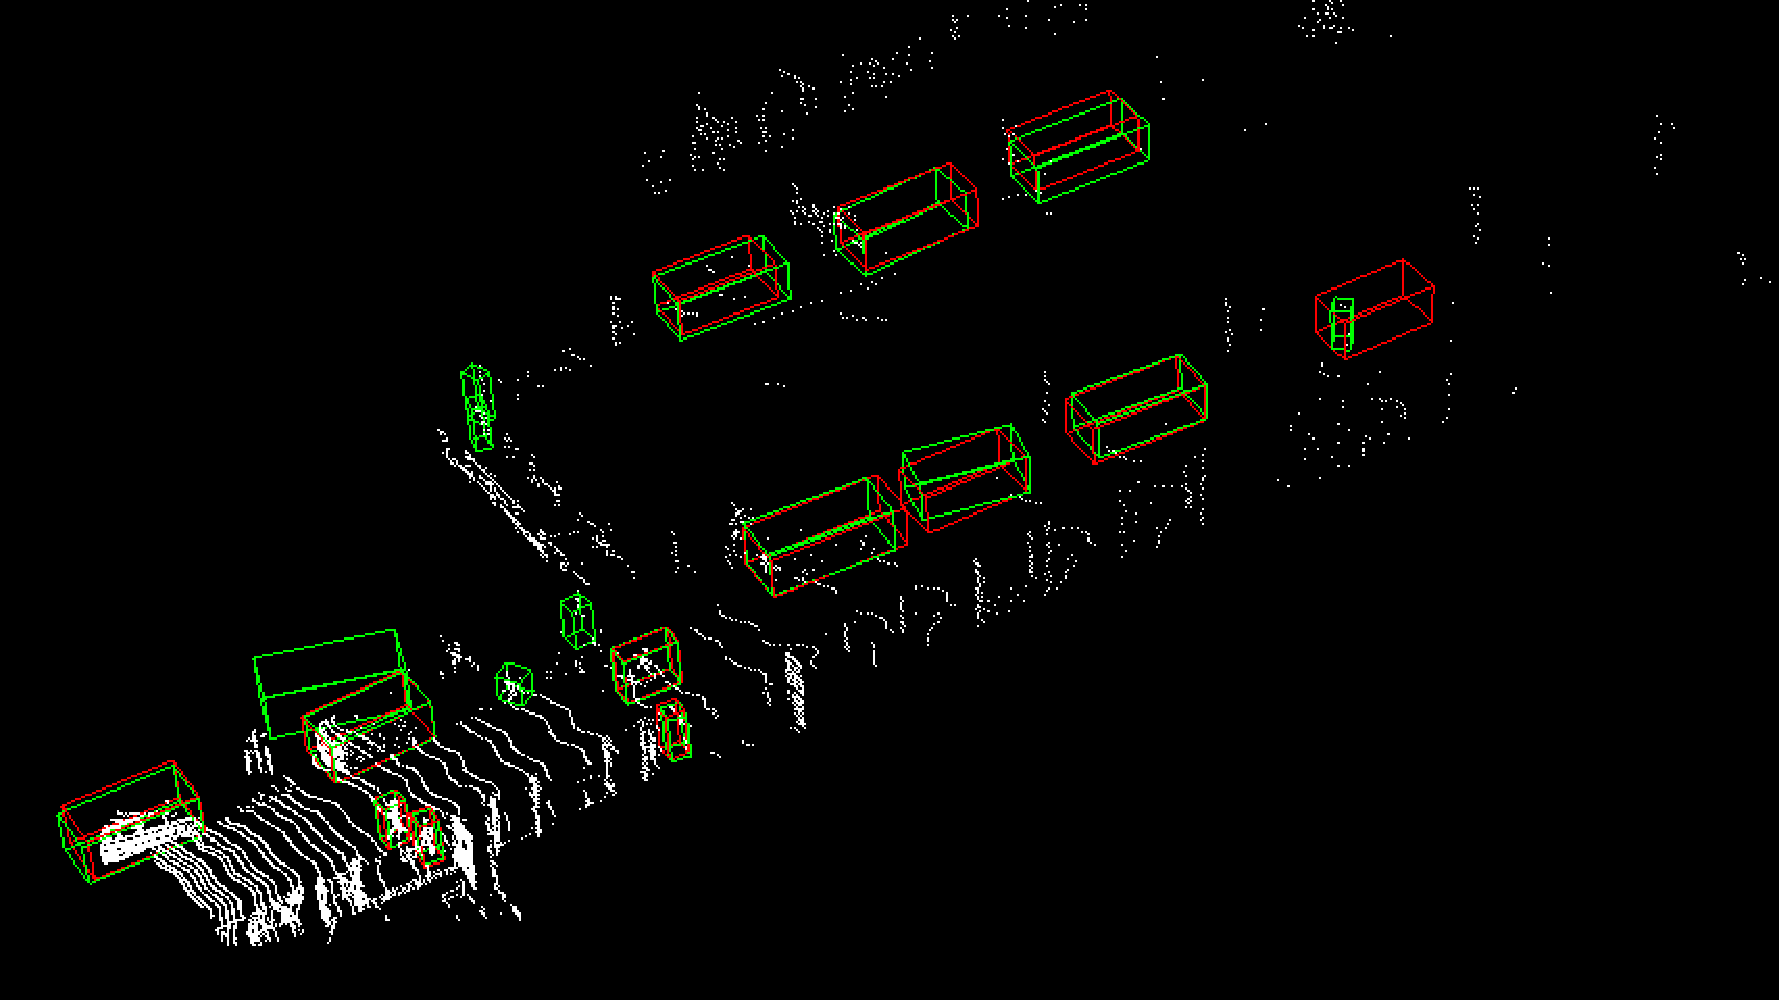}
        \end{subfigure}%
        \begin{subfigure}{\textwidth}
            \centering
            \includegraphics[width=0.99\textwidth]{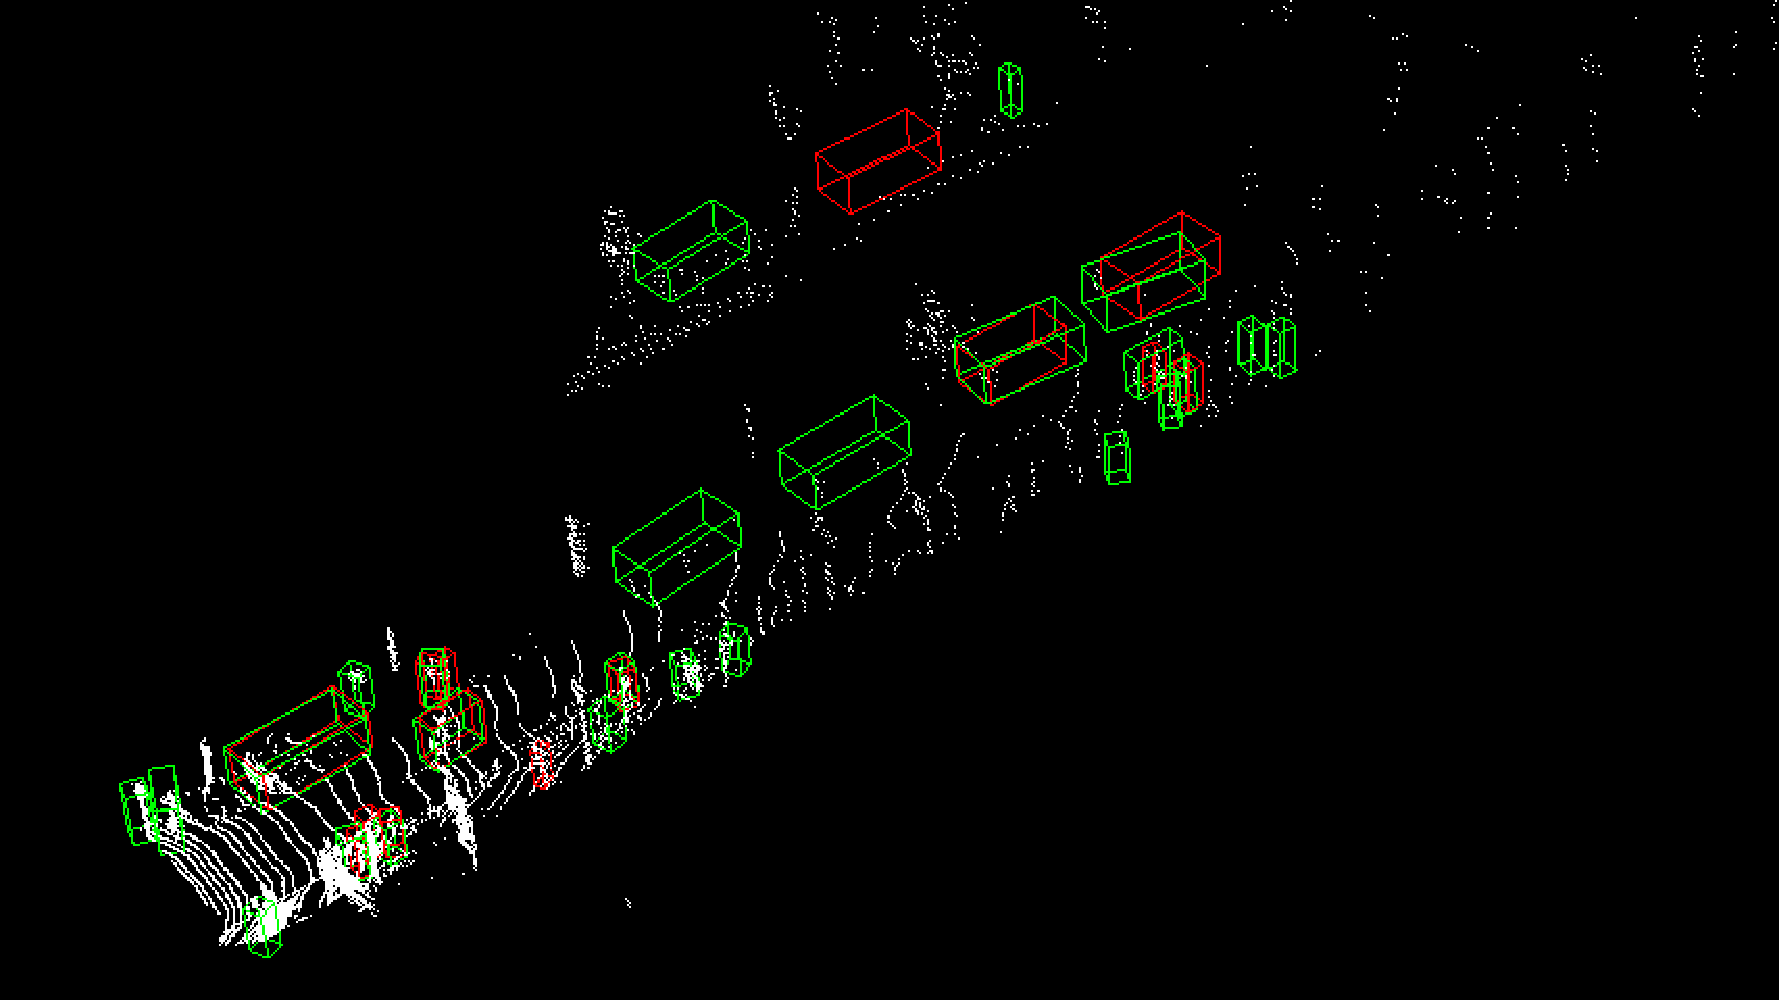}
        \end{subfigure}%
        \begin{subfigure}{\textwidth}
            \centering
            \includegraphics[width=0.99\textwidth]{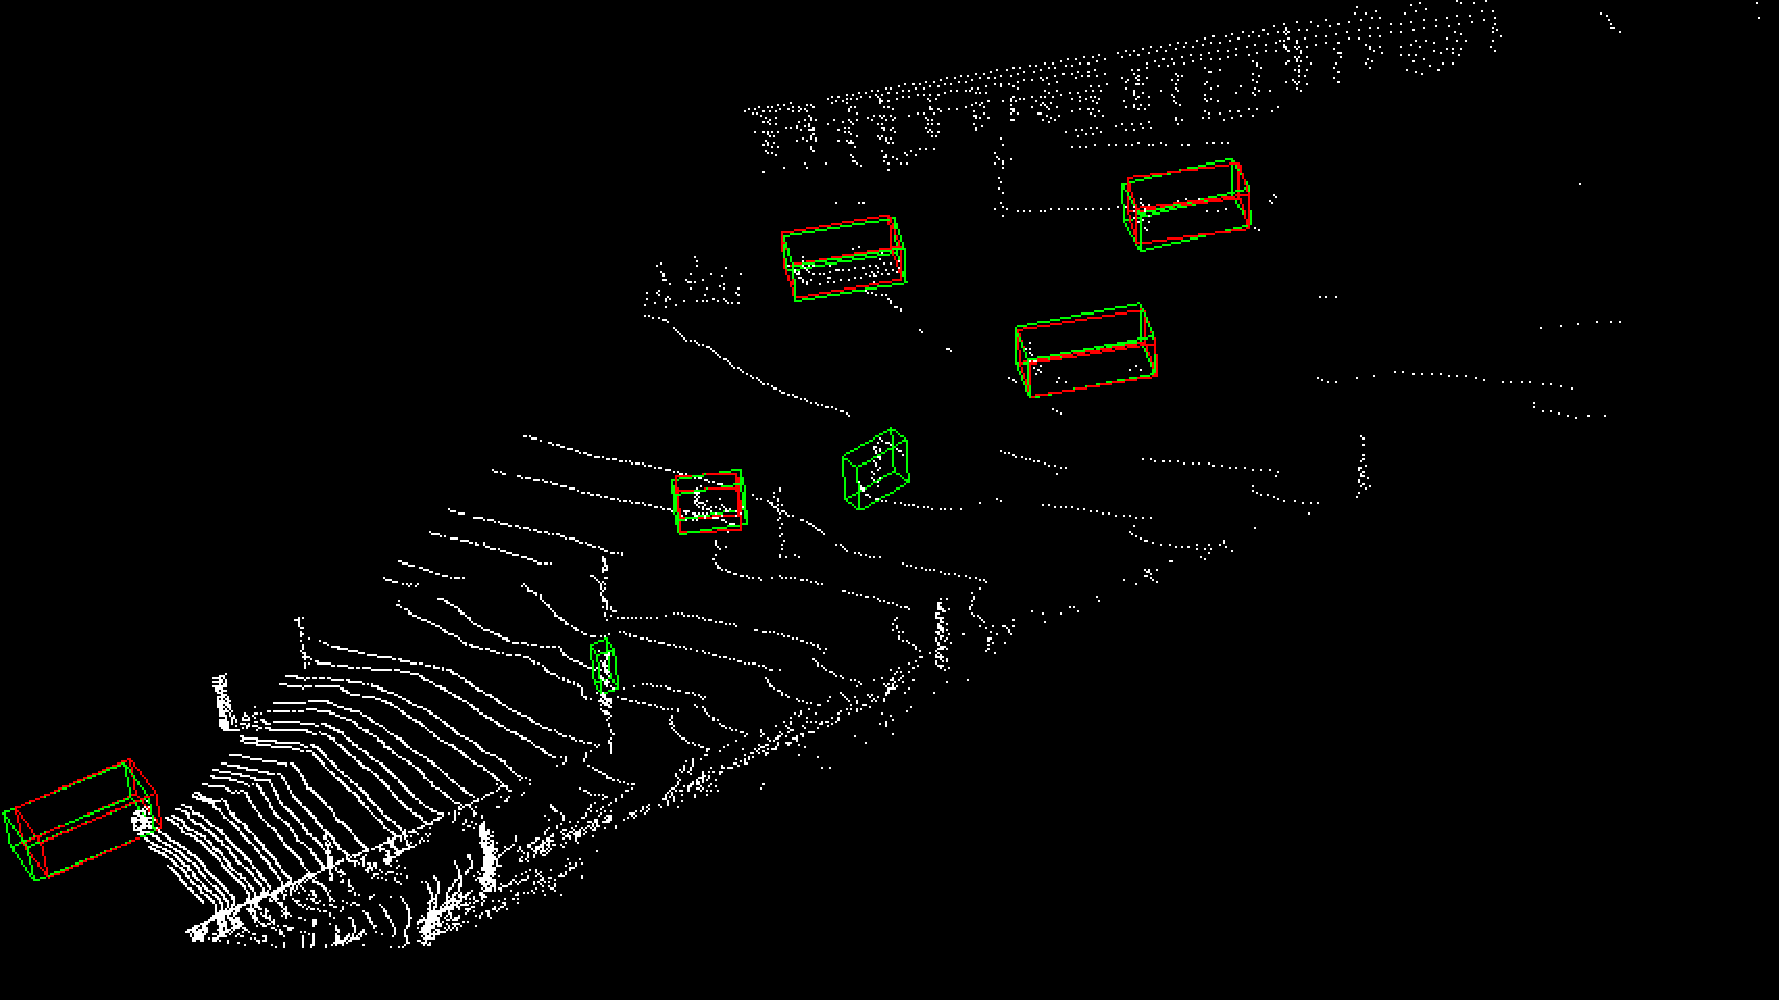}
        \end{subfigure}%
    \end{minipage}\\
    %%%%%%%%%%%%%%%%%SECOND%%%%%%%%%%%%%%%%%%%%%
    \begin{minipage}[t!]{0.29\textwidth}
        \centering
        \begin{subfigure}{.5\textwidth}
            \caption{SECOND}
        \end{subfigure}%
        \begin{subfigure}{\textwidth}
            \centering
            \includegraphics[width=0.99\textwidth]{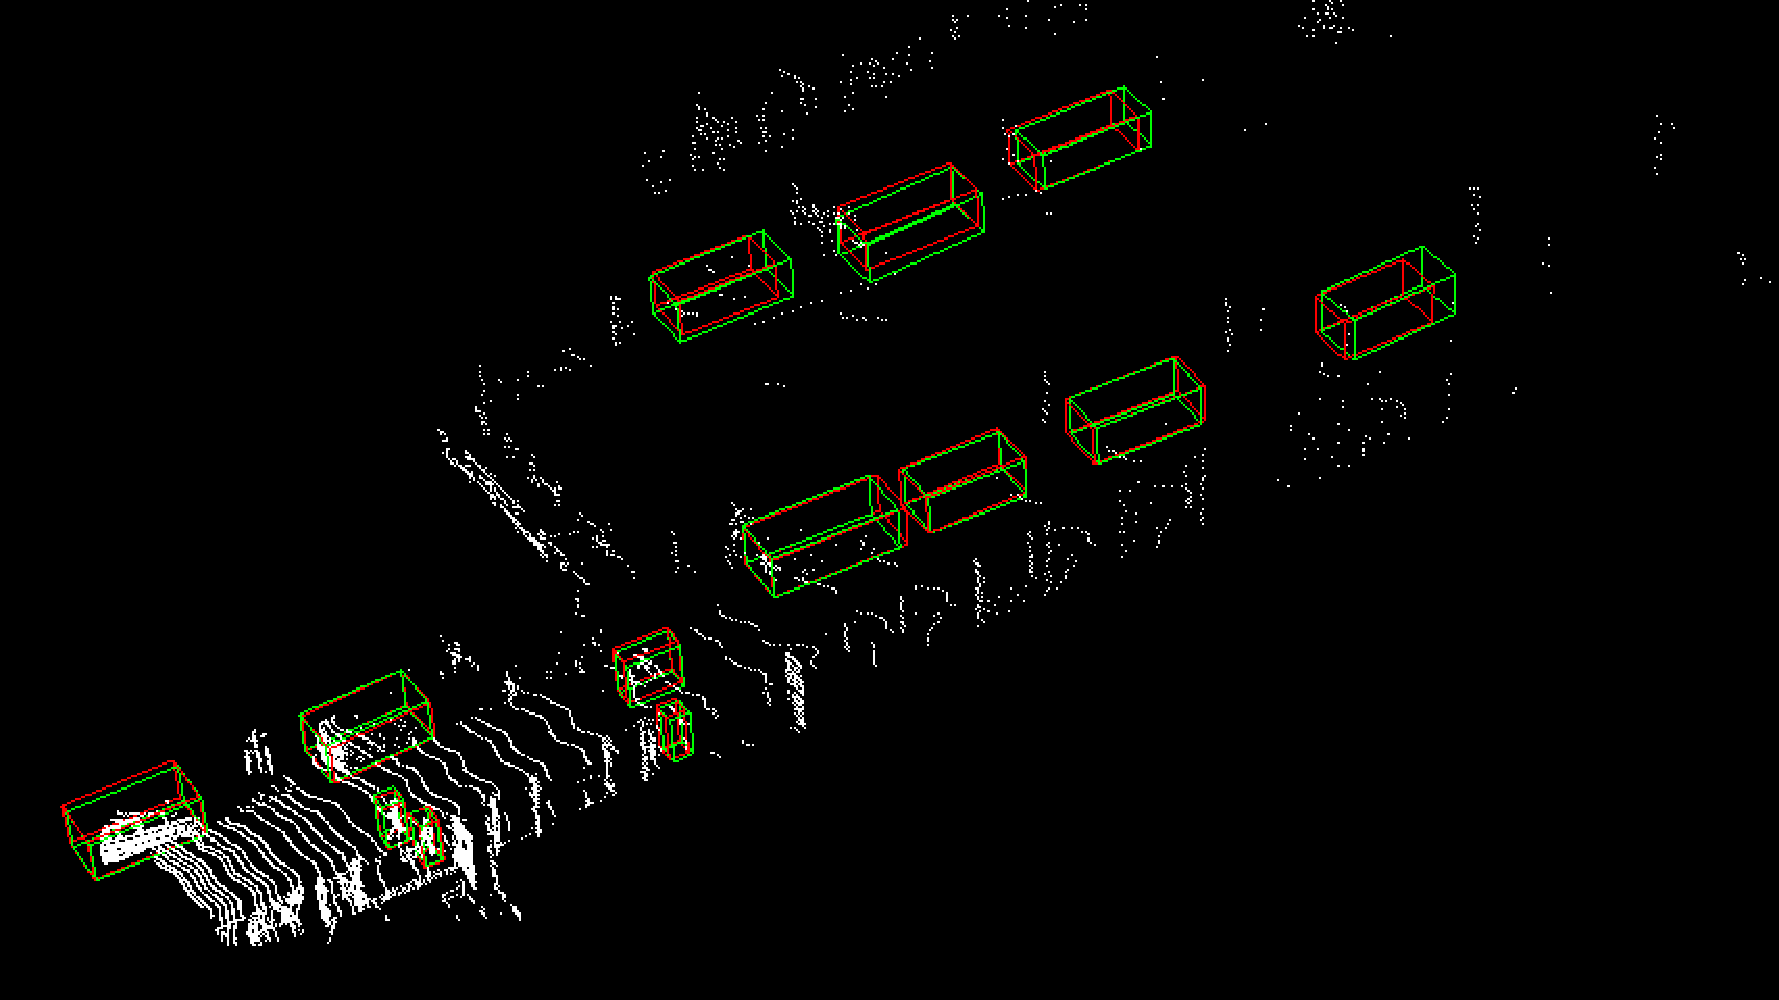}
        \end{subfigure}%
        \begin{subfigure}{\textwidth}
            \centering
            \includegraphics[width=0.99\textwidth]{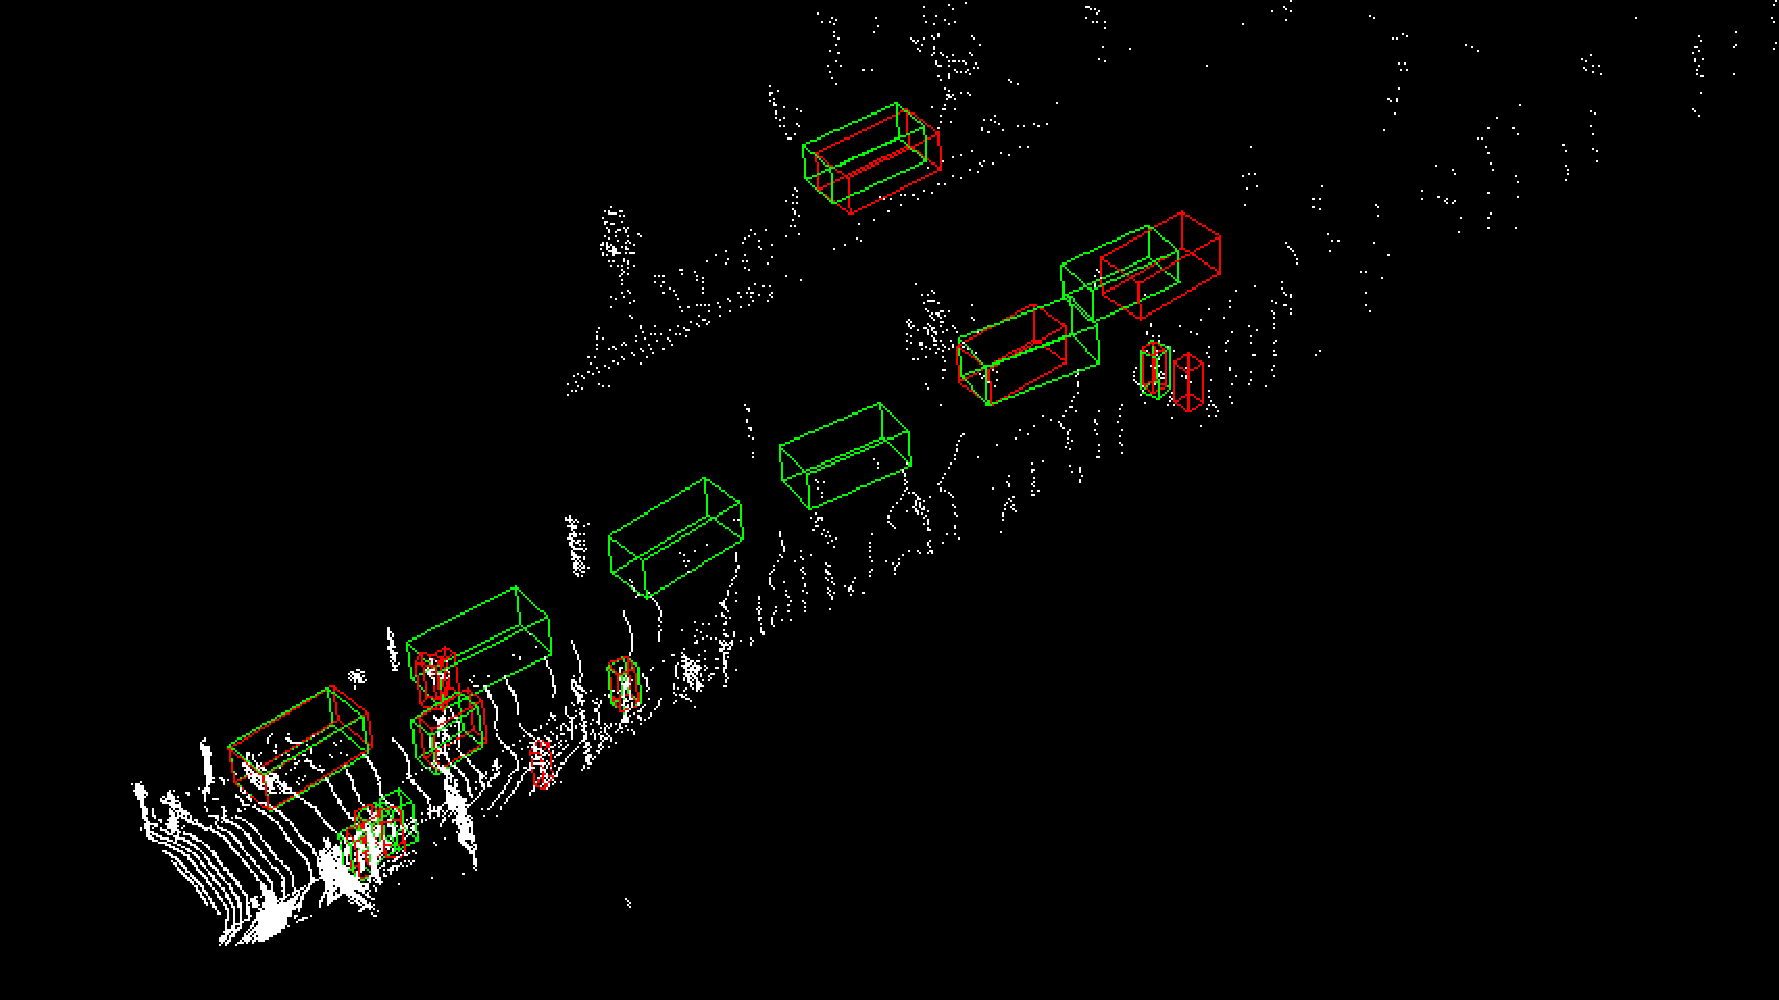}
        \end{subfigure}%
        \begin{subfigure}{\textwidth}
            \centering
            \includegraphics[width=0.99\textwidth]{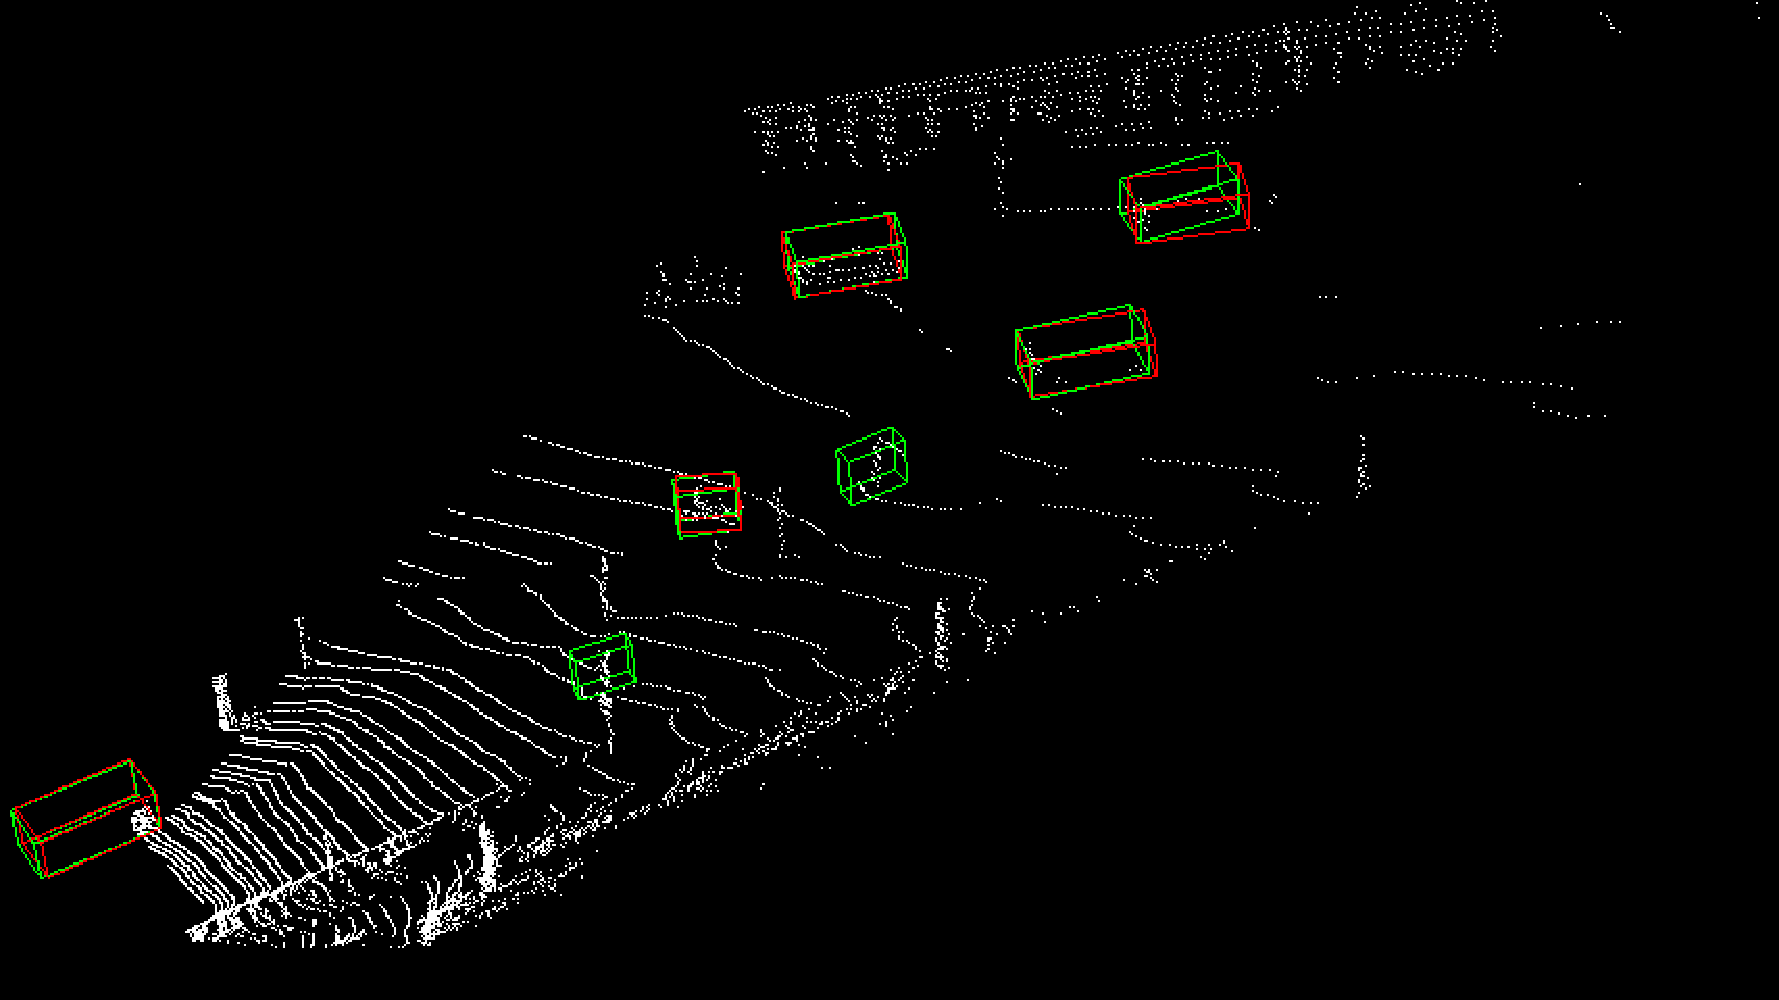}
        \end{subfigure}%
    \end{minipage}\\
    %%%%%%%%%%%%%%%%%Centerpoint%%%%%%%%%%%%%%%%%%%%%
    \begin{minipage}[t!]{0.29\textwidth}
        \centering
        \begin{subfigure}{.5\textwidth}
            \caption{Centerpoint}
        \end{subfigure}%
        \begin{subfigure}{\textwidth}
            \centering
            \includegraphics[width=0.99\textwidth]{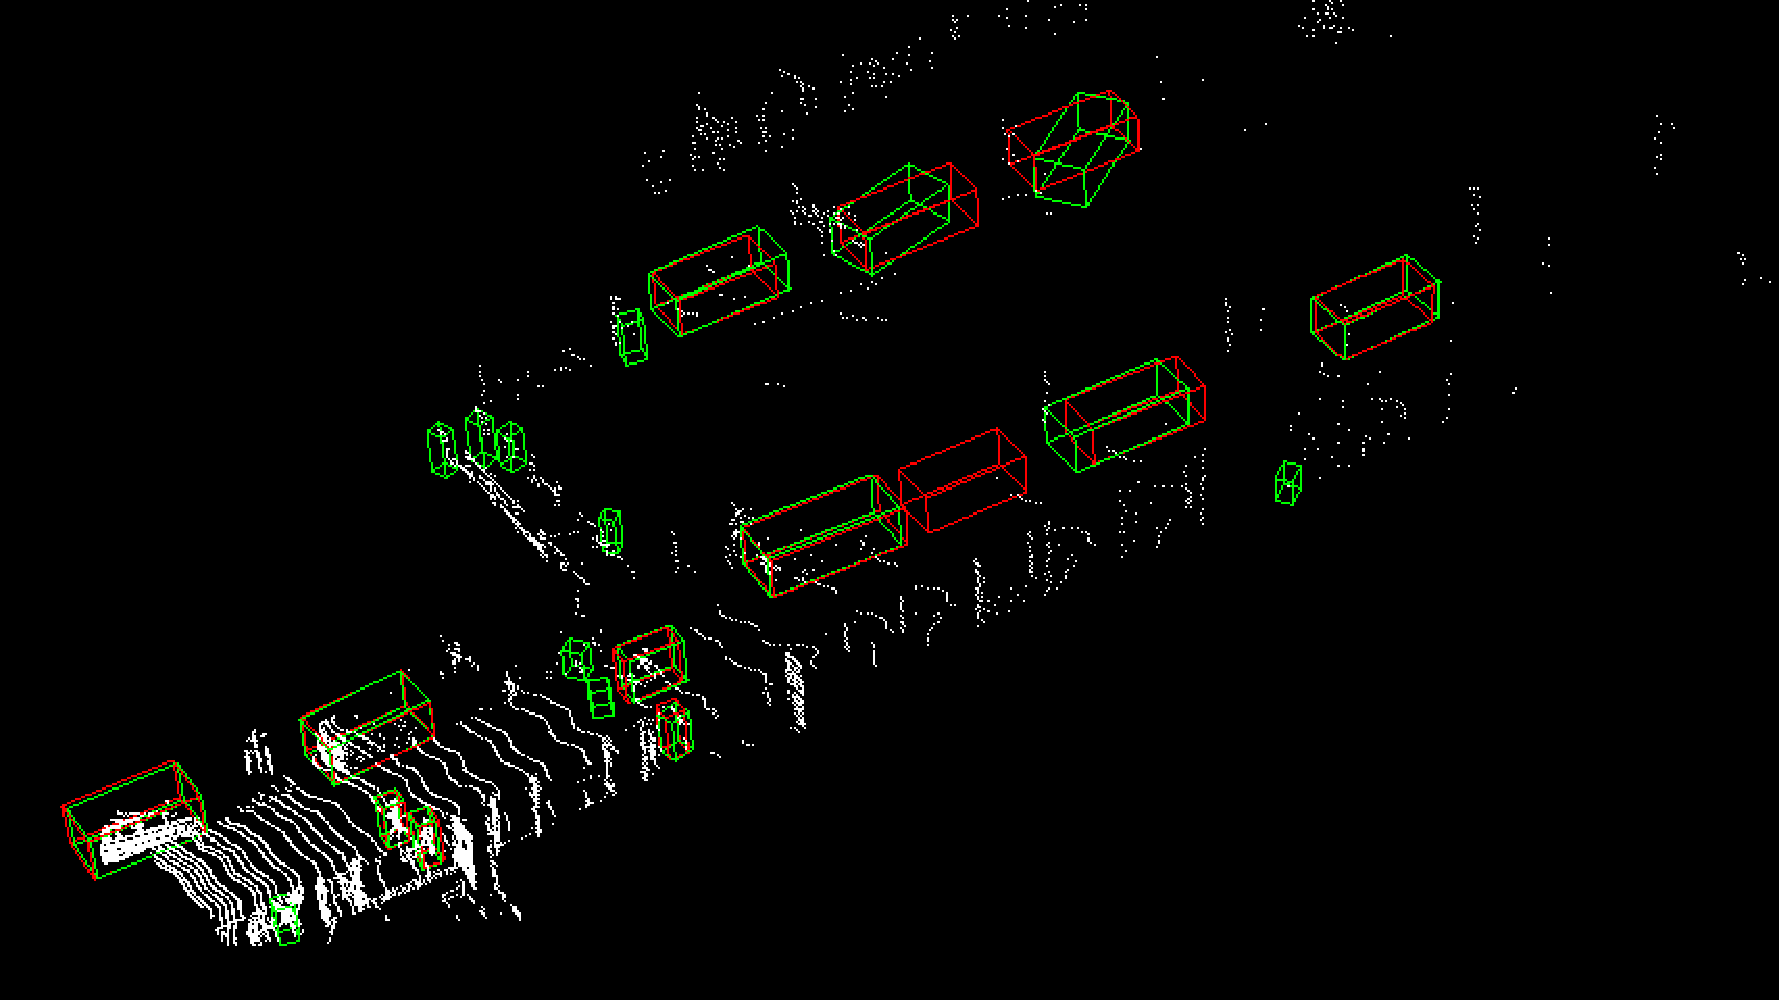}
        \end{subfigure}%
        \begin{subfigure}{\textwidth}
            \centering
            \includegraphics[width=0.99\textwidth]{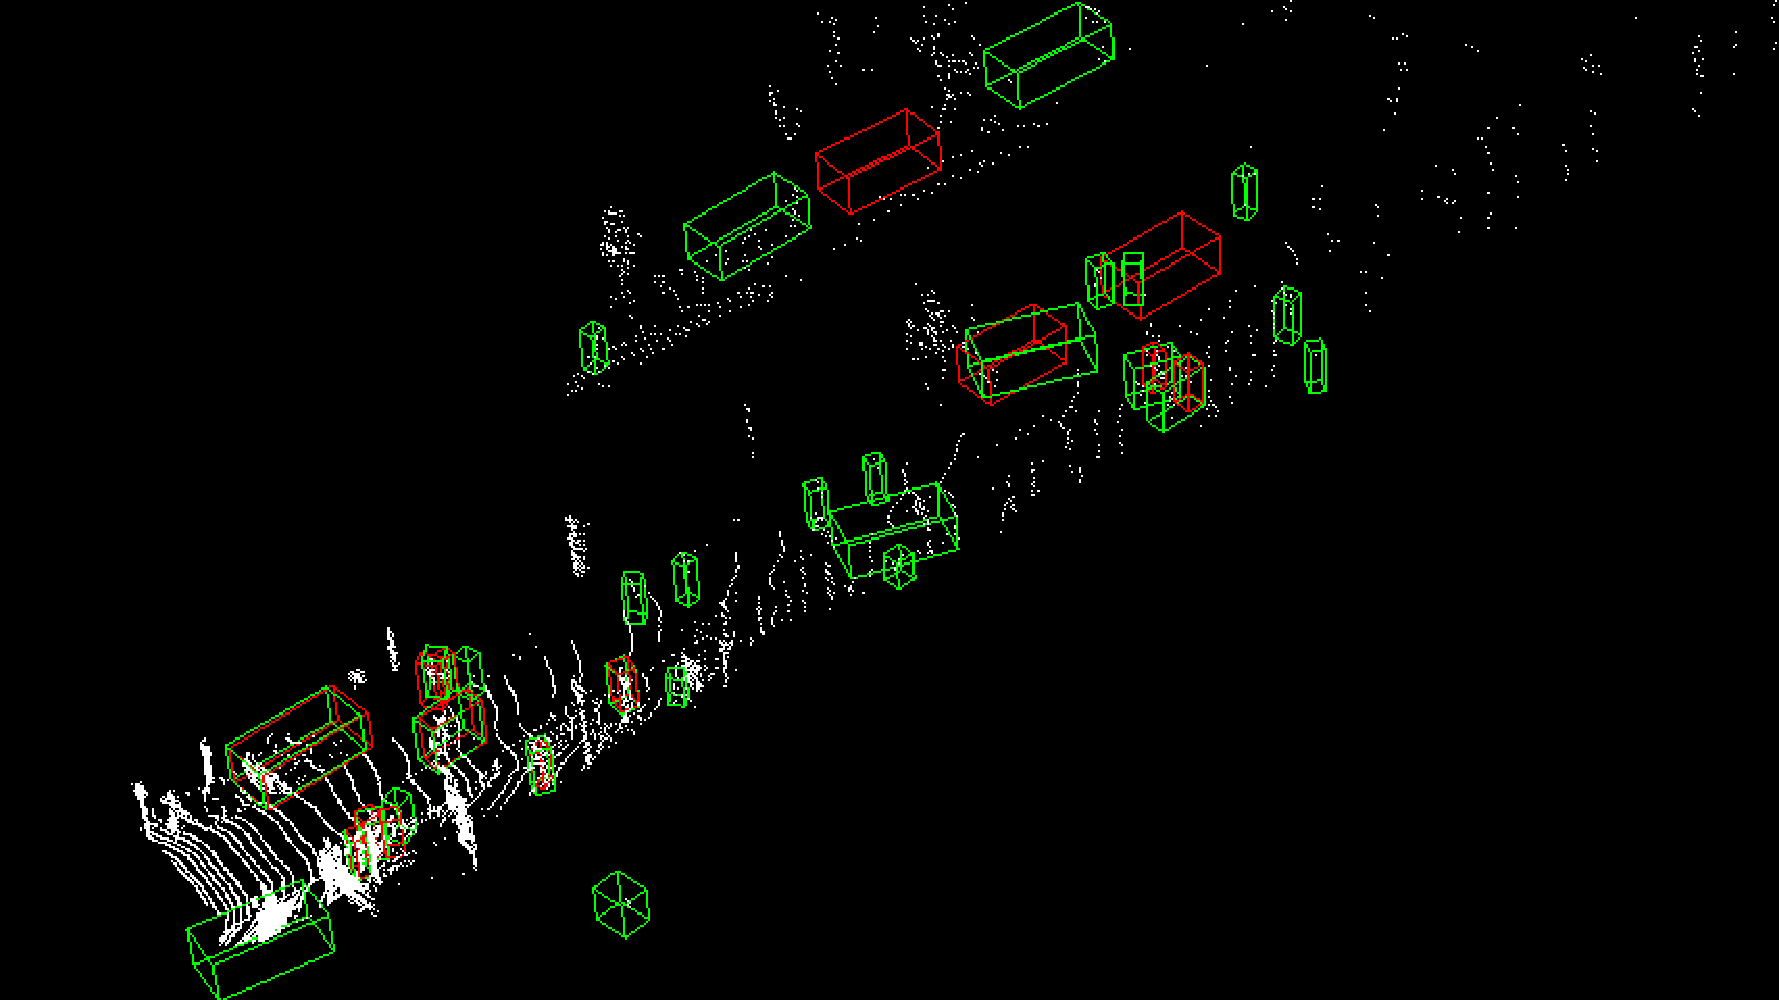}
        \end{subfigure}%
        \begin{subfigure}{\textwidth}
            \centering
            \includegraphics[width=0.99\textwidth]{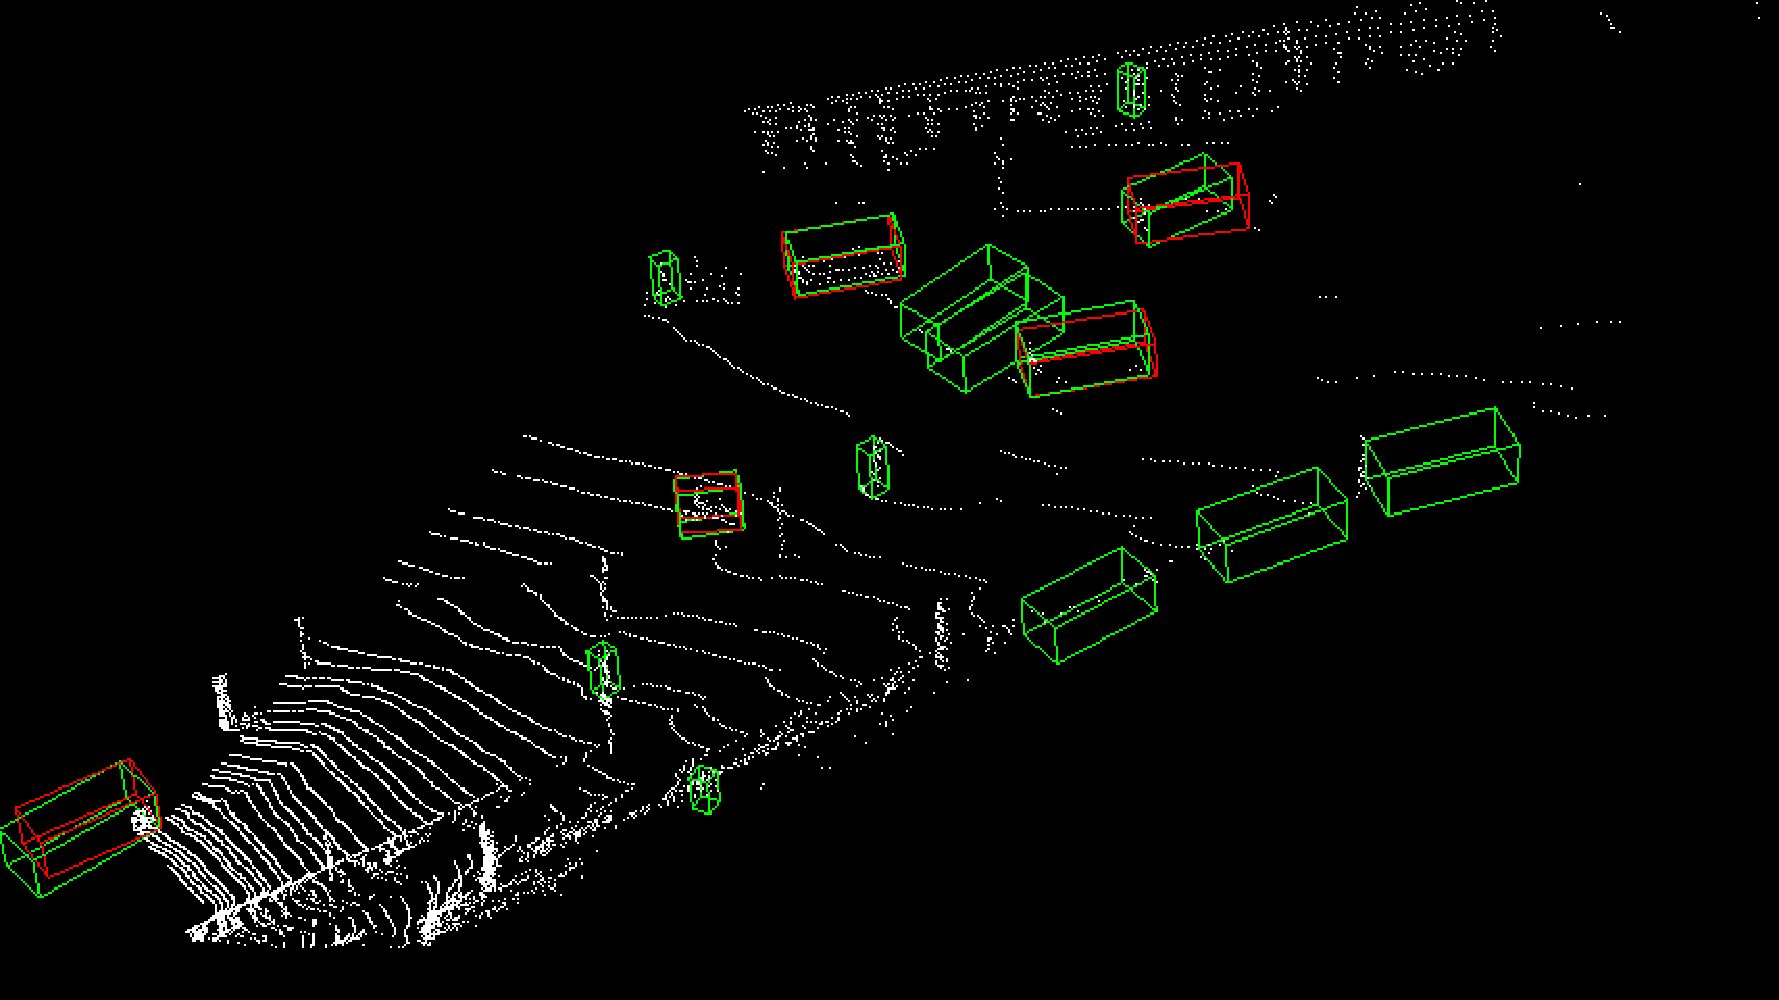}
        \end{subfigure}%
    \end{minipage}\\
    %%%%%%%%%%%%%%%%%pointrcnn%%%%%%%%%%%%%%%%%%%%%
    \begin{minipage}[t!]{0.29\textwidth}
        \centering
        \begin{subfigure}{.5\textwidth}
            \caption{PointRCNN}
        \end{subfigure}%
        \begin{subfigure}{\textwidth}
            \centering
            \includegraphics[width=0.99\textwidth]{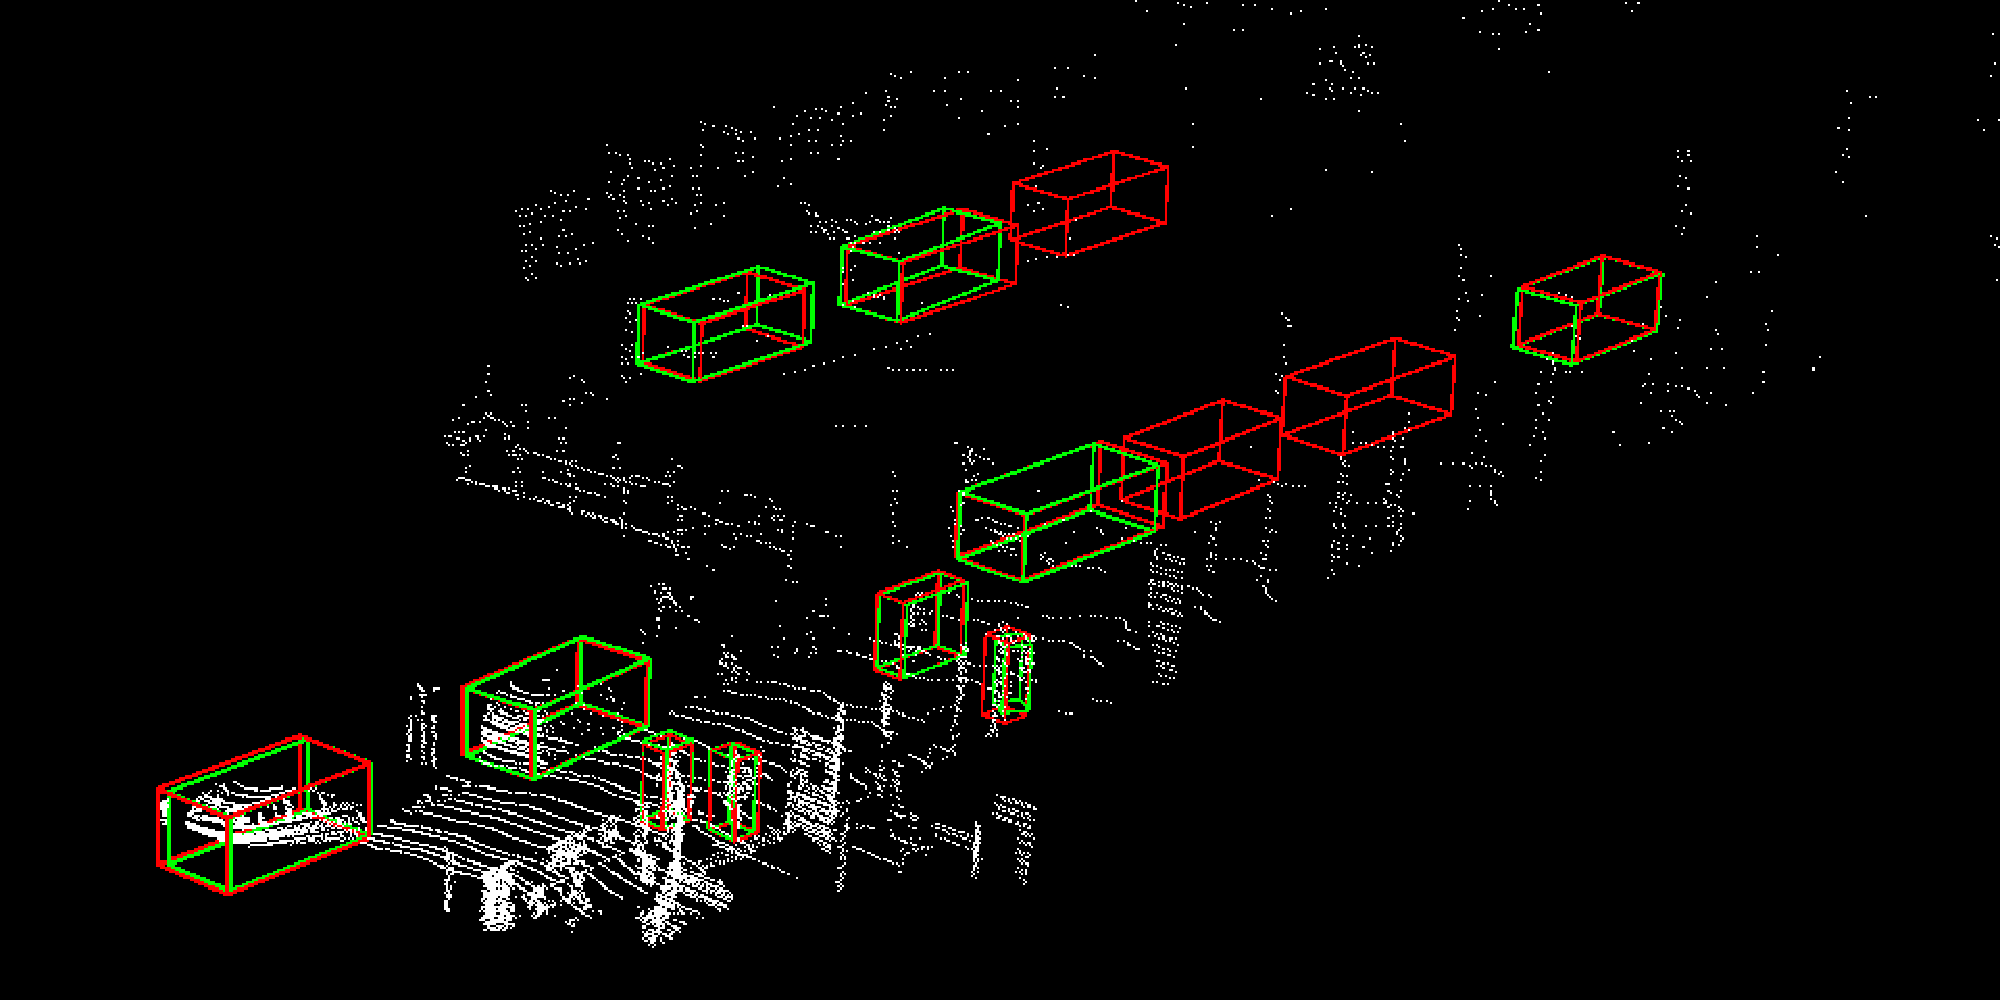}
        \end{subfigure}%
        \begin{subfigure}{\textwidth}
            \centering
            \includegraphics[width=0.99\textwidth]{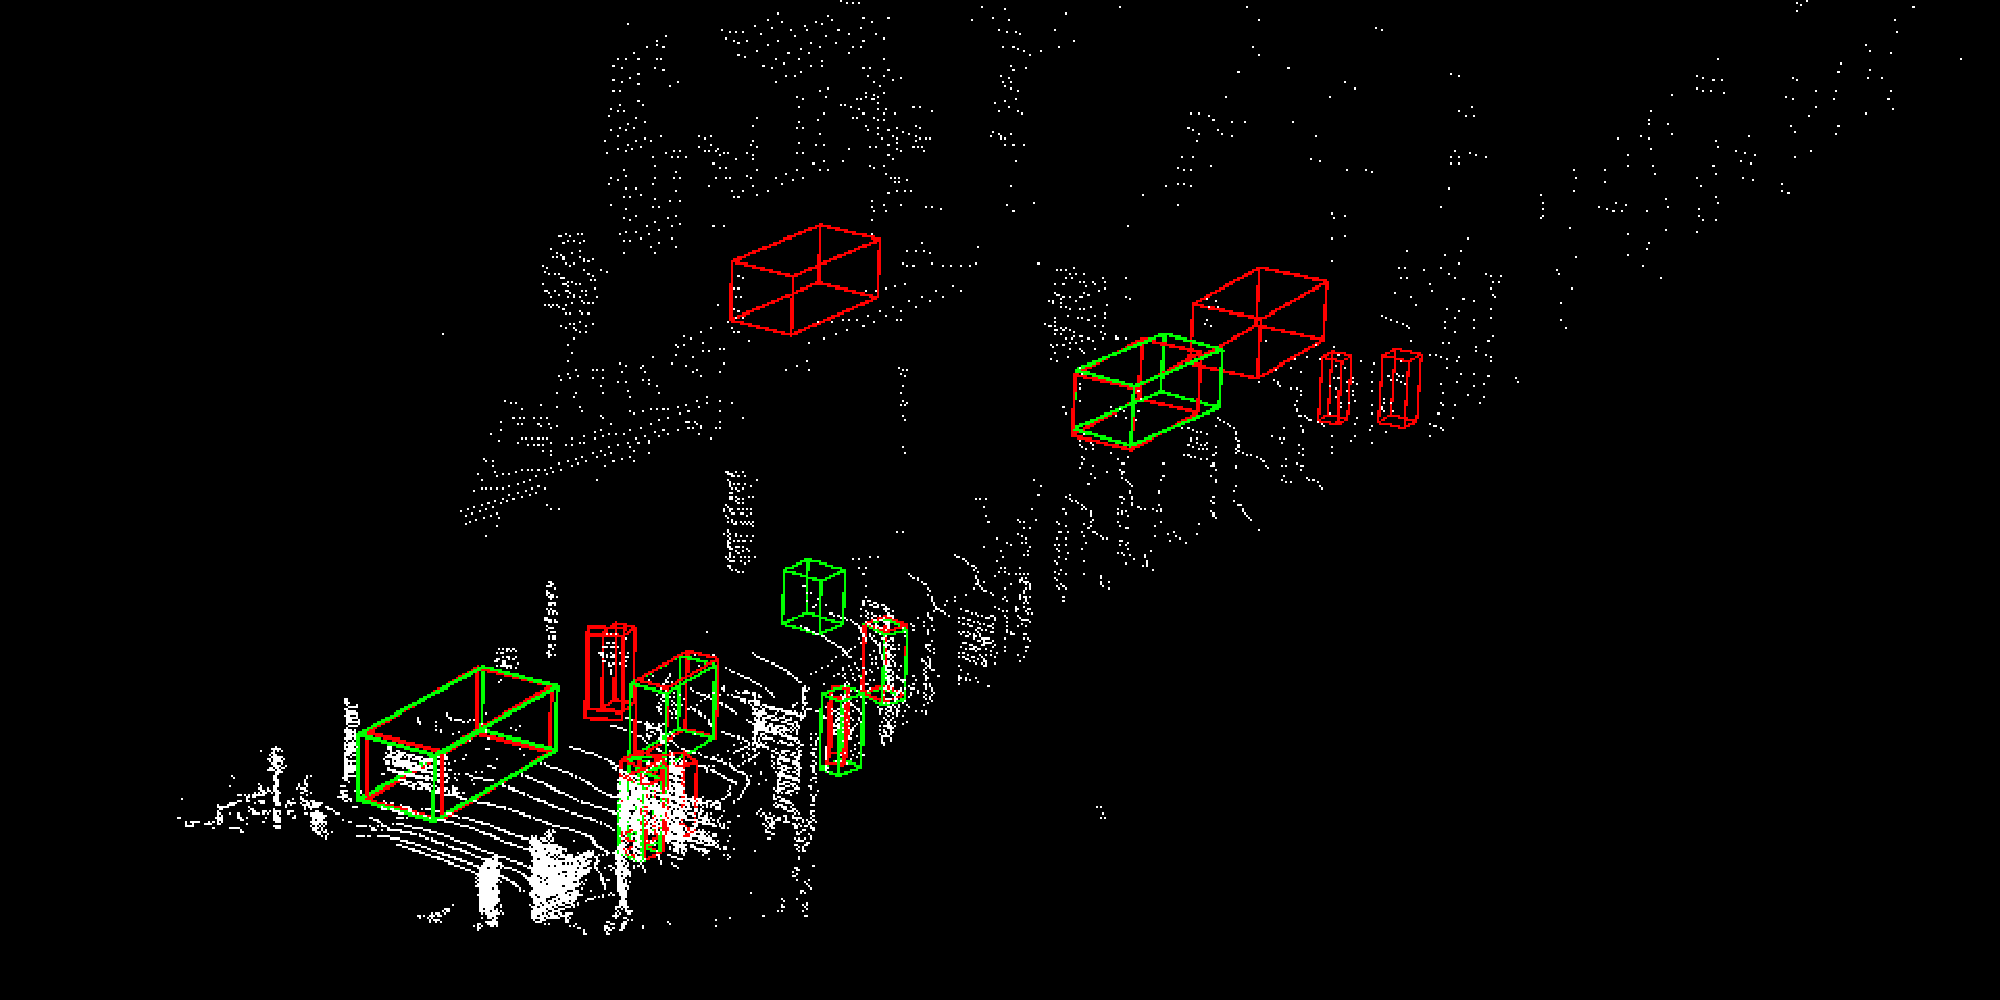}
        \end{subfigure}%
        \begin{subfigure}{\textwidth}
            \centering
            \includegraphics[width=0.99\textwidth]{figure/lidar_against_baselines_eps/pointrcnn/00162.eps}
        \end{subfigure}%
    \end{minipage}\\
\begin{minipage}[t!]{0.29\textwidth}
        \centering
        \begin{subfigure}{.5\textwidth}
            \caption{3DSSD}
        \end{subfigure}%
        \begin{subfigure}{\textwidth}
            \centering
            \includegraphics[width=.99\textwidth]{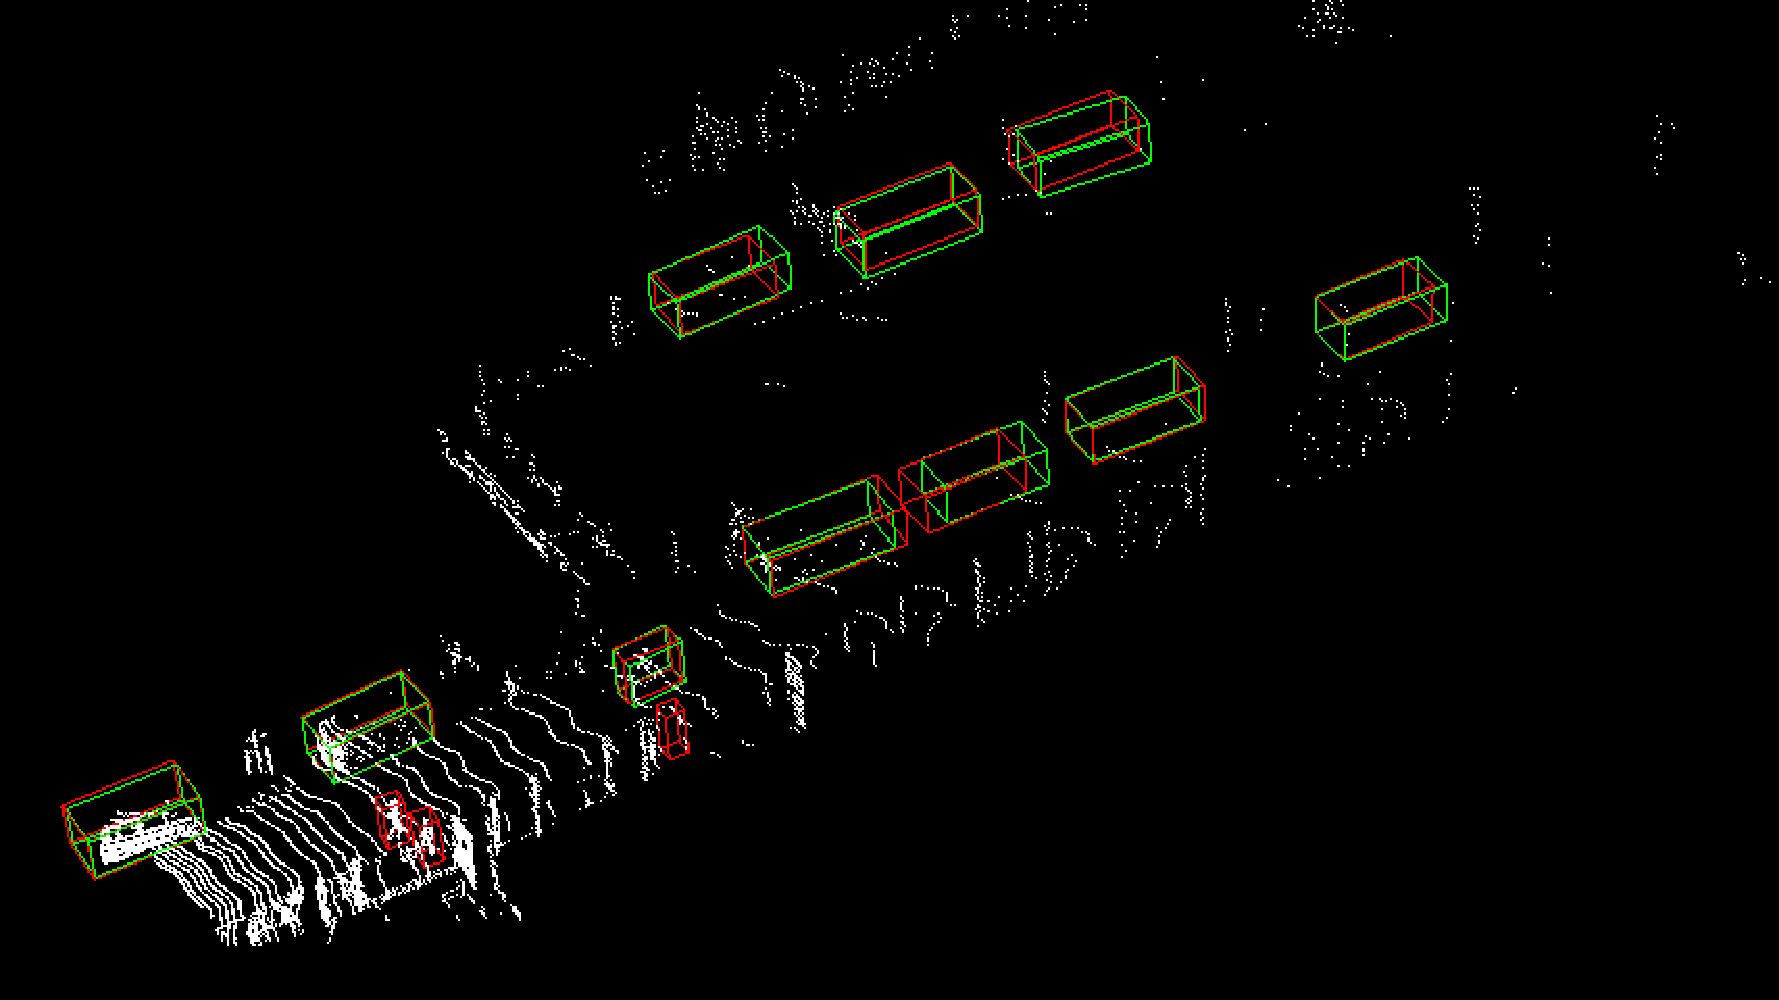}
        \end{subfigure}%
        \begin{subfigure}{\textwidth}
            \centering
            \includegraphics[width=.99\textwidth]{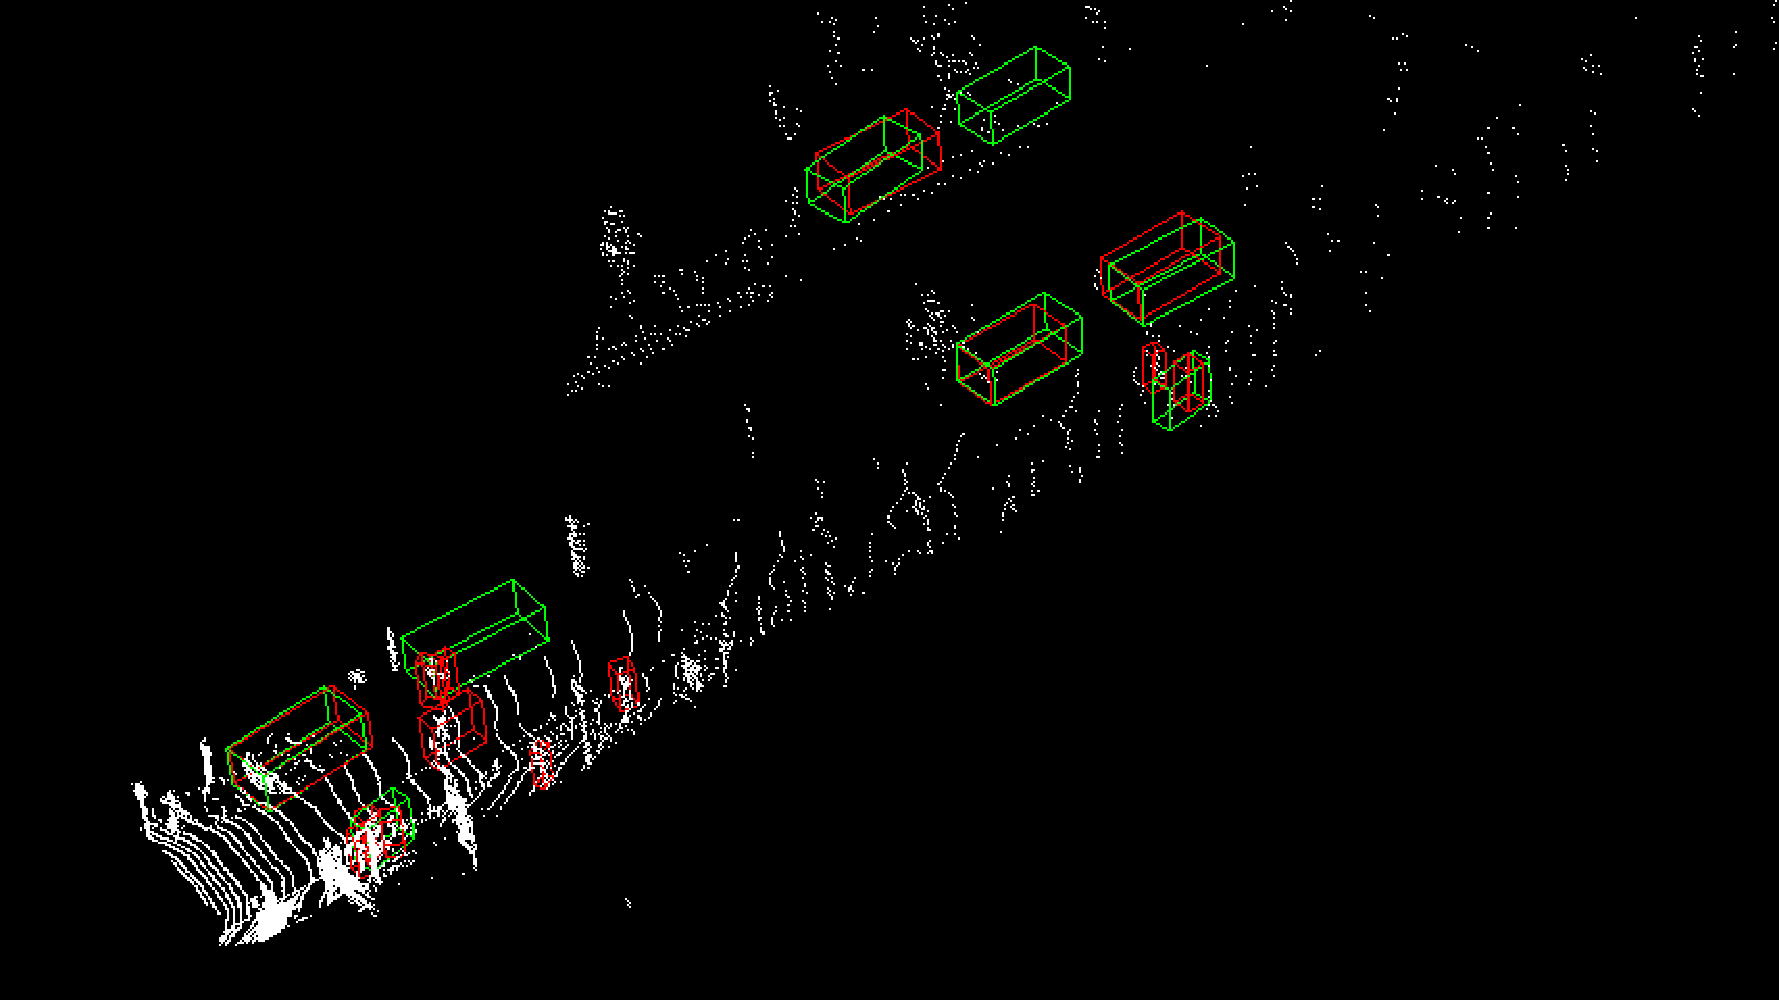}
        \end{subfigure}%
        \begin{subfigure}{\textwidth}
            \centering
            \includegraphics[width=.99\textwidth]{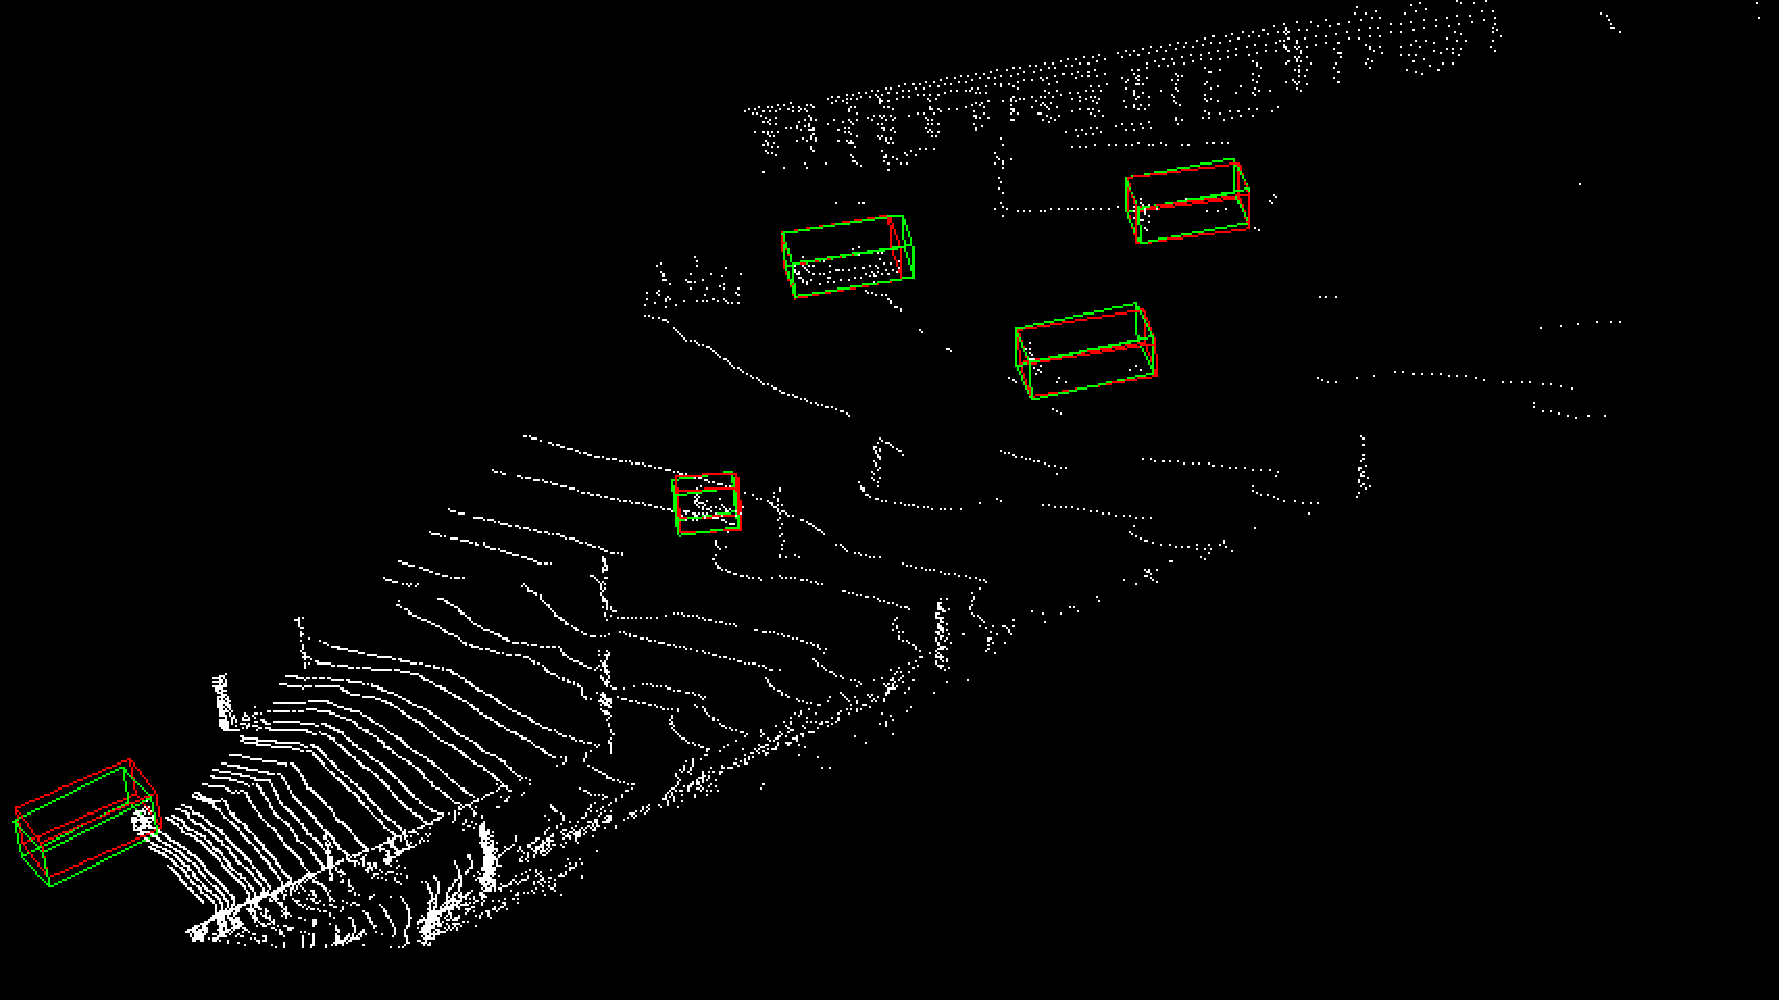}
        \end{subfigure}%
    \end{minipage}\\
    \begin{minipage}[t!]{0.29\textwidth}
        \centering
        \begin{subfigure}{.5\textwidth}
            \caption{IASSD}
        \end{subfigure}%
        \begin{subfigure}{\textwidth}
            \centering
            \includegraphics[width=0.99\textwidth]{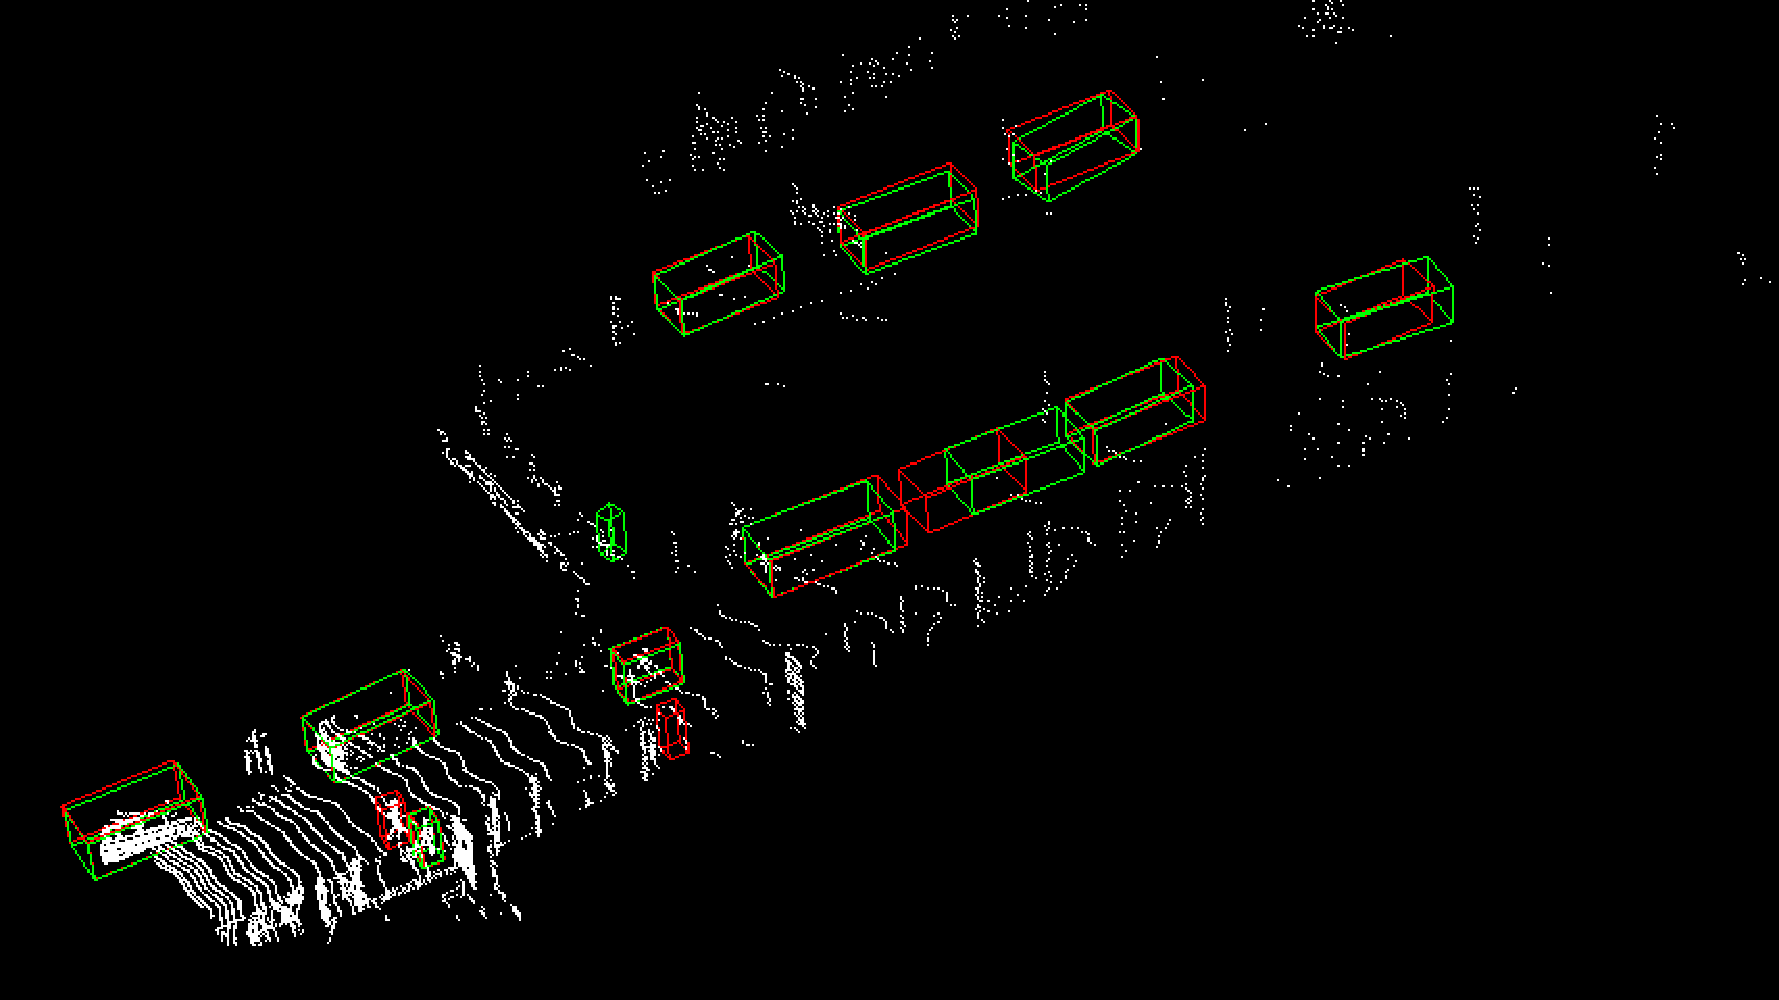}
        \end{subfigure}%
        \begin{subfigure}{\textwidth}
            \centering
            \includegraphics[width=0.99\textwidth]{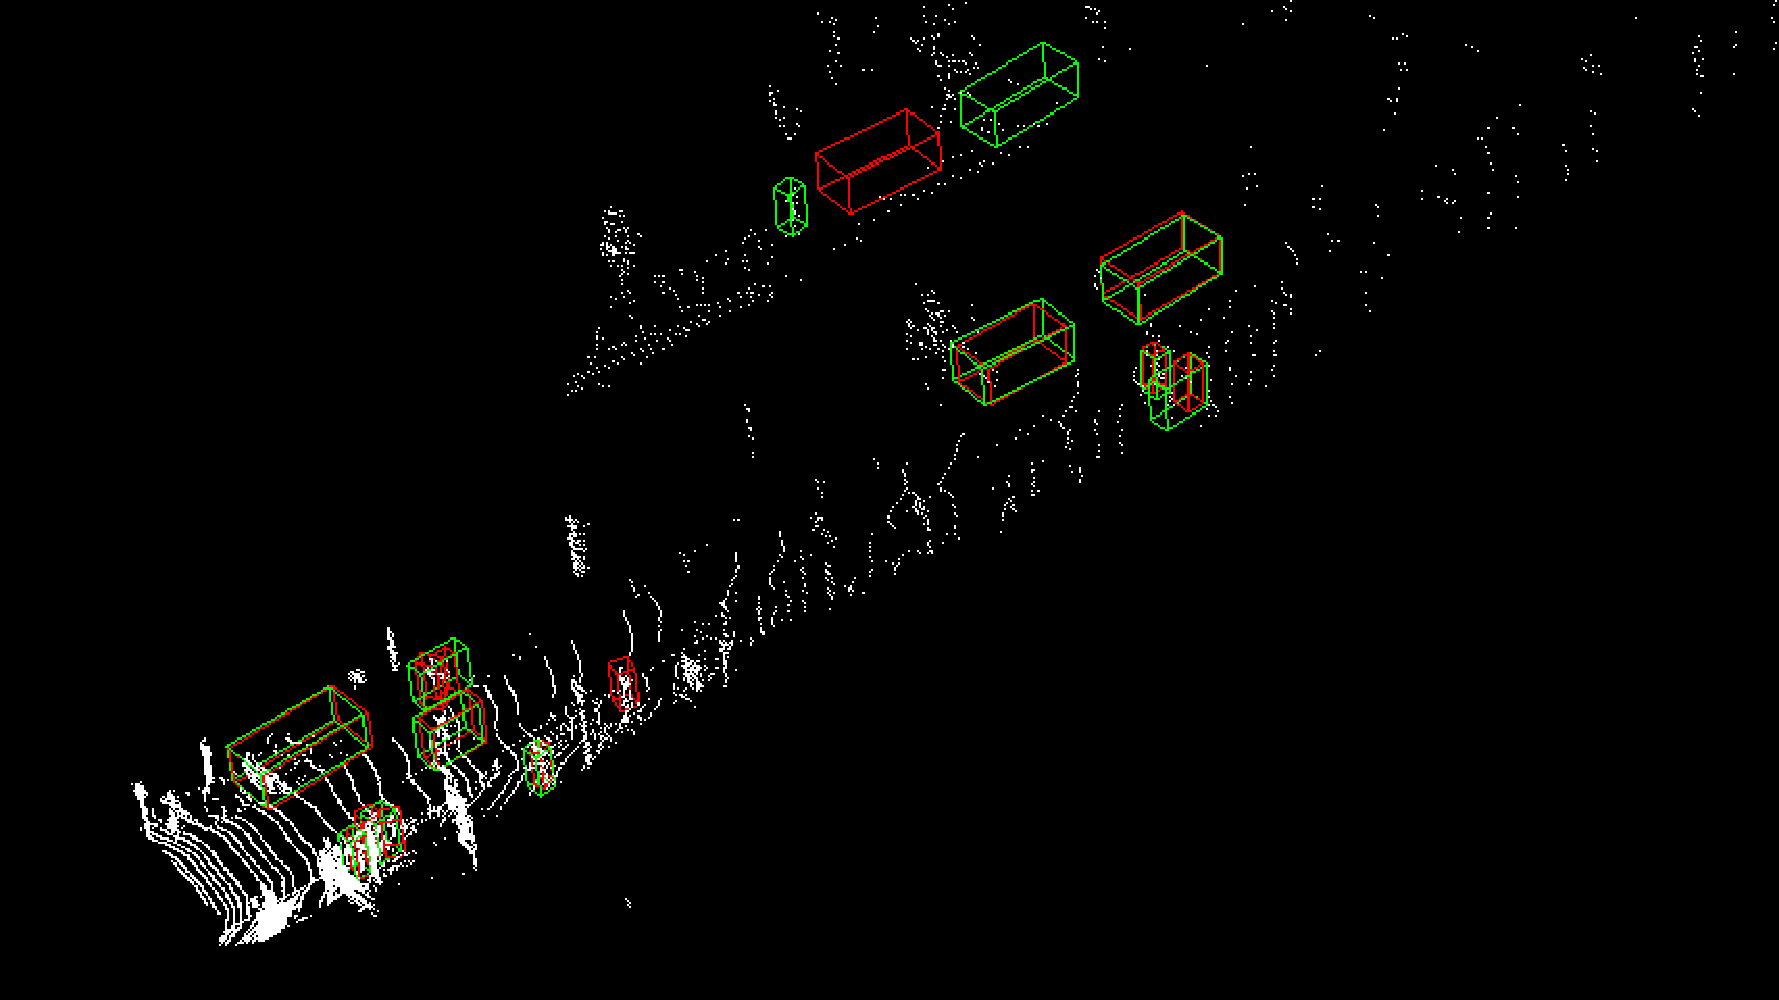}
        \end{subfigure}%
        \begin{subfigure}{\textwidth}
            \centering
            \includegraphics[width=0.99\textwidth]{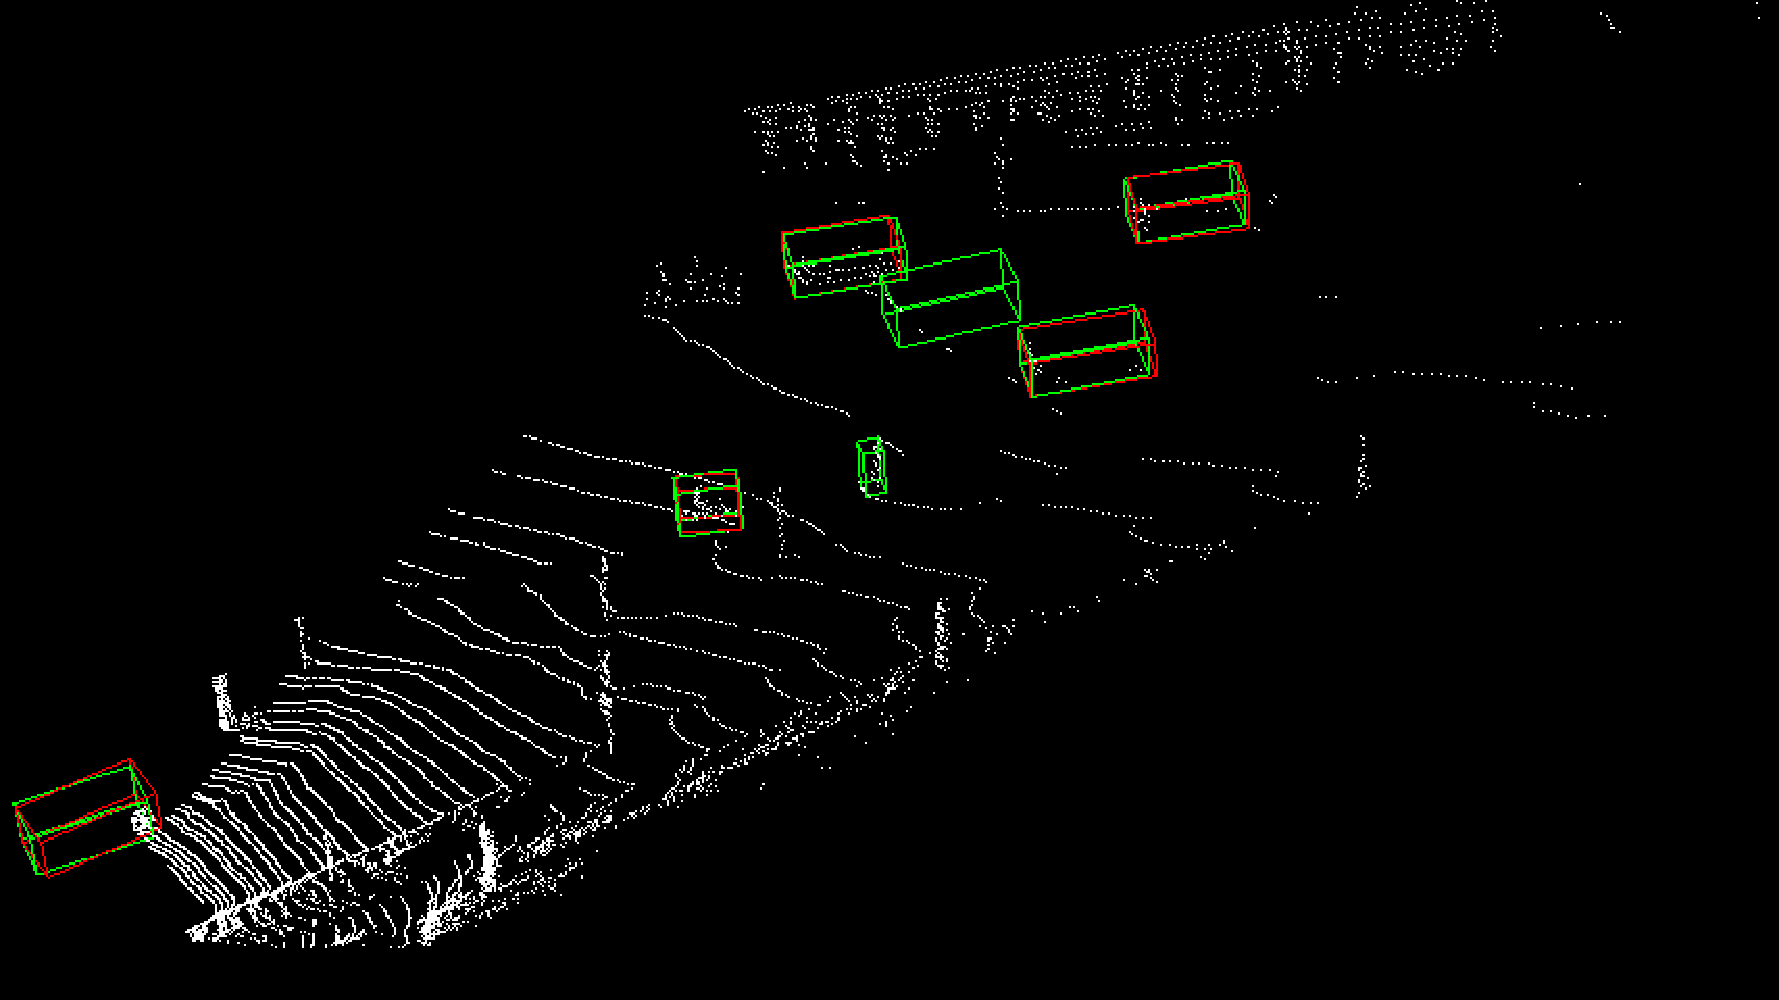}
        \end{subfigure}%
        % \begin{subfigure}{\textwidth}
        %     \centering
        %     \includegraphics[width=\textwidth]{figure/lidar_against_baselines_eps/lidar_i_lidar04740.eps}
        % \end{subfigure}%
    \end{minipage}\\
\end{figure*}
\newpage
\begin{figure*}[t]    \ContinuedFloat
    \begin{minipage}[t!]{.29\textwidth}
        \centering
        \begin{subfigure}{.5\textwidth}
            \caption{PVRCNN}
        \end{subfigure}%
        \begin{subfigure}{\textwidth}
            \centering
            \includegraphics[width=0.99\textwidth]{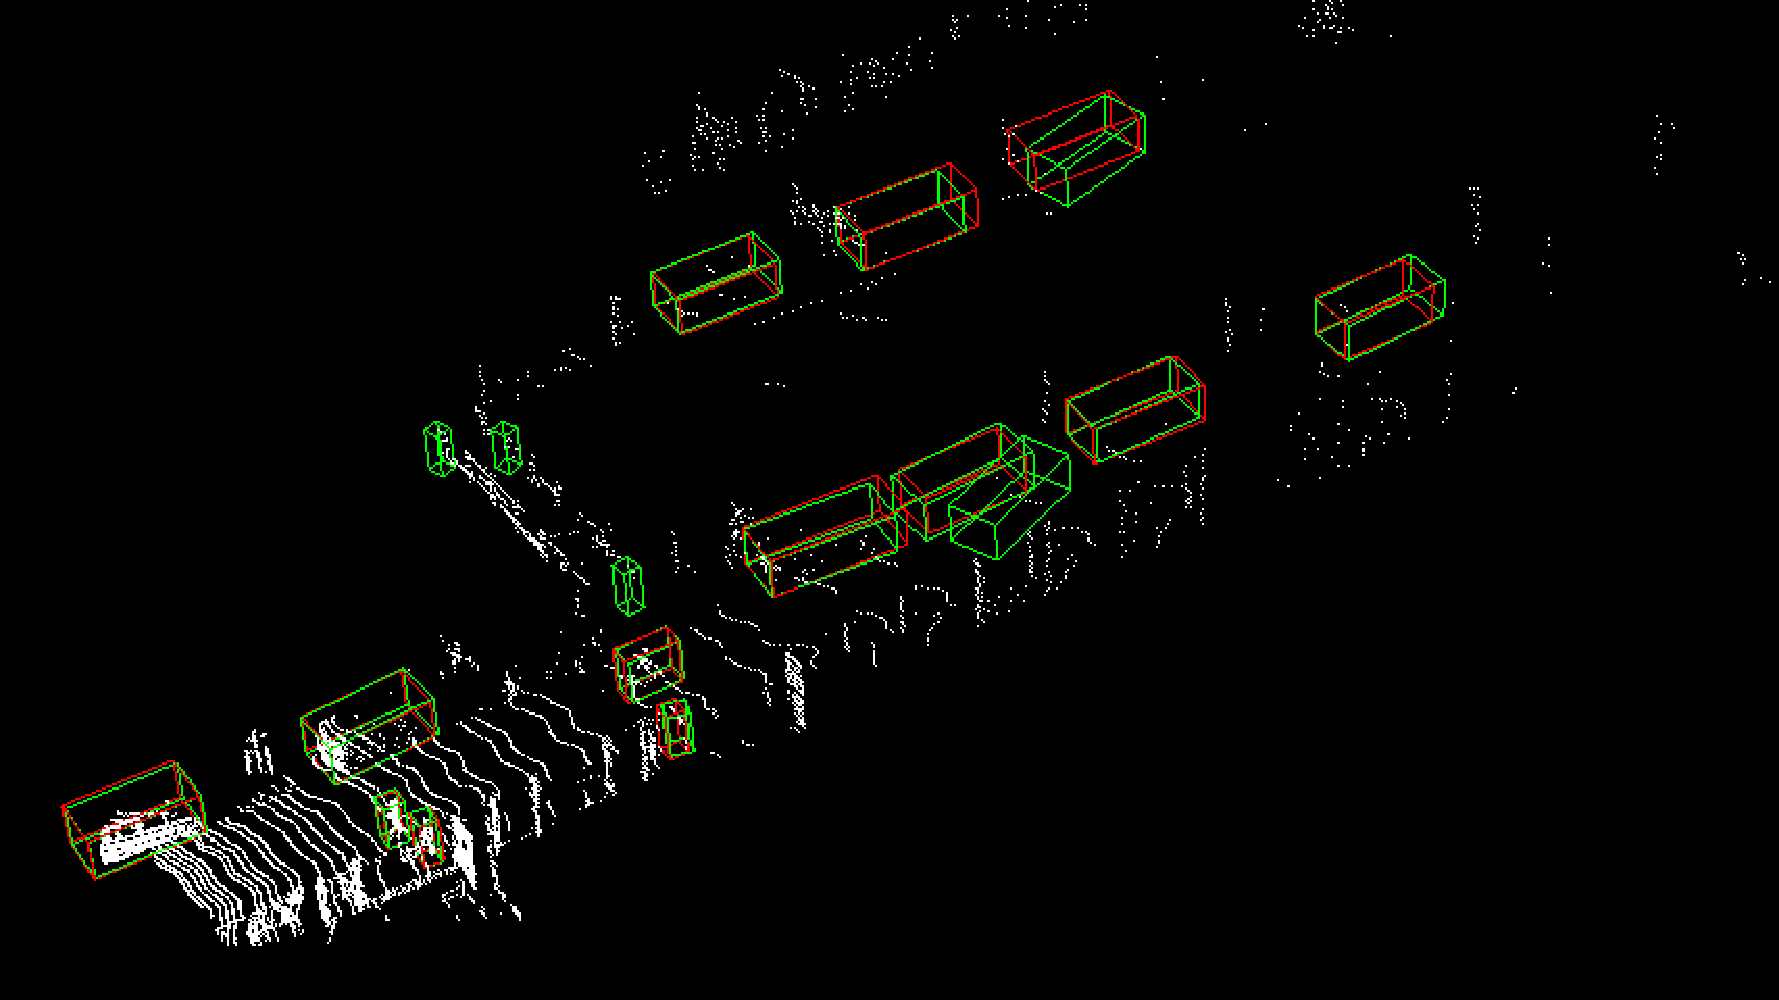}
        \end{subfigure}%
        \begin{subfigure}{\textwidth}
            \centering
            \includegraphics[width=0.99\textwidth]{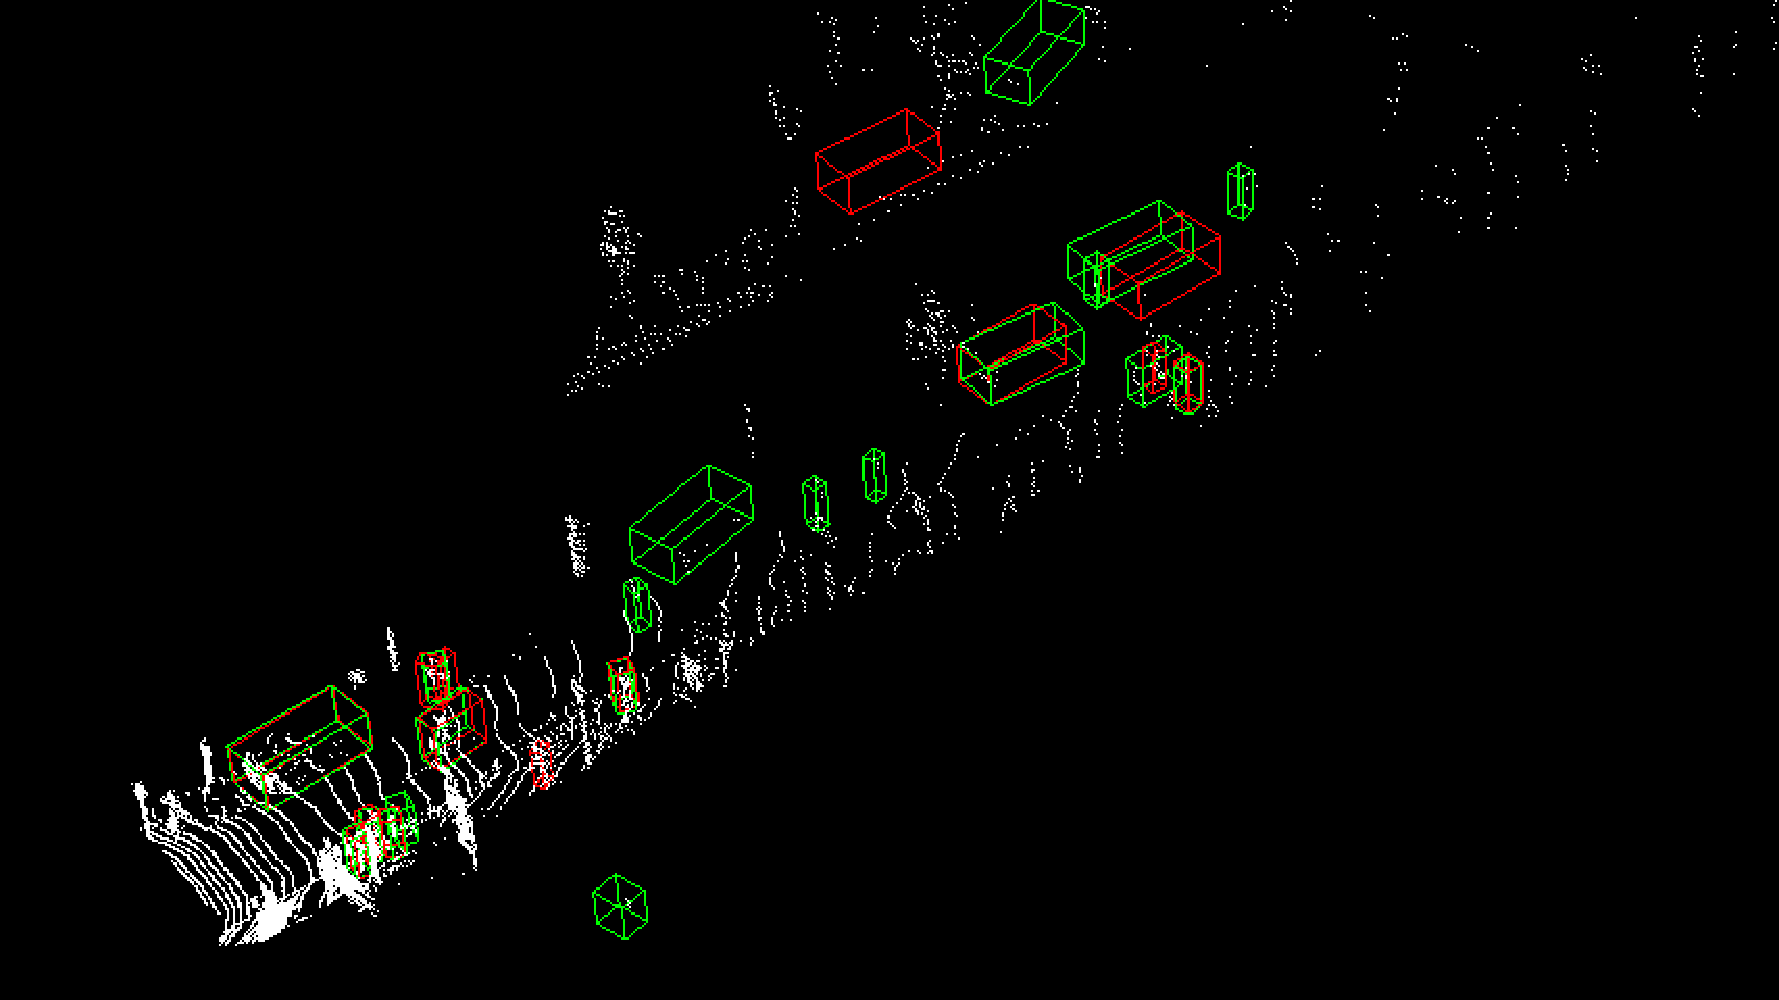}
        \end{subfigure}%
        \begin{subfigure}{\textwidth}
            \centering
            \includegraphics[width=0.99\textwidth]{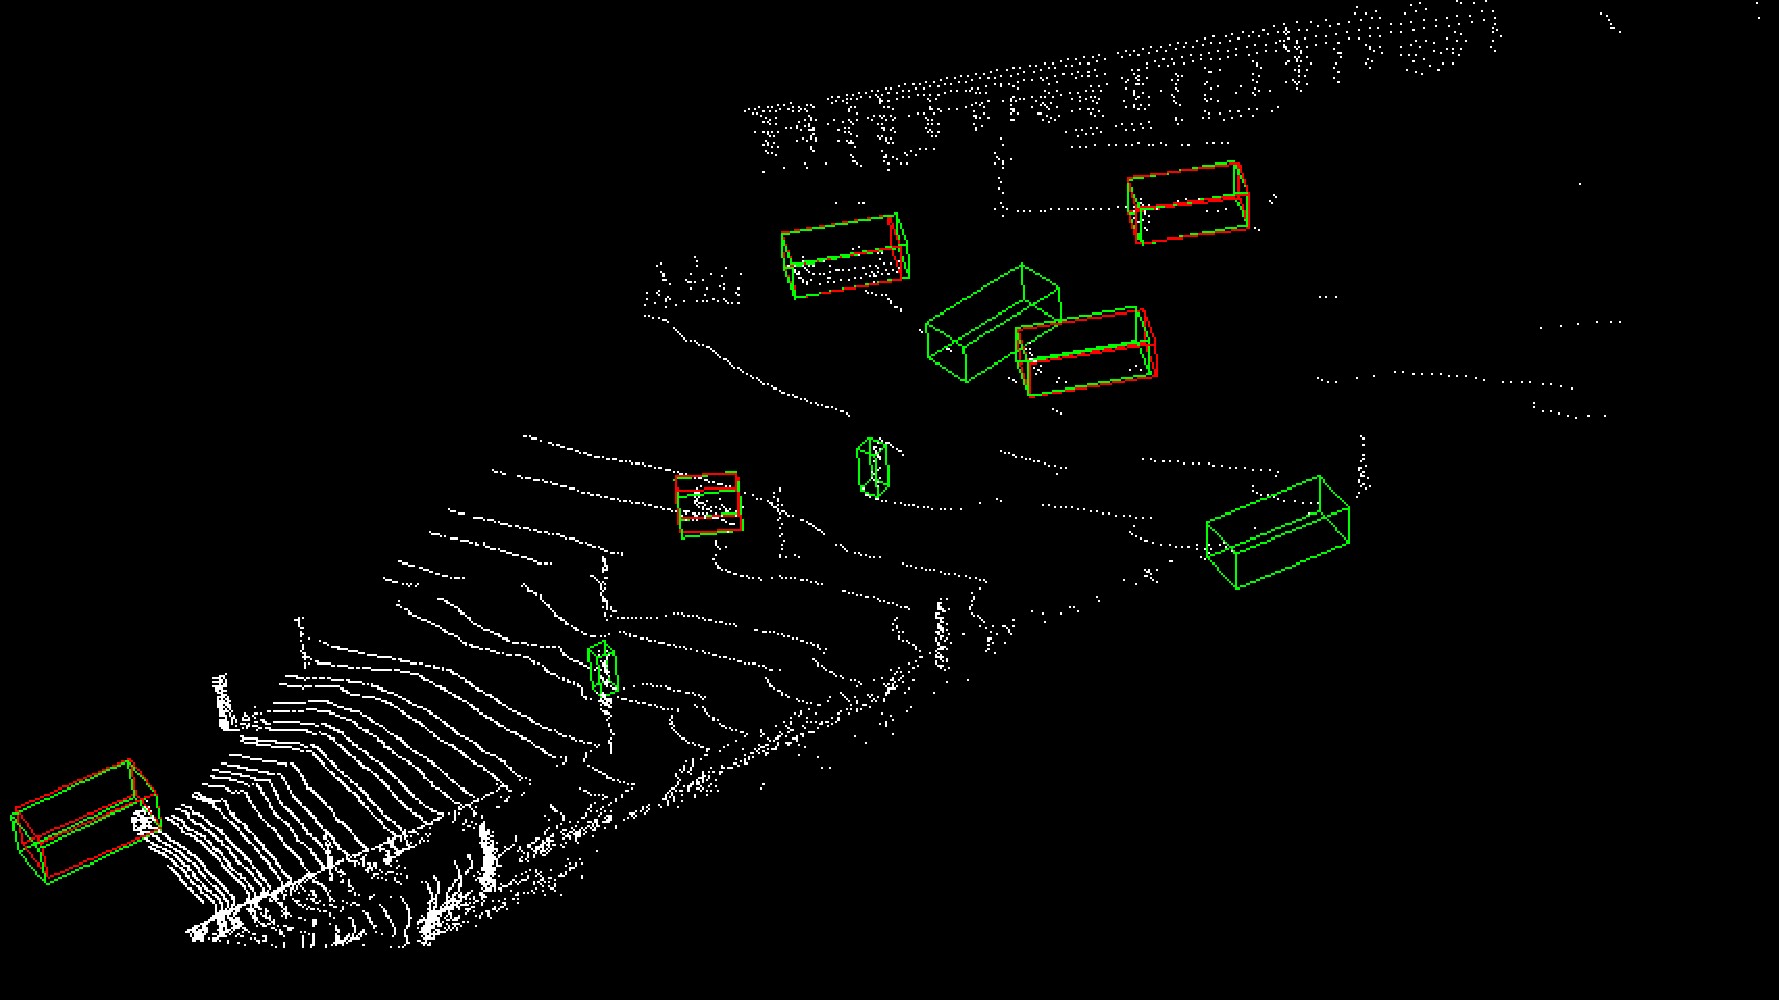}
        \end{subfigure}%
        % \begin{subfigure}{\textwidth}
        %     \centering
        %     \includegraphics[width=\textwidth]{figure/lidar_against_baselines_eps/pvrcnn_lidar04740.eps}
        % \end{subfigure}%
    \end{minipage}\\
    \caption{\gab{how many frames for comparison?}LiDAR qualitative evaluation. Predictions by different methods are shown in \textcolor{green}{green} while ground-truth bounding boxes are shown in \textcolor{red}{red}}
\end{figure*}
